# Supplementary material for: Rehearsal-Free Continual Learning over Small Non-I.I.D. Batches
Source: arXiv:1907.03799 source file (2020-04-21)
Supplement: Supplementary file 1 [file 196_AR1.tex]

\subsection{AR1*, NICv2 - 196}
\fontsize{8}{11}\selectfont
\begin{longtable}[c]{rgrgrgrgrgr}
\hline
Batch & Run 0  & Run 1  & Run 2  & Run 3  & Run 4  & Run 5  & Run 6  & Run 7  & Run 8  & Run 9  \\ \hline
\endfirsthead
\endhead
0     & 7.174  & 7.174  & 7.174  & 7.174  & 7.174  & 7.174  & 7.174  & 7.174  & 7.174  & 7.174  \\
1     & 14     & 14     & 14     & 14     & 14     & 14     & 14     & 14     & 14     & 14     \\
2     & 14.348 & 13.652 & 13.652 & 14.087 & 13.826 & 13.913 & 14.261 & 13.217 & 15.043 & 13.739 \\
3     & 14.565 & 12.652 & 13.957 & 14.565 & 13.696 & 14.609 & 15.696 & 13     & 16.609 & 14.13  \\
4     & 13.696 & 13.217 & 14.826 & 14.478 & 14.391 & 12.522 & 16.13  & 12.826 & 17.174 & 14     \\
5     & 14.957 & 13.087 & 15.304 & 14.739 & 15.217 & 13.174 & 17     & 13.217 & 16.652 & 15.87  \\
6     & 15.391 & 13.957 & 16.565 & 15.826 & 15.261 & 14.261 & 15.739 & 13     & 17.217 & 17.87  \\
7     & 15.435 & 14.87  & 17.783 & 17.522 & 16.304 & 14.304 & 15.478 & 12.826 & 17.87  & 16.087 \\
8     & 15.391 & 16.696 & 18.522 & 18.304 & 16.826 & 16.609 & 17.435 & 12.522 & 17.913 & 17.043 \\
9     & 16     & 16.783 & 16.652 & 16.304 & 17.652 & 17     & 18.174 & 12.783 & 18.217 & 17.304 \\
10    & 16.913 & 17.174 & 16.783 & 16.957 & 17.435 & 18.217 & 18.739 & 12.87  & 18.565 & 17.348 \\
11    & 17.87  & 17.435 & 17.391 & 16.435 & 16.217 & 18     & 18.696 & 13.652 & 18.739 & 17.522 \\
12    & 18.174 & 18.043 & 17.696 & 18.826 & 16.696 & 18.391 & 19     & 15     & 19.739 & 16.609 \\
13    & 17.87  & 18.304 & 18.348 & 18.522 & 16.913 & 18.13  & 18.87  & 14.609 & 20.261 & 16.435 \\
14    & 18.043 & 18.522 & 18.348 & 18.783 & 18.217 & 18.174 & 19.348 & 16.435 & 20.391 & 16.522 \\
15    & 18.739 & 19     & 19     & 18.696 & 18.957 & 20.217 & 19.739 & 16.87  & 19.391 & 16.87  \\
16    & 19     & 19.522 & 18.652 & 18.652 & 18.348 & 20.043 & 20.478 & 17.652 & 19.783 & 17.304 \\
17    & 18.826 & 19.826 & 19.261 & 19.087 & 19.783 & 19.783 & 21.783 & 17.87  & 20     & 17.957 \\
18    & 19     & 19.826 & 19.13  & 19.957 & 20.522 & 20.522 & 21.087 & 18     & 19.087 & 18.783 \\
19    & 19.435 & 20.826 & 19.348 & 20.13  & 20.609 & 20.609 & 21.217 & 18.304 & 18.696 & 20.217 \\
20    & 19.522 & 21.217 & 19.652 & 21.217 & 21.043 & 20.261 & 21.696 & 18.348 & 18.957 & 21.087 \\
21    & 19.783 & 21.783 & 19.696 & 21.565 & 21.435 & 20.174 & 21.565 & 18.391 & 19.522 & 21.13  \\
22    & 20.391 & 22.304 & 18.913 & 21.391 & 22.957 & 20.348 & 21.87  & 18.304 & 19.739 & 21.391 \\
23    & 20.522 & 22.217 & 18.217 & 21.652 & 23.696 & 20.304 & 21.87  & 18.609 & 19.826 & 21.739 \\
24    & 20.609 & 22.783 & 18.87  & 21.913 & 24.087 & 20.783 & 21.739 & 19.087 & 20.174 & 22.565 \\
25    & 20.783 & 22.609 & 19.522 & 22.348 & 24.435 & 20.783 & 21.217 & 19.391 & 21     & 23.13  \\
26    & 20.696 & 22.522 & 19.913 & 22.696 & 24.391 & 20.826 & 22.217 & 19.348 & 21.348 & 23.087 \\
27    & 21.783 & 22.217 & 21.565 & 23.783 & 24.565 & 21.696 & 22.565 & 20.652 & 21.609 & 24.174 \\
28    & 21.826 & 21.957 & 21.652 & 24.174 & 24.913 & 22.261 & 22.043 & 20.217 & 21.783 & 24.087 \\
29    & 22.217 & 21.87  & 22.696 & 24.783 & 25.913 & 21.957 & 22     & 20.391 & 22.652 & 25.522 \\
30    & 22.217 & 22.13  & 23.174 & 24.783 & 26.87  & 21.739 & 22.826 & 20.957 & 23.652 & 25.957 \\
31    & 22.435 & 22     & 23.087 & 24.565 & 27.174 & 21.913 & 22.826 & 21.783 & 23.826 & 25.783 \\
32    & 22.522 & 23.13  & 23.391 & 25.261 & 27.304 & 22.261 & 21.652 & 22.043 & 24.304 & 25.87  \\
33    & 22.783 & 23.304 & 23.913 & 25.174 & 27.609 & 22.826 & 22.565 & 21.957 & 24.348 & 25.913 \\
34    & 23.478 & 23.478 & 23.565 & 25.043 & 28.348 & 22.565 & 23.043 & 21.783 & 24.043 & 26.348 \\
35    & 23.826 & 23.435 & 24.478 & 25     & 28.957 & 22.696 & 23.261 & 21.913 & 24.087 & 26.261 \\
36    & 24.739 & 23.696 & 24.348 & 25.217 & 29.522 & 22.913 & 23.478 & 22.87  & 24.957 & 26.696 \\
37    & 25.087 & 24.087 & 24.478 & 25.217 & 30.13  & 22.087 & 23.826 & 23.043 & 25.391 & 26.913 \\
38    & 25.043 & 24.174 & 24.609 & 25.348 & 30.435 & 21.783 & 24.174 & 23.783 & 25.783 & 26.435 \\
39    & 24.826 & 24.478 & 24.696 & 25.304 & 30.217 & 21     & 24.043 & 24.217 & 26.304 & 26.522 \\
40    & 25.522 & 24.435 & 25.087 & 25.739 & 30.522 & 21.348 & 25.261 & 24.435 & 26.348 & 27.913 \\
41    & 25.913 & 24.478 & 25.348 & 26.13  & 30.913 & 21.391 & 25.304 & 24.391 & 26.13  & 27.348 \\
42    & 25.957 & 24.696 & 25.87  & 26.783 & 30.957 & 22     & 26.217 & 24.261 & 25.826 & 27.696 \\
43    & 26.435 & 25.913 & 26.348 & 26.87  & 30.652 & 22.174 & 26.478 & 24.609 & 26.261 & 28.13  \\
44    & 25.913 & 26.13  & 26.609 & 26.174 & 32.13  & 22.913 & 26.826 & 24.957 & 26.348 & 28.087 \\
45    & 26.13  & 26.261 & 25.957 & 27.304 & 32.217 & 22.522 & 26.87  & 24.957 & 26.87  & 30.043 \\
46    & 26.739 & 26.043 & 25.565 & 27.261 & 32.174 & 22.565 & 27.522 & 25.435 & 26.913 & 31.087 \\
47    & 26.957 & 26.087 & 25.435 & 27.13  & 32.261 & 23.348 & 28.348 & 25.87  & 27.261 & 31.696 \\
48    & 26.957 & 26.87  & 25.565 & 27.565 & 32.304 & 23.609 & 29.217 & 26.304 & 27.609 & 31.913 \\
49    & 26.348 & 27.304 & 25.696 & 28.304 & 32.652 & 25.348 & 29.13  & 27.174 & 27.739 & 32.348 \\
50    & 26.826 & 27.652 & 25.87  & 28.478 & 33.522 & 25.565 & 29.478 & 27.565 & 27.87  & 32.043 \\
51    & 26.696 & 28.043 & 26.783 & 28.739 & 33.304 & 25.739 & 29.609 & 27.435 & 28.696 & 32.13  \\
52    & 26.696 & 28.478 & 27.13  & 28.783 & 32.913 & 25.957 & 30.652 & 27.522 & 29.783 & 32.13  \\
53    & 27.304 & 28.478 & 27.261 & 28.957 & 33.043 & 26.522 & 30.739 & 27.522 & 29.826 & 32.652 \\
54    & 27.87  & 29.174 & 28     & 30.565 & 33.174 & 26.913 & 30.87  & 27.739 & 30.174 & 32.696 \\
55    & 27.652 & 29.957 & 28.957 & 30.783 & 33.391 & 27.522 & 30.826 & 27.826 & 31.87  & 33.174 \\
56    & 28.304 & 30     & 27.87  & 30.957 & 33.87  & 25.957 & 31.609 & 27.826 & 32.348 & 34.609 \\
57    & 28.348 & 31.478 & 27.739 & 31.087 & 33.826 & 26.174 & 32.391 & 27.826 & 32.391 & 35.043 \\
58    & 28.087 & 31.783 & 27.826 & 31.087 & 33.826 & 26.348 & 32.826 & 28.087 & 32.435 & 35     \\
59    & 29.087 & 32.304 & 27.87  & 31.391 & 33.696 & 26.565 & 32.609 & 28.13  & 32.391 & 35.739 \\
60    & 29.348 & 32.174 & 28.652 & 32     & 33.913 & 26.957 & 32.435 & 28.522 & 32.478 & 35.87  \\
61    & 29.565 & 32.391 & 28.609 & 33.043 & 34     & 27.217 & 32.783 & 28.739 & 33.174 & 35.913 \\
62    & 29.739 & 32.217 & 28.87  & 33.739 & 34.087 & 27.304 & 33.087 & 28.826 & 33.696 & 35.87  \\
63    & 29.783 & 32.304 & 28.87  & 34.739 & 34.696 & 27.478 & 32.783 & 29.217 & 33.696 & 36.522 \\
64    & 30.435 & 32.957 & 29.565 & 35.696 & 35     & 27.87  & 33.391 & 30.174 & 33.783 & 36.478 \\
65    & 30.217 & 33.609 & 29.783 & 36.13  & 35.261 & 28.087 & 34.565 & 30.304 & 34.652 & 37.348 \\
66    & 30.565 & 34.261 & 30.13  & 36.435 & 34.913 & 29     & 35.174 & 30.261 & 34.087 & 37.261 \\
67    & 30.913 & 35.174 & 30.261 & 36.565 & 35.826 & 29.609 & 35.043 & 30.435 & 34.304 & 37.348 \\
68    & 30.913 & 35.304 & 31.652 & 36.696 & 35.783 & 29.87  & 35.217 & 31.783 & 34.913 & 37.565 \\
69    & 31.174 & 35.261 & 32.217 & 36.826 & 35.696 & 30.217 & 35.261 & 31.783 & 35.391 & 38.087 \\
70    & 31.304 & 35.522 & 32.609 & 36.522 & 35.739 & 30.478 & 35     & 32.043 & 35.478 & 38.478 \\
71    & 31     & 35.609 & 32.609 & 36.913 & 35.522 & 30.783 & 35.043 & 32.913 & 35.304 & 37     \\
72    & 32.217 & 35.87  & 33.348 & 37.087 & 35.435 & 31.174 & 35.174 & 33.217 & 36.609 & 38.696 \\
73    & 32.261 & 36.217 & 33.435 & 38.435 & 35.261 & 31     & 35.783 & 33.348 & 36.652 & 38.652 \\
74    & 32.522 & 36.391 & 33.348 & 37.957 & 35.348 & 31.348 & 36.391 & 33.87  & 36.696 & 39     \\
75    & 32.87  & 36.696 & 33.783 & 38.13  & 35.217 & 31.652 & 36.783 & 34.087 & 36.739 & 39.348 \\
76    & 33.217 & 36.696 & 34.13  & 38.391 & 35.696 & 31.739 & 36.913 & 34.391 & 37.13  & 40.13  \\
77    & 33.522 & 37.13  & 34.087 & 38.783 & 35.696 & 32.13  & 36.913 & 34.435 & 37.043 & 40.087 \\
78    & 33.652 & 37.522 & 34.304 & 39     & 36.261 & 33.348 & 37     & 34.522 & 38.043 & 39.522 \\
79    & 33.652 & 37.957 & 34.348 & 38.913 & 36.13  & 33.87  & 37.13  & 34.913 & 38.87  & 39.522 \\
80    & 33.739 & 38.391 & 35.087 & 39.391 & 36.261 & 34.739 & 37.87  & 35.522 & 38.739 & 39.87  \\
81    & 33.565 & 34.478 & 36.217 & 40.043 & 36.652 & 34.174 & 38.304 & 35.696 & 38.435 & 39.826 \\
82    & 33.826 & 34.957 & 36.652 & 40.217 & 37.217 & 35.609 & 38.261 & 35.652 & 38.652 & 41.522 \\
83    & 34     & 38.174 & 36.739 & 40.652 & 37.783 & 35.609 & 38.522 & 35.739 & 38.609 & 41.304 \\
84    & 34.043 & 38.522 & 36.522 & 41.087 & 38.348 & 35.565 & 39.348 & 35.957 & 39.087 & 41.87  \\
85    & 33.957 & 39     & 36.652 & 42.87  & 38.478 & 37.348 & 39.217 & 36.13  & 39.304 & 42.217 \\
86    & 34.087 & 38.913 & 36.913 & 42.783 & 38.783 & 37.739 & 39.174 & 36.391 & 39.348 & 42.174 \\
87    & 34.261 & 39.435 & 36.565 & 42.783 & 39.174 & 37.739 & 40.478 & 36.522 & 39.043 & 42.174 \\
88    & 34.87  & 39.478 & 36.652 & 43.087 & 39.522 & 38     & 40.478 & 37.261 & 39.435 & 42.522 \\
89    & 34.87  & 39.043 & 36.435 & 43.478 & 39.913 & 38.348 & 40.826 & 37.478 & 39.478 & 42.261 \\
90    & 35.13  & 39.696 & 36.13  & 44     & 40.043 & 38.652 & 40.478 & 37.87  & 39.696 & 42.609 \\
91    & 35.087 & 40.783 & 36.13  & 44.522 & 40.13  & 38.783 & 40.913 & 38.087 & 39.696 & 42.783 \\
92    & 34.957 & 41.391 & 36.261 & 44.304 & 40.043 & 39.087 & 41     & 38.391 & 40.13  & 43.261 \\
93    & 35.304 & 41.783 & 35.913 & 44.261 & 40.261 & 39.043 & 41.043 & 38.478 & 40.174 & 42.696 \\
94    & 35.609 & 42.261 & 36     & 44.609 & 40.217 & 39.435 & 40.913 & 38.739 & 40.652 & 42.348 \\
95    & 35.696 & 41.87  & 35.957 & 45.391 & 40.565 & 39.435 & 41.565 & 39.043 & 40.652 & 42.783 \\
96    & 36.174 & 42.261 & 37.304 & 44.913 & 40.261 & 39.565 & 41.739 & 39.043 & 41.043 & 42.478 \\
97    & 36.13  & 42.13  & 37.435 & 45.087 & 40.522 & 39.913 & 41.739 & 39     & 41.391 & 43.087 \\
98    & 36.13  & 42.174 & 37.783 & 44.783 & 41     & 39.739 & 42.391 & 38.87  & 41.522 & 43.304 \\
99    & 37.522 & 42.348 & 37.87  & 44.87  & 41.87  & 39.609 & 42.348 & 39.522 & 41.913 & 43.348 \\
100   & 38.522 & 43     & 38.13  & 45.217 & 42.478 & 40.739 & 43.087 & 39.913 & 42.652 & 43.652 \\
101   & 38.565 & 44.087 & 38.261 & 45.478 & 42.696 & 40.913 & 43.174 & 40     & 42.826 & 43.826 \\
102   & 38.783 & 44.652 & 39.13  & 46.043 & 42.652 & 41     & 43.609 & 39.783 & 43.391 & 44.261 \\
103   & 39.609 & 43.739 & 39.478 & 46.043 & 43.261 & 41.174 & 43.826 & 40.435 & 43.783 & 44.304 \\
104   & 39.87  & 44     & 40.565 & 45.783 & 43.174 & 41.174 & 44.087 & 40.913 & 43.913 & 44.696 \\
105   & 41.043 & 44.826 & 41.304 & 45.826 & 43.391 & 41.478 & 44.043 & 41.652 & 44.304 & 45.13  \\
106   & 41.609 & 44.826 & 41.043 & 45.826 & 42.565 & 41.478 & 44     & 42.174 & 45.13  & 45.609 \\
107   & 41.609 & 45.304 & 41.043 & 46.348 & 42.565 & 41.652 & 45.565 & 42.261 & 45.348 & 45.913 \\
108   & 41.652 & 45.609 & 41.217 & 45.913 & 42.391 & 42.043 & 45.522 & 42.348 & 45.565 & 45.391 \\
109   & 41.609 & 45.522 & 41.391 & 45.609 & 42.391 & 42.13  & 45.696 & 43.304 & 45.652 & 45.217 \\
110   & 41.913 & 45.348 & 41.087 & 45.913 & 42.217 & 42.043 & 45.652 & 44.13  & 45.913 & 46.261 \\
111   & 41.913 & 45.13  & 41.13  & 46.783 & 43.217 & 42.565 & 46.043 & 44.348 & 46.565 & 46.348 \\
112   & 42     & 44.913 & 41.391 & 47     & 43.174 & 42.739 & 46.304 & 44.783 & 47.13  & 46.391 \\
113   & 41.913 & 45.087 & 41.739 & 46.826 & 43.609 & 42.391 & 46.609 & 44.478 & 47.217 & 46.478 \\
114   & 42     & 45.391 & 42.043 & 47.13  & 43.826 & 43.478 & 47.217 & 45     & 47.609 & 45.957 \\
115   & 42.522 & 46.435 & 42.435 & 47.304 & 43.783 & 43.391 & 47.435 & 45.087 & 47.652 & 46.348 \\
116   & 42.913 & 45.783 & 42.609 & 47.348 & 43.652 & 43.478 & 47.826 & 45.348 & 47.87  & 46.565 \\
117   & 43.087 & 47.174 & 43.478 & 48.87  & 43.522 & 43.478 & 48.435 & 45.913 & 47.87  & 46.696 \\
118   & 43.435 & 47.913 & 44.043 & 49.696 & 43.652 & 44.652 & 48.435 & 46.478 & 48.391 & 46.913 \\
119   & 43.348 & 48.087 & 44.435 & 49.739 & 43.739 & 45.478 & 48.652 & 46.522 & 48.565 & 47.13  \\
120   & 43.261 & 49.217 & 44.565 & 49.783 & 43.826 & 45.783 & 50     & 46.739 & 48.609 & 47.348 \\
121   & 43.304 & 49.304 & 45.13  & 49.696 & 44.391 & 46.304 & 50.13  & 47.435 & 50.348 & 47.652 \\
122   & 43.435 & 50.348 & 45.087 & 50.087 & 44.348 & 47.217 & 50.826 & 48.217 & 50.435 & 47.696 \\
123   & 43.348 & 50.435 & 45.478 & 50.217 & 45.435 & 46.826 & 50.783 & 48.435 & 50.957 & 47.522 \\
124   & 43.435 & 51     & 45.391 & 50.478 & 44.957 & 47.348 & 50.696 & 48.783 & 51.478 & 47.565 \\
125   & 43.739 & 51.304 & 45.913 & 50.652 & 45.304 & 47.217 & 50.957 & 48.87  & 50.739 & 47.826 \\
126   & 43.565 & 51.609 & 46.043 & 50.696 & 45.174 & 44     & 51.043 & 49.043 & 50.739 & 48.043 \\
127   & 43.565 & 51.652 & 46.087 & 51.087 & 45.217 & 43.957 & 51.696 & 49.609 & 50.609 & 48.13  \\
128   & 43.87  & 51.609 & 46.13  & 51.348 & 47.13  & 44.696 & 51.739 & 49.913 & 51.609 & 48.391 \\
129   & 43.783 & 51.652 & 46.13  & 51.696 & 47.348 & 44.522 & 51.696 & 49.87  & 52     & 48     \\
130   & 43.826 & 52.13  & 46.087 & 51.522 & 47.609 & 47.565 & 51.957 & 50.304 & 52.174 & 48.435 \\
131   & 43.826 & 52.13  & 45.826 & 51.696 & 47.478 & 49.348 & 51.478 & 50.087 & 52.087 & 48.652 \\
132   & 44.087 & 52.217 & 46.13  & 51.652 & 47.522 & 49.435 & 51.913 & 51.261 & 52.13  & 48.913 \\
133   & 44.565 & 52.261 & 46.565 & 52.043 & 48.13  & 49.478 & 51.957 & 51.739 & 52.348 & 50.348 \\
134   & 45.087 & 52.304 & 46.435 & 51.87  & 47.913 & 49.652 & 52     & 52.696 & 52.478 & 50     \\
135   & 44.739 & 52.87  & 47     & 52.043 & 48.87  & 50.13  & 51.957 & 52.609 & 52.609 & 49.913 \\
136   & 45.913 & 52.913 & 47.217 & 52.087 & 49.391 & 50.348 & 52.696 & 52.739 & 52.478 & 50.087 \\
137   & 46.478 & 53.391 & 48.174 & 52.261 & 49.13  & 50.609 & 52.826 & 52.739 & 52.957 & 50.217 \\
138   & 46.565 & 53.304 & 48.391 & 52.174 & 50.13  & 50.522 & 53.261 & 53.087 & 52.217 & 50.696 \\
139   & 46.696 & 53.696 & 49     & 52.696 & 49.652 & 51.043 & 53.522 & 53.696 & 52.261 & 51.087 \\
140   & 46.739 & 53.913 & 49.304 & 52.565 & 49.522 & 51.087 & 53.739 & 53.739 & 52.348 & 51.652 \\
141   & 47.217 & 54.652 & 49.652 & 52.565 & 49.783 & 51.348 & 54.522 & 53.913 & 53     & 51.696 \\
142   & 47.783 & 54.826 & 49.087 & 52.652 & 50.261 & 52.043 & 54.87  & 53.652 & 53.217 & 51.87  \\
143   & 47.913 & 54.783 & 49.565 & 53.609 & 50.957 & 52.565 & 54.609 & 54.696 & 53.261 & 51.739 \\
144   & 48.087 & 55.13  & 50.261 & 54.043 & 51.261 & 52.783 & 54.565 & 54.435 & 52.913 & 52.217 \\
145   & 48.565 & 55.435 & 50.13  & 53.913 & 51.826 & 52.957 & 55.435 & 54.348 & 53.217 & 52.304 \\
146   & 49.696 & 55.783 & 51.261 & 54.609 & 51.565 & 52.739 & 55.522 & 54.696 & 53.783 & 52.478 \\
147   & 50.174 & 55.957 & 51.609 & 55.043 & 52.261 & 53     & 56.13  & 54.652 & 53.435 & 52.304 \\
148   & 50.435 & 56.391 & 51.957 & 55.174 & 52.913 & 52.783 & 56.13  & 55.565 & 53.174 & 52.043 \\
149   & 50.739 & 56.696 & 52.043 & 55.565 & 52.304 & 52.522 & 56     & 55.652 & 53     & 52.261 \\
150   & 51.217 & 56.609 & 53.043 & 55.739 & 53.13  & 52.783 & 56.391 & 55.652 & 53.174 & 51.696 \\
151   & 51.435 & 56.652 & 54     & 55.435 & 53.565 & 52.957 & 56.087 & 55.783 & 53.304 & 52     \\
152   & 51.696 & 57.217 & 54.522 & 55.609 & 53.304 & 53.087 & 55.826 & 56.087 & 53.348 & 53.652 \\
153   & 52.304 & 57.913 & 54.435 & 55.478 & 53.826 & 53     & 55.957 & 56.304 & 53.478 & 53.957 \\
154   & 54.304 & 57.826 & 54.739 & 55.435 & 53.957 & 52.957 & 56.261 & 56.391 & 54.913 & 54.696 \\
155   & 54.391 & 57.739 & 54.957 & 55.87  & 54.261 & 53.261 & 56.391 & 56.348 & 54.609 & 54.261 \\
156   & 55.348 & 57.696 & 55.043 & 56.783 & 54.522 & 53.739 & 56.13  & 57     & 54.913 & 54.391 \\
157   & 55.435 & 58.261 & 54.478 & 56.913 & 54.913 & 53.957 & 56.391 & 57.391 & 55.087 & 54.565 \\
158   & 55.478 & 58.391 & 54.87  & 57.043 & 55.87  & 53.913 & 56.652 & 58.174 & 55.522 & 54.87  \\
159   & 55.609 & 58.652 & 55.391 & 57.522 & 55.913 & 53.826 & 56.609 & 58.391 & 55.783 & 55.522 \\
160   & 55.522 & 56.826 & 56.217 & 58.087 & 57.087 & 54     & 56.652 & 58.739 & 55     & 56.087 \\
161   & 55.957 & 57.043 & 56.217 & 58.522 & 56.913 & 54.957 & 57.043 & 58.957 & 55.739 & 55.957 \\
162   & 55.87  & 58.913 & 56.348 & 58.174 & 57.13  & 55.391 & 57.13  & 59.696 & 55.783 & 56.783 \\
163   & 55.87  & 58.826 & 56.913 & 57.913 & 57.348 & 55.478 & 57.435 & 59.87  & 56.304 & 56.87  \\
164   & 56.217 & 58.826 & 56.783 & 58.13  & 57.174 & 55.652 & 57.087 & 60.174 & 55.87  & 56.826 \\
165   & 56.217 & 59.043 & 56.783 & 58.304 & 57.609 & 56.043 & 57.522 & 60.304 & 55.913 & 58.304 \\
166   & 56.478 & 59.13  & 56.783 & 58.87  & 58.13  & 57.043 & 58     & 60.565 & 55.957 & 58.522 \\
167   & 57     & 59.261 & 57.348 & 59.13  & 58.261 & 57.261 & 57.826 & 60.217 & 56.478 & 58.609 \\
168   & 57.391 & 59.565 & 57.217 & 59.087 & 58.609 & 57.696 & 57.87  & 60.435 & 56.522 & 58.609 \\
169   & 57.261 & 59.348 & 57.522 & 59.435 & 58.826 & 57.957 & 58.217 & 60.609 & 56.522 & 59.087 \\
170   & 57.174 & 59.609 & 57.522 & 59.522 & 58.913 & 58.087 & 58.217 & 61.087 & 56.913 & 59.348 \\
171   & 57.435 & 59.652 & 57.826 & 59.478 & 58.522 & 58.478 & 58     & 61.348 & 57.174 & 59.217 \\
172   & 57.957 & 59.609 & 57.87  & 59.783 & 58.565 & 58.478 & 58.391 & 61.435 & 57.478 & 59.261 \\
173   & 58.217 & 59.565 & 57.652 & 59.565 & 58.739 & 58.435 & 58.565 & 61.261 & 57.522 & 59.522 \\
174   & 58.739 & 59.348 & 58.043 & 59.957 & 58.652 & 58.783 & 58.391 & 61.522 & 57.826 & 59.435 \\
175   & 58.261 & 60.13  & 58.13  & 60.13  & 58.739 & 59     & 59.087 & 62.087 & 57.913 & 59.435 \\
176   & 58.304 & 60.217 & 57.348 & 60.609 & 58.826 & 58.957 & 59.087 & 62     & 58.261 & 59.087 \\
177   & 58.783 & 60.043 & 57.783 & 60.739 & 59.261 & 58.913 & 59.696 & 62.043 & 58.348 & 59.174 \\
178   & 58.826 & 59.696 & 58.304 & 60.913 & 58.783 & 59.217 & 59.652 & 62.304 & 58.478 & 59.609 \\
179   & 58.739 & 60     & 58.783 & 61.174 & 58.913 & 59.435 & 60.261 & 62.13  & 59.565 & 58.913 \\
180   & 59.261 & 60.217 & 59.087 & 60.696 & 58.652 & 60.13  & 60.261 & 62.435 & 60     & 58.826 \\
181   & 59.043 & 60.043 & 59.652 & 60.522 & 59.087 & 60.696 & 60.696 & 62.478 & 60.435 & 58.87  \\
182   & 59.217 & 60.348 & 59.826 & 60.565 & 59.087 & 59.913 & 60.478 & 62.609 & 60     & 58.783 \\
183   & 59.087 & 60.304 & 60.087 & 60.826 & 59.217 & 60.174 & 60.043 & 62.565 & 60     & 59.043 \\
184   & 59.043 & 60.696 & 60.435 & 60.609 & 59.391 & 60.13  & 60.13  & 62.435 & 60.261 & 59.043 \\
185   & 59.391 & 60.696 & 60.435 & 60.783 & 59.217 & 60.174 & 59.826 & 62.783 & 59.783 & 58.304 \\
186   & 59.435 & 60.696 & 60.478 & 61.087 & 58.957 & 60.652 & 59.783 & 62.609 & 59.913 & 59.217 \\
187   & 59.348 & 60.826 & 60.522 & 61.304 & 58.739 & 60.348 & 59.609 & 62.609 & 60.087 & 59.261 \\
188   & 59.391 & 60.478 & 60.435 & 61.304 & 58.783 & 60.913 & 60.217 & 62.913 & 60.304 & 59.087 \\
189   & 59.522 & 60.304 & 60.739 & 61.609 & 59.348 & 61     & 60.391 & 62.826 & 60     & 58.609 \\
190   & 59.565 & 60.435 & 60.957 & 61.478 & 59.522 & 61.304 & 60.13  & 63.435 & 60.478 & 58.87  \\
191   & 59.522 & 60.522 & 61.348 & 61.783 & 59.261 & 61.609 & 59.957 & 63.261 & 60.957 & 58.87  \\
192   & 59.696 & 59.913 & 61.696 & 62.043 & 58.957 & 61.696 & 59.913 & 63.217 & 60.739 & 59     \\
193   & 59.696 & 60.261 & 61.522 & 61.826 & 58.696 & 61.304 & 59.522 & 63.348 & 61.043 & 58.957 \\
194   & 59.565 & 60.609 & 61.478 & 62     & 58.609 & 61.043 & 59.565 & 63.13  & 61.261 & 59.174 \\
195   & 59.739 & 60.522 & 61.696 & 61.478 & 58.304 & 60.913 & 59.609 & 63.261 & 61.043 & 59     \\
196   & 59.783 & 60.261 & 61.652 & 61.522 & 58.304 & 60.609 & 59.783 & 63.261 & 61.435 & 59.174 \\
\bottomrule\end{longtable}
\normalsize
