# Supplementary material for: Rehearsal-Free Continual Learning over Small Non-I.I.D. Batches
Source: arXiv:1907.03799 source file (2020-04-21)
Supplement: Supplementary file 2 [file 196_AR1_BN.tex]

\subsection{AR1* (with Batch Normalization), NICv2 - 196}
\fontsize{8}{11}\selectfont
\begin{longtable}[c]{rgrgrgrgrgr}
\hline
Batch & Run 0  & Run 1  & Run 2  & Run 3  & Run 4  & Run 5  & Run 6  & Run 7  & Run 8  & Run 9  \\ \hline
\endfirsthead
\endhead
0     & 8.127  & 8.127  & 8.127  & 8.127  & 8.127  & 8.127  & 8.127  & 8.127  & 8.127  & 8.127  \\
1     & 14.033 & 14.033 & 14.033 & 14.031 & 14.033 & 14.031 & 14.029 & 14.033 & 14.033 & 14.029 \\
2     & 14.091 & 13.984 & 14.8   & 13.956 & 14.291 & 14.504 & 14.596 & 13.389 & 15.416 & 14.48  \\
3     & 14.562 & 14.047 & 15.324 & 13.847 & 14.153 & 14.733 & 15.691 & 13.313 & 16.693 & 14.38  \\
4     & 14.3   & 13.576 & 15.687 & 14.353 & 14.191 & 13.142 & 15.871 & 13.522 & 17.922 & 14.8   \\
5     & 14.911 & 13.647 & 15.842 & 14.92  & 14.638 & 12.958 & 16.127 & 13.624 & 17.658 & 16.433 \\
6     & 15.113 & 14.269 & 16.969 & 15.467 & 14.742 & 13.68  & 15.616 & 13.271 & 17.393 & 17.927 \\
7     & 15.096 & 14.34  & 17.853 & 15.951 & 15.689 & 13.862 & 15.931 & 13.642 & 17.804 & 17.029 \\
8     & 15.209 & 14.289 & 18     & 17.104 & 15.38  & 15.38  & 16.851 & 13.287 & 17.598 & 17.222 \\
9     & 15.547 & 14.527 & 16.553 & 16.404 & 15.451 & 15.493 & 17.851 & 13.691 & 17.216 & 17.227 \\
10    & 15.92  & 16.471 & 16.591 & 17.016 & 15.531 & 15.991 & 18.371 & 13.791 & 17.313 & 17.487 \\
11    & 16.589 & 16.853 & 16.578 & 17.133 & 15.247 & 15.88  & 17.567 & 14.313 & 17.524 & 17.633 \\
12    & 17.502 & 16.578 & 16.504 & 18.013 & 15.916 & 15.82  & 18.08  & 15.207 & 18.507 & 17.98  \\
13    & 17.516 & 17.056 & 16.86  & 18.122 & 15.764 & 15.631 & 18.191 & 15.138 & 18.842 & 17.967 \\
14    & 16.791 & 17.304 & 18.067 & 18.418 & 15.876 & 16.142 & 18.331 & 16.638 & 19.404 & 18.096 \\
15    & 17.073 & 17.942 & 18.078 & 19.238 & 16.293 & 17.973 & 18.391 & 16.696 & 19.109 & 18.211 \\
16    & 17.109 & 18.282 & 18.353 & 18.293 & 16.167 & 18.524 & 19.153 & 17.896 & 19.102 & 18.816 \\
17    & 17.131 & 18.349 & 18.998 & 19.324 & 17.227 & 18.344 & 19.824 & 18.024 & 19.429 & 19.422 \\
18    & 17.587 & 18.682 & 18.998 & 19.602 & 18.24  & 18.716 & 19.556 & 18.427 & 19.096 & 19.849 \\
19    & 18.553 & 18.991 & 18.864 & 19.5   & 17.998 & 19.88  & 19.831 & 18.702 & 18.896 & 19.924 \\
20    & 18.6   & 20.289 & 19.02  & 20.153 & 18.078 & 19.813 & 20.098 & 18.673 & 19.498 & 20.802 \\
21    & 19.176 & 20.167 & 19.082 & 20.956 & 18.18  & 19.736 & 20.169 & 18.576 & 20.351 & 21.484 \\
22    & 20.024 & 20.824 & 18.944 & 21.242 & 19.047 & 20.344 & 20.509 & 18.413 & 20.591 & 21.818 \\
23    & 20.4   & 20.7   & 19.411 & 21.271 & 19.973 & 20.213 & 21.082 & 18.382 & 20.329 & 21.96  \\
24    & 20.353 & 20.858 & 18.749 & 21.449 & 20.62  & 20.253 & 20.642 & 17.976 & 20.431 & 22.702 \\
25    & 20.558 & 20.749 & 19.289 & 21.631 & 21.069 & 20.491 & 20.807 & 18.169 & 20.909 & 23.078 \\
26    & 20.818 & 20.076 & 19.449 & 21.644 & 20.749 & 20.449 & 21.749 & 18.013 & 20.913 & 23.022 \\
27    & 21.338 & 20.298 & 20.373 & 22.522 & 21     & 20.331 & 21.82  & 19.127 & 21.318 & 23.109 \\
28    & 21.249 & 19.762 & 20.704 & 22.96  & 20.924 & 20.553 & 22.036 & 19.653 & 21.722 & 23.204 \\
29    & 21.536 & 19.389 & 21.287 & 23.413 & 21.171 & 20.678 & 21.909 & 19.849 & 22.7   & 24.6   \\
30    & 22.138 & 19.638 & 21.809 & 23.562 & 22.196 & 20.72  & 22.238 & 20.34  & 23.464 & 24.631 \\
31    & 22.211 & 19.858 & 21.558 & 23.698 & 22.507 & 20.542 & 22.293 & 20.993 & 23.373 & 24.88  \\
32    & 22.269 & 20.002 & 21.651 & 23.644 & 22.764 & 20.52  & 21.751 & 20.933 & 23.431 & 25.142 \\
33    & 22.653 & 19.973 & 22.2   & 23.504 & 22.989 & 20.036 & 23.02  & 20.729 & 23.424 & 25.162 \\
34    & 23.422 & 19.842 & 21.116 & 23.433 & 23.58  & 20.562 & 23.322 & 21.04  & 23.2   & 25.976 \\
35    & 23.229 & 19.98  & 22.051 & 23.364 & 24.271 & 20.607 & 23.309 & 20.984 & 23.731 & 25.478 \\
36    & 23.776 & 21.06  & 21.96  & 23.704 & 24.22  & 20.716 & 23.204 & 20.958 & 24.058 & 25.82  \\
37    & 24.184 & 21.487 & 22.342 & 24.009 & 24.253 & 20.258 & 23.164 & 21.153 & 23.86  & 27.053 \\
38    & 24.164 & 21.538 & 22.613 & 24.138 & 23.993 & 20.198 & 23.216 & 21.849 & 24.502 & 26.324 \\
39    & 23.942 & 21.618 & 22.393 & 24.036 & 23.84  & 19.989 & 23.276 & 22.167 & 24.593 & 26.531 \\
40    & 23.86  & 21.631 & 22.629 & 24.271 & 24.096 & 20.124 & 24     & 22.464 & 24.796 & 28.14  \\
41    & 24.187 & 22.362 & 22.709 & 24.522 & 24.378 & 20.18  & 24.807 & 22.476 & 24.787 & 28.071 \\
42    & 24.367 & 22.947 & 22.889 & 24.767 & 24.698 & 20.209 & 25.16  & 22.529 & 24.322 & 28.464 \\
43    & 24.756 & 24.233 & 23.816 & 24.789 & 25.069 & 20.996 & 25.216 & 22.58  & 24.269 & 29.136 \\
44    & 25.416 & 24.178 & 24.2   & 24.776 & 26.591 & 21.067 & 25.798 & 23.498 & 24.56  & 29.46  \\
45    & 25.313 & 25.564 & 24.084 & 25.929 & 27.278 & 21.284 & 26.193 & 23.596 & 24.611 & 29.809 \\
46    & 25.831 & 25.556 & 23.973 & 25.782 & 27.749 & 21.311 & 26.484 & 24.062 & 24.893 & 30.396 \\
47    & 25.869 & 25.762 & 24.358 & 26.4   & 28.064 & 21.829 & 27.22  & 23.984 & 25.053 & 30.709 \\
48    & 25.924 & 25.947 & 24.851 & 26.793 & 28.127 & 21.853 & 27.618 & 24.207 & 24.716 & 30.736 \\
49    & 25.802 & 26.342 & 24.767 & 27.449 & 28.387 & 22.922 & 28.149 & 24.673 & 24.231 & 30.951 \\
50    & 26.46  & 26.4   & 24.929 & 27.536 & 29.258 & 23.42  & 28.473 & 24.882 & 24.931 & 30.904 \\
51    & 26.489 & 26.607 & 25.898 & 27.564 & 28.791 & 23.496 & 28.482 & 25.451 & 25.362 & 31.033 \\
52    & 26.569 & 26.729 & 25.911 & 27.549 & 28.536 & 23.427 & 29.922 & 25.629 & 25.896 & 30.682 \\
53    & 26.713 & 26.953 & 26.033 & 27.656 & 28.862 & 23.693 & 29.907 & 26.169 & 25.747 & 31.011 \\
54    & 27.6   & 27.316 & 26.153 & 29.244 & 28.776 & 24.816 & 30.271 & 25.991 & 26.364 & 30.827 \\
55    & 27.804 & 27.344 & 26.402 & 29.518 & 29.064 & 25.233 & 30.298 & 26.518 & 27.824 & 30.084 \\
56    & 28.329 & 27.716 & 26.138 & 29.927 & 29.362 & 24.04  & 30.989 & 26.427 & 28.1   & 31.033 \\
57    & 28.242 & 28.8   & 26.849 & 29.8   & 29.691 & 24.716 & 31.92  & 26.409 & 28.44  & 31.169 \\
58    & 28.262 & 28.507 & 26.638 & 30.551 & 29.84  & 25.16  & 31.958 & 26.307 & 28.467 & 31.08  \\
59    & 28.567 & 29.298 & 26.687 & 30.464 & 29.476 & 25.273 & 31.849 & 26.987 & 28.456 & 31.627 \\
60    & 28.596 & 29.86  & 26.613 & 31.176 & 30.418 & 25.478 & 31.86  & 27.256 & 28.887 & 31.789 \\
61    & 28.569 & 29.949 & 26.633 & 31.853 & 30.622 & 25.684 & 31.976 & 27.067 & 29.404 & 31.756 \\
62    & 29.151 & 30.307 & 26.636 & 32.116 & 30.931 & 25.876 & 32.767 & 27.087 & 29.958 & 31.818 \\
63    & 29.716 & 30.371 & 27.553 & 32.547 & 31.509 & 26.076 & 32.74  & 27.107 & 30.547 & 32.271 \\
64    & 29.478 & 30.404 & 28.556 & 32.462 & 31.513 & 26.32  & 33.36  & 27.118 & 30.453 & 32.538 \\
65    & 29.358 & 30.291 & 28.371 & 32.847 & 31.447 & 26.022 & 33.362 & 27.051 & 30.804 & 32.671 \\
66    & 29.484 & 30.88  & 28.887 & 33.149 & 31.409 & 27.871 & 33.711 & 27.184 & 30.827 & 32.909 \\
67    & 29.733 & 31.142 & 29.071 & 33.256 & 32.249 & 28.36  & 33.622 & 27.218 & 30.931 & 33.107 \\
68    & 30.142 & 31.273 & 31.113 & 33.487 & 32.287 & 28.509 & 34.004 & 27.391 & 31.182 & 33.209 \\
69    & 30.287 & 31.236 & 31.62  & 33.707 & 32.278 & 28.829 & 34.036 & 27.373 & 31.287 & 33.331 \\
70    & 30.367 & 31.298 & 31.449 & 33.669 & 32.553 & 29.209 & 33.936 & 27.907 & 31.169 & 33.813 \\
71    & 30.093 & 31.224 & 30.947 & 33.791 & 32.758 & 29.096 & 34.044 & 27.871 & 31.629 & 33.882 \\
72    & 30.316 & 31.244 & 31.231 & 34.031 & 32.758 & 29.02  & 34.162 & 28.384 & 32.382 & 34.264 \\
73    & 30.271 & 31.26  & 31.251 & 35.424 & 32.318 & 29.449 & 34.236 & 28.307 & 32.516 & 34.216 \\
74    & 30.42  & 31.713 & 30.884 & 36.053 & 31.96  & 29.44  & 34.364 & 28.244 & 32.382 & 34.002 \\
75    & 31.038 & 31.882 & 31.302 & 35.844 & 32.182 & 29.711 & 34.378 & 28.136 & 32.073 & 33.942 \\
76    & 31.189 & 32.002 & 31.624 & 35.873 & 32.14  & 29.871 & 34.469 & 28.242 & 31.998 & 34.124 \\
77    & 31.298 & 32.164 & 31.491 & 35.784 & 31.811 & 30.251 & 34.616 & 28.356 & 32.611 & 34.111 \\
78    & 31.422 & 33.084 & 31.211 & 35.809 & 32.018 & 31.122 & 34.802 & 28.251 & 33.422 & 34.52  \\
79    & 31.68  & 33.28  & 31.036 & 35.851 & 32.069 & 31.58  & 34.967 & 28.58  & 33.884 & 35.124 \\
80    & 31.798 & 33.722 & 31.158 & 36.076 & 32.138 & 31.684 & 35.318 & 28.847 & 34.144 & 35.324 \\
81    & 31.798 & 32.678 & 32.253 & 36.08  & 32.431 & 31.673 & 36.249 & 28.869 & 34.107 & 35.447 \\
82    & 31.989 & 32.593 & 32.7   & 36.342 & 32.562 & 32.513 & 36.542 & 28.987 & 34.371 & 36.48  \\
83    & 31.851 & 33.182 & 32.664 & 36.758 & 32.509 & 33.216 & 36.358 & 28.947 & 34.364 & 36.611 \\
84    & 31.949 & 33.418 & 32.66  & 37.211 & 33.109 & 33.436 & 37.376 & 28.944 & 34.78  & 37.231 \\
85    & 32.411 & 33.96  & 32.373 & 37.833 & 32.887 & 34.931 & 37.449 & 29.013 & 35.309 & 37.567 \\
86    & 32.156 & 34.031 & 32.447 & 37.973 & 32.924 & 34.88  & 37.747 & 29.269 & 35.338 & 37.156 \\
87    & 32.5   & 34.462 & 32.522 & 36.909 & 33.029 & 35.098 & 38.404 & 29.716 & 34.982 & 37.06  \\
88    & 32.844 & 34.891 & 32.713 & 37.056 & 33.369 & 35.216 & 38.467 & 29.742 & 35.273 & 36.951 \\
89    & 32.738 & 34.907 & 32.962 & 37.258 & 33.182 & 35.24  & 38.793 & 30.042 & 34.996 & 37.124 \\
90    & 32.876 & 35.018 & 32.756 & 38.687 & 32.656 & 35.791 & 38.849 & 30.522 & 35.678 & 37.32  \\
91    & 32.767 & 35.34  & 32.551 & 39.069 & 33.122 & 35.66  & 39.498 & 30.389 & 35.74  & 37.36  \\
92    & 32.611 & 35.527 & 32.696 & 39.704 & 33.591 & 36.002 & 39.489 & 30.507 & 35.651 & 37.278 \\
93    & 32.6   & 36.007 & 32.296 & 39.727 & 34.109 & 36.124 & 39.44  & 30.976 & 35.578 & 37.338 \\
94    & 32.769 & 35.967 & 31.8   & 39.907 & 34.06  & 36.316 & 39.636 & 31.184 & 35.9   & 37.707 \\
95    & 33.096 & 36.373 & 31.009 & 39.78  & 33.993 & 36.302 & 39.858 & 31.071 & 36.029 & 37.727 \\
96    & 33.86  & 36.773 & 30.9   & 39.233 & 33.851 & 36.202 & 39.762 & 31.073 & 35.867 & 37.998 \\
97    & 34.142 & 36.564 & 31.151 & 39.209 & 33.673 & 36.333 & 39.793 & 31.024 & 36.229 & 38.06  \\
98    & 34.162 & 36.807 & 31.349 & 39.271 & 34.467 & 36.32  & 40.436 & 31.033 & 35.862 & 37.984 \\
99    & 34.907 & 36.387 & 31.707 & 39.609 & 34.627 & 36.364 & 40.664 & 30.978 & 36.707 & 38.396 \\
100   & 34.724 & 36.88  & 31.818 & 39.438 & 34.696 & 37.127 & 40.798 & 30.991 & 36.86  & 38.569 \\
101   & 34.691 & 37.86  & 31.847 & 39.571 & 35.04  & 37.376 & 40.876 & 30.984 & 37.358 & 38.92  \\
102   & 34.676 & 38.127 & 32.72  & 39.584 & 35.498 & 37.631 & 41.187 & 30.951 & 38.18  & 38.909 \\
103   & 34.98  & 37.633 & 32.996 & 39.824 & 35.307 & 37.687 & 42.26  & 31.024 & 38.942 & 39.507 \\
104   & 35.02  & 37.727 & 33.689 & 39.904 & 35.284 & 38.26  & 42.22  & 31.107 & 39.189 & 39.893 \\
105   & 35.331 & 39.038 & 34.46  & 39.918 & 35.258 & 38.549 & 41.711 & 32.173 & 38.6   & 40.713 \\
106   & 35.382 & 38.913 & 34.82  & 40.271 & 35.049 & 38.522 & 41.718 & 32.24  & 39.178 & 40.938 \\
107   & 35.276 & 39.736 & 35.06  & 40.464 & 35.389 & 38.447 & 43.396 & 32.147 & 39.376 & 41.049 \\
108   & 36.233 & 40.12  & 33.896 & 40.391 & 35.389 & 38.509 & 43.418 & 32.6   & 39.873 & 41.236 \\
109   & 36.282 & 40.311 & 33.798 & 40.331 & 35.589 & 38.667 & 43.518 & 33.36  & 40.309 & 41.236 \\
110   & 35.989 & 40.471 & 34.073 & 40.54  & 35.542 & 38.618 & 43.464 & 34.249 & 40.649 & 41.182 \\
111   & 36.218 & 39.976 & 33.618 & 40.676 & 35.749 & 38.5   & 43.491 & 34.54  & 40.942 & 41.74  \\
112   & 36.062 & 40.464 & 33.491 & 40.467 & 35.778 & 38.458 & 43.571 & 35.078 & 40.462 & 41.813 \\
113   & 36.138 & 40.553 & 33.864 & 40.282 & 35.971 & 38.807 & 44.496 & 34.92  & 40.427 & 41.927 \\
114   & 36.164 & 40.789 & 34.009 & 40.387 & 36.184 & 38.993 & 44.947 & 35.353 & 40.991 & 41.929 \\
115   & 36.416 & 41.018 & 33.567 & 40.858 & 36.362 & 39.276 & 45.013 & 35.473 & 41.462 & 42.007 \\
116   & 36.633 & 41.64  & 34.484 & 41.369 & 36.256 & 39.109 & 45.067 & 35.696 & 40.707 & 42.436 \\
117   & 36.798 & 42.296 & 35.14  & 42.796 & 36.213 & 39.118 & 45.182 & 35.798 & 40.773 & 42.949 \\
118   & 36.891 & 42.458 & 35.167 & 43.344 & 36.273 & 39.996 & 45.302 & 36.056 & 41.193 & 43.187 \\
119   & 37.104 & 42.553 & 36.178 & 43.562 & 36.333 & 40.767 & 45.313 & 36.018 & 41.607 & 43.376 \\
120   & 36.962 & 43.771 & 35.953 & 43.358 & 36.218 & 40.682 & 45.136 & 36.473 & 41.74  & 43.402 \\
121   & 37.047 & 43.949 & 36.089 & 42.833 & 36.351 & 40.776 & 45.1   & 36.356 & 43.251 & 43.064 \\
122   & 37.253 & 43.887 & 36.222 & 42.96  & 36.242 & 41.016 & 45.382 & 36.749 & 43.642 & 43.038 \\
123   & 37.378 & 44.047 & 36.133 & 43.298 & 36.293 & 41.618 & 45.3   & 36.778 & 43.064 & 43.218 \\
124   & 37.458 & 44.122 & 35.973 & 43.549 & 36.16  & 42.34  & 45.207 & 37.351 & 42.762 & 43.051 \\
125   & 37.516 & 44.167 & 36.267 & 43.736 & 36.407 & 42.498 & 45.536 & 37.867 & 42.842 & 43.531 \\
126   & 37.402 & 44.3   & 36.409 & 44.162 & 36.456 & 41.918 & 45.893 & 39.196 & 42.767 & 43.158 \\
127   & 37.756 & 44.433 & 36.74  & 44.356 & 36.749 & 41.984 & 45.978 & 38.836 & 43.278 & 43.24  \\
128   & 38.111 & 44.733 & 36.78  & 44.313 & 37.72  & 42.247 & 45.162 & 38.687 & 44.289 & 43.131 \\
129   & 38.171 & 44.469 & 37.229 & 44.3   & 37.669 & 42.578 & 44.762 & 39.349 & 44.271 & 43.196 \\
130   & 38.258 & 44.564 & 37.058 & 44.549 & 38.309 & 43.564 & 45.116 & 39.269 & 45.531 & 44.004 \\
131   & 38.18  & 44.753 & 37.031 & 44.744 & 38.547 & 43.86  & 45.156 & 39.213 & 45.529 & 44.402 \\
132   & 38.358 & 44.722 & 36.284 & 44.764 & 38.638 & 44.129 & 45.013 & 39.242 & 45.022 & 44.52  \\
133   & 38.416 & 45.267 & 36.389 & 44.742 & 38.727 & 44.064 & 45.909 & 39.34  & 44.729 & 44.742 \\
134   & 38.362 & 45.34  & 36.538 & 44.687 & 38.631 & 44.076 & 45.784 & 39.318 & 44.831 & 44.764 \\
135   & 38.387 & 45.52  & 37.707 & 44.869 & 38.947 & 44.227 & 46.242 & 39.387 & 44.449 & 44.669 \\
136   & 39.516 & 45.849 & 37.756 & 44.993 & 38.831 & 44.398 & 46.567 & 39.413 & 44.147 & 44.947 \\
137   & 39.491 & 46.576 & 37.989 & 45.447 & 38.778 & 44.907 & 46.609 & 39.629 & 44.436 & 45.349 \\
138   & 39.449 & 46.729 & 38.724 & 45.338 & 39.52  & 44.909 & 46.822 & 39.824 & 43.891 & 45.876 \\
139   & 39.664 & 46.687 & 38.758 & 45.562 & 39.384 & 45.18  & 46.991 & 40.293 & 44.029 & 46.682 \\
140   & 39.829 & 46.56  & 39.296 & 45.407 & 40.031 & 45.698 & 47.153 & 40.382 & 44.007 & 46.884 \\
141   & 40.236 & 46.947 & 39.636 & 45.656 & 40.224 & 45.782 & 47.487 & 40.382 & 44.787 & 47.029 \\
142   & 40.484 & 46.947 & 40.071 & 45.853 & 41.253 & 45.944 & 48.004 & 39.953 & 44.893 & 46.824 \\
143   & 40.473 & 46.896 & 40.127 & 46.52  & 41.211 & 45.678 & 48.036 & 40.302 & 44.811 & 45.878 \\
144   & 40.498 & 46.942 & 41.331 & 46.976 & 41.824 & 45.553 & 48.331 & 40.293 & 44.376 & 45.893 \\
145   & 40.364 & 46.909 & 41.391 & 46.464 & 42.273 & 45.744 & 48.931 & 39.816 & 43.998 & 46.129 \\
146   & 40.947 & 47.016 & 41.347 & 46.98  & 42.14  & 45.827 & 49.342 & 40.138 & 44.293 & 46.482 \\
147   & 40.902 & 47.127 & 41.249 & 47.356 & 40.729 & 45.693 & 49.54  & 40.116 & 43.842 & 46.602 \\
148   & 40.949 & 47.038 & 41.64  & 47.876 & 41.044 & 46.038 & 49.416 & 40.313 & 43.931 & 46.711 \\
149   & 41.278 & 47.089 & 41.782 & 47.964 & 41.511 & 46.242 & 49.853 & 40.322 & 43.996 & 46.9   \\
150   & 42.556 & 46.978 & 42.129 & 48.26  & 41.816 & 45.953 & 49.778 & 40.564 & 44.627 & 46.891 \\
151   & 42.462 & 47.671 & 42.229 & 48.162 & 42.367 & 46.013 & 49.707 & 40.878 & 44.989 & 46.511 \\
152   & 42.676 & 47.693 & 42.46  & 48.462 & 42.556 & 45.913 & 49.682 & 41.076 & 45.027 & 47.331 \\
153   & 42.4   & 47.809 & 42.396 & 48.378 & 42.571 & 45.962 & 50.504 & 41.536 & 45.198 & 47.673 \\
154   & 44.338 & 46.753 & 42.218 & 48.498 & 42.996 & 46.216 & 51.247 & 41.593 & 45.931 & 47.436 \\
155   & 44.438 & 47.107 & 42.051 & 48.842 & 44.869 & 46.004 & 51.533 & 42.202 & 46.544 & 47.684 \\
156   & 44.773 & 47.184 & 42.411 & 49.276 & 44.669 & 46.216 & 51.282 & 42.52  & 46.524 & 47.78  \\
157   & 45.196 & 47.498 & 42.556 & 49.411 & 44.696 & 45.911 & 52.136 & 42.984 & 46.107 & 48.211 \\
158   & 46.127 & 46.433 & 42.902 & 49.407 & 44.658 & 46.107 & 52.087 & 43.182 & 46.091 & 48.329 \\
159   & 46.418 & 46.913 & 43.051 & 49.151 & 44.729 & 46.629 & 52.22  & 43.504 & 46.056 & 49.353 \\
160   & 46.511 & 46.802 & 43.629 & 49.06  & 44.802 & 46.484 & 52.336 & 43.611 & 45.791 & 49.429 \\
161   & 46.456 & 46.827 & 44.313 & 48.86  & 44.829 & 47.269 & 52.438 & 43.909 & 46.569 & 49.587 \\
162   & 46.738 & 47.247 & 44.802 & 48.38  & 44.493 & 47.544 & 52.649 & 43.878 & 46.556 & 49.927 \\
163   & 46.887 & 47.593 & 45.282 & 48.649 & 44.593 & 47.587 & 52.9   & 44.036 & 47.042 & 49.84  \\
164   & 47.149 & 47.911 & 45.524 & 48.693 & 44.956 & 47.956 & 52.369 & 44.329 & 47.7   & 49.88  \\
165   & 47.258 & 47.967 & 45.258 & 48.5   & 45.547 & 47.949 & 52.982 & 44.831 & 47.982 & 50.853 \\
166   & 46.927 & 48.364 & 44.984 & 49.378 & 45.789 & 48.333 & 52.638 & 45.464 & 47.409 & 50.949 \\
167   & 47.444 & 48.82  & 45.22  & 49.691 & 46.209 & 48.442 & 52.496 & 45.176 & 47.431 & 51.307 \\
168   & 47.584 & 49.147 & 45.284 & 49.54  & 46.26  & 48.711 & 52.211 & 45.596 & 47.384 & 51.413 \\
169   & 47.684 & 49.08  & 45.882 & 49.784 & 46.313 & 48.593 & 52.678 & 46.133 & 47.451 & 51.516 \\
170   & 48.024 & 49.176 & 45.48  & 50.211 & 46.149 & 48.627 & 52.576 & 46.551 & 47.853 & 51.816 \\
171   & 47.967 & 48.873 & 45.573 & 50.413 & 45.909 & 49.216 & 51.967 & 46.584 & 48.022 & 51.982 \\
172   & 47.944 & 48.691 & 45.602 & 50.224 & 46.331 & 49.127 & 51.78  & 46.778 & 48.418 & 52.196 \\
173   & 47.611 & 48.827 & 45.02  & 50.349 & 46.578 & 49.373 & 51.198 & 46.798 & 48.698 & 52.72  \\
174   & 47.513 & 48.9   & 45.493 & 50.287 & 46.453 & 49.487 & 51.502 & 46.536 & 49.084 & 53.142 \\
175   & 47.409 & 49.364 & 45.458 & 50.382 & 46.593 & 49.993 & 51.478 & 46.476 & 48.982 & 52.093 \\
176   & 47.336 & 49.433 & 44.878 & 50.607 & 46.378 & 49.824 & 51.24  & 46.582 & 49.307 & 52.253 \\
177   & 47.409 & 49.567 & 45.609 & 50.509 & 45.909 & 49.947 & 50.958 & 46.511 & 49.304 & 52.111 \\
178   & 47.276 & 49.407 & 46.002 & 50.411 & 45.98  & 50.156 & 51.011 & 47.193 & 49.364 & 51.724 \\
179   & 46.862 & 49.771 & 45.991 & 50.402 & 45.722 & 49.733 & 51.056 & 47.2   & 49.489 & 51.733 \\
180   & 46.88  & 49.276 & 46.591 & 50.413 & 45.796 & 49.822 & 51     & 46.802 & 49.96  & 51.544 \\
181   & 46.887 & 49.189 & 46.958 & 50.938 & 46.222 & 50.089 & 50.529 & 46.849 & 49.956 & 51.64  \\
182   & 46.46  & 48.842 & 47.173 & 51.1   & 46.364 & 50.133 & 49.858 & 46.751 & 49.629 & 51.789 \\
183   & 46.076 & 48.558 & 47.22  & 51.291 & 46.371 & 49.973 & 49.884 & 46.851 & 49.504 & 51.896 \\
184   & 46.044 & 48.86  & 47.176 & 51.316 & 45.86  & 50.673 & 50.031 & 47.184 & 49.738 & 51.651 \\
185   & 45.847 & 48.311 & 47.084 & 51.416 & 46.729 & 50.58  & 49.896 & 47.662 & 49.776 & 51.118 \\
186   & 46.036 & 48.54  & 47.304 & 51.773 & 47.007 & 50.862 & 49.98  & 48.176 & 49.827 & 51.569 \\
187   & 45.824 & 48.744 & 47.776 & 52.313 & 47.058 & 51.047 & 49.871 & 48.093 & 49.876 & 52.036 \\
188   & 46.467 & 48.669 & 47.487 & 52.453 & 47.144 & 51.331 & 49.958 & 48.289 & 50.018 & 51.622 \\
189   & 46.451 & 48.369 & 47.138 & 52.527 & 47.564 & 51.631 & 49.9   & 48.489 & 49.691 & 51.089 \\
190   & 46.302 & 48.687 & 47.382 & 52.798 & 48.051 & 51.909 & 49.869 & 48.716 & 49.196 & 51.016 \\
191   & 46.34  & 48.309 & 47.711 & 53.024 & 47.829 & 51.162 & 49.304 & 49.053 & 48.993 & 50.813 \\
192   & 46.338 & 47.14  & 47.94  & 53.258 & 47.731 & 51.48  & 49.304 & 49.116 & 48.882 & 51.118 \\
193   & 46.322 & 46.731 & 48.289 & 53.118 & 47.689 & 51.167 & 49.28  & 48.882 & 48.731 & 51.047 \\
194   & 46.338 & 47.038 & 48.202 & 52.947 & 47.62  & 51.611 & 49.316 & 48.751 & 48.636 & 51.491 \\
195   & 46.084 & 47.387 & 48.524 & 52.467 & 47.66  & 51.809 & 49.247 & 48.636 & 48.409 & 51.571 \\
196   & 46.356 & 47.636 & 48.789 & 52.333 & 47.518 & 52.024 & 49.28  & 48.447 & 48.118 & 51.84  \\
\bottomrule\end{longtable}
\normalsize
