# Supplementary material for: Rehearsal-Free Continual Learning over Small Non-I.I.D. Batches
Source: arXiv:1907.03799 source file (2020-04-21)
Supplement: Supplementary file 4 [file 196_EWC.tex]

\subsection{EWC, NICv2 - 196}
\fontsize{8}{11}\selectfont
\begin{longtable}[c]{rgrgrgrgrgr}
\hline
Batch & Run 0  & Run 1  & Run 2  & Run 3  & Run 4  & Run 5  & Run 6  & Run 7  & Run 8  & Run 9  \\ \hline
\endfirsthead
\endhead
0     & 1.522  & 1.522  & 1.522  & 1.522  & 1.522  & 1.522  & 1.522  & 1.522  & 1.522  & 1.522  \\
1     & 13.826 & 13.87  & 13.87  & 13.826 & 13.826 & 13.87  & 13.87  & 13.87  & 13.87  & 13.826 \\
2     & 14.174 & 14.261 & 13.696 & 14     & 13.87  & 13.826 & 14.13  & 13.739 & 14.217 & 13.826 \\
3     & 14.652 & 13.87  & 13.913 & 13.957 & 13.609 & 14.174 & 14.391 & 13.304 & 14.348 & 13.87  \\
4     & 14.696 & 14.043 & 14.13  & 14.174 & 14     & 14.217 & 14.391 & 13.087 & 14.478 & 14     \\
5     & 14.609 & 14     & 14.304 & 14.261 & 13.87  & 14.304 & 14.522 & 12.957 & 14.174 & 14.087 \\
6     & 14.609 & 14.043 & 14.783 & 14.478 & 13.696 & 14.87  & 14.304 & 13.174 & 14.217 & 14.261 \\
7     & 15.304 & 14.565 & 14.913 & 14.913 & 14.304 & 15     & 14.087 & 13.478 & 14.391 & 14.391 \\
8     & 15.304 & 14.435 & 14.783 & 14.957 & 14.826 & 15.13  & 14.261 & 13.304 & 14.13  & 14.478 \\
9     & 15.391 & 14.435 & 14.652 & 15.174 & 14.826 & 15.217 & 14.304 & 13.261 & 14.348 & 14.435 \\
10    & 15.565 & 14.652 & 14.565 & 15.304 & 14.87  & 15.739 & 14.522 & 13.522 & 14.435 & 14.478 \\
11    & 15.565 & 15.13  & 15.087 & 15.261 & 15     & 16.13  & 14.522 & 14.217 & 14.609 & 14.304 \\
12    & 15.739 & 15.435 & 15.435 & 15.565 & 14.826 & 16.261 & 14.652 & 14.609 & 14.652 & 14.739 \\
13    & 15.609 & 15.739 & 15.565 & 16     & 15.087 & 16.217 & 14.826 & 14.522 & 14.783 & 14.739 \\
14    & 15.435 & 15.783 & 15.696 & 15.826 & 15.043 & 16.217 & 14.783 & 14.478 & 15.043 & 14.609 \\
15    & 15.522 & 16     & 15.609 & 16.043 & 15.217 & 16.174 & 15.087 & 14.522 & 15.043 & 14.478 \\
16    & 15.522 & 16.217 & 15.478 & 16     & 15.174 & 15.826 & 15.13  & 14.435 & 15.13  & 14.304 \\
17    & 15.522 & 16.478 & 15.565 & 16.043 & 15.043 & 15.652 & 15.174 & 14.609 & 14.826 & 14.478 \\
18    & 15.913 & 16.522 & 15.783 & 15.957 & 14.826 & 15.652 & 15.13  & 14.739 & 14.826 & 14.696 \\
19    & 15.87  & 16.696 & 15.652 & 15.957 & 14.957 & 15.826 & 15     & 14.739 & 14.739 & 14.696 \\
20    & 15.652 & 16.739 & 15.391 & 15.522 & 14.87  & 15.87  & 14.783 & 14.783 & 14.609 & 15     \\
21    & 15.826 & 16.739 & 15.435 & 15.348 & 14.522 & 16.043 & 14.609 & 14.87  & 14.87  & 15.087 \\
22    & 15.696 & 16.609 & 15.13  & 15.478 & 14.348 & 16.13  & 14.913 & 15.087 & 14.826 & 15.348 \\
23    & 15.913 & 16.826 & 15.13  & 15.522 & 14.304 & 16.217 & 15.087 & 15.261 & 14.739 & 15.609 \\
24    & 15.957 & 16.913 & 15.478 & 15.565 & 14.522 & 16.13  & 15.13  & 15.783 & 14.609 & 15.652 \\
25    & 15.783 & 16.565 & 15.348 & 15.609 & 14.609 & 16.217 & 15.391 & 15.826 & 14.522 & 15.478 \\
26    & 15.913 & 16.739 & 15.217 & 15.696 & 14.652 & 16.217 & 15.391 & 15.783 & 14.435 & 15.435 \\
27    & 16.13  & 16.783 & 15.043 & 15.696 & 14.739 & 16.435 & 15.478 & 15.826 & 14.913 & 16     \\
28    & 15.87  & 16.522 & 14.826 & 15.652 & 14.87  & 16.565 & 15.522 & 15.739 & 14.957 & 16.348 \\
29    & 15.957 & 16.304 & 14.913 & 15.696 & 14.957 & 16.565 & 15.609 & 15.478 & 14.783 & 16.13  \\
30    & 16     & 16.696 & 15.174 & 15.522 & 15.13  & 16.391 & 15.609 & 15.739 & 14.609 & 16.217 \\
31    & 15.957 & 17.043 & 15.13  & 15.522 & 15.174 & 16.652 & 15.87  & 16     & 15     & 16.217 \\
32    & 15.957 & 17.087 & 15.391 & 15.87  & 15.174 & 16.783 & 15.826 & 16.913 & 15.261 & 16.087 \\
33    & 16.174 & 17.391 & 15.435 & 16.087 & 15.174 & 16.957 & 15.348 & 17.348 & 15.261 & 16.217 \\
34    & 15.826 & 17.174 & 15.13  & 16.043 & 15.13  & 16.696 & 15.391 & 17.609 & 15.13  & 16.348 \\
35    & 15.913 & 17.261 & 15.043 & 15.87  & 15.217 & 16.696 & 15.739 & 17.565 & 14.957 & 16.261 \\
36    & 15.87  & 17.13  & 15.304 & 15.652 & 15.174 & 16.696 & 15.783 & 17.391 & 15.043 & 16.261 \\
37    & 16.261 & 17.13  & 15.304 & 15.739 & 15.217 & 16.696 & 16.13  & 17.348 & 15.13  & 16.391 \\
38    & 16.609 & 17.043 & 15.261 & 15.609 & 14.957 & 16.696 & 16.348 & 17.565 & 14.913 & 16.261 \\
39    & 16.609 & 16.87  & 15.261 & 16     & 15.087 & 16.913 & 16.261 & 17.826 & 14.826 & 16.522 \\
40    & 16.696 & 17.13  & 15.261 & 16.13  & 15.13  & 16.87  & 16.391 & 18     & 14.696 & 16.652 \\
41    & 16.609 & 16.826 & 15.522 & 16     & 15.217 & 16.478 & 16.087 & 18.13  & 14.652 & 16.522 \\
42    & 16.696 & 16.913 & 15.87  & 16.304 & 15.304 & 16.217 & 16     & 18.261 & 14.609 & 16.565 \\
43    & 17     & 16.826 & 16.043 & 16.391 & 15.174 & 16.261 & 16.217 & 18.391 & 14.87  & 16.609 \\
44    & 17.261 & 16.957 & 16     & 16.304 & 15.304 & 16.609 & 16.348 & 18.913 & 15     & 16.957 \\
45    & 17.522 & 16.957 & 16.087 & 16.13  & 15.565 & 17.087 & 16.478 & 19.304 & 15.696 & 17.174 \\
46    & 17.696 & 17.087 & 16     & 15.435 & 15.696 & 17.13  & 16.348 & 19.261 & 15.652 & 17.391 \\
47    & 18.348 & 17.13  & 15.826 & 15.217 & 15.739 & 17.13  & 16.391 & 19.652 & 15.478 & 17.522 \\
48    & 18.435 & 17.087 & 15.739 & 15.304 & 15.957 & 17.174 & 16.652 & 19.913 & 15.826 & 17.478 \\
49    & 18.174 & 17.435 & 15.609 & 15.304 & 15.957 & 17.087 & 16.826 & 20.391 & 16.087 & 17.87  \\
50    & 18.391 & 17.522 & 15.565 & 15.391 & 16.13  & 16.957 & 17.304 & 20.87  & 16.087 & 17.783 \\
51    & 18.609 & 17.609 & 15.696 & 15.435 & 16.043 & 17.087 & 17.522 & 20.826 & 15.826 & 18     \\
52    & 18.435 & 17.913 & 15.87  & 15.957 & 16.217 & 17.435 & 17.348 & 20.696 & 15.696 & 18.435 \\
53    & 18.652 & 18.652 & 16     & 16.13  & 16.304 & 17.609 & 17.696 & 20.696 & 15.739 & 18.609 \\
54    & 19.087 & 18.826 & 15.957 & 16.13  & 16.304 & 17.739 & 18.13  & 20.609 & 16.087 & 18.783 \\
55    & 19.087 & 18.652 & 16.087 & 16.304 & 16.304 & 17.87  & 18.478 & 20.826 & 15.739 & 18.739 \\
56    & 19.13  & 18.565 & 16.13  & 16.87  & 16.304 & 18.087 & 18.435 & 21.13  & 15.739 & 18.609 \\
57    & 19.087 & 18.435 & 16.174 & 17.13  & 16.609 & 18.174 & 18.391 & 21.174 & 15.783 & 18.609 \\
58    & 18.87  & 18.391 & 16.348 & 17.043 & 16.783 & 18.174 & 18.13  & 21.696 & 15.87  & 18.609 \\
59    & 18.957 & 18.435 & 16.522 & 17.261 & 16.696 & 18.435 & 18.348 & 21.522 & 15.87  & 19.174 \\
60    & 18.87  & 18.348 & 16.522 & 17.217 & 16.826 & 18.522 & 18.435 & 21.565 & 16.261 & 19.739 \\
61    & 19.435 & 18.391 & 16.652 & 17.087 & 17.174 & 18.435 & 18.478 & 22.043 & 16.652 & 19.478 \\
62    & 20     & 18.739 & 16.565 & 17.087 & 17.609 & 18.391 & 18.478 & 21.739 & 16.826 & 18.957 \\
63    & 20.043 & 18.609 & 16.304 & 17.478 & 17.652 & 18.348 & 18.739 & 21.826 & 16.913 & 18.87  \\
64    & 20.087 & 18.739 & 16.043 & 17.565 & 17.913 & 18.435 & 18.565 & 21.87  & 17     & 18.957 \\
65    & 19.957 & 18.739 & 15.913 & 17.609 & 17.913 & 18.913 & 18.696 & 22.261 & 17.348 & 19.043 \\
66    & 20.217 & 18.609 & 15.87  & 17.957 & 18.13  & 19.043 & 19     & 22.217 & 17.565 & 19.087 \\
67    & 20.217 & 18.609 & 16.217 & 18.087 & 18.261 & 20     & 19     & 22.391 & 17.696 & 19.087 \\
68    & 20.087 & 18.913 & 16.13  & 18.217 & 18.13  & 20.087 & 19     & 22.652 & 18.348 & 19.13  \\
69    & 20.087 & 19.217 & 16.348 & 18.348 & 18.435 & 20.348 & 18.913 & 22.696 & 18.696 & 19.391 \\
70    & 20.261 & 19.304 & 16.435 & 18.391 & 18.478 & 20.087 & 19.043 & 22.87  & 18.478 & 19.304 \\
71    & 20.043 & 19.783 & 16.565 & 18.435 & 18.826 & 20.522 & 19.783 & 22.565 & 18.522 & 19.261 \\
72    & 20.261 & 20.087 & 17.174 & 18.435 & 18.826 & 20.652 & 19.826 & 22.696 & 18.913 & 19.478 \\
73    & 20.261 & 20.261 & 17.565 & 18.304 & 18.913 & 20.783 & 19.957 & 22.609 & 18.826 & 19.87  \\
74    & 20.174 & 20.087 & 18.391 & 18.652 & 19.217 & 20     & 20.391 & 22.609 & 18.739 & 20.087 \\
75    & 20.348 & 20     & 18.261 & 18.696 & 19.435 & 19.609 & 20.565 & 22.609 & 19     & 19.957 \\
76    & 20.435 & 20.217 & 18.522 & 18.826 & 19.609 & 19.957 & 20.478 & 22.565 & 19.391 & 20     \\
77    & 20.478 & 20.304 & 18.522 & 18.739 & 19.826 & 19.652 & 20.783 & 22.87  & 19.522 & 20.261 \\
78    & 21.13  & 20.391 & 19     & 18.913 & 19.913 & 19.826 & 20.696 & 22.696 & 18.87  & 20.261 \\
79    & 21.087 & 20.304 & 19.478 & 18.913 & 20.043 & 20.261 & 20.783 & 23.087 & 18.739 & 20.174 \\
80    & 21     & 20.391 & 19.652 & 18.739 & 20.174 & 20.652 & 21.043 & 22.652 & 18.826 & 20.391 \\
81    & 20.739 & 20.348 & 19.913 & 18.826 & 20.565 & 20.826 & 21.652 & 22.652 & 18.913 & 20.609 \\
82    & 21.13  & 20.391 & 20.304 & 19.304 & 20.565 & 20.435 & 21.913 & 22.652 & 19     & 21     \\
83    & 21.565 & 20.652 & 20.217 & 19.696 & 20.565 & 20.13  & 21.783 & 22.696 & 19.043 & 20.826 \\
84    & 21.826 & 20.826 & 20     & 19.957 & 21.261 & 20.217 & 21.87  & 22.696 & 19.13  & 20.739 \\
85    & 21.87  & 21     & 20.087 & 20.13  & 21.609 & 20.087 & 22.174 & 23     & 19.391 & 20.043 \\
86    & 21.739 & 21.261 & 19.783 & 20.348 & 21.304 & 20.304 & 22.609 & 23.348 & 19.565 & 20.391 \\
87    & 21.696 & 21.652 & 19.957 & 20.609 & 21.435 & 20.348 & 22.348 & 23.174 & 19.913 & 20.391 \\
88    & 21.913 & 21.913 & 20     & 20.739 & 21.609 & 20.304 & 22.435 & 23.522 & 20.087 & 20.391 \\
89    & 22.348 & 22.087 & 20.609 & 20.957 & 21.478 & 20.174 & 22     & 23.391 & 20.783 & 20.87  \\
90    & 21.87  & 22.261 & 20.913 & 20.913 & 21.913 & 20.217 & 21.826 & 23.478 & 20.957 & 21.261 \\
91    & 21.957 & 22.13  & 20.957 & 20.913 & 22.348 & 20.435 & 21.87  & 23.348 & 21     & 21.652 \\
92    & 22.043 & 21.957 & 21.174 & 21.217 & 22.652 & 20.87  & 23     & 23.565 & 21.696 & 21.913 \\
93    & 22.087 & 21.913 & 21.348 & 21.478 & 23.261 & 20.957 & 23.261 & 24     & 21.783 & 21.957 \\
94    & 22.304 & 21.783 & 21.435 & 21.957 & 23.435 & 21.174 & 23.435 & 23.957 & 22     & 22.13  \\
95    & 22.783 & 21.913 & 21.522 & 21.739 & 23.609 & 21.261 & 23.435 & 23.435 & 21.87  & 22.478 \\
96    & 23.478 & 21.609 & 21.217 & 21.87  & 22.87  & 21.739 & 23.435 & 22.435 & 22.435 & 22.739 \\
97    & 23.391 & 21.348 & 21.043 & 22.043 & 22.826 & 21.913 & 23.087 & 21.87  & 22.609 & 22.478 \\
98    & 23.609 & 21.13  & 21.348 & 22.043 & 22.957 & 22.087 & 23.609 & 21.348 & 23.13  & 22.522 \\
99    & 23.391 & 21.304 & 21.609 & 21.913 & 23.304 & 22.174 & 23.696 & 21.391 & 23.174 & 22.435 \\
100   & 23.609 & 22.043 & 21.826 & 22     & 23.522 & 22.043 & 23.739 & 21.478 & 23.174 & 22.609 \\
101   & 23.609 & 22.174 & 21.826 & 22.522 & 23.261 & 22.478 & 23.826 & 21.913 & 23.652 & 22.609 \\
102   & 23.826 & 22.435 & 21.783 & 22.13  & 23.739 & 22.522 & 23.826 & 22.435 & 23.261 & 22.478 \\
103   & 23.696 & 22.739 & 21.957 & 22.217 & 24.087 & 23.435 & 23.696 & 22.391 & 23.174 & 22.435 \\
104   & 23.739 & 22.739 & 22.783 & 22.174 & 24.087 & 23.478 & 23.913 & 22.522 & 23.913 & 23     \\
105   & 24     & 22.435 & 22.565 & 21.696 & 24.261 & 23.87  & 23.826 & 22.652 & 24.13  & 23.043 \\
106   & 24.217 & 22.522 & 22.696 & 21.739 & 24.435 & 24.13  & 23.87  & 22.652 & 24.696 & 23.261 \\
107   & 24.217 & 22.609 & 22.522 & 21.913 & 24.304 & 24.13  & 23.957 & 22.783 & 24.565 & 23.261 \\
108   & 25.13  & 22.696 & 23     & 22.261 & 24.348 & 24.261 & 24.261 & 23.304 & 24.522 & 23.478 \\
109   & 25.435 & 23.13  & 23.348 & 21.957 & 24.261 & 24.478 & 23.783 & 23.304 & 24.478 & 23.652 \\
110   & 25.304 & 23     & 23.478 & 22.348 & 24.261 & 25.174 & 23.826 & 23.348 & 24.565 & 23.522 \\
111   & 25.304 & 22.913 & 23.783 & 22.696 & 24.826 & 25.478 & 23.87  & 23.217 & 25     & 23.522 \\
112   & 25.652 & 22.696 & 23.435 & 22.87  & 25.087 & 25.696 & 24.043 & 23.217 & 25.522 & 23.261 \\
113   & 25.826 & 22.435 & 23.783 & 23     & 25.217 & 25.565 & 24.087 & 23.304 & 26     & 23.609 \\
114   & 25.87  & 22.957 & 24.043 & 22.87  & 25.478 & 25.261 & 24.304 & 23.261 & 26.043 & 23.957 \\
115   & 25.739 & 22.913 & 24.391 & 22.87  & 25.565 & 25.478 & 24.522 & 23.739 & 26.348 & 24.087 \\
116   & 25.478 & 22.652 & 24.087 & 23.435 & 25.783 & 25.478 & 24.565 & 24.13  & 26.609 & 24.043 \\
117   & 25.609 & 22.304 & 23.609 & 23.652 & 26     & 25     & 24.739 & 24.435 & 26.435 & 24.13  \\
118   & 25.435 & 22.957 & 23.783 & 24.043 & 26     & 25.13  & 24.565 & 24.652 & 26.478 & 24.435 \\
119   & 24.217 & 23.087 & 23.783 & 24.043 & 25.957 & 25.043 & 24.913 & 25.174 & 27     & 24.609 \\
120   & 22.826 & 22.957 & 23.783 & 24.043 & 25.739 & 25.261 & 24.87  & 25.217 & 27.261 & 24.565 \\
121   & 22.826 & 23.13  & 23.913 & 23.783 & 25.696 & 25.217 & 25.478 & 25.174 & 27.217 & 24.739 \\
122   & 22.783 & 23.348 & 24.174 & 23.826 & 25.652 & 25.217 & 26.087 & 25.391 & 26.783 & 23.87  \\
123   & 23.13  & 23.174 & 24.435 & 24.043 & 25.87  & 25.174 & 26.043 & 25.478 & 26.739 & 23.217 \\
124   & 23.217 & 23.652 & 24.783 & 24.826 & 25.913 & 25.304 & 25.913 & 25.957 & 27.261 & 23.696 \\
125   & 23.826 & 23.739 & 24.565 & 25.478 & 26.13  & 24.913 & 26.087 & 26.435 & 27.217 & 23.913 \\
126   & 24.435 & 24.043 & 24.478 & 25.826 & 26.696 & 24.87  & 26.304 & 27.043 & 27.739 & 21.913 \\
127   & 24.696 & 24.043 & 24.435 & 25.913 & 26.609 & 25.087 & 26.652 & 27     & 28.174 & 21.391 \\
128   & 25.087 & 24.043 & 24.826 & 25.696 & 26.652 & 25.043 & 26.696 & 27.957 & 28.783 & 22.043 \\
129   & 25.478 & 24.478 & 24.957 & 25.957 & 26.696 & 24.957 & 26.217 & 28.478 & 29.087 & 22.478 \\
130   & 25.435 & 25.391 & 24.783 & 26     & 27     & 24.652 & 26.174 & 28.435 & 29.913 & 22.478 \\
131   & 25.304 & 25.652 & 25.261 & 26.348 & 27.696 & 24.826 & 25.87  & 28.087 & 30     & 22.391 \\
132   & 25     & 26.087 & 25.609 & 26.783 & 28.304 & 24.957 & 25.826 & 28.13  & 30.348 & 22.652 \\
133   & 24.087 & 26.261 & 25.304 & 26.957 & 28.391 & 24.696 & 26.174 & 27.783 & 30.565 & 22.826 \\
134   & 23.826 & 26.13  & 25.261 & 26.87  & 28.13  & 24.739 & 26.435 & 27.913 & 30.739 & 23.174 \\
135   & 24     & 26.13  & 25.652 & 27.391 & 27.609 & 24.609 & 26.652 & 28.087 & 31.13  & 23.13  \\
136   & 24.217 & 26.348 & 26     & 27.304 & 27.783 & 24.696 & 26.957 & 28.478 & 31.652 & 23.609 \\
137   & 24.174 & 26.522 & 25.826 & 27.913 & 28.13  & 24.783 & 27.609 & 28.435 & 31.739 & 23.957 \\
138   & 23.913 & 26.435 & 26.217 & 28.348 & 28.13  & 24.913 & 27.913 & 28.391 & 31.826 & 23.87  \\
139   & 23.826 & 26.261 & 26.783 & 28.913 & 28.478 & 25     & 28.087 & 27.913 & 31.913 & 23.565 \\
140   & 24.087 & 25.783 & 26.957 & 29.391 & 28.217 & 25.174 & 28.565 & 27.696 & 32.087 & 24.217 \\
141   & 24.261 & 25.261 & 27.348 & 29.348 & 28.348 & 25.348 & 29     & 28.217 & 32.522 & 25.043 \\
142   & 24     & 25.391 & 27.522 & 29.565 & 28.174 & 25.435 & 29.13  & 28.304 & 32.913 & 25.522 \\
143   & 24.217 & 25.478 & 26.957 & 29.087 & 28.348 & 25.739 & 29.087 & 28.261 & 32.783 & 25.696 \\
144   & 23.957 & 25.913 & 26.609 & 28.913 & 28.652 & 25.783 & 29.087 & 27.783 & 32.696 & 25.783 \\
145   & 24     & 25.652 & 27     & 29.087 & 28.522 & 26.174 & 28.957 & 28.391 & 32.522 & 26.391 \\
146   & 23.87  & 25.217 & 26.87  & 29.348 & 28.783 & 26.13  & 29.043 & 28.826 & 32.435 & 26.478 \\
147   & 23.348 & 23.87  & 26.87  & 29.261 & 29.435 & 26.217 & 28.957 & 28.913 & 32.261 & 26.522 \\
148   & 23.348 & 23.087 & 26.739 & 29.739 & 29.261 & 26.565 & 29.13  & 29.217 & 32.348 & 26.217 \\
149   & 23.435 & 23.783 & 26.609 & 30.087 & 28.652 & 27.043 & 28.826 & 29.435 & 32.217 & 26.652 \\
150   & 23.522 & 24.391 & 26.652 & 29.957 & 28.609 & 27.304 & 28.783 & 29.609 & 32.565 & 26.565 \\
151   & 23.565 & 24.304 & 26.696 & 30     & 28.957 & 27.652 & 29.304 & 29.783 & 32.174 & 26.87  \\
152   & 23.652 & 24.478 & 26.565 & 30.174 & 28.826 & 27.696 & 29.522 & 29.87  & 31.522 & 26.87  \\
153   & 23.565 & 24.739 & 27     & 30.435 & 28.609 & 28.087 & 30.087 & 29.739 & 31.478 & 26.87  \\
154   & 23.913 & 24.913 & 26.826 & 30.174 & 28.696 & 28.304 & 30.565 & 29.522 & 31.565 & 27.478 \\
155   & 24.13  & 25.043 & 26.913 & 29.957 & 28.913 & 28.739 & 30.174 & 29.261 & 31.435 & 27.522 \\
156   & 24.652 & 24.826 & 26.87  & 30.13  & 29.043 & 28.783 & 29.391 & 29.957 & 31.087 & 27.435 \\
157   & 24.696 & 24.913 & 25.913 & 30.174 & 28.609 & 29.217 & 28.87  & 29.609 & 29.565 & 26.826 \\
158   & 24.522 & 26     & 25.739 & 30.043 & 28.609 & 29.043 & 29.087 & 28.391 & 29.043 & 26.609 \\
159   & 25     & 26.304 & 25.87  & 29.435 & 28.826 & 29.435 & 29.478 & 28.478 & 29.348 & 26.826 \\
160   & 24.391 & 27.174 & 25.783 & 29.826 & 28.913 & 30.174 & 29.652 & 29.478 & 29.304 & 26.913 \\
161   & 24.13  & 28.217 & 26.087 & 30.522 & 28.913 & 30.261 & 29     & 29.87  & 29.087 & 26.565 \\
162   & 24.783 & 28.913 & 26.087 & 30.522 & 29.174 & 30.522 & 29.174 & 29.87  & 29.043 & 26.957 \\
163   & 24.565 & 29.13  & 26.174 & 30.13  & 29.739 & 30.696 & 29.478 & 30.348 & 29     & 27.609 \\
164   & 24.174 & 29.348 & 26.652 & 30.391 & 30.174 & 30.826 & 29.478 & 30.957 & 29.435 & 28.174 \\
165   & 24.13  & 29.696 & 26.435 & 30.478 & 30.348 & 31.087 & 29.957 & 31.478 & 29.609 & 28.13  \\
166   & 24.261 & 29.348 & 26.652 & 30.043 & 30.478 & 31.087 & 30.783 & 31.478 & 30.217 & 27.87  \\
167   & 24.391 & 29.304 & 27.13  & 29.913 & 30.739 & 30.87  & 30.696 & 31.478 & 30.565 & 27.652 \\
168   & 24     & 29.13  & 26.826 & 30.217 & 30.826 & 30.826 & 30.478 & 31.652 & 31     & 27.739 \\
169   & 24.87  & 28.652 & 26.87  & 30.957 & 30.783 & 31     & 30.609 & 31.957 & 31.217 & 27.783 \\
170   & 24.696 & 29.043 & 26.609 & 31.348 & 30.913 & 31.87  & 31     & 31.696 & 31.652 & 27.913 \\
171   & 24.087 & 29.043 & 27.087 & 31.435 & 30.826 & 32.522 & 29.304 & 30.087 & 31.826 & 28.043 \\
172   & 24.913 & 28.957 & 27.261 & 31.478 & 31.217 & 32.435 & 28.696 & 29.739 & 31.957 & 28.174 \\
173   & 25.304 & 29.478 & 27.652 & 31.304 & 31.565 & 31.957 & 28.913 & 30.478 & 32.739 & 28.304 \\
174   & 25.522 & 29.739 & 27.87  & 31.261 & 31.826 & 31.261 & 28.696 & 30.652 & 32.913 & 28.565 \\
175   & 26     & 29.609 & 28     & 31.043 & 32.087 & 31.13  & 29.174 & 30.348 & 33.174 & 29.043 \\
176   & 26.087 & 30.087 & 28.087 & 31.043 & 32.913 & 31.348 & 29.174 & 30.609 & 33.913 & 29.522 \\
177   & 25.696 & 30.652 & 28     & 31.522 & 33.304 & 30.217 & 29.696 & 30.739 & 34.043 & 29.957 \\
178   & 24.435 & 31.043 & 27.87  & 31.826 & 33.174 & 29.522 & 29.957 & 31.348 & 34.217 & 30.261 \\
179   & 24.652 & 31.435 & 28.043 & 31.826 & 33.609 & 29.739 & 30     & 30.652 & 34.043 & 30.652 \\
180   & 25.261 & 28.478 & 28.652 & 32.739 & 33.304 & 29.826 & 28.826 & 29.609 & 33.957 & 30.783 \\
181   & 25.87  & 26.957 & 28.826 & 32.739 & 33.652 & 30.043 & 28.478 & 29.435 & 34.261 & 31.261 \\
182   & 25.783 & 27.217 & 29.043 & 32.217 & 33.348 & 30.261 & 28.609 & 28.739 & 34.435 & 31.957 \\
183   & 25.913 & 27.609 & 29     & 31.957 & 33.043 & 30.043 & 28.783 & 28.609 & 34.87  & 32.652 \\
184   & 25.13  & 27.478 & 28.826 & 31.957 & 34.087 & 30.304 & 28.739 & 28.913 & 35.304 & 32.174 \\
185   & 24.174 & 28.174 & 28.348 & 31.783 & 34.304 & 29.783 & 29.609 & 29.478 & 35.652 & 31.87  \\
186   & 24.13  & 28.739 & 27.87  & 32.043 & 34.565 & 29.522 & 30.13  & 28.739 & 34.913 & 31.739 \\
187   & 24.478 & 28.957 & 27.87  & 32.087 & 34.348 & 29.783 & 30.174 & 29.609 & 33.652 & 32.261 \\
188   & 25.348 & 29.261 & 28.217 & 31.913 & 34.87  & 30.435 & 30.696 & 30.217 & 33.435 & 32.826 \\
189   & 25.913 & 29.304 & 28.478 & 32.348 & 34.87  & 30.391 & 30.565 & 30.522 & 33     & 32.478 \\
190   & 25.565 & 29.043 & 28.174 & 32.609 & 35.609 & 30.652 & 30.913 & 30.826 & 31.87  & 31.783 \\
191   & 25.522 & 29.739 & 28.435 & 33.13  & 36.348 & 31.043 & 31.087 & 31.13  & 31.739 & 32.391 \\
192   & 24.913 & 28.043 & 28.957 & 33.043 & 36.261 & 31.478 & 31.13  & 31.261 & 31.913 & 32.783 \\
193   & 24.826 & 27.13  & 29.391 & 33.304 & 36.478 & 32.261 & 29.913 & 32.565 & 32.348 & 33.217 \\
194   & 25.217 & 25.348 & 29.652 & 33.174 & 36.826 & 32.391 & 29.609 & 33.13  & 32.217 & 32.739 \\
195   & 25.217 & 23.609 & 29.217 & 33.435 & 36.826 & 31.739 & 29.957 & 32.609 & 31.522 & 33.348 \\
196   & 25.435 & 24.652 & 28.87  & 33.478 & 37.087 & 31.217 & 29.13  & 32.652 & 30.565 & 33.261 \\
\bottomrule\end{longtable}
\normalsize
