# Supplementary material for: Rehearsal-Free Continual Learning over Small Non-I.I.D. Batches
Source: arXiv:1907.03799 source file (2020-04-21)
Supplement: Supplementary file 7 [file 391_AR1.tex]

\subsection{AR1*, NICv2 - 391}
\fontsize{8}{11}\selectfont
\begin{longtable}[c]{rgrgrgrgrgr}
\hline
Batch         & Run 0  & Run 1  & Run 2  & Run 3  & Run 4  & Run 5  & Run 6  & Run 7  & Run 8  & Run 9  \\ \hline
\endfirsthead
\endhead
0             & 7.174  & 7.174  & 7.174  & 7.174  & 7.174  & 7.174  & 7.174  & 7.174  & 7.174  & 7.174  \\
1             & 14     & 14     & 14     & 14     & 14     & 14     & 14     & 14     & 14     & 14     \\
2             & 13.435 & 13.435 & 14.696 & 14.391 & 14     & 14.391 & 13.957 & 14.043 & 14.478 & 13.87  \\
3             & 12.652 & 13.565 & 15.391 & 14.043 & 14.522 & 13.957 & 14.391 & 14.435 & 14.783 & 13.783 \\
4             & 12.087 & 13.957 & 15.565 & 14.739 & 14.609 & 14.13  & 14.696 & 14.478 & 14.174 & 13.913 \\
5             & 12.304 & 14.391 & 15.913 & 14.652 & 14.435 & 14.13  & 14.435 & 14.652 & 14.696 & 14.652 \\
6             & 12.739 & 14.13  & 16.609 & 14.174 & 14.087 & 13.609 & 14.783 & 15.391 & 14.913 & 14.348 \\
7             & 13.261 & 15.217 & 17.435 & 14.478 & 14     & 14.087 & 16     & 14.826 & 15.261 & 14.391 \\
8             & 13.261 & 15.348 & 17.609 & 14.696 & 14.652 & 13.826 & 15.783 & 14.565 & 15.304 & 14.087 \\
9             & 13.348 & 15.348 & 17.522 & 14.957 & 14.783 & 13.609 & 16.261 & 14.565 & 16.087 & 13.478 \\
10            & 13.13  & 15.652 & 17.783 & 14.783 & 14.739 & 13.391 & 16.043 & 14.826 & 15.957 & 14.348 \\
11            & 13.174 & 16.478 & 18     & 14.826 & 15.13  & 13.565 & 16.087 & 15.13  & 15.391 & 14.304 \\
12            & 13.174 & 15.913 & 17.565 & 15.174 & 14.522 & 13.739 & 16.435 & 15.261 & 15.957 & 15.217 \\
13            & 13.783 & 16.217 & 17.696 & 15.087 & 14.826 & 14.261 & 17.435 & 15.261 & 16.609 & 15.87  \\
14            & 14.13  & 16.652 & 17.609 & 14.739 & 14.957 & 14.174 & 17.348 & 15.522 & 17.348 & 16.478 \\
15            & 13.957 & 17.174 & 18.522 & 15.391 & 14.739 & 13.957 & 17.174 & 15     & 17.348 & 16.696 \\
16            & 14.565 & 17.13  & 19.478 & 15.261 & 16.652 & 14.609 & 17.348 & 15.609 & 17.478 & 17.609 \\
17            & 14.478 & 17.174 & 20.13  & 14.87  & 17     & 14.826 & 17.304 & 15.913 & 17.565 & 17.783 \\
18            & 15.043 & 17.174 & 20.391 & 15.087 & 17.391 & 15.174 & 17.348 & 15.609 & 17.391 & 17.826 \\
19            & 15.565 & 17.261 & 20.739 & 16.739 & 17.391 & 14.913 & 17.435 & 16.304 & 17.13  & 17.739 \\
20            & 15.696 & 17.348 & 20.739 & 16.348 & 17.652 & 15.174 & 17.435 & 16.435 & 17.783 & 17.696 \\
21            & 15.826 & 17.87  & 20.783 & 16.565 & 18.435 & 15.13  & 17.304 & 16.957 & 17.913 & 18.087 \\
22            & 16.087 & 17.87  & 20.609 & 16.565 & 18.261 & 15.087 & 17.957 & 16.783 & 17.913 & 17.913 \\
23            & 16.522 & 18.043 & 20.826 & 16.609 & 18.826 & 15.565 & 17.913 & 17.043 & 17.739 & 17.783 \\
24            & 16.522 & 18.043 & 20.913 & 16.87  & 19.304 & 16.217 & 18.304 & 17.217 & 17.783 & 17.739 \\
25            & 16.565 & 18.304 & 20.783 & 17.13  & 19.783 & 16.391 & 18.261 & 17.478 & 18.217 & 17.957 \\
26            & 16.696 & 18.13  & 20.783 & 17.304 & 19.826 & 16.739 & 18.217 & 17.609 & 18.13  & 18.391 \\
27            & 16.696 & 18.783 & 20.652 & 17.609 & 19.957 & 16.783 & 18.261 & 17.739 & 18.522 & 18.13  \\
28            & 16.913 & 18.783 & 21.087 & 18.217 & 20.348 & 16.783 & 18.217 & 18.087 & 18.609 & 18.174 \\
29            & 17     & 18.783 & 20.87  & 18.174 & 20.13  & 17.435 & 18.348 & 18.087 & 18.826 & 18.565 \\
30            & 17.478 & 18.783 & 20.826 & 18.609 & 20.304 & 17.522 & 18.435 & 17.957 & 18.826 & 18.739 \\
31            & 17.522 & 18.826 & 21.304 & 18.652 & 20.739 & 17.478 & 18.652 & 18.478 & 18.783 & 18.87  \\
32            & 17.696 & 19.261 & 21.435 & 18.913 & 20.913 & 17.304 & 18.87  & 18.435 & 18.478 & 18.957 \\
33            & 17.565 & 19.522 & 22.261 & 18.913 & 21.261 & 17.435 & 19.391 & 18.696 & 19     & 18.739 \\
34            & 18.13  & 19.435 & 22.304 & 19.043 & 21.391 & 17.13  & 19.783 & 19     & 18.957 & 19.043 \\
35            & 18.217 & 19.435 & 22.826 & 19.739 & 21.261 & 17.217 & 19.957 & 18.957 & 19.348 & 19.478 \\
36            & 18.304 & 19.522 & 22.87  & 19.957 & 21.348 & 17.522 & 20.348 & 18.913 & 19.826 & 19.522 \\
37            & 18.174 & 19.304 & 23.087 & 20.174 & 21.435 & 18.087 & 20.261 & 19.043 & 19.652 & 19.348 \\
38            & 18.522 & 19.217 & 23.348 & 20.087 & 21.261 & 18.217 & 20.391 & 19     & 19.565 & 19.391 \\
39            & 18.478 & 18.609 & 23.391 & 20.348 & 21.348 & 18.435 & 20.391 & 18.87  & 19.696 & 21.13  \\
40            & 18.435 & 18.565 & 23.174 & 20.435 & 21.565 & 18.435 & 20.261 & 19.435 & 20.348 & 20.957 \\
41            & 18.478 & 19.478 & 23.261 & 20.783 & 21.522 & 18.435 & 20.652 & 19.522 & 20.478 & 21.087 \\
42            & 18.652 & 19.826 & 23.087 & 20.957 & 21.522 & 18.391 & 20.652 & 19.522 & 20.478 & 21.435 \\
43            & 18.609 & 19.913 & 23.043 & 20.957 & 22.261 & 18.391 & 20.565 & 19.739 & 20.435 & 21.609 \\
44            & 18.652 & 19.739 & 23.478 & 21.043 & 22.391 & 18.348 & 20.783 & 19.783 & 20.739 & 22.13  \\
45            & 18.609 & 19.652 & 23.478 & 20.913 & 22.652 & 18.565 & 20.783 & 19.739 & 20.652 & 22.043 \\
46            & 18.739 & 19.609 & 23.304 & 21     & 23.304 & 18.696 & 20.826 & 19.652 & 20.609 & 22.522 \\
47            & 18.826 & 20.043 & 23.478 & 21.043 & 23.652 & 18.739 & 21.087 & 20.174 & 20.478 & 22.522 \\
48            & 19.043 & 20.043 & 23.565 & 20.957 & 23.913 & 19     & 21.043 & 20.13  & 20.522 & 22.783 \\
49            & 18.957 & 19.913 & 23.565 & 21     & 23.957 & 19     & 20.957 & 20.609 & 20.522 & 22.783 \\
50            & 19.261 & 20     & 23.435 & 20.783 & 23.913 & 19     & 21.174 & 20.739 & 20.478 & 22.783 \\
51            & 19.304 & 20.13  & 23.435 & 20.739 & 23.957 & 19.261 & 21.565 & 20.696 & 20.478 & 22.826 \\
52            & 19.348 & 20.087 & 23.522 & 20.826 & 24.522 & 19.652 & 21.696 & 20.826 & 20.348 & 22.87  \\
53            & 19.348 & 20     & 23.217 & 20.826 & 24.609 & 19.696 & 21.652 & 20.826 & 20.522 & 23     \\
54            & 19.304 & 20.391 & 23.348 & 20.826 & 24.826 & 19.87  & 21.565 & 21.261 & 20.783 & 22.783 \\
55            & 19.348 & 20.435 & 23.261 & 20.913 & 24.913 & 19.783 & 21.87  & 21.261 & 21.043 & 22.87  \\
56            & 19.348 & 20.348 & 23.261 & 21     & 24.609 & 19.913 & 22.13  & 21.174 & 21.13  & 22.957 \\
57            & 21.217 & 20.565 & 23.609 & 21.087 & 24.565 & 20     & 22.13  & 21.348 & 21.087 & 23     \\
58            & 21.304 & 20.261 & 23.783 & 21.913 & 24.696 & 20     & 22.13  & 21.435 & 21.739 & 23.304 \\
59            & 21.435 & 20.565 & 24.043 & 21.913 & 24.565 & 20     & 22.087 & 21.435 & 21.696 & 23.565 \\
60            & 21.435 & 20.217 & 24.304 & 22.652 & 24.565 & 20.174 & 22.13  & 22.13  & 21.87  & 23.522 \\
61            & 21.348 & 20.13  & 24.522 & 22.609 & 24.391 & 20.304 & 22.217 & 22.13  & 21.913 & 23.13  \\
62            & 21.609 & 20.826 & 24.522 & 22.522 & 24.826 & 20.565 & 22.174 & 22.217 & 21.87  & 23.13  \\
63            & 21.696 & 20.87  & 24.304 & 22.696 & 25.043 & 20.565 & 22.174 & 22.174 & 21.696 & 23.696 \\
64            & 21.739 & 20.826 & 24.304 & 23.522 & 26.043 & 21.261 & 22.261 & 22.174 & 21.913 & 23.957 \\
65            & 21.87  & 21.217 & 24.391 & 23.522 & 26.087 & 21.826 & 22.261 & 22.304 & 21.652 & 23.826 \\
66            & 21.87  & 21.217 & 24.348 & 23.609 & 26.565 & 22.043 & 22.304 & 22.348 & 21.913 & 24.174 \\
67            & 22.174 & 21     & 24.522 & 24.043 & 27.261 & 21.913 & 22.087 & 22.435 & 21.957 & 24.261 \\
68            & 22.174 & 21.565 & 24.478 & 24.261 & 27.696 & 21.913 & 22     & 22.565 & 21.783 & 24.304 \\
69            & 22.348 & 21.522 & 24.739 & 24.304 & 27.522 & 21.87  & 23     & 23.217 & 21.652 & 24.391 \\
70            & 22.217 & 21.87  & 25.739 & 24.087 & 27.913 & 21.739 & 23.261 & 23.174 & 21.826 & 24.696 \\
71            & 22.174 & 22.087 & 26.261 & 24.174 & 27.87  & 21.957 & 23.261 & 23.217 & 21.87  & 25.304 \\
72            & 22.13  & 22.087 & 27     & 24     & 27.87  & 22.087 & 23.261 & 23.304 & 21.957 & 25.696 \\
73            & 22.217 & 22.087 & 27.261 & 24.348 & 28.13  & 22.174 & 23.304 & 23.217 & 21.957 & 25.478 \\
74            & 22.304 & 22.13  & 28     & 24.435 & 27.522 & 23.043 & 23.13  & 23.13  & 22.13  & 25.478 \\
75            & 22.348 & 22.217 & 27.783 & 24.217 & 27.739 & 22.783 & 23.304 & 23.174 & 22.13  & 25.609 \\
76            & 22.087 & 22.13  & 27.957 & 24.261 & 27.87  & 22.696 & 23.261 & 23.261 & 22.652 & 25.783 \\
77            & 22.391 & 22.261 & 28.435 & 24.087 & 27.913 & 22.826 & 23.522 & 23.652 & 22.522 & 26.217 \\
78            & 22.652 & 22.435 & 28.478 & 24.522 & 28.435 & 23.087 & 23.783 & 23.609 & 22.609 & 26.391 \\
79            & 22.696 & 22.391 & 29.435 & 24.957 & 28.913 & 23.435 & 23.87  & 23.609 & 22.696 & 26.304 \\
80            & 22.783 & 22.696 & 29.609 & 24.913 & 28.739 & 23.652 & 23.913 & 23.435 & 22.87  & 26.391 \\
81            & 23.826 & 22.652 & 29.652 & 25.087 & 29.13  & 23.348 & 24.348 & 23.435 & 22.87  & 26.478 \\
82            & 24.043 & 22.565 & 29.739 & 25.783 & 29.391 & 23.304 & 24.304 & 23.435 & 23.261 & 26.478 \\
83            & 24.13  & 22.609 & 29.87  & 25.87  & 29.565 & 23.783 & 24.348 & 23.478 & 23.174 & 26.261 \\
84            & 24.174 & 22.652 & 30     & 26.043 & 29.522 & 24.087 & 24.348 & 23.435 & 23.348 & 26.913 \\
85            & 24.478 & 22.652 & 30.043 & 26.391 & 30.13  & 24.217 & 24.304 & 23.304 & 22.87  & 26.783 \\
86            & 24.913 & 22.652 & 30.087 & 26.652 & 30.217 & 24.348 & 24.261 & 23.565 & 23.13  & 27.696 \\
87            & 25.13  & 22.696 & 30.522 & 26.609 & 30.783 & 24.696 & 24.217 & 23.565 & 23.348 & 27.783 \\
88            & 25.261 & 22.652 & 30.913 & 26.739 & 30.826 & 24.565 & 24.217 & 23.87  & 23.478 & 27.957 \\
89            & 25.217 & 22.739 & 31.304 & 26.783 & 31.348 & 24.652 & 24.348 & 23.87  & 24     & 28.304 \\
90            & 25.174 & 22.783 & 31.391 & 26.87  & 31.478 & 24.652 & 24.435 & 24.348 & 23.87  & 28.304 \\
91            & 25.174 & 22.913 & 31.609 & 27.391 & 31.696 & 25.13  & 24.609 & 24.522 & 24.304 & 28.391 \\
92            & 25.348 & 22.87  & 31.609 & 27.261 & 31.783 & 25.217 & 24.739 & 24.565 & 24.391 & 28.478 \\
93            & 25.609 & 24     & 31.957 & 26.739 & 31.957 & 25.435 & 24.87  & 24.435 & 24.348 & 28.739 \\
94            & 25.435 & 24.13  & 32.087 & 26.783 & 32     & 25.565 & 24.739 & 24.478 & 24.609 & 28.739 \\
95            & 25.348 & 24.043 & 32     & 26.87  & 32.435 & 25.478 & 24.826 & 24.565 & 24.478 & 28.87  \\
96            & 26.087 & 24.13  & 32.043 & 26.652 & 32.652 & 25.696 & 24.87  & 24.522 & 24.609 & 29.13  \\
97            & 26.174 & 24.174 & 32.217 & 26.87  & 32.652 & 25.696 & 24.957 & 24.87  & 25.217 & 28.957 \\
98            & 26.087 & 24.043 & 32.435 & 27.217 & 32.87  & 25.739 & 25.043 & 25     & 25.174 & 29.087 \\
99            & 26.13  & 24.13  & 32.565 & 27.652 & 33.043 & 26.174 & 25.13  & 25.087 & 25.739 & 29.348 \\
100           & 26.435 & 24.435 & 32.217 & 27.739 & 33.261 & 26.174 & 25.391 & 25.217 & 25.696 & 29.565 \\
101           & 26.739 & 24.609 & 32.478 & 27.739 & 33.304 & 26.261 & 25.565 & 25.391 & 25.957 & 29.826 \\
102           & 27.217 & 24.913 & 32.696 & 28.304 & 33.522 & 26.435 & 25.304 & 25.478 & 26     & 30.13  \\
103           & 27.435 & 25.043 & 32.739 & 28.391 & 33.826 & 26.522 & 25.391 & 25.435 & 25.739 & 30.217 \\
104           & 27.826 & 25.043 & 33.043 & 28.217 & 34     & 26.739 & 25.435 & 25.957 & 26.217 & 30.391 \\
105           & 27.87  & 24.957 & 33.435 & 28.261 & 34.304 & 26.739 & 25.478 & 25.87  & 26.391 & 30.478 \\
106           & 27.783 & 24.957 & 33.522 & 28.348 & 34.391 & 27.13  & 25.783 & 25.913 & 26.217 & 30.565 \\
107           & 27.783 & 25.043 & 33.217 & 28.435 & 34.826 & 27.261 & 25.957 & 26.043 & 26.261 & 31.087 \\
108           & 27.957 & 24.826 & 33.087 & 28.913 & 35.261 & 27.652 & 27.696 & 26.087 & 26.522 & 31.391 \\
109           & 27.87  & 24.87  & 33.087 & 28.826 & 35.609 & 27.435 & 27.87  & 26.043 & 26.957 & 32.261 \\
110           & 28.043 & 25.348 & 33.261 & 28.87  & 35.435 & 28.565 & 28.217 & 25.87  & 26.609 & 32.565 \\
111           & 28.217 & 25.435 & 33.348 & 28.957 & 35.478 & 28.522 & 28.174 & 25.913 & 27.261 & 33.087 \\
112           & 28.609 & 25.304 & 33.435 & 28.783 & 35.522 & 28.435 & 28.652 & 26.261 & 27.217 & 33.478 \\
113           & 29.261 & 25.348 & 33.522 & 29.087 & 35.435 & 28.696 & 28.739 & 27.13  & 27.348 & 33.957 \\
114           & 29.174 & 25.304 & 33.217 & 29.087 & 35.391 & 28.826 & 28.826 & 27.217 & 27.565 & 33.565 \\
115           & 29.087 & 25.696 & 33.348 & 29.304 & 35.304 & 28.957 & 28.739 & 27.739 & 27.826 & 34.174 \\
116           & 29.174 & 26.043 & 33.261 & 29.13  & 34.609 & 28.87  & 28.696 & 27.913 & 27.957 & 34.435 \\
117           & 29.217 & 26.13  & 33.304 & 29.304 & 34.565 & 28.87  & 28.739 & 27.783 & 27.522 & 34.435 \\
118           & 29.087 & 26.043 & 33.261 & 29.565 & 34.522 & 29.043 & 29     & 28.043 & 27.783 & 34.87  \\
119           & 29.13  & 26.13  & 33.435 & 29.739 & 35.304 & 29.304 & 28.957 & 27.87  & 27.565 & 34.913 \\
120           & 29.13  & 26.13  & 33.696 & 29.739 & 35.217 & 29.217 & 29.043 & 27.826 & 27.783 & 34.913 \\
121           & 29.304 & 26.217 & 33.696 & 29.826 & 35.478 & 29.565 & 29.087 & 27.478 & 28.261 & 35.435 \\
122           & 29.696 & 26.174 & 33.87  & 29.87  & 35.783 & 29.565 & 29     & 27.652 & 28.304 & 35.391 \\
123           & 29.826 & 26.826 & 33.957 & 29.957 & 36.174 & 29.304 & 29     & 28.087 & 28.304 & 35.435 \\
124           & 29.957 & 27.391 & 34.696 & 29.913 & 36.217 & 29.304 & 29.261 & 28.304 & 28.348 & 35.522 \\
125           & 29.826 & 28.217 & 35.217 & 30.043 & 36.087 & 29.348 & 29.348 & 28.217 & 28.522 & 35.391 \\
126           & 29.783 & 28.348 & 35.174 & 30.043 & 35.957 & 29.13  & 29.261 & 28.565 & 28.696 & 35.522 \\
127           & 30.174 & 28.652 & 35.435 & 30.043 & 36     & 29.609 & 29.391 & 29.261 & 28.87  & 35.609 \\
128           & 30.304 & 28.696 & 35.609 & 30.13  & 36.087 & 29.609 & 29.87  & 29.217 & 28.739 & 35.652 \\
129           & 30.87  & 29.261 & 35.652 & 30.261 & 35.739 & 29.739 & 29.957 & 29.348 & 28.652 & 36     \\
130           & 31.174 & 29.435 & 35.478 & 30.435 & 36.087 & 29.739 & 29.957 & 29.783 & 28.826 & 35.913 \\
131           & 31.174 & 29.783 & 35.826 & 30.87  & 36.043 & 29.565 & 30.043 & 30.174 & 28.87  & 36.043 \\
132           & 31.478 & 29.696 & 35.826 & 30.609 & 35.957 & 29.652 & 30.174 & 30.174 & 29.087 & 36.13  \\
133           & 31.391 & 29.739 & 35.957 & 30.565 & 36.348 & 29.565 & 30.391 & 30.087 & 29.13  & 36.348 \\
134           & 31.522 & 29.87  & 35.783 & 30.696 & 36.304 & 29.652 & 30.348 & 29.826 & 29     & 36.217 \\
135           & 31.522 & 29.739 & 35.565 & 30.652 & 36.174 & 29.739 & 30.217 & 30.043 & 29     & 36.652 \\
136           & 31.435 & 30.087 & 35.652 & 30.522 & 36.435 & 29.957 & 30.087 & 30.174 & 28.957 & 37.174 \\
137           & 31.348 & 30.478 & 35.435 & 30.522 & 36.304 & 29.957 & 30.217 & 30.217 & 28.391 & 37.043 \\
138           & 31.609 & 30.522 & 35.348 & 30.652 & 36.478 & 30     & 30.391 & 30.304 & 29     & 37     \\
139           & 31.826 & 30.652 & 35.652 & 30.913 & 36.435 & 30.652 & 30.391 & 30.609 & 28.739 & 37.087 \\
140           & 31.652 & 30.348 & 35.304 & 32     & 36.174 & 30.913 & 30.304 & 30.696 & 28.826 & 37.261 \\
141           & 31.87  & 30.522 & 35.174 & 31.913 & 35.957 & 31.565 & 30.478 & 30.913 & 29.391 & 37.696 \\
142           & 32     & 30.522 & 35.261 & 31.957 & 35.696 & 31.609 & 30.565 & 30.913 & 29     & 37.957 \\
143           & 33.087 & 31.043 & 35.391 & 32.217 & 35.783 & 31.565 & 30.783 & 31.435 & 29.087 & 38.043 \\
144           & 33     & 31.391 & 35.391 & 32.391 & 35.957 & 31.391 & 31.043 & 31.696 & 29.435 & 38.174 \\
145           & 32.957 & 31.609 & 35.348 & 32.435 & 36     & 31.478 & 31.13  & 31.696 & 29.348 & 38.522 \\
146           & 33.087 & 31.565 & 35.261 & 32.565 & 36.043 & 31.348 & 31.217 & 31.87  & 29.261 & 38.261 \\
147           & 33.043 & 31.478 & 35.087 & 32.435 & 36.174 & 31.522 & 31.043 & 32.217 & 29.435 & 38.435 \\
148           & 33.783 & 31.739 & 35.217 & 32.696 & 36.174 & 31.913 & 30.783 & 32.217 & 29.609 & 38.435 \\
149           & 33.652 & 31.87  & 35.348 & 32.696 & 35.913 & 31.739 & 31.043 & 32.348 & 29.478 & 38.435 \\
150           & 33.87  & 31.826 & 35.522 & 32.913 & 36.174 & 31.957 & 30.957 & 32.478 & 29.522 & 38.217 \\
151           & 34.174 & 32     & 35.739 & 32.957 & 36.174 & 32.174 & 31     & 32.565 & 29.609 & 38.043 \\
152           & 34.348 & 32.13  & 35.783 & 33.13  & 36.304 & 32.174 & 31.174 & 32.609 & 29.522 & 38.13  \\
153           & 34.304 & 32.391 & 35.304 & 33.13  & 36.304 & 32.391 & 31.304 & 33.174 & 29.609 & 38.348 \\
154           & 34.043 & 32.652 & 36.043 & 32.739 & 36.304 & 33.261 & 31.391 & 33.609 & 29.609 & 38.391 \\
155           & 34.652 & 32.609 & 36.043 & 32.783 & 36.391 & 33.391 & 31.522 & 33.783 & 30.565 & 39.261 \\
156           & 34.652 & 32.826 & 36.739 & 32.783 & 36.304 & 33.435 & 31.957 & 33.739 & 30.87  & 39.174 \\
157           & 34.652 & 32.826 & 36.435 & 32.87  & 36.609 & 33.435 & 31.913 & 34.348 & 30.957 & 39.348 \\
158           & 34.435 & 32.826 & 35.696 & 33     & 36.609 & 33.522 & 31.696 & 34.478 & 31.391 & 39.217 \\
159           & 34.652 & 32.957 & 35.348 & 32.913 & 36.348 & 33.435 & 32.522 & 34.087 & 31.957 & 39.478 \\
160           & 34.783 & 33.13  & 35.565 & 33.087 & 36.174 & 33.478 & 32.522 & 34     & 32.522 & 39.609 \\
161           & 34.652 & 33.391 & 35.478 & 33.043 & 36.087 & 34     & 32.391 & 34.087 & 32.609 & 39.696 \\
162           & 34.652 & 33.304 & 35.652 & 33.13  & 35.913 & 34     & 32.435 & 34.304 & 32.565 & 39.391 \\
163           & 34.696 & 33.652 & 35.478 & 33.087 & 35.913 & 33.913 & 33.087 & 35.13  & 32.739 & 39.87  \\
164           & 34.826 & 33.826 & 35.522 & 33.13  & 35.826 & 33.87  & 33.174 & 35.435 & 32.565 & 39.652 \\
165           & 34.739 & 33.783 & 35.696 & 33.087 & 36.217 & 33.913 & 33.391 & 35.435 & 32.739 & 39.609 \\
166           & 34.957 & 33.783 & 35.696 & 33.348 & 36.348 & 34.174 & 33.304 & 35.435 & 33.087 & 39.696 \\
167           & 34.957 & 33.783 & 36.609 & 33.304 & 36.435 & 34.043 & 33.478 & 35.739 & 32.957 & 39.522 \\
168           & 34.739 & 33.87  & 36.913 & 33.739 & 37.217 & 34.522 & 33.478 & 35.652 & 33.174 & 40     \\
169           & 34.261 & 34.348 & 36.478 & 33.609 & 37.261 & 34.304 & 33.478 & 35.565 & 33.304 & 40.174 \\
170           & 34.87  & 34.522 & 36.739 & 33.435 & 37.261 & 34.435 & 33.478 & 35.609 & 33.565 & 40     \\
171           & 34.739 & 34.652 & 36.826 & 33.609 & 37.609 & 34.565 & 33.522 & 35.696 & 33.696 & 40.043 \\
172           & 35     & 34.522 & 36.609 & 33.696 & 37.696 & 35.087 & 33.522 & 35.478 & 34.174 & 39.826 \\
173           & 35.652 & 34.435 & 36.826 & 34.565 & 37.913 & 35.652 & 33.391 & 36.13  & 34.261 & 40.13  \\
174           & 35.478 & 34.957 & 36.739 & 35.13  & 37.739 & 35.696 & 33.565 & 36     & 34.435 & 40.261 \\
175           & 35.696 & 35.217 & 36.652 & 35.174 & 37.652 & 35.348 & 33.391 & 36.739 & 34.609 & 40.087 \\
176           & 35.478 & 35.13  & 36.739 & 35.174 & 37.652 & 35.696 & 33.565 & 36.696 & 35.391 & 40.522 \\
177           & 35.435 & 35.174 & 36.652 & 35.609 & 37.609 & 35.565 & 33.783 & 36.783 & 35.304 & 41     \\
178           & 35.522 & 35.174 & 36.783 & 35.826 & 37.826 & 35.87  & 34     & 37.087 & 35.174 & 41     \\
179           & 35.391 & 35.478 & 37.043 & 35.957 & 38     & 35.826 & 34.13  & 37.174 & 35.696 & 41.087 \\
180           & 36.13  & 35.739 & 37.043 & 36.522 & 37.913 & 35.783 & 33.957 & 37.174 & 35.739 & 41.261 \\
181           & 36.261 & 36     & 37     & 36.522 & 38.217 & 36     & 33.913 & 36.957 & 36     & 41.522 \\
182           & 36.261 & 36.304 & 36.87  & 36.87  & 38.174 & 35.826 & 33.739 & 36.87  & 35.87  & 41.565 \\
183           & 36.174 & 36.348 & 36.826 & 36.913 & 38.304 & 36.043 & 34.261 & 36.609 & 36.478 & 41.609 \\
184           & 36.783 & 36.565 & 36.913 & 36.913 & 38.087 & 35.957 & 34.739 & 36.565 & 37.217 & 41.87  \\
185           & 36.652 & 36.565 & 36.957 & 36.783 & 37.87  & 36.217 & 34.652 & 36.87  & 37.043 & 42.043 \\
186           & 36.696 & 36.609 & 37.304 & 37.261 & 38.522 & 36.348 & 34.696 & 36.87  & 37.435 & 41.913 \\
187           & 37.565 & 36.522 & 37.348 & 37.522 & 38.87  & 36.696 & 34.609 & 37.174 & 38.087 & 41.957 \\
188           & 37.652 & 36.522 & 37.261 & 37.217 & 38.957 & 36.739 & 34.826 & 37.13  & 38     & 42.043 \\
189           & 37.652 & 36.609 & 37.522 & 37.391 & 39     & 36.696 & 34.957 & 37.435 & 38.087 & 42.087 \\
190           & 38.478 & 36.478 & 38.174 & 37.696 & 38.957 & 36.913 & 35.435 & 37.304 & 38.522 & 42.13  \\
191           & 38.652 & 36.609 & 38.261 & 37.957 & 38.739 & 37.348 & 35.696 & 37.435 & 38.87  & 42.217 \\
192           & 38.478 & 36.87  & 38.087 & 38.174 & 38.696 & 37.696 & 36.043 & 37.609 & 39.13  & 42.087 \\
193           & 38.261 & 37.217 & 37.913 & 38.391 & 38.87  & 37.609 & 36.261 & 37.565 & 39.043 & 42.13  \\
194           & 38.261 & 37.043 & 38.174 & 38.304 & 38.957 & 37.739 & 36.565 & 37.478 & 39.739 & 42.13  \\
195           & 38.783 & 37     & 38.348 & 38.348 & 38.826 & 37.87  & 36.826 & 37.609 & 39.565 & 42.087 \\
196           & 38.957 & 36.87  & 38.217 & 39     & 38.826 & 37.609 & 36.739 & 37.826 & 40.043 & 42     \\
197           & 39.087 & 36.913 & 38.435 & 39.087 & 39     & 38.13  & 36.957 & 37.913 & 40.087 & 41.957 \\
198           & 38.957 & 37.043 & 38.391 & 39.087 & 39     & 38.348 & 37.043 & 37.826 & 40.391 & 42.174 \\
199           & 38.783 & 37.087 & 38.478 & 39.348 & 38.913 & 38.522 & 37.261 & 37.913 & 40.652 & 42.391 \\
200           & 38.652 & 37.043 & 38.826 & 39.652 & 39.087 & 38.609 & 37.435 & 38.217 & 40.957 & 42.783 \\
201           & 38.739 & 37.043 & 38.957 & 39.696 & 39.13  & 38.87  & 37.478 & 38.435 & 40.783 & 43     \\
202           & 38.522 & 37.043 & 39.087 & 39.739 & 39.304 & 38.913 & 37.87  & 38.217 & 40.957 & 43.174 \\
203           & 38.435 & 36.739 & 38.957 & 39.565 & 39.13  & 38.696 & 37.522 & 38.348 & 41.174 & 43.696 \\
204           & 38.522 & 37     & 39.217 & 39.783 & 39.652 & 38.696 & 37.783 & 38.435 & 41.522 & 43.957 \\
205           & 39.13  & 36.87  & 39.13  & 40.043 & 39.522 & 38.609 & 37.87  & 38.652 & 41.87  & 44.435 \\
206           & 39.435 & 36.696 & 38.783 & 41.87  & 39.478 & 38.913 & 37.87  & 38.609 & 42.217 & 44.174 \\
207           & 39.696 & 37.174 & 39.13  & 42.261 & 40.087 & 38.913 & 37.522 & 39.174 & 42.348 & 44.478 \\
208           & 39.696 & 37.565 & 39.261 & 42.348 & 40.13  & 39.348 & 37.348 & 39     & 42.087 & 44.826 \\
209           & 40     & 37.522 & 39.043 & 42.348 & 40.348 & 39.261 & 37.783 & 39.087 & 42.435 & 45.087 \\
210           & 40.217 & 37.478 & 39.391 & 41.957 & 40.348 & 39.609 & 38.391 & 39.13  & 42.565 & 44.913 \\
211           & 40.13  & 37.522 & 39.348 & 41.783 & 40.522 & 39.522 & 38.348 & 39     & 42.609 & 45.522 \\
212           & 40.522 & 37.478 & 39.304 & 42.478 & 40.304 & 39.783 & 38.913 & 38.913 & 42.435 & 45.696 \\
213           & 40.87  & 37.478 & 39.913 & 42.261 & 40.304 & 39.609 & 38.783 & 39.043 & 42.391 & 45.609 \\
214           & 40.652 & 37.391 & 40     & 42.522 & 40.304 & 39.652 & 39.174 & 39.217 & 42.696 & 45.609 \\
215           & 40.87  & 37.522 & 40.13  & 42.261 & 40.435 & 39.696 & 39.217 & 39.609 & 42.783 & 45.826 \\
216           & 41     & 37.348 & 40.304 & 42.391 & 40.87  & 39.609 & 39.609 & 39.478 & 42.609 & 45.478 \\
217           & 40.783 & 37.261 & 40.522 & 42.565 & 41.565 & 39.565 & 40.043 & 39.652 & 43.391 & 46     \\
218           & 41.13  & 37.13  & 40.435 & 42.609 & 41.913 & 39.478 & 40.565 & 39.957 & 43.174 & 46.087 \\
219           & 41.87  & 37.261 & 40.739 & 42.652 & 42.087 & 39.957 & 40.696 & 39.913 & 43.13  & 45.87  \\
220           & 41.696 & 37.391 & 40.652 & 42.826 & 42.043 & 40.174 & 41.217 & 40.783 & 43.304 & 46.174 \\
221           & 41.913 & 37.565 & 40.609 & 42.913 & 42.304 & 40.087 & 41.522 & 41.304 & 44.957 & 46.174 \\
222           & 42.13  & 37.478 & 40.783 & 43     & 42.522 & 40.217 & 41.522 & 40.957 & 44.957 & 46.304 \\
223           & 41.826 & 37.609 & 41     & 43     & 42.565 & 40.217 & 42.043 & 41.348 & 44.87  & 46.435 \\
224           & 41.739 & 37.739 & 41.391 & 43.087 & 42.435 & 40.13  & 42.304 & 40.957 & 44.87  & 46.87  \\
225           & 41.87  & 37.652 & 41.391 & 42.652 & 42.609 & 39.826 & 42.348 & 41.348 & 44.957 & 46.826 \\
226           & 42     & 37.652 & 41.043 & 42.783 & 42.522 & 39.957 & 42.304 & 41.739 & 45.087 & 46.87  \\
227           & 41.826 & 37.783 & 40.609 & 42.913 & 42.435 & 39.913 & 42.348 & 41.478 & 45.348 & 46.783 \\
228           & 41.957 & 37.652 & 41     & 42.913 & 42.565 & 39.826 & 42.217 & 42.043 & 45.043 & 47.174 \\
229           & 42.087 & 37.957 & 41.391 & 42.783 & 42.739 & 40.261 & 42.304 & 42.478 & 45.304 & 46.957 \\
230           & 42.261 & 38.174 & 41.87  & 42.565 & 42.783 & 40.435 & 42.087 & 42.565 & 45.609 & 47.043 \\
231           & 42.13  & 38.13  & 41.652 & 42.739 & 43.304 & 40.652 & 42.348 & 42.435 & 45.522 & 47     \\
232           & 42.304 & 38.522 & 41.783 & 42.696 & 43.696 & 40.913 & 42.391 & 42.609 & 45.957 & 46.913 \\
233           & 42.435 & 38.522 & 41.826 & 42.957 & 43.826 & 40.565 & 42.13  & 42.739 & 45.957 & 47     \\
234           & 42.304 & 38.739 & 41.609 & 43.174 & 43.826 & 40.696 & 41.957 & 42.783 & 46     & 47.087 \\
235           & 42.435 & 38.957 & 41.652 & 43.087 & 43.87  & 40.652 & 42.174 & 43.043 & 45.957 & 46.87  \\
236           & 42.478 & 38.957 & 41.826 & 43.652 & 44.217 & 40.87  & 42.13  & 42.696 & 45.913 & 46.826 \\
237           & 42.652 & 38.826 & 41.609 & 43.522 & 44.478 & 40.957 & 42.435 & 43.13  & 45.957 & 46.739 \\
238           & 42.609 & 38.957 & 41.87  & 43.478 & 44.304 & 41.304 & 42.217 & 43.13  & 46.174 & 46.957 \\
239           & 42.261 & 39.043 & 41.957 & 43.304 & 44.13  & 41.522 & 42.217 & 43.391 & 45.826 & 47     \\
240           & 42.217 & 39.348 & 42     & 43.87  & 43.913 & 41.478 & 42.652 & 42.87  & 45.565 & 46.87  \\
241           & 42.261 & 39.174 & 42.043 & 43.783 & 43.87  & 41.522 & 42.783 & 43.13  & 45.391 & 46.913 \\
242           & 42.652 & 39.739 & 42.652 & 43.565 & 44.217 & 41.435 & 42.913 & 43.478 & 45.391 & 46.522 \\
243           & 42.783 & 39.696 & 42.826 & 43.696 & 44.913 & 41.565 & 42.652 & 43.522 & 45.391 & 46.87  \\
244           & 42.609 & 40.304 & 44.565 & 43.391 & 44.826 & 41.565 & 43.522 & 43.435 & 45.565 & 46.957 \\
245           & 42.696 & 40.174 & 44.565 & 44.435 & 44.957 & 41.913 & 43.261 & 43.522 & 45.522 & 46.783 \\
246           & 42.87  & 40.217 & 44.435 & 44.739 & 45.913 & 42.261 & 43.174 & 43.522 & 45.696 & 46.783 \\
247           & 43.217 & 40.217 & 44.261 & 44.739 & 46.043 & 42.304 & 43.652 & 43.391 & 45.565 & 46.826 \\
248           & 43.391 & 40.522 & 44.609 & 44.478 & 45.957 & 42.13  & 43.826 & 43.739 & 45.652 & 47.348 \\
249           & 43.609 & 40.391 & 44.783 & 44.478 & 45.826 & 42.391 & 43.826 & 43.826 & 45.739 & 47.565 \\
250           & 43.348 & 40.522 & 44.783 & 44.913 & 45.913 & 42.522 & 44.043 & 43.739 & 45.87  & 47.261 \\
251           & 43.435 & 40.478 & 44.87  & 44.739 & 46.043 & 42.522 & 44.217 & 43.783 & 45.87  & 47.13  \\
252           & 43.565 & 40.478 & 45.174 & 45.043 & 46     & 42.435 & 44.435 & 43.478 & 46.13  & 47.217 \\
253           & 43.609 & 40.522 & 45.174 & 45.217 & 46     & 42.348 & 44.348 & 43.391 & 46.087 & 47.652 \\
254           & 43.522 & 40.478 & 45.174 & 45.696 & 45.783 & 42.478 & 44.435 & 43.261 & 46.043 & 47.652 \\
255           & 43.391 & 40.478 & 45.478 & 45.478 & 46.043 & 42.217 & 44.348 & 42.87  & 46.261 & 47.304 \\
256           & 43.478 & 40.348 & 45.522 & 46.217 & 45.87  & 42.087 & 44.696 & 43.043 & 46.174 & 47.217 \\
257           & 43.696 & 40.435 & 45.522 & 46.217 & 46.043 & 42.478 & 45     & 42.957 & 46.565 & 47.217 \\
258           & 43.783 & 41.217 & 45.435 & 46.739 & 46.043 & 42.739 & 44.739 & 42.87  & 46.435 & 47     \\
259           & 43.913 & 41.348 & 45.348 & 46.609 & 45.957 & 43.478 & 44.348 & 43.043 & 46.391 & 47.217 \\
260           & 43.957 & 41.217 & 45.087 & 46.652 & 46.13  & 43.522 & 44.435 & 43.043 & 46.739 & 47.217 \\
261           & 44.087 & 40.87  & 45.391 & 46.565 & 46.304 & 43.478 & 44.478 & 43     & 46.826 & 47.478 \\
262           & 44.087 & 41.391 & 45.696 & 46.478 & 46.13  & 43.652 & 44.435 & 43.174 & 46.87  & 47.261 \\
263           & 44.087 & 41.435 & 45.87  & 46.565 & 46.304 & 43.652 & 44.565 & 43     & 47.217 & 47.261 \\
264           & 44.826 & 41.435 & 46.087 & 47     & 46.304 & 43.652 & 44.87  & 43.217 & 47.043 & 47.652 \\
265           & 44.522 & 41.609 & 46.652 & 47.087 & 46.304 & 43.652 & 44.957 & 43.174 & 47.348 & 47.87  \\
266           & 44.739 & 41.957 & 46.609 & 47.261 & 46.304 & 43.913 & 44.783 & 43.304 & 47.087 & 47.913 \\
267           & 44.609 & 42.435 & 46.609 & 47.261 & 45.957 & 43.826 & 45.043 & 43.391 & 47.217 & 47.565 \\
268           & 44.565 & 42.217 & 46.652 & 47.304 & 46.348 & 43.696 & 45.391 & 43.391 & 47.609 & 48     \\
269           & 45.043 & 41.913 & 46.957 & 47.304 & 46.478 & 43.652 & 45.652 & 45.304 & 47.739 & 48.043 \\
270           & 45.522 & 41.739 & 47     & 47.435 & 46.565 & 43.652 & 45.565 & 45.304 & 47.522 & 48.087 \\
271           & 45.522 & 41.87  & 47.696 & 47.304 & 46.304 & 43.565 & 45.826 & 45.652 & 47.522 & 48.435 \\
272           & 45.348 & 42.217 & 47.609 & 47.565 & 46.565 & 43.348 & 45.913 & 45.696 & 47.391 & 48.348 \\
273           & 45.478 & 43     & 47.957 & 47.696 & 46.913 & 43.478 & 45.913 & 46     & 47.522 & 48.348 \\
274           & 45.478 & 42.913 & 47.913 & 47.87  & 46.826 & 43.391 & 46     & 45.826 & 47.957 & 48.217 \\
275           & 45.087 & 42.957 & 48.565 & 47.783 & 47.043 & 43.522 & 46.217 & 46     & 48.609 & 48.087 \\
276           & 45.261 & 43.13  & 48.696 & 48     & 47     & 44.478 & 46.87  & 45.957 & 48.435 & 48.522 \\
277           & 45.261 & 43.261 & 49.217 & 47.826 & 47     & 44.565 & 46.435 & 46.043 & 48.565 & 48.783 \\
278           & 45.478 & 43.217 & 49.261 & 48.652 & 47.174 & 44.696 & 46.478 & 45.783 & 48.565 & 48.913 \\
279           & 45.304 & 43.391 & 49.174 & 48.348 & 47.261 & 44.913 & 46.652 & 45.783 & 48.435 & 48.957 \\
280           & 45.435 & 43.478 & 49.304 & 48.522 & 47.435 & 44.783 & 46.609 & 45.565 & 48.435 & 48.652 \\
281           & 45.348 & 43.652 & 49.609 & 48.609 & 47.391 & 44.957 & 47.174 & 46     & 48.435 & 48.522 \\
282           & 45.87  & 43.652 & 49.652 & 48.913 & 47.609 & 45.304 & 47.217 & 45.783 & 48.739 & 49.174 \\
283           & 46.043 & 43.87  & 49.739 & 48.913 & 47.609 & 45.478 & 47.435 & 45.87  & 48.783 & 49.217 \\
284           & 45.783 & 44.478 & 49.87  & 48.957 & 47.826 & 45.391 & 47.652 & 46     & 48.739 & 49.478 \\
285           & 45.826 & 44.478 & 50.13  & 49.304 & 47.783 & 45.565 & 47.565 & 45.957 & 48.696 & 49.348 \\
286           & 45.957 & 44.913 & 50.609 & 49.348 & 47.783 & 45.391 & 47.87  & 45.826 & 48.826 & 49.348 \\
287           & 46.087 & 44.739 & 50.522 & 49.522 & 47.826 & 45.217 & 48.043 & 45.739 & 49.174 & 50.087 \\
288           & 46.13  & 45.043 & 50.739 & 49.826 & 47.783 & 45.304 & 48.087 & 45.87  & 49     & 50.261 \\
289           & 46.174 & 44.957 & 50.783 & 49.826 & 47.783 & 45.522 & 47.739 & 45.913 & 49.391 & 50.217 \\
290           & 46.391 & 46.87  & 50.609 & 50.13  & 47.783 & 45.609 & 47.696 & 46.783 & 49.391 & 50.652 \\
291           & 47.087 & 46.957 & 50.565 & 50.043 & 47.913 & 45.522 & 47.957 & 47.13  & 49.435 & 50.696 \\
292           & 47.261 & 46.652 & 50.826 & 50.217 & 48.043 & 45.522 & 48.435 & 47     & 49.478 & 50.522 \\
293           & 47.261 & 47.391 & 51.043 & 50.435 & 48.087 & 45.435 & 48.478 & 47.652 & 49.217 & 50.609 \\
294           & 47.261 & 48.043 & 50.913 & 50.565 & 48.174 & 46.043 & 48.261 & 47.565 & 49.217 & 50.174 \\
295           & 47.217 & 48.087 & 51.174 & 50.696 & 48.217 & 46.696 & 48.609 & 47.565 & 49.348 & 50.435 \\
296           & 47.957 & 48.304 & 51.087 & 50.652 & 48.217 & 47.043 & 48.522 & 47.783 & 49.739 & 50.435 \\
297           & 47.783 & 48.391 & 51     & 50.783 & 48.435 & 47.348 & 48.739 & 47.913 & 49.826 & 50.478 \\
298           & 48.391 & 48.565 & 51.043 & 51     & 48.957 & 47.391 & 48.739 & 48.087 & 49.652 & 50.348 \\
299           & 48.609 & 48.957 & 51.087 & 50.87  & 48.652 & 47.783 & 48.783 & 48     & 49.652 & 50.304 \\
300           & 48.652 & 49.043 & 51.174 & 51.348 & 48.739 & 49.391 & 49.261 & 47.913 & 49.696 & 50.217 \\
301           & 49     & 48.826 & 51.043 & 51.783 & 48.391 & 49.391 & 48.87  & 47.957 & 49.739 & 50.348 \\
302           & 49.348 & 49.087 & 51.348 & 51.87  & 48.652 & 49.565 & 49     & 48.043 & 49.913 & 50.565 \\
303           & 49.783 & 49.348 & 51.522 & 52.348 & 48.522 & 49.478 & 48.87  & 48.043 & 49.739 & 50.609 \\
304           & 50     & 49.304 & 52.043 & 52.261 & 48.652 & 49.478 & 48.826 & 48.087 & 49.739 & 50.478 \\
305           & 49.913 & 49.391 & 52     & 52.609 & 48.652 & 49.87  & 49.043 & 48.087 & 50.174 & 50.609 \\
306           & 49.913 & 49.13  & 51.739 & 52.304 & 48.826 & 49.87  & 49.13  & 48.348 & 50.174 & 50.565 \\
307           & 50.13  & 49     & 51.87  & 52.783 & 48.696 & 49.87  & 49.087 & 48.217 & 50.304 & 51.043 \\
308           & 50.304 & 49.13  & 52.478 & 52.478 & 48.87  & 49.957 & 49.174 & 48.217 & 50.783 & 50.957 \\
309           & 50.304 & 49.348 & 52.652 & 52.739 & 49     & 49.783 & 49.217 & 48.217 & 50.652 & 50.87  \\
310           & 50.261 & 49.826 & 52.348 & 52.826 & 48.957 & 50     & 49.13  & 48.261 & 50.696 & 51.217 \\
311           & 50.304 & 49.913 & 52.261 & 52.696 & 48.87  & 50.043 & 49.043 & 48.261 & 50.783 & 51.348 \\
312           & 50.609 & 49.87  & 52.304 & 52.783 & 48.696 & 50.522 & 49.435 & 48.435 & 50.652 & 51.348 \\
313           & 50.696 & 50.043 & 52.478 & 52.87  & 49     & 50.652 & 49.217 & 48.435 & 50.913 & 51.609 \\
314           & 51     & 50.261 & 52.652 & 53.261 & 48.522 & 50.652 & 49.261 & 49.304 & 50.87  & 51.826 \\
315           & 51.174 & 50.391 & 52.304 & 53.261 & 48.435 & 50.783 & 49.565 & 49.348 & 50.652 & 51.739 \\
316           & 51.435 & 50.261 & 52.391 & 53.739 & 48.652 & 50.826 & 49.304 & 49.783 & 50.565 & 51.696 \\
317           & 51.435 & 50.391 & 52.261 & 53.565 & 48.435 & 50.957 & 49.174 & 50.13  & 50.565 & 51.696 \\
318           & 51.652 & 50.304 & 52.217 & 53.609 & 49     & 51.087 & 49.957 & 50.261 & 50.478 & 51.652 \\
319           & 51.87  & 50.783 & 52.391 & 53.957 & 49.391 & 51.087 & 50.043 & 50.217 & 50.261 & 52.13  \\
320           & 52.174 & 50.913 & 52.826 & 54.348 & 49.609 & 51.217 & 50.261 & 50.261 & 50.304 & 52.043 \\
321           & 52.087 & 50.826 & 52.739 & 54.565 & 49.696 & 51.435 & 50.391 & 50.435 & 51     & 52     \\
322           & 52.087 & 51.043 & 52.826 & 54.652 & 50.217 & 51.391 & 50.261 & 50.522 & 50.696 & 52.13  \\
323           & 52.087 & 50.957 & 53.13  & 54.826 & 50.043 & 51.478 & 50.261 & 50.522 & 50.696 & 52.043 \\
324           & 52.174 & 50.957 & 53.217 & 54.87  & 50.043 & 51.696 & 50.087 & 50.609 & 51.174 & 52     \\
325           & 52.043 & 51.435 & 53     & 54.913 & 50.087 & 51.739 & 50.478 & 50.478 & 51.217 & 51.217 \\
326           & 52.13  & 51.652 & 53.522 & 55.217 & 49.957 & 52.174 & 50.435 & 50.435 & 51.174 & 51.217 \\
327           & 52.348 & 51.435 & 53.304 & 55.565 & 50.13  & 52.826 & 50.913 & 50.696 & 51.174 & 51.043 \\
328           & 52.391 & 51.696 & 53.348 & 55.217 & 50.13  & 53.174 & 51.304 & 50.913 & 51.391 & 50.826 \\
329           & 52.522 & 51.522 & 53.261 & 55.348 & 50.087 & 53.391 & 51.652 & 51.13  & 51.304 & 51.174 \\
330           & 52.435 & 52     & 53.261 & 55.435 & 50.174 & 53.565 & 52.043 & 51.174 & 51.261 & 51.087 \\
331           & 52.217 & 51.913 & 53.217 & 55.261 & 50.087 & 53.522 & 52.913 & 51.261 & 51.217 & 51.217 \\
332           & 52.174 & 52.217 & 53.261 & 55.261 & 50.522 & 53.565 & 53     & 51.478 & 51.391 & 51.739 \\
333           & 52.087 & 52.565 & 53.478 & 55.435 & 50.609 & 53.565 & 53     & 51.87  & 51.087 & 52.174 \\
334           & 52.348 & 52.609 & 53.522 & 55.261 & 50.957 & 53.565 & 52.957 & 51.913 & 51.13  & 52.435 \\
335           & 52.174 & 52.652 & 53.348 & 55.609 & 51     & 53.652 & 52.826 & 52.043 & 51.739 & 52.696 \\
336           & 52.087 & 53.043 & 53.391 & 55.478 & 51.043 & 54     & 53.261 & 52.043 & 51.478 & 52.609 \\
337           & 52.087 & 52.957 & 53.652 & 55.087 & 51.609 & 54.13  & 53.739 & 52     & 51.13  & 52.652 \\
338           & 52.087 & 52.957 & 53.783 & 55.13  & 51.478 & 54.391 & 54.304 & 52.087 & 51.609 & 53.13  \\
339           & 52.261 & 53.391 & 53.609 & 55.783 & 51.783 & 54.304 & 54.391 & 52.261 & 51.522 & 53.652 \\
340           & 52.304 & 53.087 & 53.435 & 55.609 & 51.652 & 54.348 & 54.217 & 52.783 & 51.826 & 53.696 \\
341           & 52.261 & 53.174 & 53.522 & 55.391 & 51.609 & 54.391 & 53.957 & 52.957 & 52.348 & 54.304 \\
342           & 52.13  & 53.174 & 53.304 & 55.565 & 51.652 & 54.478 & 54.304 & 53.261 & 52.391 & 54.348 \\
343           & 52.348 & 53.696 & 53.522 & 55.565 & 51.609 & 54.609 & 54.913 & 53.435 & 52.87  & 54.478 \\
344           & 52.478 & 53.913 & 53.522 & 55.609 & 51.609 & 54.348 & 55.043 & 53.652 & 52.957 & 54.391 \\
345           & 52.957 & 53.609 & 54.043 & 55.652 & 51.696 & 54.261 & 55.174 & 53.957 & 53.217 & 54.478 \\
346           & 53     & 53.609 & 53.913 & 55.957 & 52.087 & 53.913 & 55.304 & 54.174 & 53.174 & 54.391 \\
347           & 52.783 & 53.913 & 53.565 & 56     & 52.565 & 53.565 & 55.522 & 54.87  & 53.652 & 54.87  \\
348           & 52.783 & 53.913 & 53.826 & 56.217 & 52.217 & 54.13  & 55.696 & 55.13  & 53.913 & 54.696 \\
349           & 53.348 & 53.652 & 54.261 & 55.913 & 52.957 & 53.783 & 55.87  & 54.913 & 54     & 54.609 \\
350           & 53.087 & 53.522 & 54.739 & 55.913 & 52.261 & 53.652 & 55.826 & 54.783 & 53.957 & 54.652 \\
351           & 53.087 & 54.217 & 54.565 & 55.783 & 52.174 & 53.478 & 55.87  & 54.826 & 54.174 & 54.826 \\
352           & 53.348 & 54.13  & 54.522 & 55.957 & 52.304 & 53.609 & 55.826 & 54.913 & 54.652 & 54.696 \\
353           & 53.13  & 53.696 & 54.957 & 55.957 & 52.435 & 53.522 & 55.348 & 54.739 & 54.609 & 55.217 \\
354           & 52.696 & 53.565 & 55.13  & 55.739 & 52.565 & 53.217 & 55.783 & 54.739 & 54.565 & 55.391 \\
355           & 53.261 & 53.522 & 55.043 & 55.739 & 52.391 & 53.696 & 55.783 & 55.174 & 54.652 & 55.652 \\
356           & 53.304 & 53.565 & 54.957 & 56     & 52.739 & 53.957 & 55.435 & 55.522 & 54.739 & 55.522 \\
357           & 53.783 & 53.652 & 55.087 & 55.913 & 52.609 & 53.913 & 55.565 & 55.261 & 54.261 & 55.391 \\
358           & 53.783 & 54.217 & 55.043 & 55.783 & 52.522 & 54.174 & 56.087 & 55.261 & 54.565 & 55.739 \\
359           & 54.174 & 54.217 & 54.87  & 55.87  & 52.609 & 54.217 & 56     & 55.261 & 54.826 & 55.826 \\
360           & 54.13  & 54.217 & 55.087 & 56.087 & 52.609 & 54.652 & 56.261 & 55.391 & 54.87  & 55.696 \\
361           & 54.217 & 53.826 & 54.783 & 56.174 & 53.13  & 54.826 & 56.304 & 55.609 & 54.783 & 55.435 \\
362           & 54.087 & 53.739 & 55     & 56.522 & 53.13  & 54.478 & 56.217 & 55.652 & 54.957 & 55.565 \\
363           & 53.913 & 54     & 54.913 & 56.304 & 53     & 54.304 & 56.435 & 55.348 & 54.783 & 55.696 \\
364           & 53.87  & 53.913 & 54.913 & 56.261 & 53.261 & 54.261 & 56.826 & 55.348 & 54.565 & 55.957 \\
365           & 54.043 & 54.348 & 55.217 & 55.957 & 53.435 & 54.565 & 56.826 & 55.348 & 54.304 & 56.174 \\
366           & 54.087 & 54.652 & 55.174 & 55.565 & 53.739 & 54.304 & 57.261 & 55.217 & 54.609 & 55.957 \\
367           & 54.522 & 54.652 & 55.304 & 56.087 & 53.783 & 54.261 & 56.957 & 55.087 & 54.217 & 55.913 \\
368           & 54.696 & 54.913 & 55.261 & 56     & 54.435 & 54.565 & 57.087 & 55.478 & 54.304 & 56.087 \\
369           & 54.174 & 55.348 & 55.826 & 55.913 & 54.826 & 54.391 & 57.174 & 55.304 & 54     & 56     \\
370           & 54.522 & 54.87  & 55.913 & 55.957 & 54.696 & 54.522 & 57     & 55.565 & 54.043 & 55.87  \\
371           & 54.739 & 54.913 & 56.043 & 56.174 & 55     & 55.043 & 57.348 & 55.739 & 53.739 & 55.783 \\
372           & 55.043 & 54.696 & 55.913 & 56.696 & 55.087 & 54.522 & 57.435 & 55.478 & 53.652 & 55.652 \\
373           & 54.913 & 55     & 56.087 & 56.826 & 55.304 & 54.348 & 57.826 & 55.739 & 53.783 & 55.957 \\
374           & 54.826 & 55.739 & 56     & 56.783 & 55.391 & 54.391 & 57.696 & 55.826 & 54.087 & 56.087 \\
375           & 55.174 & 55.609 & 55.913 & 56.565 & 55.478 & 54.652 & 57.913 & 55.522 & 54.174 & 56.435 \\
376           & 55.348 & 55.783 & 55.957 & 56.261 & 55.565 & 54.391 & 57.739 & 55.391 & 54.348 & 56.391 \\
377           & 55.391 & 55.957 & 55.957 & 56.652 & 55.522 & 53.913 & 58.043 & 55.435 & 54.348 & 56.609 \\
378           & 55.783 & 55.609 & 56     & 56.609 & 55.435 & 53.783 & 58.304 & 54.652 & 54.304 & 56.739 \\
379           & 55.739 & 55.783 & 55.826 & 56.478 & 55.609 & 53.739 & 58.435 & 55.043 & 54.391 & 57.13  \\
380           & 55.435 & 55.435 & 56.043 & 56.087 & 55.478 & 53.783 & 58.565 & 54.913 & 54.522 & 57.087 \\
381           & 55.087 & 55.304 & 56.043 & 56.13  & 55.739 & 54.087 & 58.609 & 55.217 & 54.913 & 57.304 \\
382           & 55.565 & 55.478 & 56     & 56     & 55.609 & 54.609 & 58.783 & 55.609 & 54.826 & 57.391 \\
383           & 55.174 & 55.652 & 56.261 & 56.217 & 55.304 & 55     & 58.913 & 55.652 & 55.261 & 57.13  \\
384           & 55     & 55.826 & 56.304 & 55.957 & 55.478 & 54.87  & 58.826 & 55.435 & 54.783 & 57.348 \\
385           & 55     & 56.565 & 56.261 & 55.913 & 55.826 & 54.609 & 59.043 & 55.478 & 55.13  & 57.043 \\
386           & 55.087 & 55.913 & 56.13  & 55.957 & 55.304 & 54.652 & 59.13  & 55.652 & 55.217 & 57.174 \\
387           & 55.826 & 56.304 & 56.261 & 56.043 & 55     & 55.261 & 58.913 & 55.391 & 55.478 & 57.174 \\
388           & 56.087 & 56.261 & 56.13  & 56.174 & 55     & 55.13  & 58.87  & 55.435 & 55.826 & 57.304 \\
389           & 56.217 & 56.261 & 56.043 & 56.217 & 55.043 & 55.391 & 59     & 55.609 & 55.522 & 57.696 \\
390           & 56.217 & 56.174 & 55.696 & 56.435 & 54.957 & 55.348 & 58.913 & 55.783 & 55.478 & 57.478 \\
391           & 56.217 & 56.304 & 56.087 & 56.348 & 54.957 & 55.522 & 58.609 & 55.87  & 55.696 & 57.609 \\
\bottomrule\end{longtable}
\normalsize
