# Supplementary material for: Rehearsal-Free Continual Learning over Small Non-I.I.D. Batches
Source: arXiv:1907.03799 source file (2020-04-21)
Supplement: Supplementary file 8 [file 391_AR1_BN.tex]

\subsection{AR1* (with Batch Normalization), NICv2 - 391}
\fontsize{8}{11}\selectfont
\begin{longtable}[c]{rgrgrgrgrgr}
\hline
Batch & Run 0  & Run 1  & Run 2  & Run 3  & Run 4  & Run 5  & Run 6  & Run 7  & Run 8  & Run 9  \\ \hline
\endfirsthead
\endhead
0     & 8.304  & 8.304  & 8.304  & 8.304  & 8.304  & 8.304  & 8.304  & 8.304  & 8.304  & 8.304  \\
1     & 14.391 & 14.391 & 14.391 & 14.391 & 14.391 & 14.391 & 14.391 & 14.391 & 14.391 & 14.391 \\
2     & 14.348 & 14.348 & 14.957 & 14.652 & 15.13  & 14.652 & 15.087 & 15.13  & 14.87  & 14.783 \\
3     & 14.13  & 14.826 & 15.391 & 15     & 15.348 & 14.826 & 15.174 & 15.348 & 14.913 & 14.957 \\
4     & 13.826 & 14.957 & 15.609 & 15.304 & 15.478 & 15.217 & 15.565 & 15.652 & 15.043 & 15.217 \\
5     & 14.13  & 15.087 & 15.478 & 15.304 & 15.565 & 15.13  & 16.217 & 16.087 & 15.174 & 15.783 \\
6     & 14.304 & 15.13  & 15.261 & 15.087 & 15.391 & 15.174 & 16.217 & 15.913 & 14.957 & 16     \\
7     & 14.565 & 14.913 & 15.217 & 15.348 & 15.348 & 15.087 & 16.304 & 16     & 15     & 16.087 \\
8     & 14.348 & 15     & 15.435 & 15.739 & 16.043 & 15.304 & 16.348 & 16.261 & 15.261 & 15.783 \\
9     & 14.783 & 14.957 & 15.304 & 15.826 & 15.87  & 15.043 & 16.391 & 16.304 & 15.478 & 15.478 \\
10    & 14.826 & 14.87  & 15.261 & 15.652 & 15.826 & 14.783 & 16.609 & 16.174 & 15.391 & 15.565 \\
11    & 14.565 & 14.87  & 15.609 & 15.565 & 15.826 & 14.87  & 16.565 & 15.87  & 15.13  & 15.609 \\
12    & 14.609 & 15     & 16     & 15.522 & 15.913 & 15.043 & 16.652 & 15.652 & 14.913 & 15.739 \\
13    & 14.696 & 15.217 & 16.217 & 15.478 & 16.217 & 15.087 & 16.609 & 15.87  & 15.609 & 15.783 \\
14    & 14.913 & 15.087 & 16.304 & 15.435 & 16.261 & 15.13  & 16.652 & 15.696 & 15.783 & 15.652 \\
15    & 14.783 & 15.217 & 16.435 & 15.304 & 16     & 14.826 & 16.435 & 15.696 & 15.565 & 15.957 \\
16    & 15.348 & 15.13  & 16.391 & 15.565 & 16     & 14.826 & 16.087 & 15.739 & 15.609 & 16.087 \\
17    & 15     & 15.217 & 16.565 & 15.522 & 15.957 & 14.913 & 16.565 & 15.783 & 15.739 & 16     \\
18    & 14.913 & 15.304 & 16     & 15.391 & 16     & 14.957 & 16.478 & 15.522 & 15.652 & 16.087 \\
19    & 14.826 & 15.348 & 16.087 & 15.391 & 15.783 & 14.913 & 16.304 & 15.739 & 15.696 & 16     \\
20    & 14.652 & 15.174 & 15.87  & 15.043 & 16.043 & 14.957 & 16.261 & 16.217 & 15.609 & 16     \\
21    & 14.913 & 15.217 & 16.174 & 15.174 & 16.087 & 14.696 & 16.087 & 16.261 & 15.565 & 16.043 \\
22    & 14.696 & 15     & 16.304 & 15.087 & 15.957 & 14.609 & 16.13  & 16.13  & 15.435 & 15.783 \\
23    & 14.783 & 15.304 & 16.522 & 14.87  & 15.957 & 14.609 & 15.739 & 16.391 & 15.565 & 15.739 \\
24    & 15     & 15.304 & 16.565 & 15.13  & 16.043 & 14.478 & 15.652 & 16.391 & 15.391 & 15.696 \\
25    & 14.652 & 15.435 & 16.565 & 15.043 & 16.348 & 14.739 & 15.565 & 16.565 & 15.609 & 15.435 \\
26    & 14.913 & 15.217 & 16.174 & 15.087 & 16.174 & 14.739 & 15.609 & 16.522 & 15.652 & 15.478 \\
27    & 15.043 & 15.391 & 15.957 & 15.13  & 16.13  & 14.696 & 15.478 & 16.609 & 15.696 & 15.478 \\
28    & 15.087 & 15.348 & 15.696 & 15.13  & 16.261 & 14.565 & 15.696 & 16.609 & 15.696 & 15.609 \\
29    & 15.087 & 15.174 & 15.522 & 15.174 & 16.435 & 14.739 & 15.261 & 16.522 & 15.435 & 15.783 \\
30    & 15.043 & 15.217 & 15.565 & 15.348 & 16.522 & 14.652 & 15.217 & 16.304 & 15.348 & 15.87  \\
31    & 15.217 & 15.087 & 15.565 & 15.348 & 16.739 & 14.826 & 15.174 & 16.261 & 15.391 & 15.652 \\
32    & 15.217 & 15.261 & 15.522 & 15.391 & 16.565 & 14.913 & 15.348 & 16.609 & 15.261 & 15.435 \\
33    & 15.174 & 15.261 & 15.522 & 15.435 & 16.652 & 15.13  & 15.261 & 16.609 & 15.391 & 15.522 \\
34    & 15.043 & 15.174 & 15.783 & 15.391 & 16.478 & 15.13  & 15.304 & 16.696 & 15.348 & 15.435 \\
35    & 15.174 & 14.957 & 15.87  & 15.565 & 16.739 & 15.13  & 15.391 & 16.391 & 15.391 & 15.478 \\
36    & 15.478 & 14.913 & 15.957 & 15.565 & 16.696 & 15.217 & 15.304 & 16.565 & 15.391 & 15.565 \\
37    & 15.565 & 14.913 & 15.913 & 15.565 & 16.652 & 15.261 & 15.304 & 16.739 & 15.261 & 15.478 \\
38    & 15.826 & 15.087 & 15.913 & 15.478 & 16.565 & 15.435 & 15.435 & 16.522 & 15.13  & 15.522 \\
39    & 15.391 & 14.957 & 16     & 15.478 & 16.217 & 15.435 & 15.522 & 16.304 & 15.087 & 15.522 \\
40    & 15.391 & 15.043 & 15.913 & 15.522 & 15.87  & 15.435 & 15.522 & 16.261 & 15     & 15.565 \\
41    & 15.565 & 15.348 & 16.043 & 15.739 & 15.783 & 15.435 & 15.652 & 16.261 & 15     & 15.435 \\
42    & 15.565 & 15.304 & 15.957 & 15.696 & 15.826 & 15.522 & 15.522 & 16.391 & 14.957 & 15.565 \\
43    & 15.217 & 15.348 & 15.913 & 15.826 & 15.913 & 15.609 & 15.652 & 16.304 & 14.783 & 15.478 \\
44    & 15.478 & 15.087 & 15.826 & 15.739 & 15.913 & 15.522 & 15.739 & 16.304 & 14.652 & 15.522 \\
45    & 15.217 & 15.087 & 16     & 15.826 & 15.826 & 15.435 & 15.87  & 16.261 & 14.696 & 15.478 \\
46    & 15.261 & 14.913 & 15.957 & 15.739 & 15.957 & 15.348 & 15.739 & 16.087 & 14.609 & 15.522 \\
47    & 15.696 & 14.913 & 16.217 & 15.783 & 15.87  & 15.391 & 15.435 & 16.174 & 14.565 & 15.478 \\
48    & 15.478 & 14.435 & 16     & 15.826 & 15.826 & 15.478 & 15.391 & 16.087 & 14.565 & 15.435 \\
49    & 15.217 & 14.348 & 16.174 & 15.783 & 15.87  & 15.391 & 15.391 & 16.174 & 14.348 & 15.478 \\
50    & 15.348 & 14.261 & 16.261 & 15.826 & 15.87  & 15.609 & 15.435 & 16.174 & 14.261 & 15.522 \\
51    & 15.478 & 14.304 & 16.217 & 15.87  & 15.826 & 15.609 & 15.348 & 15.913 & 14.174 & 15.565 \\
52    & 15.739 & 14.348 & 16.217 & 15.913 & 15.826 & 15.609 & 15.391 & 16     & 14.348 & 15.783 \\
53    & 15.565 & 14.783 & 16     & 16.043 & 15.913 & 15.565 & 15.478 & 15.87  & 14.304 & 15.783 \\
54    & 15.609 & 14.913 & 16     & 16.043 & 15.913 & 15.565 & 15.478 & 15.826 & 14.478 & 15.391 \\
55    & 15.739 & 15.043 & 16.043 & 15.913 & 15.913 & 15.348 & 15.565 & 16.043 & 14.739 & 15.348 \\
56    & 15.826 & 15.087 & 16.13  & 15.957 & 15.87  & 15.348 & 15.522 & 15.826 & 14.826 & 15.348 \\
57    & 15.783 & 14.913 & 16.087 & 15.783 & 15.826 & 15.304 & 15.435 & 15.739 & 14.87  & 15.435 \\
58    & 15.739 & 15     & 16.217 & 15.783 & 15.957 & 15.261 & 15.391 & 15.783 & 14.739 & 15.478 \\
59    & 15.739 & 14.87  & 16.217 & 15.826 & 15.913 & 15.304 & 15.435 & 15.826 & 14.87  & 15.522 \\
60    & 15.696 & 14.783 & 16.304 & 15.783 & 15.913 & 15.435 & 15.348 & 15.783 & 14.87  & 15.478 \\
61    & 15.696 & 14.87  & 16.391 & 15.957 & 15.696 & 15.304 & 15.435 & 15.783 & 14.783 & 15.348 \\
62    & 15.652 & 14.783 & 16.217 & 16.348 & 15.87  & 15.435 & 15.391 & 15.826 & 14.87  & 15.261 \\
63    & 15.739 & 14.913 & 16.087 & 16.348 & 15.826 & 15.435 & 15.609 & 15.609 & 14.826 & 15.478 \\
64    & 15.783 & 14.696 & 16.043 & 16.348 & 15.826 & 15.391 & 15.609 & 15.652 & 15     & 15.522 \\
65    & 16     & 14.696 & 16.087 & 16     & 15.739 & 15.348 & 15.522 & 15.87  & 15     & 15.478 \\
66    & 16.13  & 14.609 & 16.261 & 15.957 & 15.739 & 15.348 & 15.609 & 15.87  & 14.957 & 15.696 \\
67    & 15.826 & 15.174 & 16.348 & 15.957 & 15.783 & 15.261 & 15.565 & 16.13  & 14.957 & 15.87  \\
68    & 16.13  & 15.087 & 16.565 & 16.348 & 15.783 & 15.478 & 15.826 & 16.13  & 15     & 15.87  \\
69    & 16.13  & 15.304 & 16.522 & 16.435 & 15.783 & 15.739 & 15.739 & 16.217 & 15.087 & 15.957 \\
70    & 16.043 & 15.391 & 16.565 & 16.435 & 15.957 & 15.87  & 15.87  & 16.043 & 15.217 & 15.783 \\
71    & 16     & 15.348 & 16.522 & 16.261 & 15.957 & 15.826 & 15.609 & 16.174 & 14.957 & 15.826 \\
72    & 16.043 & 15.522 & 16.522 & 15.87  & 15.913 & 15.783 & 15.609 & 16.174 & 14.957 & 16     \\
73    & 16     & 15.478 & 16.522 & 15.87  & 16     & 15.739 & 15.261 & 15.957 & 14.826 & 15.826 \\
74    & 16.13  & 15.478 & 16.522 & 15.913 & 15.826 & 15.739 & 15.217 & 16.043 & 14.739 & 15.87  \\
75    & 16.043 & 15.652 & 16.478 & 15.957 & 15.87  & 15.696 & 15.174 & 15.957 & 14.783 & 15.826 \\
76    & 16     & 15.652 & 16.478 & 16.043 & 15.913 & 15.565 & 15.304 & 15.957 & 14.826 & 15.826 \\
77    & 16.348 & 15.696 & 16.478 & 15.957 & 15.826 & 15.696 & 15.174 & 16     & 14.87  & 15.783 \\
78    & 16.261 & 15.522 & 16.478 & 16     & 15.826 & 15.696 & 15.217 & 16.087 & 14.783 & 15.783 \\
79    & 16.217 & 15.609 & 16.478 & 16     & 15.826 & 15.696 & 15.435 & 16     & 14.783 & 15.826 \\
80    & 16.261 & 15.696 & 16.391 & 15.913 & 15.652 & 15.826 & 15.391 & 15.957 & 14.87  & 15.826 \\
81    & 16.261 & 15.696 & 16.391 & 15.913 & 15.696 & 15.783 & 15.348 & 15.957 & 14.87  & 15.826 \\
82    & 16.348 & 15.739 & 16.391 & 15.913 & 15.739 & 15.783 & 15.304 & 15.87  & 15.043 & 15.87  \\
83    & 16.261 & 15.652 & 16.391 & 15.783 & 15.696 & 15.739 & 15.348 & 15.87  & 15     & 15.87  \\
84    & 16.261 & 15.696 & 16.217 & 15.87  & 15.652 & 15.783 & 15.522 & 15.826 & 15.13  & 15.87  \\
85    & 16.261 & 15.565 & 16.261 & 15.783 & 15.652 & 15.652 & 15.478 & 15.783 & 15.217 & 15.913 \\
86    & 16.217 & 15.609 & 16.261 & 15.739 & 15.565 & 15.739 & 15.435 & 15.783 & 15.13  & 15.913 \\
87    & 16.261 & 15.739 & 16.348 & 15.826 & 15.478 & 15.783 & 15.435 & 15.87  & 15.13  & 15.87  \\
88    & 16.13  & 15.696 & 16.609 & 15.739 & 15.522 & 15.739 & 15.739 & 15.87  & 15.174 & 15.826 \\
89    & 15.826 & 15.826 & 16.565 & 15.87  & 15.435 & 15.739 & 15.609 & 15.783 & 15.174 & 15.826 \\
90    & 16     & 15.913 & 16.522 & 15.826 & 15.435 & 15.696 & 15.652 & 15.739 & 15.087 & 15.739 \\
91    & 16     & 15.913 & 16.435 & 15.87  & 15.391 & 15.609 & 15.826 & 16.043 & 15.13  & 15.739 \\
92    & 16.043 & 16     & 16.522 & 15.913 & 15.435 & 15.435 & 15.783 & 15.913 & 15.13  & 15.739 \\
93    & 16.043 & 15.957 & 16.565 & 15.87  & 15.391 & 15.391 & 15.87  & 15.696 & 15.087 & 15.783 \\
94    & 16.174 & 15.957 & 16.391 & 15.913 & 15.478 & 15.478 & 15.565 & 15.652 & 15.087 & 15.826 \\
95    & 16.217 & 15.783 & 16.478 & 15.957 & 15.565 & 15.522 & 15.565 & 16     & 15.13  & 15.783 \\
96    & 16.217 & 15.783 & 16.478 & 15.739 & 15.565 & 15.609 & 15.391 & 15.957 & 15.261 & 15.783 \\
97    & 16.261 & 15.565 & 16.478 & 15.87  & 15.522 & 15.609 & 15.391 & 16.087 & 15.304 & 16.087 \\
98    & 16.174 & 15.652 & 16.565 & 15.739 & 15.522 & 15.652 & 15.348 & 16.087 & 15.13  & 16.043 \\
99    & 16.217 & 15.783 & 16.565 & 15.696 & 15.522 & 15.652 & 15.348 & 16.043 & 15.261 & 16.043 \\
100   & 16.174 & 15.826 & 16.261 & 15.696 & 15.783 & 15.696 & 15.304 & 16.13  & 15.304 & 15.913 \\
101   & 16.174 & 15.87  & 16.348 & 15.696 & 15.609 & 15.652 & 15.348 & 16.087 & 15.13  & 16.087 \\
102   & 16.217 & 15.826 & 16.261 & 15.652 & 15.652 & 15.609 & 15.304 & 16.13  & 15.348 & 16.087 \\
103   & 16.13  & 15.783 & 16.217 & 15.696 & 15.609 & 15.565 & 15.304 & 16.261 & 15.174 & 16     \\
104   & 16.261 & 15.87  & 16.217 & 15.609 & 15.652 & 15.565 & 15.348 & 16.261 & 15.348 & 16.087 \\
105   & 16.13  & 15.783 & 16.217 & 15.652 & 15.739 & 15.565 & 15.435 & 16.391 & 15.261 & 15.957 \\
106   & 16.13  & 16.087 & 16.261 & 15.739 & 15.652 & 15.565 & 15.217 & 16.304 & 15.087 & 15.913 \\
107   & 16.13  & 16.13  & 16.174 & 15.696 & 15.609 & 15.565 & 15.391 & 16.261 & 15.087 & 15.913 \\
108   & 16.13  & 16.174 & 16.043 & 15.739 & 15.565 & 15.957 & 15.391 & 16.217 & 15.13  & 16     \\
109   & 16.174 & 16.174 & 16.043 & 15.696 & 15.652 & 15.913 & 15.435 & 16.261 & 15.13  & 16.043 \\
110   & 16.13  & 16     & 16     & 15.739 & 15.609 & 15.957 & 15.391 & 16.217 & 15.174 & 16.087 \\
111   & 16.174 & 16.043 & 16.043 & 15.783 & 15.609 & 15.87  & 15.565 & 16.261 & 15.087 & 16.174 \\
112   & 16.13  & 16.043 & 16.043 & 15.739 & 15.565 & 15.783 & 15.565 & 16.304 & 15.087 & 16     \\
113   & 16.174 & 16     & 16.13  & 15.696 & 15.609 & 15.783 & 15.565 & 16.304 & 15.043 & 15.957 \\
114   & 16     & 16.043 & 16.087 & 15.739 & 15.652 & 15.739 & 15.522 & 16.304 & 15.043 & 16.087 \\
115   & 16.13  & 15.957 & 16.087 & 15.783 & 15.609 & 15.652 & 15.391 & 16.391 & 15.043 & 16.13  \\
116   & 16.13  & 15.87  & 16.043 & 15.609 & 15.609 & 15.739 & 15.435 & 16.261 & 15.087 & 16.043 \\
117   & 16.087 & 15.913 & 16     & 15.696 & 15.609 & 15.87  & 15.783 & 16.174 & 15.043 & 16.13  \\
118   & 16.087 & 15.913 & 15.913 & 15.696 & 15.609 & 15.913 & 15.783 & 16.261 & 15     & 16.174 \\
119   & 16.043 & 15.957 & 15.913 & 15.696 & 15.652 & 15.783 & 15.696 & 16.304 & 15.043 & 16.174 \\
120   & 16.087 & 16.043 & 16.087 & 15.696 & 15.652 & 15.696 & 15.783 & 16.261 & 15.13  & 16.043 \\
121   & 16.043 & 15.826 & 16.043 & 15.739 & 15.565 & 15.696 & 15.783 & 16.261 & 15.217 & 15.913 \\
122   & 16.087 & 16     & 16.13  & 15.783 & 15.739 & 15.652 & 15.87  & 16.217 & 15.261 & 16     \\
123   & 16.043 & 15.913 & 16.13  & 15.87  & 15.739 & 15.609 & 15.739 & 16.174 & 15.304 & 16.043 \\
124   & 16     & 15.87  & 16.087 & 15.826 & 15.609 & 15.652 & 15.696 & 16.217 & 15.304 & 16.13  \\
125   & 16.087 & 15.913 & 16.13  & 15.783 & 15.391 & 15.609 & 15.652 & 16.348 & 15.261 & 16.13  \\
126   & 16.043 & 15.87  & 16.043 & 15.783 & 15.565 & 15.696 & 15.826 & 16.348 & 15.217 & 16.261 \\
127   & 15.957 & 15.913 & 16     & 15.652 & 15.478 & 15.696 & 15.826 & 16.391 & 15.304 & 16.217 \\
128   & 15.913 & 15.913 & 16     & 15.783 & 15.304 & 15.565 & 15.783 & 16.391 & 15.304 & 16.261 \\
129   & 16.087 & 15.957 & 16     & 15.783 & 15.304 & 15.522 & 15.783 & 16.304 & 15.261 & 16.13  \\
130   & 16.217 & 15.957 & 16.043 & 15.87  & 15.261 & 15.609 & 15.739 & 16.348 & 15.261 & 16.087 \\
131   & 16.217 & 15.913 & 16     & 15.783 & 15.174 & 15.478 & 15.739 & 16.348 & 15.261 & 15.957 \\
132   & 16.217 & 15.826 & 16     & 15.826 & 15.304 & 15.565 & 15.739 & 16.391 & 15.478 & 16     \\
133   & 16.174 & 15.783 & 16.087 & 15.826 & 15.304 & 15.609 & 15.826 & 16.391 & 15.478 & 15.87  \\
134   & 16.217 & 15.87  & 16.043 & 15.957 & 15.217 & 15.609 & 15.783 & 16.304 & 15.609 & 15.826 \\
135   & 16.13  & 15.783 & 16.174 & 15.913 & 15.304 & 15.522 & 15.522 & 16.435 & 15.783 & 15.87  \\
136   & 16     & 15.913 & 16.087 & 15.87  & 15.261 & 15.522 & 15.652 & 16.391 & 15.696 & 15.957 \\
137   & 16.043 & 15.913 & 16     & 15.87  & 15.174 & 15.478 & 15.652 & 16.391 & 15.696 & 15.913 \\
138   & 16.087 & 16.087 & 16     & 15.826 & 15.13  & 15.261 & 15.565 & 16.304 & 15.696 & 15.826 \\
139   & 16.043 & 16.043 & 16.043 & 15.826 & 15.217 & 15.348 & 15.478 & 16.261 & 15.652 & 15.739 \\
140   & 16.13  & 16.087 & 16.13  & 15.826 & 15.304 & 15.174 & 15.435 & 16.174 & 15.739 & 15.652 \\
141   & 16.348 & 16     & 16.087 & 15.609 & 15.304 & 15.348 & 15.391 & 16.174 & 15.696 & 15.696 \\
142   & 16.217 & 16.043 & 16.174 & 15.565 & 15.261 & 15.435 & 15.522 & 16.391 & 15.696 & 15.652 \\
143   & 16.217 & 15.957 & 16.174 & 15.522 & 15.261 & 15.348 & 15.609 & 16.304 & 15.522 & 15.652 \\
144   & 16.217 & 16     & 16.217 & 15.522 & 15.174 & 15.348 & 15.609 & 16.217 & 15.391 & 15.652 \\
145   & 16.217 & 16.087 & 16.261 & 15.565 & 15.217 & 15.304 & 15.609 & 16.304 & 15.261 & 15.609 \\
146   & 16.174 & 16.13  & 16.304 & 15.565 & 15.13  & 15.348 & 15.652 & 16.217 & 15.174 & 15.696 \\
147   & 16.174 & 16.217 & 16.391 & 15.696 & 15.261 & 15.391 & 15.478 & 16.261 & 15.435 & 15.739 \\
148   & 16.13  & 16.174 & 16.391 & 15.652 & 15.304 & 15.435 & 15.478 & 16.174 & 15.261 & 15.913 \\
149   & 16.217 & 16     & 16.435 & 15.652 & 15.348 & 15.348 & 15.565 & 16.174 & 15.217 & 15.957 \\
150   & 16.304 & 16.043 & 16.348 & 15.652 & 15.522 & 15.435 & 15.435 & 16.087 & 15.304 & 15.913 \\
151   & 16.304 & 16     & 16.261 & 15.739 & 15.522 & 15.435 & 15.435 & 16.261 & 15.217 & 15.783 \\
152   & 16.261 & 16     & 16.087 & 15.739 & 15.565 & 15.391 & 15.565 & 16.174 & 15.217 & 15.826 \\
153   & 16.174 & 16.043 & 16.043 & 15.783 & 15.609 & 15.348 & 15.565 & 16.087 & 15.348 & 15.957 \\
154   & 16.174 & 16.043 & 16.043 & 15.783 & 15.348 & 15.348 & 15.565 & 16     & 15.522 & 15.913 \\
155   & 16.174 & 16     & 16.043 & 16     & 15.391 & 15.391 & 15.522 & 16     & 15.522 & 15.87  \\
156   & 16.217 & 15.957 & 16     & 15.913 & 15.565 & 15.391 & 15.522 & 16     & 15.522 & 15.957 \\
157   & 16.13  & 15.826 & 16.087 & 15.913 & 15.652 & 15.391 & 15.522 & 16.087 & 15.652 & 16.087 \\
158   & 16.13  & 15.913 & 16.043 & 15.87  & 15.565 & 15.348 & 15.522 & 16.174 & 15.565 & 16.087 \\
159   & 16     & 15.913 & 16.043 & 15.913 & 15.609 & 15.391 & 15.522 & 16.174 & 15.696 & 16.087 \\
160   & 15.87  & 15.87  & 16.043 & 15.913 & 15.652 & 15.435 & 15.522 & 16.217 & 15.696 & 16.043 \\
161   & 15.957 & 15.87  & 16.087 & 15.957 & 15.652 & 15.478 & 15.522 & 16.13  & 15.783 & 15.913 \\
162   & 15.913 & 15.87  & 16.043 & 15.913 & 15.652 & 15.478 & 15.522 & 16.217 & 15.739 & 15.957 \\
163   & 15.913 & 15.87  & 16     & 15.913 & 15.652 & 15.217 & 15.522 & 16.304 & 15.696 & 15.957 \\
164   & 15.913 & 15.87  & 16.087 & 15.913 & 15.652 & 15.174 & 15.522 & 16.261 & 15.696 & 15.913 \\
165   & 15.913 & 15.87  & 16.043 & 15.913 & 15.609 & 15.174 & 15.478 & 16.261 & 15.652 & 16     \\
166   & 15.87  & 15.87  & 16.174 & 15.913 & 15.652 & 15.217 & 15.609 & 16.261 & 15.652 & 15.87  \\
167   & 15.913 & 15.913 & 16.174 & 15.87  & 15.652 & 15.609 & 15.565 & 16.304 & 15.696 & 15.957 \\
168   & 15.913 & 15.957 & 16.174 & 15.826 & 15.696 & 15.565 & 15.652 & 16.13  & 15.696 & 15.957 \\
169   & 15.913 & 15.913 & 16.174 & 15.913 & 15.696 & 15.522 & 15.609 & 16.217 & 15.696 & 16.043 \\
170   & 15.913 & 15.87  & 16.174 & 15.696 & 15.783 & 15.826 & 15.609 & 16.13  & 15.783 & 16.087 \\
171   & 15.957 & 15.913 & 16.087 & 15.826 & 15.652 & 15.696 & 15.609 & 15.957 & 15.783 & 16.087 \\
172   & 15.87  & 15.913 & 16.087 & 15.826 & 15.696 & 15.696 & 15.609 & 16.043 & 15.913 & 16.087 \\
173   & 15.913 & 15.87  & 16.13  & 15.826 & 15.652 & 15.826 & 15.652 & 15.957 & 15.826 & 16     \\
174   & 15.957 & 15.826 & 16     & 15.87  & 15.696 & 15.609 & 15.609 & 15.913 & 15.739 & 16.087 \\
175   & 15.957 & 15.913 & 16     & 15.826 & 15.652 & 15.783 & 15.609 & 15.957 & 15.739 & 16.043 \\
176   & 15.957 & 15.913 & 16.043 & 15.826 & 15.609 & 15.739 & 15.739 & 15.913 & 15.783 & 16     \\
177   & 15.957 & 15.913 & 15.957 & 15.826 & 15.609 & 15.783 & 15.739 & 15.957 & 15.739 & 16.087 \\
178   & 15.957 & 15.913 & 16     & 15.826 & 15.609 & 15.783 & 15.783 & 16.043 & 15.826 & 16.087 \\
179   & 16.087 & 15.913 & 16.043 & 15.783 & 15.652 & 15.609 & 15.826 & 16.043 & 15.739 & 16.13  \\
180   & 16.13  & 15.957 & 15.913 & 15.826 & 15.652 & 15.696 & 15.826 & 16.087 & 15.826 & 16.087 \\
181   & 16.217 & 15.913 & 16.174 & 15.87  & 15.696 & 15.783 & 15.739 & 16.13  & 15.826 & 16.043 \\
182   & 16.217 & 15.826 & 16.087 & 15.826 & 15.696 & 15.652 & 15.826 & 16.087 & 15.826 & 15.957 \\
183   & 16.217 & 15.826 & 16.043 & 15.87  & 16.087 & 15.696 & 15.87  & 16.174 & 15.826 & 15.957 \\
184   & 16.174 & 15.913 & 16.174 & 15.826 & 16.043 & 15.652 & 15.739 & 16.043 & 15.826 & 15.957 \\
185   & 16.217 & 15.826 & 16.174 & 15.87  & 16.043 & 15.652 & 15.739 & 16     & 15.826 & 15.826 \\
186   & 16.174 & 15.826 & 16.174 & 15.87  & 16.174 & 15.696 & 15.739 & 15.957 & 15.87  & 15.87  \\
187   & 16.13  & 15.87  & 16.043 & 15.957 & 16.261 & 15.652 & 15.739 & 15.913 & 15.957 & 15.87  \\
188   & 16.174 & 15.913 & 16     & 15.826 & 16.174 & 15.652 & 15.739 & 15.957 & 15.913 & 15.87  \\
189   & 16.174 & 15.826 & 16.043 & 15.913 & 16     & 15.652 & 15.739 & 15.957 & 15.783 & 15.87  \\
190   & 16.261 & 15.87  & 16.13  & 15.913 & 16.043 & 15.652 & 15.739 & 15.957 & 15.87  & 15.826 \\
191   & 16.304 & 15.87  & 16.043 & 15.87  & 16.13  & 15.696 & 15.826 & 15.957 & 15.957 & 15.826 \\
192   & 16.304 & 15.913 & 16.043 & 15.913 & 16.087 & 15.609 & 15.783 & 15.913 & 16     & 15.826 \\
193   & 16.391 & 15.913 & 16.043 & 15.87  & 16.13  & 15.696 & 15.652 & 15.957 & 16     & 15.826 \\
194   & 16.391 & 15.957 & 16.087 & 15.913 & 16.087 & 15.609 & 15.652 & 15.957 & 16     & 15.826 \\
195   & 16.391 & 15.957 & 16     & 15.913 & 16.174 & 15.696 & 15.522 & 15.957 & 16.043 & 15.826 \\
196   & 16.348 & 15.826 & 16.043 & 15.957 & 16.043 & 15.696 & 15.609 & 16     & 16     & 15.87  \\
197   & 16.348 & 15.783 & 16.043 & 16     & 16.043 & 15.565 & 15.652 & 16.043 & 16     & 15.783 \\
198   & 16.391 & 15.826 & 15.957 & 16     & 16.087 & 15.609 & 15.696 & 16.087 & 15.87  & 15.913 \\
199   & 16.348 & 15.87  & 15.739 & 16     & 16.043 & 15.652 & 15.739 & 15.957 & 15.826 & 16.13  \\
200   & 16.304 & 15.87  & 15.783 & 15.957 & 15.957 & 15.609 & 15.739 & 16     & 16.043 & 16.087 \\
201   & 16.304 & 15.826 & 15.913 & 16     & 16     & 15.522 & 15.739 & 16.043 & 16     & 16.174 \\
202   & 16.261 & 15.783 & 15.87  & 16.087 & 16     & 15.609 & 15.739 & 16.043 & 15.913 & 16.217 \\
203   & 16.174 & 15.783 & 15.957 & 16.043 & 16.043 & 15.565 & 15.696 & 15.957 & 15.783 & 16.217 \\
204   & 16.217 & 15.826 & 15.913 & 16.043 & 16.043 & 15.522 & 15.826 & 15.913 & 15.739 & 16.217 \\
205   & 16.261 & 15.739 & 15.913 & 16.087 & 16.087 & 15.522 & 15.783 & 15.957 & 15.783 & 16.261 \\
206   & 16.217 & 15.739 & 15.87  & 16.043 & 16.087 & 15.522 & 15.696 & 15.957 & 15.87  & 16.261 \\
207   & 16.304 & 15.652 & 15.913 & 16.087 & 16     & 15.609 & 15.783 & 16     & 15.783 & 16.261 \\
208   & 16.261 & 15.696 & 16     & 16.13  & 15.957 & 15.522 & 15.739 & 15.826 & 15.783 & 16.217 \\
209   & 16.261 & 15.652 & 15.957 & 16     & 15.783 & 15.565 & 15.739 & 15.826 & 15.87  & 16.217 \\
210   & 16.304 & 15.696 & 15.957 & 15.913 & 15.913 & 15.522 & 15.696 & 15.87  & 15.826 & 16.13  \\
211   & 16.217 & 15.783 & 15.957 & 15.913 & 15.913 & 15.609 & 15.783 & 15.913 & 16.087 & 16.13  \\
212   & 16.261 & 15.826 & 16     & 15.957 & 15.913 & 15.652 & 15.739 & 15.826 & 16.043 & 16.261 \\
213   & 16.304 & 15.913 & 15.957 & 16.087 & 15.913 & 15.522 & 15.739 & 15.783 & 16.087 & 16.261 \\
214   & 16.348 & 16     & 16     & 16.174 & 15.87  & 15.696 & 15.739 & 15.826 & 16.043 & 16.261 \\
215   & 16.348 & 15.913 & 16.13  & 16.174 & 15.783 & 15.609 & 15.739 & 15.957 & 16     & 16.261 \\
216   & 16.174 & 15.913 & 16.13  & 16.174 & 15.87  & 15.565 & 15.696 & 16     & 16.043 & 16.261 \\
217   & 16.174 & 15.87  & 16.087 & 16.174 & 15.87  & 15.565 & 15.696 & 15.913 & 15.913 & 16.13  \\
218   & 16.261 & 15.913 & 16     & 16.174 & 15.826 & 15.609 & 15.565 & 15.957 & 16     & 16.261 \\
219   & 16.217 & 15.87  & 16.087 & 16.087 & 15.783 & 15.609 & 15.478 & 16.043 & 16.043 & 16.217 \\
220   & 16.087 & 15.87  & 16     & 16.087 & 15.739 & 15.739 & 15.565 & 16.043 & 15.957 & 16.217 \\
221   & 16.087 & 15.826 & 16.043 & 16.087 & 15.783 & 15.652 & 15.652 & 16.043 & 15.913 & 16.174 \\
222   & 16.13  & 15.87  & 16.043 & 16.174 & 15.957 & 15.609 & 15.739 & 16.087 & 16.043 & 16.087 \\
223   & 16.174 & 15.913 & 16.087 & 16.13  & 16.174 & 15.652 & 15.565 & 16     & 15.87  & 16.217 \\
224   & 16.174 & 16     & 16.087 & 16.174 & 16.043 & 15.652 & 15.652 & 16     & 15.957 & 16.13  \\
225   & 16.13  & 16     & 16.043 & 16.13  & 16.174 & 15.652 & 15.652 & 15.957 & 15.826 & 16.043 \\
226   & 16.261 & 16.13  & 16.13  & 16.043 & 16.087 & 15.565 & 15.609 & 15.913 & 15.826 & 16.174 \\
227   & 16.261 & 15.957 & 16.13  & 16.087 & 16.087 & 15.696 & 15.565 & 15.913 & 15.826 & 16.043 \\
228   & 16.217 & 15.957 & 16.174 & 16.043 & 16     & 15.652 & 15.565 & 15.913 & 15.913 & 16.043 \\
229   & 16.261 & 16.043 & 16.174 & 16.174 & 16     & 15.739 & 15.565 & 15.826 & 15.957 & 16.174 \\
230   & 16.261 & 16     & 16.261 & 16.087 & 15.913 & 15.739 & 15.435 & 15.87  & 15.87  & 16.13  \\
231   & 16.217 & 16.043 & 16.261 & 16.174 & 15.913 & 15.783 & 15.522 & 15.957 & 15.87  & 16.087 \\
232   & 16.087 & 16.087 & 16.217 & 16.087 & 15.913 & 15.87  & 15.565 & 15.826 & 15.913 & 16.087 \\
233   & 16.174 & 16.13  & 16.217 & 16.13  & 16     & 15.783 & 15.652 & 15.826 & 15.957 & 16.043 \\
234   & 16.13  & 16.087 & 16.174 & 16.13  & 16.087 & 15.783 & 15.565 & 15.913 & 16.043 & 16.043 \\
235   & 16.217 & 16.13  & 16.217 & 16.13  & 16     & 15.739 & 15.609 & 15.957 & 16.043 & 16.13  \\
236   & 16.13  & 16.13  & 16.217 & 16.13  & 16.043 & 15.826 & 15.652 & 16     & 16     & 16.087 \\
237   & 16.217 & 16.174 & 16.217 & 16.13  & 16.087 & 15.826 & 15.609 & 16.087 & 16.087 & 16.13  \\
238   & 16.217 & 16.043 & 16.217 & 16.13  & 16.348 & 15.957 & 15.652 & 15.957 & 16     & 16.174 \\
239   & 16.217 & 16.043 & 16.304 & 16.13  & 16.13  & 15.913 & 15.696 & 15.913 & 16.217 & 16.043 \\
240   & 16.217 & 16.13  & 16.348 & 16.13  & 16.13  & 16.087 & 15.652 & 15.87  & 16.13  & 16.13  \\
241   & 16.261 & 15.957 & 16.304 & 16.13  & 16.174 & 15.913 & 15.739 & 15.913 & 16.043 & 16.087 \\
242   & 16.261 & 16.043 & 16.348 & 16.13  & 16.13  & 15.957 & 15.739 & 16     & 16.174 & 16.087 \\
243   & 16.304 & 16.087 & 16.348 & 16.087 & 16.13  & 15.913 & 15.739 & 16     & 16.174 & 16.087 \\
244   & 16.13  & 16.043 & 16.435 & 16.043 & 16.087 & 15.87  & 15.826 & 15.957 & 16.087 & 15.957 \\
245   & 16.174 & 16.087 & 16.435 & 16.087 & 16.174 & 15.913 & 15.783 & 15.87  & 16.087 & 16     \\
246   & 16.174 & 15.957 & 16.435 & 16.13  & 16.087 & 16.043 & 15.826 & 15.913 & 15.913 & 15.957 \\
247   & 16.217 & 16     & 16.435 & 16.087 & 16.174 & 15.957 & 15.826 & 15.87  & 16     & 15.913 \\
248   & 16.174 & 16.043 & 16.478 & 16.13  & 16.13  & 16     & 15.826 & 15.87  & 16     & 16.043 \\
249   & 16.13  & 16.087 & 16.522 & 16.087 & 16.087 & 15.957 & 15.783 & 15.826 & 16.13  & 15.957 \\
250   & 16.13  & 16.043 & 16.435 & 16.174 & 15.957 & 15.783 & 15.783 & 15.739 & 15.913 & 16     \\
251   & 16.261 & 15.913 & 16.348 & 15.957 & 16     & 15.826 & 15.739 & 15.87  & 15.913 & 16     \\
252   & 16.174 & 15.913 & 16.304 & 15.957 & 15.957 & 15.783 & 15.696 & 15.826 & 16     & 15.826 \\
253   & 16.174 & 16     & 16.348 & 15.913 & 15.87  & 15.87  & 15.696 & 15.696 & 15.957 & 15.957 \\
254   & 16.087 & 16.087 & 16.348 & 15.87  & 15.957 & 15.783 & 15.783 & 15.696 & 16     & 16     \\
255   & 16.087 & 16.043 & 16.435 & 15.913 & 15.913 & 15.87  & 15.87  & 15.783 & 15.913 & 16     \\
256   & 16.087 & 15.957 & 16.304 & 16.043 & 15.913 & 15.87  & 15.913 & 15.652 & 15.957 & 16     \\
257   & 16.087 & 15.957 & 16.304 & 16.043 & 16     & 15.826 & 15.87  & 15.826 & 15.957 & 16     \\
258   & 16.13  & 16     & 16.261 & 16.087 & 15.957 & 15.826 & 15.826 & 15.826 & 15.913 & 16     \\
259   & 16.13  & 15.913 & 16.174 & 16     & 15.957 & 15.826 & 15.783 & 15.826 & 15.87  & 16.043 \\
260   & 16.087 & 15.957 & 16.174 & 16     & 15.957 & 15.87  & 15.783 & 15.957 & 15.87  & 16     \\
261   & 16.043 & 15.913 & 16.217 & 16.174 & 15.913 & 15.652 & 15.826 & 16     & 15.87  & 16.087 \\
262   & 16.13  & 16     & 16.217 & 16.174 & 15.957 & 15.739 & 15.783 & 15.826 & 15.826 & 16     \\
263   & 16.13  & 16     & 16.174 & 16.217 & 15.826 & 15.609 & 15.783 & 15.913 & 15.87  & 16     \\
264   & 16.13  & 15.87  & 16.174 & 16.087 & 15.87  & 15.609 & 15.652 & 16     & 15.826 & 16.043 \\
265   & 16.13  & 16     & 16.174 & 16.13  & 15.87  & 15.609 & 15.652 & 15.957 & 15.826 & 16.043 \\
266   & 16.13  & 15.87  & 16     & 16.174 & 15.783 & 15.565 & 15.652 & 15.957 & 15.826 & 16.087 \\
267   & 16.174 & 15.913 & 16     & 16.261 & 15.87  & 15.522 & 15.739 & 15.957 & 15.826 & 16     \\
268   & 16.13  & 16.087 & 16.043 & 16.174 & 16     & 15.522 & 15.652 & 15.957 & 15.957 & 16.087 \\
269   & 16.13  & 16     & 15.957 & 16.174 & 16     & 15.565 & 15.609 & 15.913 & 15.913 & 15.957 \\
270   & 16.174 & 15.87  & 16     & 16.217 & 16     & 15.609 & 15.652 & 15.957 & 15.957 & 15.87  \\
271   & 16.043 & 15.913 & 16.043 & 16.217 & 16     & 15.565 & 15.739 & 15.87  & 15.957 & 15.783 \\
272   & 16.087 & 16     & 16.087 & 16.13  & 15.957 & 15.652 & 15.652 & 15.87  & 15.957 & 15.87  \\
273   & 16.13  & 16     & 16.087 & 16.174 & 15.957 & 15.652 & 15.609 & 15.739 & 16.13  & 15.696 \\
274   & 16.13  & 15.957 & 16.13  & 16.087 & 16.043 & 15.652 & 15.652 & 15.783 & 16.043 & 15.783 \\
275   & 16.13  & 15.913 & 16.174 & 16.043 & 16.043 & 15.522 & 15.652 & 15.783 & 16.043 & 15.913 \\
276   & 16.087 & 15.913 & 16.13  & 15.957 & 16.043 & 15.522 & 15.652 & 15.696 & 15.957 & 15.957 \\
277   & 16.043 & 15.913 & 16.087 & 16     & 16.087 & 15.652 & 15.652 & 15.739 & 16.043 & 15.957 \\
278   & 16.087 & 15.826 & 16     & 16     & 16.043 & 15.696 & 15.609 & 15.652 & 15.957 & 15.87  \\
279   & 16.043 & 15.826 & 16.13  & 15.913 & 16.087 & 15.739 & 15.609 & 15.652 & 15.957 & 15.87  \\
280   & 16.13  & 15.739 & 16     & 15.957 & 15.913 & 15.609 & 15.609 & 15.696 & 16.043 & 15.913 \\
281   & 16.087 & 15.739 & 16     & 15.957 & 15.913 & 15.696 & 15.522 & 15.696 & 16.043 & 15.957 \\
282   & 16     & 15.696 & 16.043 & 16.043 & 15.87  & 15.652 & 15.522 & 15.696 & 15.957 & 16.043 \\
283   & 16     & 15.696 & 16.13  & 16     & 15.913 & 15.652 & 15.522 & 15.696 & 16.043 & 15.957 \\
284   & 16.087 & 15.652 & 16.174 & 16.043 & 15.87  & 15.609 & 15.522 & 15.652 & 16.043 & 16.087 \\
285   & 16.13  & 15.87  & 16.217 & 16.087 & 15.87  & 15.609 & 15.478 & 15.826 & 16.043 & 15.957 \\
286   & 16.13  & 15.87  & 16.217 & 16.13  & 15.913 & 15.609 & 15.609 & 15.826 & 16.13  & 16.043 \\
287   & 16.043 & 15.87  & 16.174 & 16.217 & 16     & 15.652 & 15.609 & 15.826 & 16.087 & 16.087 \\
288   & 16.087 & 15.87  & 16.261 & 16.043 & 15.87  & 15.609 & 15.652 & 15.826 & 16.043 & 16.087 \\
289   & 16.174 & 15.87  & 16.261 & 16.217 & 15.826 & 15.565 & 15.609 & 15.826 & 16.043 & 15.87  \\
290   & 16.087 & 15.87  & 16.261 & 16.217 & 15.783 & 15.565 & 15.609 & 15.652 & 16.043 & 15.913 \\
291   & 16.087 & 15.739 & 16.174 & 16.174 & 15.826 & 15.478 & 15.652 & 15.783 & 16.13  & 16     \\
292   & 16.043 & 15.739 & 16.217 & 16.13  & 15.826 & 15.696 & 15.783 & 15.783 & 16.087 & 16.087 \\
293   & 16.043 & 15.652 & 16.217 & 16.087 & 15.826 & 15.696 & 15.565 & 15.739 & 16.087 & 16.087 \\
294   & 16.043 & 15.652 & 16.217 & 16     & 15.913 & 15.739 & 15.565 & 15.783 & 16.043 & 16.087 \\
295   & 16.13  & 15.739 & 16.261 & 16.087 & 15.913 & 15.652 & 15.565 & 15.87  & 16.087 & 16.043 \\
296   & 16.174 & 15.652 & 16.261 & 16.087 & 16     & 15.696 & 15.609 & 15.913 & 16.087 & 16.087 \\
297   & 16.217 & 15.957 & 16.261 & 16.087 & 16     & 15.696 & 15.609 & 15.913 & 16.13  & 15.957 \\
298   & 16.13  & 15.957 & 16.261 & 16.174 & 16.391 & 15.696 & 15.652 & 15.913 & 16.087 & 16     \\
299   & 16.174 & 15.957 & 16.261 & 16.174 & 16.348 & 15.652 & 15.522 & 15.87  & 16.043 & 16.043 \\
300   & 16.13  & 16     & 16.261 & 16.043 & 16.348 & 15.652 & 15.522 & 15.957 & 16.043 & 15.87  \\
301   & 16.13  & 16.043 & 16.043 & 16.043 & 16.304 & 15.652 & 15.565 & 15.957 & 16.087 & 16     \\
302   & 16.087 & 15.957 & 16.087 & 16.13  & 16.304 & 15.609 & 15.478 & 15.957 & 16.13  & 15.957 \\
303   & 16.13  & 15.913 & 16.043 & 16.087 & 16.348 & 15.609 & 15.522 & 15.87  & 16.043 & 16.087 \\
304   & 16.13  & 15.957 & 16.13  & 16.087 & 16.217 & 15.565 & 15.478 & 15.913 & 16.087 & 16.304 \\
305   & 16.261 & 15.957 & 16.087 & 16.043 & 16.174 & 15.696 & 15.478 & 16     & 16.174 & 16.304 \\
306   & 16.217 & 15.957 & 16.087 & 16.043 & 16.304 & 15.696 & 15.565 & 16     & 16.13  & 16.304 \\
307   & 16.261 & 15.826 & 16.13  & 16.087 & 16.261 & 15.87  & 15.522 & 15.957 & 16.217 & 16.13  \\
308   & 16.13  & 15.957 & 16.13  & 16.087 & 16.13  & 15.783 & 15.565 & 16.087 & 16.13  & 16.13  \\
309   & 16.217 & 15.913 & 16.087 & 16.043 & 16.304 & 15.739 & 15.478 & 15.957 & 16.087 & 16.087 \\
310   & 16.217 & 15.957 & 16     & 16     & 16.348 & 15.87  & 15.478 & 15.913 & 16.043 & 16.087 \\
311   & 16.217 & 15.957 & 16.043 & 16     & 16.217 & 15.783 & 15.478 & 15.957 & 16.13  & 16.087 \\
312   & 16.174 & 16     & 16     & 16     & 16.174 & 15.783 & 15.478 & 15.957 & 16.043 & 16.087 \\
313   & 16.13  & 15.957 & 16.043 & 16.043 & 16.217 & 15.783 & 15.522 & 15.913 & 16.174 & 16.174 \\
314   & 16.13  & 16     & 16     & 16.087 & 16.13  & 15.87  & 15.522 & 16     & 16.13  & 16.174 \\
315   & 16.13  & 16.087 & 16     & 16.087 & 16.087 & 15.87  & 15.522 & 16     & 16.13  & 16.087 \\
316   & 16.174 & 16     & 16     & 16.043 & 16.13  & 15.87  & 15.478 & 16.043 & 16.087 & 16.087 \\
317   & 16.087 & 16     & 16     & 15.957 & 16.13  & 15.87  & 15.478 & 15.913 & 16.043 & 16.087 \\
318   & 16.087 & 15.957 & 16.174 & 15.957 & 16.174 & 15.826 & 15.522 & 15.957 & 16.13  & 16.13  \\
319   & 16.087 & 16     & 16.087 & 16.043 & 16.261 & 15.826 & 15.739 & 15.913 & 16.13  & 16.13  \\
320   & 16.13  & 16     & 16.087 & 16.043 & 16.174 & 15.783 & 15.696 & 15.87  & 16.13  & 16.13  \\
321   & 16.087 & 16.043 & 16.13  & 16     & 16.174 & 15.826 & 15.652 & 15.826 & 16.087 & 16.261 \\
322   & 16.13  & 16.043 & 16.261 & 16.043 & 16.174 & 15.957 & 15.609 & 15.783 & 16.13  & 16.13  \\
323   & 16.087 & 16.087 & 16.261 & 16.043 & 16.217 & 15.87  & 15.565 & 15.826 & 16.13  & 16.217 \\
324   & 16.13  & 16.043 & 16.261 & 15.957 & 16.261 & 15.957 & 15.565 & 15.783 & 16.087 & 16.174 \\
325   & 16     & 16     & 16.217 & 15.913 & 16.217 & 16     & 15.565 & 15.826 & 16.087 & 16     \\
326   & 16.043 & 16.13  & 16.13  & 15.913 & 16.217 & 16.087 & 15.478 & 15.826 & 16     & 15.957 \\
327   & 16.043 & 16.13  & 16.043 & 16     & 16.174 & 16     & 15.522 & 15.826 & 16.087 & 15.957 \\
328   & 16.043 & 16.043 & 16.087 & 16     & 16.13  & 16     & 15.652 & 15.826 & 16     & 16     \\
329   & 16.043 & 15.957 & 15.957 & 15.957 & 16.261 & 15.957 & 15.565 & 15.87  & 15.87  & 15.957 \\
330   & 16.087 & 16.043 & 15.957 & 15.957 & 16.348 & 16     & 15.522 & 15.826 & 15.957 & 15.87  \\
331   & 16.043 & 16.13  & 15.957 & 15.957 & 16.391 & 15.913 & 15.609 & 15.913 & 16     & 15.913 \\
332   & 16     & 16.174 & 15.913 & 15.913 & 16.261 & 15.87  & 15.652 & 16     & 15.913 & 15.87  \\
333   & 16     & 16.174 & 16     & 15.87  & 16.217 & 16.087 & 15.609 & 15.913 & 15.783 & 16.043 \\
334   & 16.043 & 16.217 & 15.87  & 15.87  & 16.13  & 16.087 & 15.565 & 15.913 & 15.87  & 16     \\
335   & 16.043 & 16.13  & 16     & 15.957 & 16.304 & 16.13  & 15.565 & 15.826 & 15.826 & 15.957 \\
336   & 16.043 & 16.13  & 15.957 & 16     & 16.304 & 16.13  & 15.609 & 15.87  & 15.826 & 16.043 \\
337   & 16.043 & 16.087 & 15.957 & 16     & 16.174 & 16.043 & 15.696 & 15.826 & 15.826 & 16.043 \\
338   & 16.13  & 16.13  & 15.957 & 15.957 & 16.261 & 15.957 & 15.652 & 15.826 & 15.826 & 16.043 \\
339   & 16.043 & 16.13  & 15.913 & 16     & 15.913 & 15.957 & 15.652 & 15.783 & 15.739 & 16     \\
340   & 16.087 & 16.174 & 15.826 & 15.957 & 15.913 & 15.913 & 15.696 & 15.783 & 15.696 & 15.957 \\
341   & 16     & 16.174 & 15.739 & 16.13  & 15.87  & 16     & 15.739 & 15.783 & 15.739 & 15.826 \\
342   & 16.13  & 16.174 & 15.739 & 16     & 15.913 & 15.913 & 15.696 & 15.783 & 15.696 & 15.826 \\
343   & 16.13  & 16.174 & 15.696 & 16.043 & 15.913 & 15.913 & 15.826 & 15.739 & 15.826 & 15.913 \\
344   & 16.043 & 16.087 & 15.696 & 16     & 15.913 & 15.87  & 15.739 & 15.739 & 15.739 & 15.913 \\
345   & 16     & 16.087 & 15.739 & 16.087 & 15.913 & 15.913 & 15.739 & 15.783 & 15.783 & 15.957 \\
346   & 16     & 16.087 & 15.739 & 16.043 & 15.957 & 16     & 15.739 & 15.826 & 15.783 & 15.913 \\
347   & 15.913 & 16.174 & 15.826 & 16.13  & 15.957 & 16     & 15.739 & 15.826 & 15.783 & 15.87  \\
348   & 16.087 & 16.174 & 15.826 & 16.087 & 15.957 & 15.957 & 15.739 & 15.826 & 15.696 & 15.826 \\
349   & 16     & 16.13  & 15.913 & 15.913 & 16.043 & 16     & 15.739 & 15.826 & 15.696 & 15.87  \\
350   & 15.826 & 16.13  & 15.957 & 15.87  & 15.957 & 16.043 & 15.739 & 15.739 & 15.739 & 16     \\
351   & 16     & 16.087 & 15.826 & 15.87  & 15.957 & 16.043 & 15.739 & 15.783 & 15.739 & 15.957 \\
352   & 15.913 & 16.087 & 15.957 & 15.957 & 15.826 & 16     & 15.739 & 15.696 & 15.783 & 16     \\
353   & 15.826 & 16.087 & 16.043 & 15.913 & 15.957 & 16.043 & 15.739 & 15.783 & 15.739 & 16.043 \\
354   & 15.783 & 16.043 & 15.957 & 15.783 & 15.87  & 16.043 & 15.739 & 15.783 & 15.739 & 16.174 \\
355   & 15.826 & 16.043 & 15.87  & 15.913 & 15.826 & 16.087 & 15.783 & 15.783 & 15.739 & 16.174 \\
356   & 15.696 & 16.087 & 16     & 15.87  & 15.826 & 15.957 & 15.783 & 15.783 & 15.739 & 16.13  \\
357   & 15.783 & 16.087 & 15.957 & 15.826 & 15.783 & 16     & 15.739 & 15.783 & 15.783 & 16.13  \\
358   & 15.783 & 16.087 & 15.957 & 15.87  & 15.87  & 15.957 & 15.739 & 15.826 & 15.783 & 16.174 \\
359   & 15.783 & 16.043 & 16.043 & 15.913 & 15.826 & 15.957 & 15.739 & 15.696 & 15.783 & 16.174 \\
360   & 15.783 & 16.043 & 16     & 15.87  & 15.87  & 16     & 15.739 & 15.652 & 15.783 & 16.174 \\
361   & 15.783 & 15.87  & 15.957 & 15.87  & 15.87  & 16     & 15.696 & 15.609 & 15.739 & 16.13  \\
362   & 15.87  & 15.87  & 16     & 15.87  & 15.87  & 16.043 & 15.696 & 15.826 & 15.739 & 15.913 \\
363   & 15.87  & 16     & 16     & 15.609 & 15.826 & 16     & 15.696 & 15.826 & 15.739 & 15.957 \\
364   & 15.87  & 16     & 16     & 15.609 & 15.826 & 16     & 15.739 & 15.826 & 15.739 & 15.87  \\
365   & 15.957 & 16     & 15.957 & 15.652 & 15.826 & 16.043 & 15.783 & 15.826 & 15.87  & 16.174 \\
366   & 15.957 & 16     & 15.957 & 15.739 & 15.826 & 16     & 15.783 & 15.739 & 15.826 & 16.13  \\
367   & 15.957 & 16     & 15.957 & 15.696 & 15.826 & 15.826 & 15.783 & 15.783 & 15.913 & 16.174 \\
368   & 16     & 16     & 15.957 & 15.739 & 15.826 & 15.957 & 15.826 & 15.739 & 15.696 & 16.174 \\
369   & 15.913 & 16     & 15.87  & 15.783 & 15.783 & 15.913 & 15.739 & 15.652 & 15.652 & 16.043 \\
370   & 15.957 & 16     & 15.826 & 15.739 & 15.87  & 16     & 15.739 & 15.739 & 15.565 & 16.043 \\
371   & 15.783 & 16     & 15.87  & 15.696 & 15.739 & 15.957 & 15.739 & 15.739 & 15.652 & 15.957 \\
372   & 15.826 & 15.957 & 15.87  & 15.696 & 15.652 & 15.957 & 16     & 15.696 & 15.609 & 15.87  \\
373   & 15.87  & 15.957 & 15.913 & 15.783 & 15.652 & 15.87  & 16.043 & 15.696 & 15.609 & 16.043 \\
374   & 15.739 & 15.87  & 15.957 & 15.783 & 15.739 & 15.913 & 16.13  & 15.783 & 15.652 & 16     \\
375   & 15.739 & 15.913 & 15.826 & 15.826 & 15.826 & 15.826 & 16.13  & 15.826 & 15.609 & 16.043 \\
376   & 15.739 & 15.957 & 15.957 & 15.87  & 15.609 & 15.696 & 16     & 15.87  & 15.696 & 16     \\
377   & 15.696 & 15.87  & 15.87  & 15.87  & 15.696 & 15.739 & 16.087 & 15.652 & 15.696 & 16.13  \\
378   & 15.739 & 15.913 & 15.87  & 15.87  & 15.609 & 15.609 & 15.913 & 15.652 & 15.696 & 16.13  \\
379   & 15.739 & 15.957 & 15.826 & 15.826 & 15.739 & 15.609 & 16     & 15.696 & 15.739 & 16.13  \\
380   & 15.783 & 15.957 & 15.826 & 15.783 & 15.696 & 15.565 & 15.957 & 15.696 & 15.783 & 16.174 \\
381   & 15.739 & 15.826 & 15.783 & 15.783 & 15.739 & 15.565 & 15.957 & 15.652 & 15.826 & 16.174 \\
382   & 15.739 & 15.957 & 15.826 & 15.739 & 15.696 & 15.652 & 15.87  & 15.609 & 15.826 & 16.391 \\
383   & 15.652 & 15.913 & 15.783 & 15.783 & 15.739 & 15.783 & 15.957 & 15.565 & 15.696 & 16     \\
384   & 15.609 & 15.826 & 15.913 & 15.826 & 15.783 & 15.696 & 16     & 15.565 & 15.739 & 16     \\
385   & 15.739 & 15.783 & 15.783 & 15.739 & 15.783 & 15.696 & 15.913 & 15.522 & 15.739 & 16.043 \\
386   & 15.739 & 15.913 & 15.87  & 15.696 & 15.783 & 15.609 & 15.87  & 15.696 & 15.696 & 16.13  \\
387   & 15.696 & 15.913 & 15.826 & 15.609 & 15.696 & 15.783 & 15.783 & 15.565 & 15.783 & 16.087 \\
388   & 15.739 & 15.826 & 15.739 & 15.696 & 15.652 & 15.826 & 15.696 & 15.565 & 15.783 & 16.043 \\
389   & 15.652 & 15.739 & 15.783 & 15.696 & 15.652 & 15.739 & 15.696 & 15.565 & 15.739 & 16.087 \\
390   & 15.652 & 15.739 & 15.696 & 15.609 & 15.609 & 15.652 & 15.652 & 15.739 & 15.783 & 16.13  \\
391   & 15.652 & 15.652 & 15.826 & 15.652 & 15.522 & 15.609 & 15.609 & 15.565 & 15.652 & 16.087 \\
\bottomrule\end{longtable}
\normalsize
