# Supplementary material for: Rehearsal-Free Continual Learning over Small Non-I.I.D. Batches
Source: arXiv:1907.03799 source file (2020-04-21)
Supplement: Supplementary file 9 [file 391_CWR.tex]

\subsection{CWR*, NICv2 - 391}
\fontsize{8}{11}\selectfont
\begin{longtable}[c]{rgrgrgrgrgr}
\hline
Batch & Run 0  & Run 1  & Run 2  & Run 3  & Run 4  & Run 5  & Run 6  & Run 7  & Run 8  & Run 9  \\ \hline
\endfirsthead
\endhead
0     & 7.174  & 7.174  & 7.174  & 7.174  & 7.174  & 7.174  & 7.174  & 7.174  & 7.174  & 7.174  \\
1     & 14     & 14     & 14     & 14     & 14     & 14     & 14     & 14     & 14     & 14     \\
2     & 13.435 & 13.435 & 14.696 & 14.391 & 14.043 & 14.391 & 14.043 & 14     & 14.478 & 13.87  \\
3     & 12.652 & 13.565 & 15.348 & 14.043 & 14.522 & 13.957 & 14.348 & 14.478 & 14.826 & 13.783 \\
4     & 12.087 & 13.957 & 15.565 & 14.739 & 14.565 & 14.13  & 14.696 & 14.522 & 14.217 & 13.87  \\
5     & 12.304 & 14.348 & 15.913 & 14.609 & 14.435 & 14.043 & 14.522 & 14.609 & 14.696 & 14.652 \\
6     & 12.739 & 14.13  & 16.609 & 14.087 & 14.087 & 13.609 & 14.826 & 15.391 & 14.913 & 14.391 \\
7     & 13.261 & 15.217 & 17.435 & 14.522 & 14     & 14.087 & 16.043 & 14.783 & 15.261 & 14.435 \\
8     & 13.261 & 15.348 & 17.565 & 14.696 & 14.565 & 13.783 & 15.826 & 14.565 & 15.348 & 14.087 \\
9     & 13.348 & 15.304 & 17.565 & 14.957 & 14.739 & 13.609 & 16.217 & 14.609 & 16.087 & 13.522 \\
10    & 13.13  & 15.652 & 17.783 & 14.783 & 14.696 & 13.391 & 16.13  & 14.739 & 15.913 & 14.348 \\
11    & 13.261 & 16.478 & 17.913 & 14.826 & 15.087 & 13.565 & 16.13  & 15.087 & 15.391 & 14.348 \\
12    & 13.174 & 15.913 & 17.565 & 15.174 & 14.565 & 13.739 & 16.478 & 15.304 & 15.957 & 15.217 \\
13    & 13.826 & 16.261 & 17.652 & 15     & 14.783 & 14.261 & 17.478 & 15.261 & 16.522 & 15.913 \\
14    & 14.087 & 16.609 & 17.609 & 14.783 & 14.957 & 14.174 & 17.348 & 15.609 & 17.261 & 16.478 \\
15    & 14     & 17.13  & 18.478 & 15.391 & 14.739 & 13.957 & 17.217 & 15.087 & 17.261 & 16.696 \\
16    & 14.565 & 17.087 & 19.478 & 15.261 & 16.652 & 14.565 & 17.348 & 15.652 & 17.304 & 17.652 \\
17    & 14.435 & 17.174 & 20.217 & 14.826 & 16.957 & 14.826 & 17.261 & 15.913 & 17.565 & 17.696 \\
18    & 15     & 17.217 & 20.391 & 15.043 & 17.348 & 15.13  & 17.391 & 15.652 & 17.391 & 17.826 \\
19    & 15.522 & 17.217 & 20.565 & 16.652 & 17.391 & 14.913 & 17.348 & 16.217 & 17.13  & 17.739 \\
20    & 15.696 & 17.304 & 20.783 & 16.174 & 17.652 & 15.13  & 17.348 & 16.435 & 17.739 & 17.652 \\
21    & 15.826 & 17.826 & 20.652 & 16.609 & 18.391 & 15.087 & 17.391 & 16.913 & 17.957 & 18.043 \\
22    & 16.13  & 17.913 & 20.609 & 16.565 & 18.174 & 15.087 & 18     & 16.826 & 17.913 & 17.913 \\
23    & 16.565 & 17.913 & 20.783 & 16.522 & 18.739 & 15.522 & 18     & 17     & 17.739 & 17.783 \\
24    & 16.478 & 18.087 & 20.913 & 16.826 & 19.261 & 16.174 & 18.435 & 17.261 & 17.739 & 17.739 \\
25    & 16.522 & 18.304 & 20.826 & 17.174 & 19.739 & 16.478 & 18.348 & 17.391 & 18.174 & 17.957 \\
26    & 16.652 & 18.217 & 20.826 & 17.261 & 19.826 & 16.783 & 18.217 & 17.609 & 18.174 & 18.348 \\
27    & 16.609 & 18.783 & 20.739 & 17.565 & 20     & 16.739 & 18.261 & 17.739 & 18.609 & 18.304 \\
28    & 16.913 & 18.783 & 21.13  & 18.174 & 20.304 & 16.783 & 18.261 & 18.087 & 18.652 & 18.13  \\
29    & 17     & 18.783 & 20.826 & 18.174 & 20.13  & 17.435 & 18.174 & 18.087 & 18.783 & 18.478 \\
30    & 17.522 & 18.783 & 20.913 & 18.609 & 20.391 & 17.522 & 18.522 & 17.957 & 18.826 & 18.913 \\
31    & 17.609 & 18.826 & 21.435 & 18.696 & 20.913 & 17.478 & 18.652 & 18.522 & 18.826 & 18.913 \\
32    & 17.652 & 19.217 & 21.435 & 19.043 & 20.957 & 17.217 & 18.87  & 18.522 & 18.478 & 19     \\
33    & 17.565 & 19.435 & 22.261 & 19     & 21.217 & 17.435 & 19.391 & 18.739 & 19.087 & 18.783 \\
34    & 18.174 & 19.391 & 22.261 & 19.043 & 21.348 & 17.13  & 19.783 & 18.957 & 19.043 & 19.087 \\
35    & 18.217 & 19.478 & 22.783 & 19.87  & 21.391 & 17.174 & 20     & 19     & 19.391 & 19.478 \\
36    & 18.348 & 19.478 & 22.826 & 19.957 & 21.478 & 17.522 & 20.348 & 18.826 & 19.87  & 19.565 \\
37    & 18.391 & 19.217 & 23.043 & 20.217 & 21.652 & 18.043 & 20.304 & 19     & 19.652 & 19.435 \\
38    & 18.522 & 19.174 & 23.348 & 20     & 21.478 & 18.435 & 20.435 & 19     & 19.652 & 19.348 \\
39    & 18.565 & 18.565 & 23.435 & 20.348 & 21.391 & 18.435 & 20.391 & 18.87  & 19.739 & 21     \\
40    & 18.609 & 18.478 & 23.174 & 20.304 & 21.565 & 18.478 & 20.348 & 19.435 & 20.261 & 20.957 \\
41    & 18.652 & 19.348 & 23.217 & 20.696 & 21.522 & 18.435 & 20.739 & 19.435 & 20.435 & 21.217 \\
42    & 18.652 & 19.609 & 23     & 20.957 & 21.522 & 18.478 & 20.739 & 19.435 & 20.478 & 21.522 \\
43    & 18.565 & 19.783 & 23     & 20.957 & 22.261 & 18.435 & 20.652 & 19.739 & 20.522 & 21.652 \\
44    & 18.609 & 19.696 & 23.478 & 21.043 & 22.348 & 18.348 & 21     & 19.783 & 20.609 & 22.174 \\
45    & 18.522 & 19.609 & 23.348 & 21     & 22.696 & 18.478 & 20.913 & 19.652 & 20.609 & 22.174 \\
46    & 18.696 & 19.652 & 23.174 & 21.043 & 23.348 & 18.652 & 20.957 & 19.652 & 20.522 & 22.609 \\
47    & 18.913 & 20.13  & 23.261 & 21.087 & 23.565 & 18.739 & 21.217 & 20.043 & 20.522 & 22.696 \\
48    & 19.217 & 20.13  & 23.217 & 20.826 & 23.957 & 18.957 & 21.304 & 20.087 & 20.478 & 22.913 \\
49    & 19.174 & 19.913 & 23.217 & 20.957 & 24     & 19.043 & 21.174 & 20.565 & 20.435 & 23.043 \\
50    & 19.391 & 20.087 & 23.087 & 20.783 & 23.826 & 19     & 21.217 & 20.696 & 20.391 & 22.87  \\
51    & 19.304 & 20.174 & 23.13  & 20.696 & 23.87  & 19.261 & 21.522 & 20.652 & 20.304 & 23     \\
52    & 19.304 & 20.261 & 23.217 & 20.913 & 24.478 & 19.652 & 21.783 & 20.783 & 20.261 & 23     \\
53    & 19.261 & 20.13  & 23.13  & 20.87  & 24.478 & 19.783 & 21.652 & 20.826 & 20.522 & 23.087 \\
54    & 19.261 & 20.391 & 23.217 & 20.913 & 24.739 & 19.957 & 21.652 & 21.174 & 20.478 & 22.826 \\
55    & 19.13  & 20.348 & 23.261 & 20.913 & 24.957 & 19.957 & 22     & 21.087 & 20.696 & 23.043 \\
56    & 19.217 & 20.348 & 23.217 & 21     & 24.478 & 20.043 & 22.174 & 21.13  & 20.87  & 23.304 \\
57    & 21.13  & 20.609 & 23.348 & 21.043 & 24.478 & 20.13  & 22.217 & 21.348 & 21.043 & 23.261 \\
58    & 21.13  & 20.261 & 23.565 & 22     & 24.609 & 20.087 & 22.174 & 21.391 & 21.826 & 23.522 \\
59    & 21.174 & 20.478 & 23.783 & 22     & 24.478 & 20.13  & 22.174 & 21.391 & 21.696 & 23.739 \\
60    & 21.391 & 20.13  & 24.087 & 22.609 & 24.565 & 20.304 & 22.174 & 22.13  & 21.87  & 23.783 \\
61    & 21.13  & 20.043 & 24.435 & 22.522 & 24.435 & 20.391 & 22.174 & 22.261 & 21.87  & 23.478 \\
62    & 21.522 & 20.609 & 24.435 & 22.652 & 24.826 & 20.696 & 22.13  & 22.304 & 21.826 & 23.435 \\
63    & 21.739 & 20.826 & 24.261 & 22.652 & 25.087 & 20.609 & 22.043 & 22.174 & 21.652 & 24.087 \\
64    & 21.696 & 20.783 & 24.261 & 23.609 & 26.13  & 21.261 & 22.261 & 22.174 & 21.783 & 24.348 \\
65    & 21.957 & 21.13  & 24.348 & 23.609 & 26.087 & 21.913 & 22.217 & 22.304 & 21.565 & 24.217 \\
66    & 22.087 & 21.174 & 24.348 & 23.739 & 26.696 & 22.13  & 22.217 & 22.261 & 21.783 & 24.739 \\
67    & 22.13  & 21     & 24.435 & 24.217 & 27.391 & 22.13  & 22.087 & 22.391 & 21.87  & 24.522 \\
68    & 22.174 & 21.522 & 24.522 & 24.348 & 27.696 & 22.043 & 22     & 22.652 & 21.696 & 24.696 \\
69    & 22.304 & 21.435 & 24.783 & 24.478 & 27.609 & 22.043 & 23.043 & 23.13  & 21.696 & 24.478 \\
70    & 22.217 & 21.739 & 25.87  & 23.957 & 27.87  & 22.043 & 23.348 & 23.13  & 21.739 & 24.696 \\
71    & 22.174 & 22     & 26.391 & 24.13  & 27.87  & 22.348 & 23.348 & 23.087 & 21.87  & 25.304 \\
72    & 22.261 & 21.87  & 26.957 & 23.913 & 27.87  & 22.348 & 23.391 & 23.217 & 21.957 & 25.609 \\
73    & 22.217 & 22.087 & 27.304 & 24.348 & 28.261 & 22.435 & 23.217 & 23.13  & 21.957 & 25.435 \\
74    & 22.348 & 22.261 & 27.913 & 24.435 & 27.522 & 23.391 & 23.087 & 23     & 22.348 & 25.478 \\
75    & 22.391 & 22.174 & 27.739 & 24.348 & 27.739 & 22.957 & 23.478 & 22.913 & 22.391 & 25.696 \\
76    & 22.174 & 22.087 & 27.913 & 24.348 & 27.739 & 22.87  & 23.522 & 23.217 & 22.87  & 25.826 \\
77    & 22.478 & 22.174 & 28.348 & 24.261 & 27.87  & 23.087 & 23.739 & 23.565 & 22.739 & 26.217 \\
78    & 22.913 & 22.304 & 28.304 & 24.565 & 28.478 & 23.478 & 24.13  & 23.739 & 22.739 & 26.391 \\
79    & 22.739 & 22.348 & 29.391 & 25.043 & 28.913 & 23.609 & 24.217 & 23.565 & 22.826 & 26.304 \\
80    & 22.783 & 22.522 & 29.565 & 25.043 & 28.696 & 23.783 & 24.13  & 23.609 & 22.957 & 26.435 \\
81    & 23.87  & 22.565 & 29.652 & 25.174 & 29.087 & 23.565 & 24.391 & 23.609 & 23     & 26.565 \\
82    & 24.043 & 22.522 & 29.957 & 25.957 & 29.304 & 23.478 & 24.304 & 23.696 & 23.391 & 26.522 \\
83    & 24.13  & 22.609 & 29.826 & 25.957 & 29.478 & 24.13  & 24.478 & 23.565 & 23.217 & 26.478 \\
84    & 24.217 & 22.565 & 29.826 & 26.261 & 29.609 & 24.652 & 24.565 & 23.565 & 23.261 & 26.957 \\
85    & 24.391 & 22.565 & 30     & 26.478 & 30.217 & 24.478 & 24.435 & 23.522 & 22.783 & 26.957 \\
86    & 24.913 & 22.609 & 30.13  & 26.87  & 30.261 & 24.522 & 24.391 & 23.739 & 23.217 & 27.783 \\
87    & 24.957 & 22.652 & 30.522 & 26.652 & 31.043 & 24.696 & 24.304 & 23.739 & 23.304 & 27.957 \\
88    & 25.217 & 22.565 & 30.783 & 26.696 & 30.957 & 24.522 & 24.13  & 24.043 & 23.304 & 27.826 \\
89    & 25.087 & 22.609 & 31.174 & 26.652 & 31.348 & 24.522 & 24.217 & 24.087 & 23.652 & 28.13  \\
90    & 24.957 & 22.565 & 31.261 & 27.043 & 31.522 & 24.565 & 24.435 & 24.478 & 23.696 & 28.13  \\
91    & 25.13  & 22.565 & 31.696 & 27.304 & 31.739 & 25.348 & 24.609 & 24.696 & 24.087 & 28.13  \\
92    & 25.217 & 22.652 & 31.739 & 27.174 & 31.783 & 25.348 & 24.739 & 24.609 & 24.348 & 28.348 \\
93    & 25.391 & 23.652 & 32.087 & 26.783 & 32     & 25.565 & 24.565 & 24.565 & 24.261 & 28.609 \\
94    & 25.348 & 23.913 & 32.087 & 26.783 & 31.957 & 25.522 & 24.522 & 24.609 & 24.609 & 28.739 \\
95    & 25.217 & 23.87  & 32.043 & 26.826 & 32.304 & 25.565 & 24.652 & 24.609 & 24.565 & 28.739 \\
96    & 26.087 & 23.957 & 32.478 & 26.696 & 32.565 & 25.783 & 24.783 & 24.435 & 24.696 & 29     \\
97    & 26.087 & 24     & 32.565 & 26.783 & 32.609 & 25.913 & 24.87  & 24.435 & 25.13  & 29.043 \\
98    & 25.957 & 23.826 & 32.783 & 27.13  & 32.913 & 26     & 24.87  & 24.739 & 25.043 & 29.174 \\
99    & 26     & 24.043 & 32.565 & 27.522 & 33     & 26.217 & 25.043 & 24.826 & 25.348 & 29.261 \\
100   & 26.391 & 24.435 & 32.435 & 27.522 & 33.043 & 26.304 & 25.217 & 24.957 & 25.348 & 29.348 \\
101   & 26.696 & 24.565 & 32.696 & 27.652 & 33.217 & 26.304 & 25.478 & 25.13  & 25.739 & 29.522 \\
102   & 27.174 & 24.913 & 32.957 & 28.217 & 33.391 & 26.391 & 25.174 & 25.391 & 25.87  & 29.696 \\
103   & 27.348 & 25.087 & 32.826 & 28.261 & 33.652 & 26.609 & 25.261 & 25.304 & 25.696 & 29.652 \\
104   & 27.826 & 25.13  & 33.087 & 28.304 & 33.87  & 27     & 25.565 & 25.87  & 26.087 & 30     \\
105   & 27.826 & 25.087 & 33.522 & 28.304 & 34.087 & 27     & 25.478 & 25.739 & 26.174 & 30.217 \\
106   & 27.783 & 25.043 & 33.609 & 28.391 & 34.304 & 27.391 & 25.957 & 25.826 & 26     & 30.348 \\
107   & 27.696 & 25.13  & 33.217 & 28.435 & 34.739 & 27.435 & 26     & 26.13  & 25.957 & 31     \\
108   & 28.043 & 24.957 & 33.304 & 28.87  & 35     & 27.696 & 27.783 & 26.087 & 26.261 & 31.261 \\
109   & 27.783 & 24.957 & 33.13  & 28.783 & 35.217 & 27.87  & 27.87  & 26.087 & 26.783 & 32.174 \\
110   & 28     & 25.348 & 33.478 & 28.826 & 35.174 & 28.696 & 28.261 & 26.087 & 26.565 & 32.522 \\
111   & 28.217 & 25.304 & 33.348 & 28.913 & 35.348 & 28.826 & 28.13  & 26.043 & 27.13  & 32.87  \\
112   & 28.609 & 25.304 & 33.783 & 28.739 & 35.391 & 28.783 & 28.478 & 26.348 & 27     & 33.261 \\
113   & 29.348 & 25.348 & 33.739 & 29.043 & 35.261 & 29.043 & 28.522 & 27.217 & 26.87  & 33.652 \\
114   & 29.174 & 25.261 & 33.348 & 29.13  & 35.348 & 29.13  & 28.565 & 27.261 & 27     & 33.304 \\
115   & 29.174 & 25.826 & 33.435 & 29.348 & 35.174 & 29.087 & 28.609 & 27.696 & 27.478 & 33.957 \\
116   & 29.13  & 26.261 & 33.348 & 29     & 34.478 & 29.13  & 28.522 & 27.957 & 27.783 & 34.348 \\
117   & 29.174 & 26.261 & 33.348 & 29.435 & 34.304 & 29.217 & 28.87  & 27.696 & 27.391 & 34.261 \\
118   & 29.217 & 26.13  & 33.348 & 29.435 & 34.522 & 29.348 & 28.957 & 28     & 27.522 & 34.522 \\
119   & 29.087 & 26.043 & 33.435 & 29.783 & 34.957 & 29.522 & 28.826 & 27.913 & 27.435 & 34.609 \\
120   & 29.261 & 26.348 & 33.565 & 29.957 & 35     & 29.478 & 28.913 & 27.826 & 27.565 & 34.739 \\
121   & 29.522 & 26.217 & 33.609 & 29.783 & 35.13  & 29.696 & 28.913 & 27.739 & 28     & 35.478 \\
122   & 29.652 & 26.391 & 33.826 & 30.043 & 35.435 & 29.609 & 28.783 & 27.87  & 27.826 & 35.174 \\
123   & 29.739 & 26.913 & 33.826 & 30.043 & 35.696 & 29.609 & 28.826 & 28.261 & 27.783 & 35.348 \\
124   & 29.826 & 27.478 & 34.478 & 30.043 & 35.913 & 29.391 & 29.087 & 28.261 & 28.043 & 35.565 \\
125   & 29.652 & 28.261 & 35     & 30.087 & 35.783 & 29.522 & 29.043 & 28.435 & 28.304 & 35.522 \\
126   & 29.913 & 28.348 & 35.217 & 30     & 35.696 & 29.261 & 29.478 & 28.739 & 28.304 & 35.522 \\
127   & 30.174 & 28.609 & 35.565 & 30.13  & 35.522 & 29.826 & 29.522 & 29.522 & 28.348 & 35.739 \\
128   & 30.217 & 28.565 & 35.435 & 30.217 & 35.739 & 29.652 & 29.957 & 29.391 & 28.261 & 35.783 \\
129   & 30.826 & 29.304 & 35.609 & 30.391 & 35.739 & 29.826 & 30.043 & 29.435 & 28.304 & 36.087 \\
130   & 31.174 & 29.478 & 35.522 & 30.391 & 35.957 & 29.609 & 30.13  & 29.783 & 28.739 & 36     \\
131   & 31.087 & 29.652 & 35.609 & 31     & 36.13  & 29.609 & 30.13  & 30.13  & 28.739 & 36.261 \\
132   & 31.609 & 29.739 & 35.609 & 30.739 & 35.826 & 29.739 & 30.261 & 30.174 & 28.87  & 36.043 \\
133   & 31.522 & 29.565 & 35.739 & 30.87  & 36.609 & 29.87  & 30.391 & 30.043 & 29     & 36.261 \\
134   & 31.739 & 29.783 & 35.783 & 30.957 & 36.435 & 29.87  & 30.391 & 30     & 28.87  & 36.174 \\
135   & 31.522 & 29.913 & 35.609 & 30.739 & 36.348 & 29.87  & 30.435 & 30     & 28.913 & 36.609 \\
136   & 31.391 & 30     & 35.696 & 30.565 & 36.652 & 30.087 & 30.217 & 30.304 & 28.826 & 36.87  \\
137   & 31.391 & 30.609 & 35.609 & 30.435 & 36.609 & 30.13  & 30.261 & 30.391 & 28.826 & 36.826 \\
138   & 31.565 & 30.652 & 35.609 & 30.913 & 36.696 & 30.261 & 30.435 & 30.348 & 29.13  & 36.87  \\
139   & 31.826 & 30.783 & 35.696 & 31.087 & 36.522 & 30.783 & 30.435 & 30.696 & 29.174 & 36.826 \\
140   & 31.739 & 30.565 & 35.478 & 32.087 & 36.391 & 31     & 30.522 & 30.696 & 29.087 & 37.043 \\
141   & 32.13  & 30.696 & 35.435 & 32.087 & 36.174 & 31.696 & 30.609 & 30.957 & 29.652 & 37.522 \\
142   & 32.391 & 30.609 & 35.435 & 32.043 & 35.87  & 31.696 & 30.522 & 30.783 & 29.217 & 38.043 \\
143   & 33.391 & 31     & 35.435 & 32.261 & 35.957 & 31.609 & 30.565 & 31.087 & 29.391 & 38.087 \\
144   & 33.478 & 31.261 & 35.391 & 32.435 & 36.043 & 31.391 & 30.696 & 31.391 & 29.435 & 38.304 \\
145   & 33.435 & 31.565 & 35.435 & 32.304 & 36.217 & 31.435 & 31     & 31.348 & 29.478 & 38.478 \\
146   & 33.391 & 31.696 & 35.304 & 32.435 & 36.261 & 31.304 & 30.826 & 31.783 & 29.435 & 38.043 \\
147   & 33.478 & 31.783 & 35.261 & 32.696 & 36.217 & 31.435 & 30.957 & 32.087 & 29.652 & 38.13  \\
148   & 33.826 & 32     & 35.348 & 32.739 & 36.435 & 32     & 30.913 & 32.174 & 29.739 & 38.478 \\
149   & 33.87  & 32.087 & 35.609 & 32.652 & 36.174 & 32.043 & 30.957 & 32.174 & 29.696 & 38.348 \\
150   & 34.261 & 32.13  & 35.696 & 32.826 & 36.391 & 32.087 & 31.087 & 32.348 & 29.565 & 38.261 \\
151   & 34.391 & 32.043 & 35.913 & 32.696 & 36.391 & 32.304 & 30.957 & 32.522 & 29.391 & 38     \\
152   & 34.478 & 32.087 & 35.739 & 32.696 & 36.391 & 32.391 & 31.087 & 32.435 & 29.348 & 37.913 \\
153   & 34.522 & 32.522 & 35.478 & 32.87  & 36.609 & 32.478 & 31.087 & 33.13  & 29.609 & 38     \\
154   & 34.348 & 32.696 & 36.391 & 32.435 & 36.609 & 33.391 & 31.217 & 33.522 & 29.565 & 38.174 \\
155   & 34.652 & 32.957 & 36.348 & 32.609 & 36.522 & 33.609 & 31.391 & 33.565 & 30.348 & 38.478 \\
156   & 34.696 & 33.217 & 36.478 & 32.783 & 36.478 & 33.652 & 31.609 & 33.565 & 30.87  & 38.522 \\
157   & 34.304 & 33.261 & 36.522 & 33.13  & 36.652 & 33.435 & 31.783 & 34.087 & 30.913 & 39.217 \\
158   & 34.304 & 33.304 & 36.174 & 33.174 & 36.739 & 33.652 & 31.783 & 34.304 & 31.522 & 38.913 \\
159   & 34.348 & 33.174 & 35.739 & 33.043 & 36.478 & 33.652 & 32.435 & 34.174 & 32.043 & 38.957 \\
160   & 34.435 & 33.261 & 36.087 & 33.13  & 36.391 & 33.783 & 32.348 & 33.957 & 32.565 & 39.217 \\
161   & 34.609 & 33.348 & 35.87  & 33.13  & 36.478 & 34.043 & 32.174 & 34.174 & 32.522 & 39.217 \\
162   & 34.348 & 33.348 & 35.87  & 33.13  & 36.391 & 34.043 & 32.652 & 34.261 & 32.609 & 39.391 \\
163   & 34.435 & 33.348 & 35.913 & 33.13  & 36.435 & 34     & 32.913 & 35     & 32.739 & 39.478 \\
164   & 34.435 & 33.478 & 35.913 & 33.174 & 36.261 & 34.043 & 33.13  & 35.217 & 32.783 & 39.522 \\
165   & 34.522 & 33.652 & 36.087 & 33.348 & 36.652 & 33.826 & 33.478 & 35.348 & 32.696 & 39.478 \\
166   & 34.652 & 33.696 & 36     & 33.565 & 36.652 & 34.13  & 33.783 & 35.435 & 33     & 39.609 \\
167   & 34.783 & 33.957 & 36.739 & 33.304 & 36.957 & 34.13  & 33.609 & 35.565 & 33     & 39.652 \\
168   & 34.652 & 34.043 & 36.739 & 33.522 & 37.783 & 34.565 & 33.783 & 35.609 & 32.913 & 39.957 \\
169   & 34.565 & 34.435 & 36.826 & 33.435 & 37.652 & 34.478 & 33.696 & 35.609 & 33     & 40.087 \\
170   & 35.087 & 34.478 & 37.13  & 33.348 & 37.565 & 34.609 & 33.522 & 35.609 & 33.391 & 39.957 \\
171   & 35.261 & 34.522 & 37.261 & 33.739 & 37.913 & 34.739 & 33.522 & 35.478 & 33.609 & 39.913 \\
172   & 35.348 & 34.696 & 36.957 & 33.826 & 37.739 & 35     & 33.478 & 35.348 & 33.957 & 40.087 \\
173   & 35.826 & 34.609 & 37.261 & 34.652 & 37.957 & 35.478 & 33.522 & 35.652 & 34.13  & 40.304 \\
174   & 35.826 & 34.957 & 37.043 & 35.174 & 37.826 & 35.435 & 33.652 & 35.652 & 34.087 & 40.304 \\
175   & 35.826 & 35.304 & 37.043 & 35     & 37.696 & 35.13  & 33.652 & 36.348 & 34.478 & 40.261 \\
176   & 35.87  & 35.348 & 37.043 & 35.087 & 37.739 & 35.348 & 33.957 & 36.348 & 35.174 & 40.391 \\
177   & 35.652 & 35.391 & 36.913 & 35.565 & 37.652 & 35.391 & 34.043 & 36.565 & 35.217 & 40.957 \\
178   & 35.565 & 35.391 & 36.957 & 36.087 & 37.957 & 35.304 & 34.087 & 36.652 & 35.174 & 41     \\
179   & 35.783 & 35.783 & 37.609 & 36.217 & 38.13  & 35.261 & 34.217 & 36.913 & 35.739 & 41.304 \\
180   & 36.391 & 36.043 & 37.304 & 36.435 & 38.043 & 35.304 & 34.217 & 36.652 & 35.696 & 41.522 \\
181   & 36.609 & 36.435 & 37.348 & 36.522 & 38.217 & 35.478 & 34.217 & 36.478 & 35.913 & 41.696 \\
182   & 36.435 & 36.478 & 37.087 & 36.652 & 38.565 & 35.304 & 34.217 & 36.696 & 35.913 & 41.696 \\
183   & 36.522 & 36.478 & 37.304 & 36.826 & 38.522 & 35.609 & 34.478 & 36.783 & 36.609 & 41.957 \\
184   & 36.957 & 36.696 & 37.478 & 36.826 & 38.478 & 35.435 & 34.609 & 36.609 & 37.217 & 41.826 \\
185   & 36.826 & 36.652 & 37.348 & 37.217 & 38.304 & 35.957 & 34.565 & 36.783 & 37.13  & 42.043 \\
186   & 36.913 & 36.652 & 37.652 & 37.348 & 38.739 & 35.826 & 34.609 & 36.913 & 37.435 & 42     \\
187   & 37.522 & 36.609 & 37.652 & 37.739 & 39.13  & 36.435 & 34.652 & 37.174 & 38.13  & 42     \\
188   & 37.652 & 36.696 & 37.783 & 37.696 & 39.087 & 36.522 & 34.913 & 37.174 & 37.957 & 42.391 \\
189   & 37.87  & 36.87  & 37.783 & 37.696 & 39.043 & 36.913 & 35     & 37.348 & 38.087 & 42.609 \\
190   & 38.435 & 36.87  & 38.043 & 37.957 & 38.913 & 36.826 & 35.522 & 37.304 & 38.696 & 42.565 \\
191   & 38.652 & 36.913 & 38.217 & 38.087 & 39.087 & 37.391 & 35.826 & 37.261 & 38.739 & 42.87  \\
192   & 38.565 & 37.043 & 38     & 38.348 & 39     & 37.696 & 35.913 & 37.522 & 39.043 & 42.913 \\
193   & 38.565 & 37.304 & 38.13  & 38.696 & 39.043 & 37.652 & 36.043 & 37.522 & 39.087 & 42.609 \\
194   & 38.565 & 37.435 & 38.13  & 38.522 & 39.435 & 37.696 & 36.391 & 37.652 & 39.696 & 42.435 \\
195   & 38.87  & 37.478 & 38.087 & 38.783 & 39.522 & 38.087 & 36.783 & 37.696 & 39.435 & 42.435 \\
196   & 39.304 & 37.391 & 38.13  & 39.174 & 39.522 & 37.826 & 36.652 & 37.826 & 39.826 & 42.348 \\
197   & 39.261 & 37.435 & 38.348 & 39.435 & 39.652 & 38.087 & 36.609 & 37.87  & 40.043 & 42.13  \\
198   & 39.391 & 37.522 & 38.435 & 39.435 & 39.609 & 38.348 & 37     & 37.739 & 39.87  & 42.348 \\
199   & 39.304 & 37.391 & 38.348 & 39.565 & 39.565 & 38.348 & 37.13  & 37.87  & 40.609 & 42.478 \\
200   & 39.261 & 37.435 & 38.739 & 39.565 & 39.565 & 38.435 & 37.13  & 38.174 & 40.783 & 42.957 \\
201   & 39.261 & 37.304 & 38.87  & 39.609 & 39.478 & 38.696 & 37.087 & 38.435 & 40.435 & 43.348 \\
202   & 38.913 & 37.348 & 38.957 & 39.522 & 39.826 & 38.652 & 37.13  & 38.478 & 40.913 & 43.391 \\
203   & 39.261 & 37.174 & 39.043 & 39.696 & 39.826 & 38.913 & 37.13  & 38.478 & 40.87  & 44.043 \\
204   & 39.174 & 37.391 & 39.304 & 39.913 & 39.957 & 38.87  & 37.522 & 38.478 & 41.174 & 44.348 \\
205   & 39.696 & 37.478 & 39.087 & 40.087 & 40.043 & 38.609 & 37.826 & 38.696 & 41.696 & 44.304 \\
206   & 39.783 & 37.391 & 39.043 & 41.913 & 40.174 & 38.739 & 37.609 & 38.826 & 42.043 & 44.304 \\
207   & 40.174 & 37.609 & 39.087 & 42.13  & 40.609 & 38.696 & 37.435 & 39.348 & 42.043 & 44.739 \\
208   & 40.043 & 37.739 & 39.522 & 42.348 & 40.435 & 38.87  & 37.391 & 39.304 & 41.783 & 44.739 \\
209   & 40.435 & 37.783 & 39.304 & 42.261 & 40.696 & 38.87  & 37.435 & 39.478 & 42     & 45.087 \\
210   & 40.739 & 37.696 & 39.348 & 42.391 & 40.652 & 39.217 & 38.304 & 39.261 & 42.217 & 44.957 \\
211   & 40.652 & 38.043 & 39.391 & 42.174 & 40.783 & 39.348 & 38.348 & 39.478 & 42.348 & 45.261 \\
212   & 40.435 & 38.043 & 39.304 & 42.739 & 40.261 & 39.478 & 38.565 & 39.217 & 42.304 & 45.391 \\
213   & 40.783 & 38.13  & 39.783 & 42.391 & 40.391 & 39.435 & 38.565 & 39.174 & 42.261 & 45.957 \\
214   & 40.783 & 37.913 & 39.696 & 42.478 & 40.304 & 39.609 & 38.87  & 39.304 & 42.478 & 45.652 \\
215   & 41     & 38     & 40.13  & 42.391 & 40.391 & 39.652 & 38.87  & 39.435 & 42.609 & 45.696 \\
216   & 40.696 & 38.174 & 40.261 & 42.652 & 40.826 & 39.391 & 39.348 & 39.435 & 42.522 & 45.783 \\
217   & 41     & 38.087 & 40.565 & 42.565 & 41.652 & 39.739 & 39.696 & 39.826 & 43.261 & 46.348 \\
218   & 41.043 & 38.13  & 40.696 & 42.522 & 41.957 & 39.478 & 40.348 & 39.957 & 43.304 & 46.435 \\
219   & 41.826 & 38.13  & 40.957 & 42.391 & 42.217 & 39.826 & 40.13  & 39.913 & 43.043 & 46.565 \\
220   & 41.87  & 38.13  & 40.913 & 42.435 & 42.261 & 40     & 40.609 & 40.652 & 43.304 & 46.565 \\
221   & 42.174 & 38.13  & 40.957 & 42.391 & 42.435 & 40     & 40.913 & 41.043 & 45     & 46.435 \\
222   & 42.174 & 38.304 & 41.174 & 42.522 & 42.652 & 40.217 & 41.043 & 40.957 & 45.217 & 46.565 \\
223   & 42.261 & 38.348 & 41.304 & 42.565 & 42.478 & 40.087 & 41.391 & 41.043 & 45.13  & 46.522 \\
224   & 42.043 & 38.435 & 41.826 & 42.435 & 42.217 & 40     & 41.783 & 40.826 & 45.217 & 46.696 \\
225   & 42.304 & 38.435 & 41.826 & 42.304 & 42.522 & 39.957 & 41.609 & 41     & 45.261 & 46.652 \\
226   & 42.348 & 38.391 & 41.565 & 42.348 & 42.348 & 40     & 42.087 & 41.13  & 45.565 & 46.739 \\
227   & 42.217 & 38.435 & 41.261 & 42.478 & 42.261 & 39.696 & 42.13  & 41.174 & 45.609 & 46.696 \\
228   & 42.261 & 38.261 & 41.696 & 42.391 & 42.435 & 39.696 & 42.043 & 41.609 & 45.391 & 46.609 \\
229   & 42.174 & 38.391 & 41.826 & 42.652 & 42.478 & 39.957 & 41.87  & 42.174 & 45.522 & 46.478 \\
230   & 42.087 & 38.522 & 42.391 & 42.652 & 42.565 & 40.043 & 41.957 & 42.087 & 45.957 & 46.609 \\
231   & 42.043 & 38.565 & 42.348 & 42.783 & 43.261 & 40.261 & 42.304 & 42.043 & 45.87  & 46.522 \\
232   & 42.304 & 39     & 42.478 & 42.913 & 43.391 & 40.783 & 42.217 & 42.043 & 46.174 & 46.304 \\
233   & 42.348 & 39.217 & 42.696 & 42.783 & 43.522 & 40.435 & 42.13  & 42.304 & 46.304 & 46.609 \\
234   & 42.478 & 39.391 & 42.391 & 42.87  & 43.826 & 40.304 & 42.13  & 42.391 & 46.087 & 46.739 \\
235   & 42.652 & 39.261 & 42.565 & 43.043 & 43.261 & 40.348 & 42.043 & 42.348 & 46.087 & 46.652 \\
236   & 42.609 & 39.261 & 42.87  & 43.217 & 44     & 40.522 & 42.304 & 42.391 & 46.304 & 46.609 \\
237   & 43     & 39.304 & 42.826 & 43.087 & 44.261 & 40.478 & 42.391 & 42.609 & 46.391 & 46.565 \\
238   & 43.043 & 39.522 & 42.522 & 43.087 & 44.478 & 40.696 & 42.174 & 42.957 & 46.174 & 46.696 \\
239   & 42.957 & 39.522 & 42.696 & 43.261 & 44.261 & 40.957 & 42.304 & 43     & 46.217 & 46.565 \\
240   & 43     & 39.826 & 42.739 & 43.565 & 44.478 & 41.174 & 42.652 & 42.609 & 45.957 & 46.609 \\
241   & 43.13  & 39.652 & 43.087 & 43.391 & 44.478 & 41.174 & 42.739 & 42.957 & 46.13  & 46.348 \\
242   & 43.391 & 39.957 & 43.696 & 43.522 & 44.565 & 41.261 & 42.913 & 43.478 & 45.87  & 46.348 \\
243   & 43.348 & 39.957 & 43.739 & 43.565 & 45.043 & 41.609 & 42.522 & 43.348 & 46.13  & 46.739 \\
244   & 42.957 & 40.478 & 45.522 & 43.435 & 45     & 41.826 & 43.435 & 43.348 & 46     & 46.739 \\
245   & 43.348 & 40.565 & 45.435 & 43.87  & 45     & 41.783 & 43.391 & 43.174 & 45.957 & 46.826 \\
246   & 43.478 & 40.478 & 45.478 & 44.217 & 45.87  & 42.261 & 43.304 & 43.261 & 46.087 & 46.739 \\
247   & 43.652 & 40.435 & 45.261 & 44.304 & 46.174 & 42.217 & 43.652 & 42.87  & 46.13  & 46.87  \\
248   & 43.739 & 40.696 & 45.652 & 44.391 & 46.174 & 42.174 & 43.87  & 43.087 & 46.217 & 47.13  \\
249   & 44.087 & 40.565 & 45.652 & 44.478 & 46.087 & 42.348 & 43.87  & 43.435 & 46.261 & 47.261 \\
250   & 43.87  & 40.87  & 45.391 & 44.783 & 46.217 & 42.478 & 43.826 & 43.304 & 46.087 & 47.043 \\
251   & 44.217 & 40.609 & 45.652 & 44.522 & 46.043 & 42.565 & 44.348 & 43.783 & 46.522 & 47     \\
252   & 44     & 40.696 & 45.783 & 44.783 & 46.261 & 42.478 & 44.783 & 43.391 & 46.826 & 47.043 \\
253   & 44.174 & 40.522 & 45.826 & 45.435 & 46.435 & 42.435 & 44.609 & 43.391 & 46.652 & 47.435 \\
254   & 43.913 & 40.739 & 45.739 & 45.739 & 46.304 & 42.391 & 44.826 & 43.522 & 46.522 & 47.565 \\
255   & 43.87  & 40.739 & 46.174 & 45.478 & 46.304 & 42.478 & 44.826 & 43.174 & 46.913 & 47.652 \\
256   & 43.739 & 40.652 & 46.13  & 45.957 & 46.304 & 42.478 & 44.957 & 43.174 & 46.913 & 47.783 \\
257   & 43.783 & 40.913 & 46.13  & 46.217 & 46.174 & 42.783 & 45.217 & 43.391 & 46.913 & 47.696 \\
258   & 43.739 & 41.565 & 46.348 & 46.304 & 46.261 & 43.087 & 45.043 & 43.261 & 47.087 & 47.609 \\
259   & 43.783 & 41.565 & 46.522 & 46.348 & 46.261 & 43.391 & 44.783 & 43.478 & 47.087 & 47.652 \\
260   & 44.043 & 41.826 & 46.304 & 46.217 & 46.217 & 43.652 & 44.826 & 43.522 & 47.435 & 47.87  \\
261   & 44.217 & 41.609 & 46.609 & 46.348 & 46.348 & 43.565 & 44.739 & 43.565 & 47.435 & 48.217 \\
262   & 44.348 & 41.913 & 47     & 46.304 & 46.565 & 43.565 & 44.565 & 43.348 & 47.478 & 48.13  \\
263   & 44.609 & 42.174 & 46.957 & 46.522 & 46.565 & 43.565 & 44.652 & 43     & 47.957 & 47.87  \\
264   & 45.391 & 42.174 & 47.087 & 46.696 & 46.609 & 43.783 & 44.913 & 43.348 & 47.783 & 48.174 \\
265   & 44.957 & 42.435 & 47.652 & 47.13  & 46.739 & 43.696 & 44.739 & 43.217 & 48.043 & 48.043 \\
266   & 45.391 & 42.522 & 47.826 & 47.174 & 46.609 & 43.783 & 44.957 & 43.391 & 47.87  & 48.087 \\
267   & 45.174 & 42.739 & 47.783 & 47.391 & 46.478 & 43.652 & 44.87  & 43.348 & 47.87  & 47.609 \\
268   & 44.739 & 42.739 & 48.043 & 47.391 & 46.609 & 43.652 & 45.217 & 43.348 & 48     & 47.783 \\
269   & 45.087 & 42.609 & 48     & 47.609 & 46.87  & 43.739 & 45.13  & 45.174 & 48.391 & 47.87  \\
270   & 45.652 & 42.609 & 48.348 & 47.739 & 46.478 & 43.957 & 45.609 & 45     & 48.174 & 47.957 \\
271   & 45.783 & 42.652 & 48.87  & 47.87  & 46.609 & 43.826 & 45.783 & 45.391 & 47.913 & 47.913 \\
272   & 45.739 & 42.87  & 48.913 & 47.739 & 46.783 & 43.696 & 45.565 & 45.565 & 47.957 & 47.826 \\
273   & 45.348 & 43.217 & 48.957 & 47.87  & 47     & 43.739 & 45.435 & 45.696 & 47.87  & 47.826 \\
274   & 45.304 & 43.304 & 49.043 & 47.87  & 47.13  & 43.696 & 45.826 & 45.739 & 48.043 & 47.87  \\
275   & 44.957 & 43.391 & 49.348 & 47.913 & 47.565 & 43.87  & 45.913 & 45.826 & 48.435 & 48.13  \\
276   & 45.174 & 43.435 & 49.565 & 48.087 & 47.522 & 44.783 & 46.261 & 46.087 & 48.696 & 48.696 \\
277   & 44.783 & 43.609 & 49.826 & 48.217 & 47.696 & 45     & 46.087 & 45.957 & 48.826 & 48.609 \\
278   & 45.087 & 43.696 & 49.87  & 48.696 & 47.826 & 45.13  & 45.913 & 45.826 & 48.87  & 48.391 \\
279   & 44.957 & 43.652 & 50.043 & 48.609 & 47.783 & 45.304 & 46.391 & 45.87  & 48.609 & 48.565 \\
280   & 44.739 & 43.87  & 49.87  & 48.609 & 47.913 & 45.13  & 46.217 & 45.957 & 48.783 & 48.478 \\
281   & 44.522 & 43.87  & 50.13  & 48.739 & 48     & 45.043 & 47.174 & 46.043 & 48.739 & 48.304 \\
282   & 45.043 & 44.087 & 50.304 & 49.043 & 48.13  & 45.174 & 47     & 45.87  & 48.913 & 49.087 \\
283   & 45.261 & 44.087 & 50.174 & 48.913 & 48.087 & 45.304 & 47.522 & 45.913 & 49.13  & 49.261 \\
284   & 45.261 & 44.565 & 50.348 & 49.087 & 48.174 & 45.435 & 47.565 & 46.043 & 49.087 & 49.174 \\
285   & 45.217 & 44.739 & 50.522 & 49.391 & 48.261 & 45.522 & 47.391 & 46.13  & 48.913 & 48.826 \\
286   & 45.522 & 44.783 & 50.783 & 49.609 & 48.043 & 45.522 & 47.826 & 46.261 & 49.043 & 49.087 \\
287   & 45.826 & 44.87  & 50.565 & 49.739 & 48.478 & 45.522 & 47.957 & 46.217 & 49.348 & 49.913 \\
288   & 45.826 & 45     & 50.87  & 49.522 & 48.522 & 45.478 & 48     & 46.391 & 49.522 & 49.957 \\
289   & 45.957 & 45.043 & 50.913 & 50.174 & 48.348 & 45.913 & 48     & 46.478 & 50     & 49.87  \\
290   & 46.217 & 46.87  & 50.826 & 50.391 & 48.217 & 45.739 & 48     & 47.043 & 50     & 50.435 \\
291   & 46.696 & 47.043 & 50.913 & 50.609 & 48.261 & 45.522 & 48.217 & 47.13  & 50.043 & 50.304 \\
292   & 46.826 & 46.913 & 51.087 & 50.609 & 48.522 & 45.87  & 48.609 & 47.043 & 49.957 & 50.652 \\
293   & 47     & 47.826 & 51.087 & 50.478 & 48.565 & 45.739 & 48.478 & 47.783 & 50     & 50.522 \\
294   & 46.87  & 48.304 & 51.13  & 50.391 & 48.652 & 46.174 & 48.522 & 47.696 & 49.913 & 50.652 \\
295   & 46.696 & 48.217 & 51.087 & 50.565 & 48.696 & 46.652 & 48.652 & 47.565 & 50.087 & 50.739 \\
296   & 47.435 & 48.435 & 51.087 & 50.609 & 48.87  & 47.087 & 48.739 & 47.913 & 50.348 & 50.783 \\
297   & 47.696 & 48.391 & 51.174 & 50.87  & 49.174 & 47.478 & 48.783 & 48.043 & 50.391 & 50.739 \\
298   & 48.522 & 48.696 & 51.043 & 50.957 & 49.217 & 47.565 & 48.87  & 48.087 & 50.043 & 50.826 \\
299   & 48.739 & 48.739 & 51     & 51.174 & 49.304 & 47.696 & 48.783 & 48.217 & 50.348 & 50.87  \\
300   & 48.826 & 49.348 & 51.348 & 51.478 & 49.609 & 49.348 & 49.348 & 48.043 & 50.348 & 50.957 \\
301   & 49.087 & 49.13  & 51.391 & 51.652 & 49.435 & 49.478 & 49.087 & 48.087 & 50.391 & 51.174 \\
302   & 49.261 & 49.261 & 51.826 & 51.783 & 49.609 & 49.174 & 49.217 & 48.304 & 50.435 & 51.304 \\
303   & 49.652 & 49.174 & 52.087 & 51.826 & 49.522 & 49.391 & 49.217 & 48.217 & 50.174 & 51.217 \\
304   & 50.174 & 49     & 52.174 & 52.217 & 49.478 & 49.348 & 49.043 & 48.391 & 50.261 & 51.174 \\
305   & 50.043 & 49     & 52.391 & 52.391 & 49.348 & 49.609 & 49.391 & 48.261 & 50.696 & 51.478 \\
306   & 49.826 & 48.87  & 52.696 & 52.478 & 49.826 & 49.696 & 49.435 & 48.478 & 50.565 & 51.348 \\
307   & 50.174 & 48.913 & 52.565 & 52.652 & 49.565 & 49.826 & 49.348 & 48.609 & 50.87  & 51.783 \\
308   & 50.217 & 49.087 & 52.261 & 52.478 & 49.739 & 49.696 & 49.087 & 48.435 & 51.043 & 51.913 \\
309   & 50.261 & 48.957 & 52.609 & 52.696 & 49.739 & 49.957 & 49.304 & 48.565 & 51.391 & 51.478 \\
310   & 49.87  & 49.435 & 52.522 & 52.478 & 49.652 & 50.217 & 49.478 & 48.609 & 51.217 & 51.826 \\
311   & 50.261 & 49.478 & 52.609 & 52.435 & 49.522 & 50.087 & 49.217 & 48.696 & 51.304 & 51.913 \\
312   & 50.435 & 49.739 & 52.348 & 52.522 & 49.522 & 50.435 & 49.609 & 48.652 & 51.304 & 51.739 \\
313   & 50.565 & 49.87  & 52.348 & 52.696 & 49.478 & 50.435 & 49.478 & 48.739 & 51.435 & 52.261 \\
314   & 50.826 & 49.913 & 52.565 & 53.087 & 49.435 & 50.652 & 49.435 & 49.478 & 51.609 & 52.261 \\
315   & 51.13  & 50.043 & 52.609 & 53.217 & 49.13  & 50.826 & 49.696 & 49.609 & 51.478 & 52.304 \\
316   & 51.217 & 49.87  & 52.783 & 53.826 & 49.391 & 50.783 & 49.478 & 49.957 & 51.348 & 52.043 \\
317   & 51.435 & 49.913 & 52.783 & 54.087 & 49.348 & 50.826 & 49.522 & 50.391 & 51.565 & 52.391 \\
318   & 51.565 & 50.174 & 52.913 & 54.217 & 49.87  & 51.217 & 50.304 & 50.435 & 51.565 & 52.174 \\
319   & 51.783 & 50.826 & 52.87  & 54.174 & 50     & 51.261 & 49.957 & 50.435 & 51.348 & 52.217 \\
320   & 51.739 & 50.87  & 53.391 & 54.565 & 50.652 & 51.478 & 50.391 & 50.565 & 51.478 & 52.261 \\
321   & 51.739 & 50.826 & 53.391 & 54.739 & 50.739 & 51.87  & 50.391 & 50.696 & 51.826 & 52.261 \\
322   & 51.783 & 51.043 & 53.522 & 54.87  & 50.826 & 51.609 & 50.435 & 50.913 & 52.13  & 52.652 \\
323   & 52.087 & 50.87  & 53.696 & 54.739 & 50.739 & 51.957 & 50.391 & 50.783 & 52.043 & 52.522 \\
324   & 51.87  & 50.87  & 53.609 & 54.696 & 50.826 & 52.217 & 50.304 & 51     & 52.13  & 52.609 \\
325   & 51.609 & 50.957 & 53.652 & 54.522 & 50.696 & 52.174 & 50.522 & 50.957 & 52.13  & 52.304 \\
326   & 51.696 & 51.391 & 53.87  & 54.826 & 50.826 & 52.478 & 50.391 & 50.913 & 52.043 & 52.348 \\
327   & 51.957 & 51.391 & 53.957 & 54.783 & 50.913 & 53.217 & 50.609 & 51.043 & 52.391 & 52.348 \\
328   & 51.826 & 51.348 & 53.826 & 54.826 & 50.783 & 54     & 50.87  & 51.217 & 51.957 & 52.217 \\
329   & 51.826 & 51.739 & 53.826 & 55     & 50.826 & 54.043 & 51     & 51.174 & 52.304 & 52.478 \\
330   & 52.13  & 52.043 & 53.826 & 54.913 & 51     & 53.913 & 51.739 & 51.261 & 52.13  & 52.261 \\
331   & 51.565 & 52     & 53.826 & 54.957 & 51.174 & 53.565 & 52.391 & 51.913 & 52.217 & 52.696 \\
332   & 51.435 & 52.391 & 53.696 & 54.652 & 51.391 & 53.348 & 52.478 & 51.783 & 52.261 & 53.13  \\
333   & 51.304 & 52.304 & 53.957 & 54.783 & 51.174 & 53.348 & 52.522 & 52     & 52.174 & 53.217 \\
334   & 51.435 & 52.652 & 53.739 & 54.957 & 51.826 & 53.348 & 52.348 & 52.174 & 52.13  & 53.217 \\
335   & 51.478 & 52.826 & 53.913 & 54.957 & 51.652 & 53.435 & 52.087 & 52.217 & 52.87  & 53.696 \\
336   & 51.739 & 53.043 & 53.826 & 55.217 & 51.652 & 53.696 & 52.87  & 52.304 & 52.826 & 53.478 \\
337   & 52     & 53.087 & 54.043 & 55.13  & 52.174 & 53.783 & 53     & 52.174 & 52.652 & 53.783 \\
338   & 51.957 & 53.13  & 53.87  & 55.348 & 52.174 & 54.174 & 53.435 & 52.087 & 52.826 & 54.304 \\
339   & 52.435 & 53.652 & 53.609 & 55.739 & 52.13  & 54.217 & 53.391 & 52.391 & 52.826 & 54.609 \\
340   & 52.304 & 53.174 & 53.87  & 55.739 & 52.217 & 54.304 & 53.304 & 52.696 & 53.174 & 54.565 \\
341   & 52.217 & 53.478 & 53.783 & 55.435 & 52.348 & 54.391 & 53.304 & 53.087 & 53.174 & 55.174 \\
342   & 52.522 & 53.478 & 53.826 & 55.478 & 52.13  & 54.348 & 53.435 & 53.391 & 53.348 & 55.435 \\
343   & 52.739 & 53.652 & 54     & 55.217 & 52.087 & 54.261 & 53.87  & 53.522 & 53.783 & 55.478 \\
344   & 52.783 & 54     & 54.348 & 55.739 & 52.261 & 54.217 & 54.217 & 53.478 & 53.913 & 55.348 \\
345   & 53.478 & 53.739 & 54.435 & 55.783 & 52.478 & 54.304 & 54.609 & 53.652 & 54.304 & 55.304 \\
346   & 53.609 & 54.217 & 54.391 & 56.174 & 52.522 & 53.913 & 55.043 & 54     & 54.13  & 55.087 \\
347   & 53.217 & 54.087 & 54.217 & 56.174 & 53.13  & 53.87  & 55.13  & 54.87  & 54.652 & 55.478 \\
348   & 53.304 & 53.913 & 54.174 & 56.522 & 53.13  & 54.217 & 55.435 & 55.043 & 54.826 & 55.522 \\
349   & 53.435 & 53.696 & 54.522 & 56.043 & 53.174 & 54     & 55.478 & 54.913 & 54.783 & 56.043 \\
350   & 53.478 & 53.783 & 55.304 & 56     & 53.13  & 53.957 & 55.957 & 54.913 & 54.87  & 56.435 \\
351   & 53.174 & 54.174 & 54.913 & 55.913 & 53.043 & 54.13  & 55.696 & 54.652 & 55.217 & 56.478 \\
352   & 53.478 & 53.957 & 54.826 & 55.913 & 52.913 & 53.957 & 55.783 & 54.913 & 55.435 & 56.522 \\
353   & 53.348 & 53.696 & 55.391 & 55.913 & 53.348 & 53.739 & 55.739 & 54.957 & 55.609 & 56.609 \\
354   & 53.217 & 53.652 & 55.217 & 55.739 & 53.435 & 53.565 & 55.957 & 55.174 & 55.696 & 56.783 \\
355   & 53.652 & 53.652 & 55.13  & 55.87  & 53.435 & 53.957 & 56.043 & 55.13  & 55.826 & 56.261 \\
356   & 53.652 & 53.652 & 54.913 & 56.174 & 53.826 & 54.478 & 55.957 & 55.348 & 55.783 & 56.304 \\
357   & 53.87  & 53.304 & 55     & 56.13  & 53.957 & 54.217 & 56.13  & 55     & 55.478 & 56.043 \\
358   & 54.261 & 53.652 & 55     & 56     & 53.783 & 54.348 & 56.348 & 55.174 & 55.478 & 56.261 \\
359   & 54.261 & 53.652 & 54.826 & 55.913 & 53.739 & 54.435 & 56.391 & 54.913 & 55.609 & 56.435 \\
360   & 54.391 & 54.043 & 55.043 & 56.261 & 53.826 & 54.304 & 56.696 & 54.913 & 55.739 & 56.565 \\
361   & 54.913 & 53.783 & 54.826 & 56.435 & 54.087 & 54.435 & 56.826 & 55.217 & 55.739 & 56.565 \\
362   & 54.609 & 53.739 & 54.913 & 56.652 & 53.957 & 54.565 & 56.652 & 55.13  & 55.87  & 56.696 \\
363   & 54.478 & 54.087 & 55     & 56.522 & 53.783 & 54.391 & 56.913 & 55.043 & 55.652 & 56.652 \\
364   & 54.391 & 54     & 55.043 & 56.217 & 54.087 & 54.391 & 57.261 & 54.783 & 55.391 & 56.348 \\
365   & 54.826 & 54.217 & 55.13  & 56.087 & 54.478 & 54.478 & 57.261 & 54.87  & 55.174 & 56.348 \\
366   & 54.696 & 54.348 & 54.957 & 56.13  & 54.696 & 54.174 & 57.478 & 54.87  & 55.478 & 56.565 \\
367   & 55.13  & 54.391 & 55.13  & 56.348 & 55     & 54.174 & 57.478 & 55     & 55.391 & 56.565 \\
368   & 55.261 & 54.609 & 55.261 & 56.304 & 55.478 & 54.609 & 57.609 & 55.348 & 55.652 & 56.652 \\
369   & 54.87  & 54.826 & 55.609 & 56.348 & 55.261 & 54.217 & 57.391 & 55.652 & 55.348 & 56.739 \\
370   & 55.043 & 54.87  & 55.565 & 56.609 & 55.478 & 54.565 & 57.261 & 55.739 & 55.435 & 57.087 \\
371   & 55     & 55.261 & 55.652 & 56.739 & 55.478 & 54.652 & 57.391 & 56     & 55.261 & 57.043 \\
372   & 55.13  & 55.174 & 55.783 & 57.304 & 55.435 & 54.783 & 57.826 & 55.87  & 55.174 & 57.087 \\
373   & 55.174 & 55.522 & 55.783 & 57.348 & 55.783 & 54.696 & 58.217 & 55.87  & 54.826 & 57.13  \\
374   & 55.174 & 55.957 & 55.826 & 57.304 & 55.783 & 54.739 & 58     & 56.304 & 55.348 & 57.087 \\
375   & 55.522 & 55.739 & 55.957 & 57.043 & 56.217 & 54.739 & 58.522 & 56.435 & 55.435 & 57.217 \\
376   & 55.652 & 55.913 & 55.783 & 57     & 56.304 & 54.783 & 58.348 & 56.348 & 55.304 & 57.348 \\
377   & 55.565 & 56.174 & 55.826 & 57.13  & 56.522 & 54.348 & 58.739 & 55.913 & 54.913 & 57.522 \\
378   & 56.043 & 56     & 55.87  & 57.13  & 56.478 & 54.304 & 58.739 & 55.826 & 55.087 & 57.565 \\
379   & 56.043 & 56.087 & 55.913 & 56.957 & 56.652 & 54.174 & 58.913 & 56.217 & 55.435 & 57.609 \\
380   & 55.826 & 56.13  & 55.913 & 56.826 & 56.435 & 54.13  & 59.261 & 56.348 & 55.652 & 57.87  \\
381   & 55.783 & 56.304 & 55.826 & 56.957 & 56.522 & 54.348 & 59.174 & 56.478 & 56.174 & 57.913 \\
382   & 56.261 & 56.391 & 55.696 & 56.739 & 56.348 & 54.522 & 59.043 & 56.783 & 56     & 57.783 \\
383   & 56     & 56.565 & 55.87  & 56.826 & 56.217 & 55     & 59.217 & 56.609 & 56.087 & 57.565 \\
384   & 56.13  & 56.609 & 56.043 & 56.783 & 56.261 & 54.696 & 59.261 & 56.696 & 55.87  & 57.522 \\
385   & 56.565 & 57.13  & 56     & 56.739 & 56.304 & 54.478 & 59.348 & 56.696 & 56.261 & 57.522 \\
386   & 56.739 & 56.87  & 56.261 & 56.522 & 56.217 & 54.696 & 59.174 & 56.739 & 56.478 & 57.696 \\
387   & 56.783 & 57.043 & 56.348 & 56.739 & 55.87  & 55.174 & 59.217 & 56.522 & 56.565 & 57.739 \\
388   & 57.174 & 56.783 & 56.304 & 56.87  & 55.783 & 55.174 & 59.087 & 56.609 & 56.783 & 57.696 \\
389   & 57.304 & 56.478 & 56.217 & 57.087 & 56.13  & 55.478 & 59     & 56.652 & 56.609 & 58.13  \\
390   & 57.174 & 56.435 & 56.043 & 57.478 & 56.174 & 55.783 & 58.957 & 56.783 & 56.478 & 58.174 \\
391   & 57.565 & 56.478 & 56.087 & 57.391 & 55.957 & 55.826 & 58.652 & 57.043 & 56.696 & 58.217 \\
\bottomrule\end{longtable}
\normalsize
