# Supplementary material for: Rehearsal-Free Continual Learning over Small Non-I.I.D. Batches
Source: arXiv:1907.03799 source file (2020-04-21)
Supplement: Supplementary file 10 [file 391_EWC.tex]

\subsection{EWC, NICv2 - 391}
\fontsize{8}{11}\selectfont
\begin{longtable}[c]{rgrgrgrgrgr}
\hline
Batch & Run 0  & Run 1  & Run 2  & Run 3  & Run 4  & Run 5  & Run 6  & Run 7  & Run 8  & Run 9  \\ \hline
\endfirsthead
\endhead
0     & 1.522  & 1.522  & 1.522  & 1.522  & 1.522  & 1.522  & 1.522  & 1.522  & 1.522  & 1.522  \\
1     & 13.87  & 13.826 & 13.826 & 13.87  & 13.87  & 13.826 & 13.87  & 13.826 & 13.87  & 13.826 \\
2     & 13.87  & 13.913 & 13.739 & 14.304 & 14.043 & 14.261 & 14     & 14.043 & 14.522 & 14.261 \\
3     & 14     & 13.87  & 14.13  & 14.304 & 14.478 & 14.522 & 13.957 & 13.913 & 14.261 & 14.217 \\
4     & 14     & 14.304 & 14.174 & 13.913 & 14.522 & 14.478 & 13.783 & 13.957 & 14.217 & 13.957 \\
5     & 14.348 & 14.435 & 13.957 & 14.087 & 14.217 & 14.435 & 13.783 & 13.957 & 14.261 & 14.174 \\
6     & 14.087 & 14.348 & 13.87  & 14.217 & 14.217 & 14.478 & 13.957 & 13.913 & 14.435 & 14.087 \\
7     & 14.261 & 14.217 & 13.652 & 14.652 & 14.087 & 14.783 & 13.957 & 13.696 & 14.391 & 14.087 \\
8     & 14.087 & 14.261 & 13.957 & 14.565 & 14.087 & 14.609 & 14     & 13.957 & 14.565 & 14.087 \\
9     & 14.304 & 14.261 & 14     & 14.609 & 14.087 & 14.652 & 14.174 & 13.957 & 14.739 & 14.13  \\
10    & 14.304 & 14.391 & 14.174 & 14.652 & 14     & 14.522 & 14.261 & 14.304 & 14.478 & 14.174 \\
11    & 13.87  & 14.261 & 13.957 & 14.609 & 14.043 & 14.391 & 14.391 & 14.435 & 14.478 & 14.304 \\
12    & 14.174 & 14.348 & 14.087 & 14.609 & 13.957 & 14.391 & 14.348 & 14.522 & 14.609 & 14.435 \\
13    & 14.087 & 14.348 & 14.217 & 14.565 & 14.13  & 14.391 & 13.957 & 14.652 & 14.739 & 14.304 \\
14    & 13.913 & 14.348 & 14.348 & 14.652 & 14.217 & 14.391 & 14.043 & 14.609 & 14.609 & 14.435 \\
15    & 13.826 & 14.348 & 14.652 & 14.652 & 14.261 & 14.522 & 14.043 & 14.609 & 14.609 & 14.652 \\
16    & 13.957 & 14.435 & 14.565 & 14.696 & 14.391 & 14.696 & 14.217 & 14.565 & 14.609 & 14.304 \\
17    & 13.913 & 14.435 & 14.348 & 14.783 & 14.522 & 14.739 & 14.304 & 14.783 & 14.696 & 14.087 \\
18    & 13.87  & 14.391 & 14.522 & 14.565 & 14.391 & 14.826 & 14.174 & 14.696 & 14.826 & 13.957 \\
19    & 14     & 14.348 & 14.478 & 14.652 & 14.478 & 14.609 & 14.217 & 14.609 & 14.957 & 13.826 \\
20    & 14.217 & 14.435 & 14.609 & 14.391 & 14.348 & 14.609 & 14.348 & 14.609 & 14.87  & 13.478 \\
21    & 14.391 & 14.652 & 14.478 & 14.522 & 14.522 & 14.478 & 14.348 & 14.609 & 14.826 & 13.783 \\
22    & 14.391 & 14.609 & 14.478 & 14.522 & 14.391 & 14.652 & 14.391 & 14.609 & 14.652 & 13.696 \\
23    & 14.478 & 14.565 & 14.478 & 14.565 & 14.522 & 14.609 & 14.348 & 14.652 & 14.739 & 13.478 \\
24    & 14.348 & 14.435 & 14.348 & 14.696 & 14.478 & 14.522 & 14.652 & 14.565 & 14.739 & 13.478 \\
25    & 14.478 & 14.304 & 14.391 & 14.739 & 14.478 & 14.696 & 14.609 & 14.783 & 14.739 & 13.739 \\
26    & 14.522 & 14.043 & 14.435 & 14.696 & 14.391 & 14.652 & 14.522 & 14.739 & 14.609 & 13.913 \\
27    & 14.435 & 14.217 & 14.217 & 14.478 & 14.565 & 14.652 & 14.435 & 14.696 & 14.652 & 13.957 \\
28    & 14.522 & 14.174 & 14.261 & 14.304 & 14.565 & 14.783 & 14.478 & 14.783 & 14.652 & 14.13  \\
29    & 14.522 & 14.391 & 14.435 & 14.391 & 14.478 & 14.522 & 14.435 & 14.826 & 14.739 & 14.043 \\
30    & 14.565 & 14.435 & 14.478 & 14.478 & 14.391 & 14.696 & 14.435 & 14.913 & 14.826 & 14.043 \\
31    & 14.478 & 14.304 & 14.435 & 14.609 & 14.609 & 14.696 & 14.391 & 14.783 & 14.87  & 14     \\
32    & 14.435 & 14.304 & 14.348 & 14.783 & 14.652 & 14.87  & 14.348 & 14.522 & 14.957 & 13.913 \\
33    & 14.391 & 14.348 & 14.348 & 14.783 & 14.609 & 15     & 14.391 & 14.565 & 14.957 & 13.696 \\
34    & 14.478 & 14.348 & 14.348 & 14.696 & 14.696 & 14.957 & 14.478 & 14.478 & 14.826 & 14.087 \\
35    & 14.522 & 14.435 & 14.522 & 14.826 & 14.609 & 14.957 & 14.435 & 14.87  & 14.696 & 14.217 \\
36    & 14.391 & 14.435 & 14.478 & 14.783 & 14.522 & 15.13  & 14.565 & 14.957 & 14.783 & 14.261 \\
37    & 14.391 & 14.435 & 14.261 & 14.652 & 14.435 & 14.957 & 14.522 & 14.609 & 14.783 & 14.174 \\
38    & 14.435 & 14.522 & 14.261 & 15.043 & 14.391 & 14.826 & 14.391 & 14.783 & 14.826 & 14.174 \\
39    & 14.261 & 14.565 & 14.348 & 14.957 & 14.304 & 14.913 & 14.348 & 14.478 & 14.696 & 14.304 \\
40    & 14.304 & 15     & 14.304 & 14.87  & 14.217 & 15     & 14.087 & 14.391 & 14.826 & 14.217 \\
41    & 14.261 & 15.043 & 14.261 & 14.913 & 14.348 & 14.913 & 14.391 & 14.435 & 14.826 & 14.174 \\
42    & 14.13  & 15.087 & 14.435 & 15     & 14.435 & 14.826 & 14.478 & 14.652 & 14.783 & 14.348 \\
43    & 14.13  & 15     & 14.478 & 14.957 & 14.348 & 14.783 & 14.652 & 14.696 & 14.652 & 14.348 \\
44    & 14.087 & 14.87  & 14.478 & 14.913 & 14.261 & 14.739 & 14.522 & 14.783 & 14.696 & 14.435 \\
45    & 14.174 & 14.565 & 14.304 & 15     & 14.391 & 14.696 & 14.391 & 14.783 & 14.609 & 14.348 \\
46    & 14.391 & 14.609 & 14.391 & 14.957 & 14.348 & 14.609 & 14.435 & 14.435 & 14.696 & 14.348 \\
47    & 14.478 & 14.696 & 14.217 & 14.826 & 14.261 & 14.565 & 14.522 & 14.391 & 14.565 & 14.261 \\
48    & 14.522 & 14.609 & 14.217 & 14.913 & 14.348 & 14.696 & 14.391 & 14.261 & 14.652 & 14.217 \\
49    & 14.478 & 14.391 & 14.087 & 14.913 & 14.391 & 14.652 & 14.565 & 14.435 & 14.217 & 14.217 \\
50    & 14.565 & 14.304 & 14.043 & 14.783 & 14.478 & 14.565 & 14.696 & 14.304 & 14.174 & 14.174 \\
51    & 14.652 & 14.217 & 13.913 & 14.826 & 14.652 & 14.522 & 14.652 & 14.435 & 14.217 & 14.13  \\
52    & 14.565 & 14.348 & 13.826 & 14.783 & 14.609 & 14.478 & 14.652 & 14.435 & 14.217 & 13.957 \\
53    & 14.391 & 14.478 & 14     & 15.043 & 14.609 & 14.391 & 14.565 & 14.565 & 14.348 & 14.043 \\
54    & 14.391 & 14.609 & 13.826 & 15     & 14.652 & 14.174 & 14.478 & 14.435 & 14.783 & 13.826 \\
55    & 14.348 & 14.217 & 13.652 & 15     & 14.609 & 14.174 & 14.435 & 14.565 & 14.739 & 13.826 \\
56    & 14.478 & 14.13  & 13.696 & 14.826 & 14.826 & 14.261 & 14.522 & 14.565 & 14.522 & 13.696 \\
57    & 14.435 & 14.13  & 13.783 & 14.652 & 14.696 & 14.261 & 14.348 & 14.217 & 14.522 & 13.913 \\
58    & 14.609 & 14.261 & 13.696 & 14.739 & 14.826 & 14.043 & 14.522 & 14.304 & 14.696 & 14.087 \\
59    & 14.609 & 14.217 & 13.739 & 14.609 & 14.826 & 14.261 & 14.348 & 14.348 & 14.652 & 14.217 \\
60    & 14.478 & 14.13  & 13.783 & 14.565 & 14.565 & 14.391 & 14.348 & 14.13  & 14.565 & 14.13  \\
61    & 14.565 & 14.217 & 13.739 & 14.609 & 14.696 & 14.261 & 14.261 & 14.087 & 14.435 & 14.174 \\
62    & 14.652 & 14.261 & 14.087 & 14.652 & 14.565 & 14.348 & 14.261 & 14.043 & 14.304 & 14.043 \\
63    & 14.652 & 14.087 & 13.913 & 14.565 & 14.652 & 14.217 & 14.391 & 14     & 14.391 & 14.043 \\
64    & 14.652 & 14.13  & 13.913 & 14.565 & 14.739 & 14.348 & 14.478 & 14     & 14.217 & 13.652 \\
65    & 14.783 & 14.217 & 13.826 & 14.435 & 14.739 & 14.174 & 14.348 & 14.13  & 14.13  & 13.565 \\
66    & 14.739 & 14     & 13.826 & 14.435 & 14.609 & 14.261 & 14.261 & 14.087 & 14.174 & 13.435 \\
67    & 14.696 & 13.826 & 13.87  & 14.478 & 14.522 & 14.217 & 14.261 & 14.13  & 14.13  & 13.348 \\
68    & 14.522 & 13.87  & 13.696 & 14.391 & 14.478 & 14.217 & 14.043 & 14.087 & 14.174 & 13.391 \\
69    & 14.609 & 13.826 & 13.696 & 14.348 & 14.13  & 14.174 & 13.957 & 14.13  & 14.087 & 13.304 \\
70    & 14.565 & 13.696 & 13.478 & 14.348 & 13.913 & 14.217 & 14     & 14.174 & 14.087 & 13.261 \\
71    & 14.522 & 13.652 & 13.522 & 14.174 & 13.957 & 14.13  & 14     & 14.13  & 14.087 & 13.348 \\
72    & 14.043 & 13.565 & 13.478 & 14.174 & 14.087 & 14.217 & 14     & 14.13  & 14.391 & 13.304 \\
73    & 13.913 & 13.652 & 13.435 & 14.087 & 14.13  & 14.261 & 13.87  & 14     & 14.391 & 13.217 \\
74    & 13.957 & 13.739 & 13.565 & 14.217 & 14.087 & 13.957 & 13.739 & 14.13  & 14.435 & 13.652 \\
75    & 13.913 & 13.783 & 13.565 & 14.13  & 14.043 & 14     & 13.739 & 14.087 & 14.174 & 13.565 \\
76    & 13.783 & 13.783 & 13.609 & 14.261 & 13.913 & 14     & 13.913 & 14.217 & 14.217 & 13.565 \\
77    & 13.913 & 13.696 & 13.739 & 14.217 & 13.913 & 14.087 & 14     & 14.13  & 14.261 & 13.478 \\
78    & 13.87  & 13.826 & 13.565 & 14.043 & 14     & 14.174 & 13.957 & 14.304 & 14.391 & 13.652 \\
79    & 13.739 & 13.565 & 13.609 & 14.13  & 13.87  & 14.174 & 14.087 & 14.174 & 14.304 & 13.739 \\
80    & 13.783 & 13.609 & 13.783 & 14.217 & 14     & 14     & 14.087 & 14.13  & 14.391 & 13.565 \\
81    & 13.696 & 13.609 & 13.87  & 14.217 & 14.087 & 14     & 14.043 & 14.174 & 14.391 & 13.435 \\
82    & 13.696 & 13.478 & 13.739 & 14.13  & 14.217 & 13.957 & 14.043 & 14     & 14.391 & 13.435 \\
83    & 13.696 & 13.478 & 13.783 & 14.13  & 13.957 & 14     & 13.87  & 14     & 14.391 & 13.565 \\
84    & 13.826 & 13.348 & 13.478 & 14.13  & 13.957 & 14     & 13.826 & 13.957 & 14.304 & 13.522 \\
85    & 13.783 & 13.304 & 13.435 & 14.087 & 13.913 & 14     & 13.652 & 13.696 & 14.261 & 13.783 \\
86    & 13.783 & 13.478 & 13.435 & 13.913 & 13.87  & 14     & 13.565 & 13.565 & 14.391 & 13.652 \\
87    & 13.739 & 13.261 & 13.304 & 13.87  & 13.783 & 13.913 & 13.652 & 13.522 & 14.348 & 13.522 \\
88    & 13.783 & 13.043 & 13.261 & 13.739 & 13.826 & 13.913 & 13.304 & 13.522 & 14.391 & 13.478 \\
89    & 13.87  & 13.13  & 13.261 & 13.783 & 13.87  & 13.87  & 13.348 & 13.435 & 14.261 & 13.522 \\
90    & 13.87  & 13.261 & 13.304 & 13.696 & 13.783 & 14     & 13.261 & 13.478 & 14.087 & 13.696 \\
91    & 14.087 & 13.217 & 13.348 & 13.739 & 13.739 & 13.913 & 13.261 & 13.478 & 14.261 & 13.652 \\
92    & 14.043 & 13.304 & 13.261 & 13.609 & 13.826 & 13.652 & 13.391 & 13.435 & 14.304 & 13.609 \\
93    & 14.087 & 13.304 & 13.217 & 13.609 & 13.696 & 13.565 & 13.174 & 13.391 & 14.174 & 13.478 \\
94    & 14.043 & 13.348 & 13.217 & 13.565 & 13.652 & 13.565 & 13.478 & 13.478 & 14.217 & 13.565 \\
95    & 13.957 & 13.261 & 13.435 & 13.478 & 13.609 & 13.696 & 13.435 & 13.391 & 14     & 13.565 \\
96    & 14.043 & 13.391 & 13.304 & 13.565 & 13.565 & 13.696 & 13.435 & 13.435 & 14     & 13.478 \\
97    & 14.087 & 13.217 & 13.435 & 13.478 & 13.478 & 13.826 & 13.348 & 13.87  & 14.087 & 13.609 \\
98    & 13.826 & 12.913 & 13.652 & 13.478 & 13.478 & 13.696 & 13.174 & 13.87  & 14.087 & 13.609 \\
99    & 13.957 & 12.696 & 13.696 & 13.391 & 13.435 & 13.652 & 13.478 & 13.87  & 14.087 & 13.696 \\
100   & 14.13  & 12.87  & 13.435 & 13.217 & 13.435 & 13.652 & 13.348 & 14.13  & 14.13  & 13.435 \\
101   & 14.13  & 12.783 & 13.348 & 13.348 & 13.304 & 13.739 & 13.261 & 14.217 & 14.13  & 13.261 \\
102   & 14     & 12.783 & 13.348 & 13.261 & 13.261 & 13.609 & 13.478 & 14.217 & 14.043 & 13.391 \\
103   & 14.043 & 12.783 & 13.391 & 13.174 & 13.391 & 13.522 & 13.435 & 14.087 & 14     & 13.478 \\
104   & 13.783 & 12.565 & 13.435 & 13.087 & 13.435 & 13.522 & 13.391 & 14     & 14     & 13.348 \\
105   & 13.696 & 12.652 & 13.565 & 12.826 & 13.391 & 13.565 & 13.391 & 13.696 & 14.087 & 13.522 \\
106   & 13.652 & 12.696 & 13.304 & 12.826 & 13.478 & 13.522 & 13.435 & 13.609 & 14     & 13.304 \\
107   & 13.609 & 12.739 & 13.348 & 12.87  & 13.304 & 13.348 & 13.609 & 13.826 & 13.957 & 13.217 \\
108   & 13.522 & 12.783 & 13.217 & 12.87  & 13.261 & 13.478 & 13.348 & 13.826 & 13.957 & 13.043 \\
109   & 13.565 & 12.87  & 13.174 & 12.739 & 13.261 & 13.565 & 13.217 & 13.739 & 13.957 & 12.957 \\
110   & 13.609 & 12.739 & 13.217 & 12.652 & 13.304 & 13.565 & 13.043 & 13.696 & 13.783 & 12.826 \\
111   & 13.652 & 12.783 & 13.348 & 12.652 & 13.304 & 13.391 & 13.217 & 13.783 & 13.783 & 12.913 \\
112   & 13.696 & 12.696 & 13.261 & 12.652 & 13.348 & 13.348 & 13.087 & 13.783 & 13.565 & 12.913 \\
113   & 13.565 & 12.87  & 13.391 & 12.696 & 13.478 & 13.348 & 13.043 & 13.739 & 13.565 & 13.043 \\
114   & 13.435 & 12.913 & 13.435 & 12.652 & 13.391 & 13.261 & 13.043 & 13.696 & 13.522 & 12.913 \\
115   & 13.348 & 12.913 & 13.304 & 12.652 & 13.435 & 13.13  & 13     & 13.696 & 13.565 & 12.87  \\
116   & 13.348 & 12.783 & 13.217 & 12.609 & 13.348 & 13.13  & 12.913 & 13.652 & 13.391 & 12.87  \\
117   & 13.217 & 12.739 & 13.348 & 12.522 & 13.304 & 13.174 & 12.652 & 13.652 & 13.391 & 12.957 \\
118   & 13.13  & 12.696 & 13.478 & 12.565 & 13     & 13.043 & 12.739 & 13.478 & 13.435 & 12.826 \\
119   & 13.261 & 12.609 & 13.435 & 12.609 & 13.087 & 13.043 & 12.739 & 13.435 & 13.435 & 12.87  \\
120   & 13.304 & 12.565 & 13.565 & 12.348 & 13.087 & 13.13  & 12.739 & 13.478 & 13.217 & 12.913 \\
121   & 13.261 & 12.696 & 13.609 & 12.304 & 13.043 & 13.174 & 12.739 & 13.478 & 13.217 & 12.957 \\
122   & 13.304 & 12.652 & 13.609 & 12.348 & 12.783 & 13.261 & 12.826 & 13.478 & 13.217 & 12.783 \\
123   & 13     & 12.565 & 13.609 & 12.348 & 12.913 & 12.826 & 12.826 & 13.478 & 13.391 & 12.826 \\
124   & 12.739 & 12.391 & 13.652 & 12.348 & 13     & 12.957 & 12.87  & 13.478 & 13.304 & 12.565 \\
125   & 12.913 & 12.478 & 13.783 & 12.435 & 13.043 & 12.913 & 12.913 & 13.478 & 13.174 & 12.87  \\
126   & 12.957 & 12.478 & 13.652 & 12.348 & 13.13  & 12.87  & 12.913 & 13.478 & 13.217 & 13.043 \\
127   & 12.913 & 12.348 & 13.478 & 12.478 & 13     & 12.783 & 12.826 & 13.565 & 13.261 & 13.043 \\
128   & 13     & 12.304 & 13.391 & 12.348 & 13     & 12.783 & 12.826 & 13.565 & 13.261 & 13.13  \\
129   & 12.957 & 12.522 & 13.435 & 12.174 & 13     & 12.87  & 12.783 & 13.435 & 13.304 & 13.043 \\
130   & 13     & 12.435 & 13.522 & 12.087 & 13.043 & 12.826 & 12.913 & 13.435 & 13.13  & 12.783 \\
131   & 13.043 & 12.478 & 13.478 & 12.13  & 13     & 12.522 & 12.826 & 13.522 & 13.13  & 12.913 \\
132   & 13.13  & 12.348 & 13.565 & 12.087 & 12.739 & 12.522 & 12.783 & 13.391 & 13     & 13     \\
133   & 12.522 & 12.391 & 13.696 & 11.957 & 13     & 12.696 & 12.696 & 13.478 & 12.957 & 13.043 \\
134   & 12.478 & 12.348 & 13.783 & 12.13  & 12.913 & 12.696 & 12.783 & 13.652 & 12.913 & 13     \\
135   & 12.522 & 12.261 & 13.783 & 11.565 & 12.913 & 12.652 & 12.739 & 13.696 & 12.913 & 12.826 \\
136   & 12.565 & 12.391 & 13.739 & 11.739 & 12.609 & 12.696 & 12.696 & 13.609 & 13     & 12.87  \\
137   & 12.348 & 12.304 & 13.435 & 11.826 & 12.739 & 12.565 & 12.652 & 13.478 & 13.087 & 12.783 \\
138   & 12.261 & 12.391 & 13.435 & 11.696 & 12.652 & 12.652 & 12.739 & 13.478 & 13.217 & 12.652 \\
139   & 12.304 & 12.522 & 13.565 & 11.739 & 12.696 & 12.565 & 12.87  & 13.565 & 13.087 & 12.652 \\
140   & 12.261 & 12.696 & 13.609 & 11.696 & 12.522 & 12.478 & 12.87  & 13.478 & 13.217 & 12.609 \\
141   & 12.391 & 12.391 & 13.652 & 11.783 & 12.652 & 12.391 & 12.522 & 13.435 & 12.957 & 12.609 \\
142   & 12.217 & 12.435 & 13.565 & 11.826 & 12.565 & 12.565 & 12.739 & 13.522 & 12.826 & 12.652 \\
143   & 12.217 & 12.391 & 13.522 & 11.739 & 12.435 & 12.348 & 12.609 & 13.478 & 13.217 & 12.522 \\
144   & 12.087 & 12.435 & 13.478 & 11.913 & 12.304 & 12.261 & 12.478 & 13.565 & 13.087 & 12.522 \\
145   & 12.13  & 12.391 & 13.478 & 11.739 & 12.391 & 12.304 & 12.652 & 13.522 & 13.043 & 12.522 \\
146   & 12.13  & 12.478 & 13.348 & 12.174 & 12.522 & 12.304 & 12.652 & 13.522 & 12.87  & 12.565 \\
147   & 12.174 & 12.478 & 13.304 & 12.304 & 12.652 & 12.217 & 12.652 & 13.435 & 12.696 & 12.609 \\
148   & 12.261 & 12.478 & 13.217 & 12.261 & 12.696 & 12.391 & 12.696 & 13.217 & 12.826 & 12.522 \\
149   & 12.478 & 12.522 & 13.217 & 12.348 & 12.783 & 12.261 & 12.565 & 13.174 & 12.783 & 12.739 \\
150   & 12.174 & 12.565 & 13.043 & 12.348 & 12.87  & 12.348 & 12.609 & 13.043 & 12.522 & 12.565 \\
151   & 12.087 & 12.478 & 12.783 & 12.348 & 13.087 & 12.087 & 12.696 & 12.913 & 12.261 & 12.739 \\
152   & 12.13  & 12.478 & 12.696 & 12.391 & 12.957 & 12.13  & 12.609 & 12.87  & 12.217 & 12.565 \\
153   & 12.304 & 12.391 & 12.609 & 12.391 & 12.913 & 12     & 12.609 & 12.739 & 12.217 & 12.522 \\
154   & 12.261 & 12.391 & 12.696 & 12.217 & 12.957 & 12.13  & 12.609 & 12.652 & 12.304 & 12.348 \\
155   & 12     & 12.435 & 12.696 & 12.13  & 12.87  & 12.087 & 12.391 & 12.87  & 12.478 & 12.391 \\
156   & 12.13  & 12.478 & 12.565 & 12.174 & 13.043 & 12     & 12.652 & 12.696 & 12.348 & 12.435 \\
157   & 12.087 & 12.435 & 12.783 & 12.217 & 13.13  & 12     & 12.652 & 12.565 & 12.435 & 12.522 \\
158   & 11.739 & 12.348 & 12.609 & 12.261 & 13.087 & 12     & 12.696 & 12.696 & 12.565 & 12.609 \\
159   & 11.696 & 12.304 & 12.348 & 12.435 & 12.87  & 11.957 & 12.609 & 12.478 & 12.783 & 12.522 \\
160   & 11.783 & 12.348 & 12.304 & 12.478 & 12.826 & 12.043 & 12.304 & 12.609 & 12.696 & 12.478 \\
161   & 11.913 & 12.087 & 12.261 & 12.348 & 12.913 & 12.13  & 12.13  & 12.217 & 12.696 & 12.522 \\
162   & 11.826 & 11.957 & 12.087 & 12.304 & 12.957 & 11.609 & 12.087 & 12.13  & 12.652 & 12.435 \\
163   & 11.739 & 11.826 & 12.174 & 12.391 & 12.87  & 11.826 & 12.087 & 12.087 & 12.609 & 12.435 \\
164   & 11.609 & 11.826 & 12.348 & 12.391 & 12.522 & 11.913 & 12.174 & 12.087 & 12.652 & 12.391 \\
165   & 11.609 & 11.913 & 12.217 & 12.391 & 12.478 & 11.826 & 12.217 & 12.043 & 12.609 & 12.391 \\
166   & 11.696 & 11.957 & 12.348 & 12.217 & 12.739 & 11.783 & 12.13  & 11.913 & 12.652 & 12.478 \\
167   & 11.478 & 12     & 12.261 & 11.913 & 12.739 & 11.913 & 12.13  & 11.957 & 12.783 & 12.391 \\
168   & 11.652 & 12.174 & 12.13  & 12.087 & 12.783 & 11.913 & 12     & 11.913 & 12.565 & 12.478 \\
169   & 11.261 & 11.957 & 12.043 & 12.043 & 12.87  & 11.87  & 11.957 & 11.783 & 12.609 & 12.652 \\
170   & 11.304 & 12.043 & 12.043 & 12.174 & 12.826 & 11.783 & 12.043 & 11.826 & 12.739 & 12.565 \\
171   & 11.522 & 12     & 12     & 12.13  & 12.739 & 11.826 & 12.087 & 11.913 & 12.739 & 12.609 \\
172   & 11.391 & 12.217 & 11.522 & 12     & 12.739 & 11.957 & 11.957 & 11.87  & 12.609 & 12.565 \\
173   & 11.435 & 12.174 & 11.609 & 12.043 & 12.609 & 11.957 & 12.087 & 11.957 & 12.609 & 12.391 \\
174   & 11.652 & 12.174 & 11.87  & 11.957 & 12.696 & 11.913 & 12.13  & 11.87  & 12.478 & 12.478 \\
175   & 11.696 & 12.174 & 11.87  & 11.957 & 12.739 & 12     & 12     & 11.826 & 12.435 & 12.435 \\
176   & 11.739 & 12.261 & 11.826 & 11.739 & 12.87  & 11.696 & 11.913 & 11.739 & 12.565 & 12.391 \\
177   & 11.739 & 12.217 & 11.696 & 11.783 & 12.826 & 11.652 & 11.913 & 11.913 & 12.696 & 12.391 \\
178   & 11.783 & 12.13  & 11.652 & 11.739 & 12.696 & 11.609 & 12     & 12.043 & 12.609 & 12.304 \\
179   & 11.609 & 12     & 11.609 & 11.565 & 12.565 & 11.609 & 12.217 & 12     & 12.435 & 12.348 \\
180   & 11.391 & 12     & 11.478 & 11.522 & 12.652 & 11.522 & 12.043 & 11.783 & 12.522 & 12.217 \\
181   & 11.348 & 12     & 11.522 & 11.565 & 12.522 & 11.609 & 12     & 11.739 & 12.565 & 12.217 \\
182   & 11.348 & 11.826 & 11.435 & 11.652 & 12.391 & 11.565 & 11.957 & 11.87  & 12.609 & 11.957 \\
183   & 11.304 & 11.913 & 11.435 & 11.565 & 12.391 & 11.435 & 11.957 & 11.609 & 12.565 & 11.739 \\
184   & 11.217 & 11.87  & 11.391 & 11.739 & 12.435 & 11.435 & 11.913 & 11.652 & 12.478 & 11.87  \\
185   & 11.217 & 11.913 & 11.522 & 11.739 & 12.13  & 11.435 & 11.957 & 11.652 & 12.435 & 11.913 \\
186   & 11.174 & 11.957 & 11.435 & 11.652 & 12.174 & 11.304 & 11.696 & 11.652 & 12.391 & 12.304 \\
187   & 11.391 & 11.783 & 11.304 & 11.696 & 12.174 & 11.261 & 11.739 & 11.478 & 12.348 & 12.043 \\
188   & 11.391 & 11.696 & 11.391 & 11.739 & 12.13  & 11.304 & 11.783 & 11.391 & 12.217 & 12     \\
189   & 11.13  & 11.696 & 11.478 & 11.652 & 12.174 & 11.261 & 11.826 & 11.304 & 12.087 & 12.043 \\
190   & 11.348 & 11.652 & 11.304 & 11.826 & 12.087 & 11.304 & 11.391 & 11.261 & 12.13  & 11.87  \\
191   & 11.391 & 11.696 & 11.391 & 11.826 & 12.261 & 11.522 & 11.348 & 11.261 & 11.826 & 11.913 \\
192   & 11.261 & 11.565 & 11.391 & 11.913 & 12.174 & 11.522 & 11.391 & 11.217 & 11.957 & 11.87  \\
193   & 10.913 & 11.478 & 11.087 & 11.913 & 12.13  & 11.13  & 11.391 & 11.174 & 11.913 & 11.913 \\
194   & 11.087 & 11.304 & 11     & 11.826 & 12     & 11.043 & 11.435 & 11.13  & 11.652 & 11.957 \\
195   & 10.913 & 11.391 & 11.13  & 11.652 & 12.13  & 11.174 & 11.217 & 11.043 & 11.652 & 12     \\
196   & 11.087 & 11.348 & 11.217 & 11.696 & 12.13  & 11.087 & 11.522 & 11     & 11.609 & 11.913 \\
197   & 10.913 & 11.391 & 11     & 11.565 & 12.174 & 11.043 & 11.609 & 10.87  & 11.478 & 11.739 \\
198   & 10.478 & 11.522 & 10.87  & 11.435 & 12.13  & 10.826 & 11.478 & 10.739 & 11.565 & 11.478 \\
199   & 10.522 & 11.609 & 10.652 & 11.522 & 12.348 & 10.739 & 11.522 & 10.652 & 11.609 & 11.435 \\
200   & 10.609 & 11.565 & 10.957 & 11.652 & 12.435 & 11.087 & 11.652 & 10.478 & 11.565 & 11.435 \\
201   & 10.652 & 11.565 & 10.913 & 11.478 & 12.435 & 11.304 & 11.609 & 10.522 & 11.478 & 11.478 \\
202   & 10.565 & 11.435 & 10.913 & 11.565 & 12.348 & 11.174 & 11.609 & 10.565 & 11.478 & 11.304 \\
203   & 10.348 & 11.043 & 11.174 & 11.435 & 12.13  & 11.13  & 11.652 & 10.391 & 11.522 & 11.435 \\
204   & 10.304 & 11.087 & 11     & 11.478 & 12.087 & 11.217 & 11.652 & 10.304 & 11.478 & 11.391 \\
205   & 10.348 & 11     & 11     & 11.217 & 12.087 & 11.043 & 11.696 & 10.348 & 11.391 & 11.174 \\
206   & 10.348 & 10.957 & 10.739 & 11.174 & 12.13  & 11     & 11.696 & 10.261 & 11.348 & 11.174 \\
207   & 10.348 & 10.826 & 10.696 & 11.087 & 12.261 & 10.696 & 11.696 & 10.304 & 11.13  & 11.217 \\
208   & 10.522 & 10.652 & 10.652 & 10.957 & 12.261 & 10.739 & 11.739 & 10.348 & 11.13  & 11.217 \\
209   & 10.609 & 10.609 & 10.696 & 11.13  & 12.217 & 10.565 & 11.783 & 10.13  & 11.217 & 11.304 \\
210   & 10.348 & 10.478 & 10.783 & 10.957 & 12.261 & 10.696 & 11.739 & 10.13  & 11.261 & 11.391 \\
211   & 10.217 & 10.565 & 10.13  & 10.783 & 12.174 & 10.565 & 11.565 & 10.391 & 11.043 & 11.391 \\
212   & 10.348 & 10.652 & 10.217 & 10.739 & 11.913 & 10.739 & 11.435 & 10.478 & 11.174 & 11.435 \\
213   & 10.391 & 10.739 & 10.174 & 10.739 & 11.87  & 10.826 & 11.435 & 10.522 & 11.174 & 11.304 \\
214   & 10.043 & 10.609 & 10     & 10.391 & 12     & 10.739 & 11.217 & 10.391 & 11     & 11.043 \\
215   & 10     & 10.435 & 10.13  & 10.478 & 11.913 & 10.565 & 11.217 & 10.435 & 10.87  & 11     \\
216   & 10.043 & 10.174 & 10.435 & 10.739 & 11.739 & 10.609 & 11.174 & 10.391 & 11.043 & 10.913 \\
217   & 10     & 10.304 & 10.435 & 10.522 & 11.696 & 10.435 & 11.174 & 10.739 & 10.87  & 10.87  \\
218   & 10.043 & 10.478 & 10.304 & 10.783 & 11.783 & 10.565 & 11.217 & 10.565 & 10.826 & 10.739 \\
219   & 9.913  & 10.391 & 10.174 & 10.87  & 11.87  & 10.565 & 10.87  & 10.565 & 10.87  & 10.478 \\
220   & 9.87   & 10.478 & 10.087 & 10.826 & 11.739 & 10.609 & 10.87  & 10.609 & 10.87  & 10.478 \\
221   & 9.913  & 10.304 & 10.174 & 10.652 & 11.739 & 10.522 & 11     & 10.609 & 10.783 & 10.217 \\
222   & 9.87   & 10.304 & 10.217 & 10.565 & 11.696 & 10.565 & 10.957 & 10.696 & 10.652 & 10.304 \\
223   & 9.609  & 10.304 & 10.217 & 10.565 & 11.696 & 10.13  & 10.913 & 9.826  & 10.435 & 10.261 \\
224   & 9.478  & 10.435 & 10.217 & 10.391 & 11.652 & 9.957  & 10.783 & 9.522  & 10.565 & 10.261 \\
225   & 9.391  & 9.652  & 10.13  & 10.13  & 11.696 & 10.174 & 10.87  & 9.522  & 10.739 & 10.348 \\
226   & 9.435  & 9.565  & 10.217 & 10.043 & 11.696 & 10.13  & 10.913 & 9.565  & 10.696 & 10.391 \\
227   & 9.609  & 9.348  & 10.391 & 10.13  & 11.783 & 10.087 & 11.043 & 9.348  & 10.652 & 10.391 \\
228   & 9.217  & 9.348  & 10.522 & 10.043 & 11.783 & 10.043 & 10.957 & 9.565  & 10.565 & 10.391 \\
229   & 9.261  & 9.435  & 10.696 & 9.957  & 11.783 & 10     & 10.957 & 9.565  & 10.783 & 10.435 \\
230   & 9.261  & 9.522  & 10.609 & 10     & 11.783 & 10.087 & 10.913 & 9.435  & 10.609 & 10.174 \\
231   & 9.261  & 9.522  & 10.348 & 9.783  & 11.87  & 9.957  & 10.826 & 9.522  & 10.304 & 9.913  \\
232   & 9.174  & 9.565  & 10.522 & 9.87   & 11.957 & 10     & 10.826 & 9.478  & 10.435 & 10.043 \\
233   & 9.217  & 9.609  & 10.304 & 9.783  & 11.87  & 9.87   & 10.739 & 9.478  & 10.609 & 10.087 \\
234   & 9.087  & 9.435  & 10.261 & 9.739  & 12     & 9.652  & 10.652 & 9.304  & 10.522 & 10.043 \\
235   & 9.13   & 9.391  & 10.304 & 9.739  & 12     & 9.739  & 10.696 & 9.435  & 10.348 & 9.87   \\
236   & 9.348  & 9.304  & 10.087 & 9.783  & 12.043 & 9.565  & 10.609 & 9.478  & 10.348 & 9.826  \\
237   & 9.348  & 9.348  & 10     & 9.783  & 11.913 & 9.522  & 10.565 & 9.478  & 10.261 & 9.913  \\
238   & 9.391  & 9.304  & 10.174 & 9.739  & 11.957 & 9.522  & 10.13  & 9.13   & 10.174 & 10     \\
239   & 9.565  & 9.304  & 10.217 & 9.913  & 12     & 9.261  & 9.957  & 9.043  & 10.217 & 9.913  \\
240   & 9.609  & 9.174  & 10.304 & 10.087 & 12.087 & 9.261  & 10.174 & 9.043  & 10.13  & 9.957  \\
241   & 9.696  & 9.304  & 10.304 & 9.739  & 11.826 & 9.348  & 10.174 & 9.13   & 10.087 & 9.87   \\
242   & 9.652  & 9.348  & 10.391 & 9.391  & 11.87  & 9.435  & 10.217 & 8.609  & 9.913  & 9.957  \\
243   & 9.696  & 9.304  & 10.304 & 9.478  & 11.783 & 9.217  & 10     & 8.522  & 9.87   & 9.826  \\
244   & 9.652  & 9.348  & 10.391 & 9.783  & 11.913 & 9.043  & 10.043 & 8.609  & 9.87   & 9.957  \\
245   & 10.043 & 9.261  & 10.13  & 9.957  & 11.913 & 9.087  & 9.87   & 8.609  & 9.696  & 9.739  \\
246   & 9.913  & 8.913  & 10     & 9.87   & 12.043 & 9.174  & 10.13  & 8.609  & 9.652  & 9.522  \\
247   & 10     & 8.913  & 10.13  & 9.696  & 12.217 & 9.261  & 9.739  & 8.522  & 9.522  & 9.609  \\
248   & 10     & 8.348  & 10.217 & 9.609  & 11.913 & 8.957  & 9.652  & 8.522  & 9.261  & 9.783  \\
249   & 9.826  & 8.391  & 10.217 & 9.826  & 11.957 & 9      & 9.913  & 8.565  & 9.174  & 10.043 \\
250   & 9.957  & 8.435  & 9.957  & 9.913  & 11.783 & 9.13   & 10     & 8.478  & 9.13   & 9.783  \\
251   & 10.174 & 8.435  & 9.957  & 9.87   & 11.652 & 9.13   & 9.87   & 8.478  & 9.261  & 9.913  \\
252   & 10.043 & 8.435  & 10.087 & 9.739  & 11.696 & 9.261  & 9.783  & 8.435  & 9.304  & 10.13  \\
253   & 9.87   & 8.565  & 10.043 & 9.913  & 11.522 & 9.217  & 9.957  & 8.391  & 9.565  & 10.13  \\
254   & 9.826  & 8.652  & 10.261 & 9.87   & 11.478 & 9.174  & 10.13  & 8.261  & 9.739  & 9.957  \\
255   & 9.652  & 8.609  & 10.217 & 9.87   & 11.478 & 9.087  & 9.957  & 8.13   & 9.696  & 9.913  \\
256   & 9.739  & 8.739  & 10.087 & 9.652  & 11.565 & 8.957  & 9.87   & 8.13   & 9.565  & 9.609  \\
257   & 9.739  & 8.739  & 10.13  & 9.696  & 11.304 & 9      & 9.913  & 7.87   & 9.609  & 9.478  \\
258   & 9.783  & 8.696  & 9.87   & 9.565  & 11.174 & 9.087  & 10     & 7.739  & 9.391  & 9.391  \\
259   & 9.739  & 8.696  & 9.783  & 9.435  & 11.043 & 9.043  & 9.957  & 7.609  & 9.478  & 8.826  \\
260   & 9.696  & 8.565  & 9.739  & 9.391  & 10.957 & 9.043  & 9.913  & 7.87   & 9.522  & 8.696  \\
261   & 9.652  & 8.565  & 9.391  & 9.478  & 11.174 & 8.913  & 10.043 & 7.826  & 9.565  & 8.739  \\
262   & 9.217  & 8.478  & 9.478  & 9.478  & 11.261 & 8.826  & 10.043 & 7.957  & 9.391  & 8.957  \\
263   & 9.304  & 8.348  & 9.304  & 9.696  & 11     & 8.783  & 10.13  & 7.739  & 9.304  & 9.043  \\
264   & 9.391  & 8.174  & 9.261  & 9.652  & 10.826 & 8.696  & 10.174 & 7.609  & 9.043  & 8.696  \\
265   & 9.261  & 8.261  & 9.348  & 9.609  & 10.957 & 8.478  & 10     & 7.652  & 9.043  & 8.696  \\
266   & 9.217  & 8.348  & 9.261  & 9.609  & 10.913 & 8.478  & 10     & 7.696  & 9      & 8.739  \\
267   & 9.217  & 8.391  & 9.304  & 9.478  & 11     & 8.217  & 10.13  & 7.739  & 9.087  & 8.522  \\
268   & 9.13   & 8.391  & 9.348  & 9.609  & 11.261 & 8.217  & 10.043 & 7.522  & 9.304  & 8.565  \\
269   & 9.087  & 8.478  & 9.435  & 9.565  & 11.217 & 8.565  & 10.13  & 7.435  & 9.391  & 8.609  \\
270   & 9.087  & 8.478  & 9.348  & 9.391  & 11.304 & 8.652  & 10     & 7.696  & 9.522  & 8.739  \\
271   & 8.696  & 8.522  & 9.304  & 9.391  & 10.957 & 8.652  & 10.043 & 7.739  & 9.261  & 8.783  \\
272   & 8.478  & 8.261  & 9.304  & 9.478  & 10.87  & 8.609  & 9.87   & 7.696  & 9.087  & 8.783  \\
273   & 8.565  & 8.304  & 9.261  & 9.609  & 10.652 & 8.652  & 9.826  & 7.739  & 8.87   & 8.739  \\
274   & 8.478  & 8.522  & 9.348  & 9.652  & 10.652 & 8.652  & 9.739  & 7.696  & 8.826  & 8.826  \\
275   & 8.565  & 8.348  & 9.348  & 9.522  & 10.565 & 8.435  & 9.696  & 7.652  & 8.696  & 8.696  \\
276   & 8.478  & 8.522  & 9.348  & 9.391  & 10.522 & 8.565  & 9.652  & 7.609  & 8.696  & 8.826  \\
277   & 8.478  & 8.478  & 9.478  & 9.435  & 10.522 & 8.522  & 9.261  & 7.739  & 8.696  & 8.913  \\
278   & 8.217  & 8.652  & 9.391  & 9.739  & 10.217 & 8.696  & 8.957  & 7.609  & 8.739  & 9      \\
279   & 8.304  & 8.783  & 9.348  & 9.783  & 10.174 & 8.696  & 9.261  & 7.696  & 8.826  & 8.957  \\
280   & 8.043  & 8.652  & 9.217  & 9.826  & 10.348 & 8.783  & 9.391  & 7.696  & 8.478  & 8.696  \\
281   & 8.217  & 8.652  & 9.174  & 9.913  & 10.174 & 8.739  & 9.348  & 7.652  & 8.391  & 8.522  \\
282   & 8.13   & 8.826  & 9.174  & 10.087 & 10.304 & 8.652  & 9.261  & 7.478  & 8.217  & 8.391  \\
283   & 8.174  & 8.783  & 9.087  & 9.957  & 10.174 & 8.348  & 9.435  & 7.435  & 8.217  & 8.478  \\
284   & 8.217  & 8.913  & 8.957  & 9.739  & 10     & 8.478  & 9.391  & 7.435  & 8.261  & 8.522  \\
285   & 8.13   & 8.826  & 8.913  & 9.696  & 9.913  & 8.261  & 9.391  & 7.348  & 8.261  & 8.522  \\
286   & 8.174  & 8.696  & 8.913  & 9.696  & 9.957  & 8.304  & 9.565  & 7.522  & 8.043  & 8.522  \\
287   & 8      & 8.957  & 8.957  & 9.696  & 10.174 & 8.348  & 9.304  & 7.391  & 8.043  & 8.652  \\
288   & 8.043  & 8.87   & 9.304  & 9.826  & 9.957  & 8.304  & 9.348  & 7.261  & 7.783  & 8.609  \\
289   & 8      & 8.783  & 9.348  & 9.913  & 9.87   & 8.261  & 9.217  & 7.174  & 7.783  & 8.652  \\
290   & 7.87   & 8.609  & 9.348  & 9.696  & 9.87   & 8.043  & 9.174  & 7.174  & 7.87   & 8.739  \\
291   & 7.87   & 8.696  & 9.348  & 9.783  & 9.957  & 7.957  & 9.217  & 7.217  & 7.783  & 8.565  \\
292   & 7.87   & 8.87   & 9.609  & 9.913  & 9.652  & 7.957  & 9.087  & 6.957  & 7.739  & 8.391  \\
293   & 8.174  & 8.913  & 9.609  & 10.087 & 9.609  & 8      & 8.783  & 6.87   & 7.783  & 8.348  \\
294   & 8.043  & 8.739  & 9.522  & 9.913  & 9.174  & 7.913  & 8.696  & 6.739  & 7.652  & 8.391  \\
295   & 7.826  & 8.783  & 9.391  & 9.783  & 9.261  & 8.043  & 8.609  & 6.87   & 7.609  & 8.435  \\
296   & 7.826  & 8.87   & 9.304  & 9.609  & 9.217  & 8.261  & 8.609  & 6.913  & 7.826  & 8.478  \\
297   & 7.826  & 8.957  & 9.261  & 9.696  & 9.217  & 8.304  & 8.565  & 6.87   & 7.783  & 8.261  \\
298   & 8      & 8.783  & 9.217  & 9.739  & 9.13   & 8.478  & 8.783  & 6.783  & 7.652  & 8.217  \\
299   & 7.957  & 8.913  & 9.087  & 9.652  & 9.348  & 8.217  & 8.783  & 6.696  & 7.609  & 8.217  \\
300   & 8.13   & 9      & 9      & 9.696  & 9.261  & 8.261  & 8.826  & 6.696  & 7.478  & 8.522  \\
301   & 8.13   & 8.957  & 9.435  & 9.696  & 9.478  & 8.478  & 8.348  & 6.739  & 7.478  & 8.435  \\
302   & 8.217  & 8.913  & 9.261  & 9.609  & 9.391  & 8.217  & 8.348  & 6.783  & 7.435  & 8.609  \\
303   & 8.174  & 8.957  & 9.391  & 9.435  & 9.435  & 8.435  & 8.522  & 6.87   & 7.304  & 8.565  \\
304   & 8.087  & 8.913  & 9.783  & 9.348  & 9.435  & 8.304  & 8.609  & 6.783  & 7.174  & 8.435  \\
305   & 8.13   & 8.87   & 9.783  & 9.217  & 9.565  & 8.609  & 8.826  & 7.174  & 7.13   & 8.522  \\
306   & 8.217  & 8.957  & 9.522  & 9.174  & 9.739  & 8.696  & 8.826  & 7.391  & 7.304  & 8.391  \\
307   & 8.261  & 8.913  & 9.478  & 9.043  & 9.696  & 8.652  & 8.391  & 7.304  & 7.217  & 8.174  \\
308   & 7.87   & 8.739  & 9.391  & 9.043  & 9.696  & 8.609  & 7.913  & 7.304  & 7.391  & 8.304  \\
309   & 7.652  & 8.609  & 9.348  & 8.957  & 9.522  & 8.739  & 7.87   & 7.435  & 7.435  & 8.304  \\
310   & 7.783  & 8.565  & 9.348  & 9.13   & 9.652  & 8.522  & 7.826  & 7.391  & 7.391  & 8.217  \\
311   & 7.696  & 8.652  & 9.043  & 9.304  & 9.609  & 8.609  & 7.783  & 7.217  & 7.391  & 8.304  \\
312   & 7.696  & 8.391  & 8.913  & 9.087  & 9.783  & 8.652  & 7.696  & 7.261  & 7.478  & 7.957  \\
313   & 7.652  & 8.435  & 8.739  & 9.087  & 9.609  & 8.696  & 7.609  & 7.435  & 7.348  & 8.13   \\
314   & 7.652  & 8.348  & 8.826  & 9      & 9.609  & 8.957  & 7.609  & 7.391  & 7.261  & 8.043  \\
315   & 7.652  & 8.435  & 8.87   & 8.957  & 9.217  & 8.957  & 7.522  & 7.348  & 7.13   & 8.13   \\
316   & 7.478  & 8.348  & 8.913  & 9.13   & 9.304  & 8.87   & 7.478  & 7.391  & 7.087  & 7.565  \\
317   & 7.522  & 8.304  & 8.826  & 8.957  & 9.348  & 8.913  & 7.478  & 7.304  & 7.043  & 7.652  \\
318   & 7.522  & 8.435  & 8.87   & 8.913  & 9.348  & 8.826  & 7.522  & 7.217  & 6.913  & 7.739  \\
319   & 7.391  & 8.391  & 8.565  & 8.783  & 9.304  & 8.913  & 7.609  & 7.13   & 6.783  & 7.826  \\
320   & 7.435  & 8.391  & 8.522  & 8.87   & 9.348  & 8.913  & 7.565  & 7.087  & 6.696  & 7.957  \\
321   & 7.348  & 8.522  & 8.304  & 8.87   & 9.522  & 8.913  & 7.391  & 6.696  & 6.783  & 8.043  \\
322   & 7.435  & 8.217  & 7.913  & 8.391  & 9.478  & 8.87   & 7.304  & 6.522  & 6.783  & 8.217  \\
323   & 7.348  & 8.217  & 8.043  & 8.261  & 9.565  & 8.739  & 6.609  & 6.522  & 6.652  & 7.913  \\
324   & 7.304  & 8.348  & 8.043  & 8.174  & 9.391  & 8.87   & 6.478  & 6.522  & 6.783  & 7.913  \\
325   & 7.348  & 8.174  & 8.13   & 7.391  & 9.435  & 8.913  & 6.435  & 6.435  & 6.783  & 8.043  \\
326   & 7.261  & 8.087  & 8.261  & 7.087  & 9.435  & 8.913  & 6.435  & 6.609  & 6.783  & 7.87   \\
327   & 7.217  & 7.957  & 8.565  & 7.174  & 9.565  & 9      & 6.609  & 6.696  & 6.826  & 7.826  \\
328   & 7.174  & 7.783  & 8.435  & 7.261  & 9.174  & 8.957  & 6.739  & 6.652  & 6.913  & 7.739  \\
329   & 7.13   & 7.913  & 8.478  & 7.217  & 9.174  & 9      & 6.478  & 6.696  & 6.565  & 7.739  \\
330   & 7.217  & 7.957  & 8.391  & 7.261  & 9      & 8.652  & 6.435  & 6.609  & 6.391  & 7.957  \\
331   & 7.348  & 7.87   & 8.348  & 7.391  & 8.957  & 8.565  & 6.391  & 6.522  & 6.261  & 7.913  \\
332   & 7.348  & 7.87   & 7.87   & 7.435  & 9.043  & 8.522  & 6.261  & 6.348  & 6.174  & 7.826  \\
333   & 7.348  & 7.652  & 7.826  & 7.435  & 8.783  & 8.478  & 6.348  & 6.348  & 6.304  & 7.826  \\
334   & 7      & 7.696  & 7.652  & 7.478  & 8.87   & 8.478  & 6.217  & 6.217  & 6.348  & 7.739  \\
335   & 6.87   & 7.783  & 7.609  & 7.565  & 8.609  & 8.522  & 6.13   & 6.304  & 6.348  & 7.565  \\
336   & 6.87   & 7.826  & 7.522  & 7.391  & 8.609  & 8.609  & 6.261  & 6.174  & 6.087  & 7.609  \\
337   & 6.783  & 7.522  & 7.348  & 6.783  & 8.522  & 8.261  & 6.13   & 6.304  & 6.087  & 7.609  \\
338   & 6.739  & 7.609  & 7.304  & 6.391  & 8.217  & 7.826  & 6.348  & 6.565  & 6.13   & 7.609  \\
339   & 6.739  & 7.522  & 6.783  & 6.435  & 8.391  & 7.739  & 6.391  & 6.348  & 6.174  & 7.739  \\
340   & 6.435  & 7.739  & 6.783  & 6.391  & 8.435  & 7.826  & 6.478  & 6.304  & 5.913  & 7.783  \\
341   & 6.522  & 7.739  & 6.522  & 6.609  & 8.435  & 7.783  & 6.565  & 6.348  & 5.87   & 7.739  \\
342   & 6.609  & 7.609  & 6.087  & 6.435  & 8.304  & 7.739  & 5.826  & 6.391  & 5.783  & 7.652  \\
343   & 6.522  & 7.565  & 6.13   & 6.565  & 8.391  & 7.696  & 5.783  & 6.391  & 5.739  & 7.696  \\
344   & 6.217  & 7.435  & 6.174  & 6.13   & 8.391  & 7.609  & 5.783  & 6.435  & 5.87   & 7.739  \\
345   & 6.348  & 7.261  & 6.043  & 6.174  & 8.391  & 7.609  & 5.783  & 6.304  & 5.87   & 7.957  \\
346   & 6.348  & 7      & 6.174  & 6.217  & 8.261  & 7.478  & 5.957  & 6.304  & 5.304  & 7.957  \\
347   & 6.043  & 6.87   & 6.043  & 6.087  & 8.261  & 7.087  & 5.957  & 6.304  & 5.435  & 7.826  \\
348   & 5.913  & 7      & 6.174  & 6.174  & 8      & 7.13   & 6      & 6.478  & 5.304  & 7.913  \\
349   & 5.957  & 6.783  & 6.304  & 6      & 8.217  & 7.348  & 6.13   & 6.348  & 5.217  & 8.261  \\
350   & 5.826  & 6.696  & 6.217  & 6.13   & 8.304  & 7.174  & 6.261  & 6.174  & 5.304  & 8.261  \\
351   & 5.87   & 6.696  & 5.957  & 5.783  & 8.348  & 6.957  & 6.13   & 6.217  & 5.435  & 8.348  \\
352   & 5.913  & 6.522  & 6      & 5.478  & 8.174  & 6.826  & 6.087  & 6.348  & 5.609  & 7.652  \\
353   & 5.87   & 6.478  & 6.087  & 5.522  & 8.174  & 6.783  & 6.304  & 6.522  & 5.609  & 7.522  \\
354   & 5.739  & 6.478  & 6.217  & 5.609  & 8      & 6.87   & 6.304  & 6.652  & 5.478  & 7.478  \\
355   & 5.87   & 6.609  & 5.609  & 5.522  & 7.913  & 6.739  & 6.174  & 6.783  & 4.957  & 7.435  \\
356   & 5.739  & 6.609  & 5.696  & 5.522  & 7.826  & 6.739  & 6.087  & 6.87   & 4.87   & 7.522  \\
357   & 5.652  & 6.478  & 5.696  & 5.478  & 7.826  & 6.739  & 5.957  & 6.783  & 4.609  & 7.565  \\
358   & 5.826  & 6.522  & 5.826  & 5.478  & 7.652  & 6.478  & 5.913  & 6.696  & 4.783  & 7.696  \\
359   & 6      & 6.609  & 5.826  & 5.478  & 7.522  & 6.304  & 5.783  & 6.957  & 4.913  & 7.826  \\
360   & 6      & 6.391  & 6.043  & 5.522  & 7.609  & 6.435  & 5.696  & 6.783  & 5.13   & 7.739  \\
361   & 6.13   & 6.174  & 6.217  & 5.522  & 7.478  & 6.217  & 5.739  & 6.87   & 5.174  & 7.739  \\
362   & 6.087  & 6.261  & 6.217  & 5.522  & 7.304  & 6.522  & 5.913  & 6.913  & 5.261  & 7.783  \\
363   & 5.87   & 6.087  & 6.043  & 5.652  & 7.13   & 6.652  & 6.13   & 6.913  & 5.087  & 7.696  \\
364   & 5.87   & 6.261  & 5.913  & 5.522  & 7.087  & 6.609  & 6.174  & 6.522  & 4.957  & 7.652  \\
365   & 5.913  & 6.043  & 5.174  & 5.348  & 7.043  & 6.652  & 6.217  & 6.522  & 5.13   & 7.609  \\
366   & 6.13   & 5.87   & 5.174  & 5.304  & 7.261  & 6.391  & 6.261  & 6.391  & 5.043  & 7.739  \\
367   & 6.087  & 6.043  & 5.174  & 5.261  & 7.174  & 6.478  & 6.217  & 6.391  & 5.087  & 7.783  \\
368   & 6.13   & 5.826  & 5.174  & 5.304  & 7.174  & 6.696  & 6.217  & 6.435  & 5.174  & 7.913  \\
369   & 6.043  & 5.783  & 5.13   & 5      & 7.435  & 6.783  & 6.087  & 6.391  & 5.087  & 7.739  \\
370   & 5.87   & 5.826  & 5.087  & 5      & 7.391  & 7.13   & 5.957  & 6.435  & 4.957  & 7.565  \\
371   & 5.696  & 5.696  & 5.13   & 5.087  & 7.304  & 6.826  & 6.087  & 6.13   & 5.304  & 7.478  \\
372   & 5.522  & 5.696  & 5.217  & 5      & 7      & 5.913  & 6.217  & 5.826  & 5.261  & 7.087  \\
373   & 5.826  & 5.522  & 5.13   & 5.043  & 6.957  & 5.696  & 6.478  & 5.957  & 5.174  & 7.13   \\
374   & 5.87   & 5.478  & 5      & 4.913  & 7      & 5.522  & 6.348  & 5.957  & 5.304  & 7.261  \\
375   & 5.826  & 5.435  & 5.13   & 4.957  & 6.826  & 5.261  & 6.304  & 6.087  & 5.348  & 7.304  \\
376   & 5.696  & 5.696  & 5.217  & 4.783  & 6.87   & 5.261  & 6.348  & 6.217  & 5.304  & 7.13   \\
377   & 5.652  & 5.652  & 5.478  & 4.826  & 6.826  & 5.261  & 5.783  & 6.261  & 5.478  & 7.174  \\
378   & 5.696  & 5.478  & 5.261  & 4.652  & 6.739  & 4.478  & 5.87   & 6.043  & 5.174  & 6.826  \\
379   & 5.435  & 5.435  & 5.13   & 4.957  & 6.696  & 4.957  & 5.913  & 5.696  & 5.043  & 6.826  \\
380   & 5.435  & 5.304  & 5.217  & 5.043  & 6.652  & 5.435  & 5.826  & 5.826  & 5.217  & 6.87   \\
381   & 5.348  & 5.348  & 5.261  & 5.087  & 6.478  & 4.522  & 6      & 6.043  & 5      & 6.826  \\
382   & 5.435  & 5.435  & 5.565  & 5.087  & 6.565  & 4.522  & 5.913  & 5.826  & 5.391  & 6.957  \\
383   & 5.304  & 5.391  & 5.652  & 5.13   & 6.522  & 4.652  & 5.87   & 5.783  & 5.696  & 7.087  \\
384   & 5.174  & 5.783  & 5.609  & 5.13   & 6.522  & 4.609  & 5.826  & 5.739  & 5.391  & 7.174  \\
385   & 5.522  & 5.478  & 5.522  & 5.217  & 6.565  & 4.522  & 5.783  & 5.696  & 5.043  & 7.13   \\
386   & 5.565  & 5.391  & 5.348  & 5.13   & 6.391  & 4.522  & 5.826  & 5.739  & 5.478  & 7.261  \\
387   & 5.522  & 5.565  & 5.174  & 5.174  & 6.435  & 4.478  & 5.826  & 5.304  & 5.609  & 7.174  \\
388   & 5.304  & 5.783  & 5.261  & 5.304  & 6.826  & 4.304  & 5.522  & 4.826  & 5.391  & 7.217  \\
389   & 5.522  & 5.957  & 5.087  & 5.13   & 6.609  & 4.478  & 5.478  & 4.739  & 5.217  & 7.174  \\
390   & 5.522  & 5.304  & 4.913  & 4.87   & 6.217  & 4.435  & 5.478  & 4.826  & 4.826  & 7.13   \\
391   & 5.609  & 5.348  & 4.957  & 4.826  & 6.217  & 4.565  & 5.565  & 4.522  & 4.87   & 7.217  \\
\bottomrule\end{longtable}
\normalsize
