# Supplementary material for: Rehearsal-Free Continual Learning over Small Non-I.I.D. Batches
Source: arXiv:1907.03799 source file (2020-04-21)
Supplement: Supplementary file 13 [file 79_AR1.tex]

\subsection{AR1*, NICv2 - 79}
\fontsize{8}{11}\selectfont
\begin{longtable}[c]{rgrgrgrgrgr}
\hline
Batch & Run 0  & Run 1  & Run 2  & Run 3  & Run 4  & Run 5  & Run 6  & Run 7  & Run 8  & Run 9  \\ \hline
\endfirsthead
\endhead
0     & 7.174  & 7.174  & 7.174  & 7.174  & 7.174  & 7.174  & 7.174  & 7.174  & 7.174  & 7.174  \\
1     & 14     & 14     & 14     & 14     & 14     & 14     & 14     & 14     & 14     & 14     \\
2     & 14.522 & 14.783 & 12.565 & 14.783 & 14.826 & 12.957 & 13.13  & 15.826 & 14.87  & 13.304 \\
3     & 14.913 & 14.217 & 14.522 & 15.478 & 14.826 & 13.783 & 15.478 & 15.913 & 17.087 & 14.783 \\
4     & 17.348 & 15.652 & 14     & 15.304 & 14.435 & 13.217 & 16.217 & 17     & 17.913 & 14.87  \\
5     & 18.261 & 15.783 & 14.739 & 16.304 & 15.609 & 15.261 & 15.739 & 17.696 & 19.13  & 15.913 \\
6     & 18.652 & 16.348 & 15.826 & 16.217 & 15.174 & 16.565 & 17.652 & 19.478 & 20.609 & 18.565 \\
7     & 20.696 & 16.348 & 17.217 & 18.043 & 17.217 & 18.652 & 17.957 & 20.348 & 20.435 & 19.957 \\
8     & 21.696 & 17.261 & 18.217 & 18.217 & 18.043 & 20.087 & 17.783 & 20.739 & 21.217 & 20.826 \\
9     & 22.043 & 18.043 & 19.826 & 18.739 & 18.087 & 21.522 & 18.696 & 21.087 & 21.652 & 21.957 \\
10    & 23.783 & 18.348 & 20.087 & 20.13  & 18.609 & 22.391 & 19.522 & 21.348 & 20.217 & 22.391 \\
11    & 23.478 & 19.391 & 19.522 & 19.913 & 18.652 & 22.043 & 20.696 & 21.478 & 21.174 & 24.87  \\
12    & 24.13  & 19.217 & 21.174 & 21     & 19.565 & 22     & 20.043 & 22.217 & 22.696 & 26.391 \\
13    & 23.783 & 18.957 & 21.87  & 21.739 & 21.217 & 22.913 & 20.696 & 22.739 & 22.739 & 26.087 \\
14    & 25.304 & 20.217 & 22.13  & 22.304 & 20.174 & 23.261 & 20.739 & 23.478 & 24.043 & 27.652 \\
15    & 25.565 & 20.696 & 22.913 & 22.739 & 21.304 & 23.261 & 22.13  & 25.522 & 24.043 & 27.652 \\
16    & 25.826 & 21.435 & 23.957 & 22.783 & 22.957 & 24.043 & 22.348 & 25.957 & 25     & 27.826 \\
17    & 28.522 & 21.609 & 25.217 & 23.826 & 23.174 & 25.217 & 24.739 & 25.652 & 24.087 & 28.87  \\
18    & 30.174 & 21.652 & 26     & 26.609 & 24.348 & 25.696 & 24.435 & 27.087 & 24.435 & 30.304 \\
19    & 31.348 & 22.435 & 27.217 & 27.174 & 25.435 & 25.957 & 25.913 & 28.087 & 25.174 & 31.174 \\
20    & 31.913 & 23.174 & 27.174 & 27.174 & 27     & 26.174 & 27     & 28.696 & 26.174 & 32.652 \\
21    & 32.913 & 22.957 & 27.609 & 27.478 & 27.652 & 26.739 & 28.783 & 29.435 & 26.522 & 33.435 \\
22    & 33.391 & 24     & 29.13  & 28.435 & 28.478 & 28.739 & 30.043 & 29.609 & 26.87  & 35.087 \\
23    & 33.435 & 25.087 & 29.957 & 28.478 & 29.043 & 28.696 & 30.739 & 29.957 & 28.043 & 35.652 \\
24    & 33.565 & 25.609 & 30.522 & 29.087 & 29.652 & 29.87  & 31.565 & 31.043 & 28.783 & 36.13  \\
25    & 35.043 & 27.13  & 31.652 & 29.565 & 31.13  & 30.174 & 32.609 & 33.174 & 29.609 & 37.217 \\
26    & 35.13  & 27.478 & 29.522 & 30.565 & 31.87  & 30.913 & 34.13  & 33.652 & 30.304 & 38     \\
27    & 35.217 & 28.87  & 30.739 & 31.348 & 32.478 & 31.13  & 34.304 & 34.043 & 30.304 & 38.609 \\
28    & 35.696 & 29     & 30.739 & 31.304 & 34.13  & 32.217 & 34.391 & 34.391 & 31.783 & 40.043 \\
29    & 36.478 & 28.826 & 31.043 & 31.783 & 34.304 & 33.522 & 34.913 & 34.696 & 32.174 & 42.043 \\
30    & 36.739 & 29.435 & 33.435 & 32.217 & 34.565 & 34.826 & 35.043 & 35.609 & 32.435 & 42.087 \\
31    & 38.261 & 30.435 & 34.478 & 32.217 & 35.652 & 35.565 & 35.739 & 35.87  & 33.609 & 42.391 \\
32    & 38.696 & 30.913 & 36.435 & 33.826 & 36.522 & 35.87  & 36.609 & 37.174 & 34.217 & 42.913 \\
33    & 39.217 & 31.957 & 36.87  & 34.957 & 36.609 & 37.174 & 37.391 & 38.087 & 35.174 & 42.826 \\
34    & 40.391 & 32.304 & 36.435 & 36.652 & 39.783 & 37.957 & 38.783 & 38.957 & 35.826 & 43.348 \\
35    & 41.783 & 33.13  & 35.174 & 37.043 & 40.174 & 38.13  & 40.174 & 39.435 & 36.174 & 45.174 \\
36    & 42.13  & 33.609 & 36.043 & 38.783 & 41.739 & 39.435 & 41.261 & 39.478 & 36.174 & 46.087 \\
37    & 43.13  & 34.783 & 37.783 & 39.957 & 42.826 & 39.826 & 39     & 39.826 & 36.957 & 46.13  \\
38    & 43.957 & 34.87  & 38.913 & 40.696 & 43.522 & 40.261 & 39.826 & 41.174 & 39.043 & 46.435 \\
39    & 45.522 & 37.13  & 40.087 & 42.609 & 43.478 & 40.348 & 42.435 & 42.087 & 39.957 & 47.348 \\
40    & 46.391 & 37.217 & 40.739 & 44.043 & 44.957 & 41.565 & 42.957 & 42.261 & 40.391 & 47.609 \\
41    & 46.348 & 38.304 & 42.348 & 44.13  & 45.217 & 42.739 & 44.348 & 43.696 & 40.783 & 48.087 \\
42    & 46.348 & 39.087 & 43.348 & 43.913 & 46.565 & 42.696 & 44.609 & 44.696 & 41.174 & 48.348 \\
43    & 48.043 & 41.043 & 43.652 & 45.391 & 47.478 & 43.826 & 44.913 & 45.522 & 41.783 & 48.913 \\
44    & 48.348 & 41.174 & 44.609 & 45.826 & 48     & 45.783 & 45.304 & 47.652 & 42.348 & 49.348 \\
45    & 49.391 & 41.304 & 45.174 & 46.435 & 48.391 & 46     & 46.391 & 48.739 & 42.652 & 50.522 \\
46    & 50.783 & 41.478 & 45.435 & 46.478 & 48.435 & 44.739 & 48     & 48.652 & 42.957 & 52.652 \\
47    & 50.652 & 43.391 & 47.478 & 46.522 & 48.913 & 45.87  & 48.304 & 48.783 & 42.913 & 53.696 \\
48    & 50.522 & 44.565 & 47.957 & 46.957 & 48.957 & 46     & 49.043 & 48.174 & 43.783 & 54.391 \\
49    & 51.304 & 45.565 & 48.043 & 47.261 & 49.043 & 45.87  & 49.435 & 48.348 & 44.435 & 55.087 \\
50    & 51.826 & 46     & 47.174 & 49.391 & 50.304 & 47.652 & 49.826 & 48.696 & 44.826 & 55.696 \\
51    & 48.783 & 46.174 & 46.739 & 50.652 & 50.696 & 48     & 50.478 & 49.87  & 44.913 & 55.913 \\
52    & 48.783 & 48     & 47.565 & 51.522 & 51.391 & 47.826 & 50.739 & 50.261 & 45.348 & 56.087 \\
53    & 50.826 & 49.217 & 48.652 & 52.652 & 51.87  & 49.304 & 50.783 & 50.826 & 46.043 & 55.652 \\
54    & 51.174 & 50.261 & 49.087 & 53.739 & 53.391 & 50.087 & 51.087 & 51.87  & 46.261 & 56.13  \\
55    & 51.261 & 51.087 & 49.826 & 53.522 & 54.348 & 51.435 & 51.522 & 52.739 & 48.391 & 57.348 \\
56    & 52.043 & 51.13  & 52.087 & 54.304 & 55.739 & 52.217 & 51.522 & 53.478 & 48.826 & 57.348 \\
57    & 53.261 & 51.87  & 53.087 & 55.652 & 54.435 & 50.957 & 51.826 & 54.435 & 49.609 & 57.087 \\
58    & 54.957 & 52.391 & 53.957 & 56     & 55.652 & 53     & 53.13  & 54.391 & 51.565 & 58.739 \\
59    & 56.652 & 53     & 55.13  & 56.522 & 55.391 & 53.217 & 53.913 & 55.783 & 52.565 & 59.261 \\
60    & 57.087 & 53.13  & 55.652 & 57.261 & 55.304 & 54.478 & 54.826 & 56.478 & 53.957 & 59.043 \\
61    & 57.348 & 54.043 & 56.783 & 56.565 & 55.478 & 55.261 & 56.261 & 56.783 & 54.696 & 60.609 \\
62    & 57.391 & 54.652 & 57.217 & 57.174 & 56.217 & 56.609 & 56.87  & 58.609 & 54.957 & 61.522 \\
63    & 57.739 & 55.783 & 56.478 & 58.261 & 55.652 & 57.783 & 57.304 & 59.13  & 56.261 & 63.565 \\
64    & 59.13  & 57.174 & 57.87  & 58.739 & 56.565 & 58.391 & 57.957 & 60.087 & 55.957 & 64.043 \\
65    & 60.435 & 57.739 & 60.304 & 60.13  & 59.217 & 58.783 & 58.261 & 60.913 & 57     & 64.739 \\
66    & 61.13  & 58.609 & 60.609 & 59.652 & 60.043 & 59.217 & 58.348 & 61.304 & 57.478 & 64.565 \\
67    & 61.696 & 59.217 & 61.957 & 60.391 & 60.348 & 59     & 58.652 & 62.217 & 58     & 64.652 \\
68    & 62.783 & 60.087 & 63.609 & 60.913 & 61.043 & 59.87  & 60.043 & 61.957 & 59.348 & 64.522 \\
69    & 63.957 & 59.826 & 63.435 & 61.826 & 61.87  & 59.913 & 60.826 & 62     & 61.043 & 64.391 \\
70    & 63.957 & 59.913 & 63.348 & 62.043 & 61.565 & 59.957 & 61.348 & 62.348 & 61.174 & 64.739 \\
71    & 64.087 & 60.304 & 63.217 & 62.783 & 62.087 & 61.043 & 62.304 & 62.652 & 62.391 & 64.13  \\
72    & 63.957 & 60.565 & 62.652 & 62.913 & 61.739 & 61.217 & 62.696 & 63.348 & 62.174 & 64.609 \\
73    & 64.609 & 60.87  & 62.522 & 62.957 & 62.261 & 62.174 & 63     & 63.609 & 62.391 & 64.739 \\
74    & 64.87  & 61.478 & 62.174 & 62.913 & 62.13  & 62.217 & 62.957 & 63.826 & 63.13  & 64.565 \\
75    & 65     & 61.304 & 62.435 & 62.957 & 62.261 & 61.87  & 63.478 & 63.87  & 63.435 & 64.783 \\
76    & 64.957 & 61.348 & 61.739 & 63.652 & 62.739 & 61.87  & 63.652 & 63.783 & 63.652 & 65     \\
77    & 65.174 & 61.913 & 61.696 & 64     & 62.696 & 62.304 & 63.435 & 64.043 & 63.957 & 65.174 \\
78    & 65.652 & 61.913 & 61.696 & 64.609 & 62.957 & 62.174 & 63.87  & 64.217 & 63.565 & 64.652 \\
79    & 65.522 & 61.826 & 61.783 & 64.522 & 63     & 62.522 & 64.087 & 64.043 & 63.739 & 64     \\
\bottomrule\end{longtable}
\normalsize
