# Supplementary material for: Rehearsal-Free Continual Learning over Small Non-I.I.D. Batches
Source: arXiv:1907.03799 source file (2020-04-21)
Supplement: Supplementary file 14 [file 79_AR1_BN.tex]

\subsection{AR1* (with Batch Normalization), NICv2 - 79}
\fontsize{8}{11}\selectfont
\begin{longtable}[c]{rgrgrgrgrgr}
\hline
Batch & Run 0  & Run 1  & Run 2  & Run 3  & Run 4  & Run 5  & Run 6  & Run 7  & Run 8  & Run 9  \\ \hline
\endfirsthead
\endhead
0     & 8.127  & 8.127  & 8.127  & 8.127  & 8.127  & 8.127  & 8.127  & 8.127  & 8.127  & 8.127  \\
1     & 14.031 & 14.033 & 14.031 & 14.031 & 14.033 & 14.031 & 14.031 & 14.031 & 14.031 & 14.031 \\
2     & 14.611 & 15.267 & 13.987 & 15.184 & 15.327 & 14.044 & 14.338 & 14.98  & 15.196 & 14.713 \\
3     & 15.473 & 14.907 & 15.86  & 16.342 & 15.569 & 15.344 & 16.042 & 15.933 & 16.76  & 15.973 \\
4     & 17.076 & 15.469 & 16.176 & 16.431 & 15.722 & 15.149 & 17.12  & 17.242 & 18.076 & 16.544 \\
5     & 18.033 & 16.982 & 17.187 & 16.887 & 16.371 & 16.649 & 16.944 & 17.333 & 18.924 & 16.544 \\
6     & 18.607 & 17.664 & 18.324 & 16.616 & 16.076 & 18.724 & 18.191 & 18.833 & 21.311 & 18.404 \\
7     & 19.336 & 17.036 & 18.613 & 17.884 & 16.707 & 20.324 & 18.613 & 20.08  & 21.289 & 19.851 \\
8     & 21.002 & 17.156 & 18.771 & 18.027 & 16.676 & 21.227 & 17.749 & 20.104 & 21.853 & 20.156 \\
9     & 21.14  & 17.962 & 20.538 & 19.158 & 18.242 & 21.667 & 17.931 & 20.251 & 22.429 & 20.176 \\
10    & 22.416 & 17.924 & 20.478 & 19.276 & 18.551 & 23.458 & 18.631 & 20.509 & 21.289 & 20.151 \\
11    & 22.756 & 18.844 & 20.171 & 19.687 & 18.478 & 22.751 & 19.318 & 20.776 & 21.898 & 22.478 \\
12    & 23.158 & 18.633 & 21.349 & 20.544 & 19.331 & 22.48  & 19.569 & 21.064 & 22.256 & 23.222 \\
13    & 21.38  & 18.498 & 21.524 & 21.658 & 21.062 & 22.533 & 19.716 & 21.891 & 22.178 & 24.369 \\
14    & 23.536 & 19.144 & 22.391 & 21.736 & 20.436 & 23.496 & 20.038 & 23.18  & 23.58  & 25.891 \\
15    & 23.996 & 19.309 & 23.742 & 21.978 & 21.042 & 23.389 & 20.616 & 25.378 & 23.587 & 27.071 \\
16    & 24.211 & 19.56  & 24.82  & 23.078 & 22.182 & 23.773 & 20.658 & 25.636 & 24.129 & 27.891 \\
17    & 26.951 & 19.773 & 25.1   & 23.887 & 22.622 & 25.047 & 21.989 & 25.338 & 23.733 & 28.091 \\
18    & 29.029 & 19.916 & 26.191 & 24.662 & 23.458 & 25.28  & 22.04  & 25.422 & 24.009 & 28.418 \\
19    & 28.624 & 21.607 & 26.729 & 24.604 & 25.467 & 25.562 & 23.196 & 25.596 & 24.429 & 29.762 \\
20    & 30.882 & 21.613 & 26.227 & 25.118 & 27.927 & 25.751 & 24.196 & 27.356 & 25.882 & 30.931 \\
21    & 31.242 & 21.464 & 26.644 & 25.031 & 28.562 & 25.831 & 25.98  & 28.269 & 26.253 & 31.676 \\
22    & 31.682 & 23.162 & 27.704 & 25.122 & 28.609 & 27.522 & 27.204 & 28.682 & 26.34  & 33.467 \\
23    & 31.882 & 23.996 & 28.736 & 25.307 & 29.318 & 28.362 & 27.86  & 29.351 & 26.647 & 33.609 \\
24    & 31.8   & 24.247 & 28.442 & 25.86  & 30.009 & 28.96  & 28.853 & 29.911 & 27.282 & 34.802 \\
25    & 32.816 & 25.396 & 29.184 & 26.398 & 31.46  & 29.116 & 29.898 & 31.393 & 27.502 & 34.729 \\
26    & 33.036 & 25.489 & 29.282 & 26.06  & 31.473 & 30.102 & 30.293 & 31.769 & 28.589 & 35.251 \\
27    & 33.722 & 26.522 & 30.147 & 26.702 & 31.616 & 30.547 & 31.269 & 32.269 & 29.06  & 35.987 \\
28    & 33.938 & 27.249 & 29.616 & 27.267 & 33.664 & 32.022 & 30.982 & 32.976 & 30.476 & 37.549 \\
29    & 32.962 & 27.627 & 29.791 & 27.691 & 34.236 & 32.729 & 31.598 & 33.069 & 31.076 & 38.34  \\
30    & 33.358 & 27.476 & 31.08  & 28.26  & 34.658 & 33.524 & 32.522 & 34.073 & 31.384 & 38.72  \\
31    & 33.664 & 27.767 & 31.858 & 28.453 & 35.673 & 33.727 & 32.831 & 34.238 & 32.413 & 39.698 \\
32    & 34.898 & 28.504 & 33.598 & 30.116 & 36.413 & 34.184 & 33.113 & 34.971 & 33.247 & 41.478 \\
33    & 36.647 & 28.304 & 34.616 & 31.098 & 37.264 & 34.767 & 34     & 35.578 & 34.391 & 41.007 \\
34    & 36.933 & 28.487 & 33.676 & 31.093 & 39.249 & 35.149 & 35.222 & 36.347 & 35.771 & 40.882 \\
35    & 37.829 & 28.471 & 34.349 & 31.816 & 39.287 & 35.236 & 37.184 & 36.824 & 36.136 & 42.544 \\
36    & 37.918 & 29.133 & 34.671 & 32.411 & 40.171 & 36.596 & 37.789 & 37.633 & 36.298 & 43.604 \\
37    & 39.322 & 30.42  & 35.98  & 33.733 & 40.287 & 36.849 & 38.018 & 38.382 & 37.08  & 43.484 \\
38    & 39.489 & 30.68  & 37.44  & 34.004 & 39.749 & 36.562 & 39.013 & 38.313 & 37.738 & 44.26  \\
39    & 41.304 & 33.133 & 38.76  & 36.211 & 38.46  & 36.62  & 39.253 & 38.771 & 39.371 & 45.582 \\
40    & 42.262 & 33.296 & 38.92  & 37     & 39.287 & 36.998 & 39.542 & 38.924 & 39.873 & 45.789 \\
41    & 42.322 & 33.18  & 38.942 & 37.513 & 39.924 & 37.253 & 39.529 & 39.189 & 40.984 & 45.711 \\
42    & 43.091 & 33.949 & 39.838 & 37.673 & 40.98  & 37.547 & 40.178 & 39.824 & 41.42  & 45.216 \\
43    & 43.758 & 35.791 & 40.04  & 38.009 & 42.922 & 38.591 & 40.18  & 40.236 & 41.94  & 45.88  \\
44    & 43.869 & 37.06  & 40.193 & 37.904 & 43.656 & 40.067 & 40.882 & 40.722 & 42.527 & 45.769 \\
45    & 44.098 & 37.702 & 40.287 & 38.047 & 43.182 & 40.562 & 42.144 & 43.091 & 42.589 & 46.158 \\
46    & 45.473 & 37.278 & 40.004 & 38.544 & 43.751 & 41.524 & 41.942 & 43.469 & 43.351 & 48.024 \\
47    & 45.864 & 38.227 & 40.816 & 40.18  & 45.182 & 41.658 & 43.038 & 44.447 & 43.656 & 48.362 \\
48    & 45.984 & 39.398 & 42.056 & 41.438 & 45.467 & 41.427 & 43.111 & 44.936 & 44.896 & 49.058 \\
49    & 45.5   & 40.087 & 43.871 & 41.884 & 44.891 & 42.447 & 44.329 & 45.744 & 44.627 & 49.598 \\
50    & 45.869 & 41.564 & 43.482 & 43.436 & 45.382 & 43.253 & 44.951 & 46.193 & 44.464 & 51.118 \\
51    & 45.436 & 40.687 & 43.138 & 45.402 & 46.389 & 45.856 & 46.087 & 45.718 & 44.26  & 51.071 \\
52    & 46.224 & 40.931 & 44.113 & 45.849 & 47.416 & 45.438 & 46.818 & 47.127 & 44.178 & 50.587 \\
53    & 47.016 & 42.416 & 44.56  & 46.016 & 48.978 & 45.927 & 46.778 & 47.409 & 44.369 & 50.84  \\
54    & 48.773 & 42.971 & 45.56  & 46.949 & 50.271 & 47.531 & 47.093 & 48.482 & 43.582 & 52.709 \\
55    & 48.891 & 44.716 & 46.351 & 47.32  & 50.66  & 47.54  & 47.367 & 48.827 & 45.527 & 52.382 \\
56    & 49.489 & 45.029 & 48.189 & 48.658 & 52.284 & 48.531 & 47.384 & 49.129 & 46.453 & 53.184 \\
57    & 48.711 & 45.791 & 48.231 & 48.733 & 51.942 & 47.284 & 48.471 & 49.773 & 47.829 & 53.833 \\
58    & 50.036 & 47.118 & 48.047 & 49.569 & 51.136 & 48.46  & 50.171 & 50.193 & 48.891 & 54.427 \\
59    & 50.52  & 46.993 & 49.233 & 51.213 & 50.913 & 49.156 & 50.458 & 51.902 & 49.324 & 54.987 \\
60    & 51.131 & 48.064 & 50.736 & 52.316 & 51.136 & 48.356 & 50.689 & 51.242 & 50.824 & 55.347 \\
61    & 52.544 & 49.376 & 51.742 & 51.922 & 51.989 & 51.144 & 51.702 & 51.338 & 50.607 & 56.636 \\
62    & 52.407 & 49.884 & 52.004 & 53.004 & 53.118 & 51.449 & 51.789 & 54.458 & 51.993 & 57.762 \\
63    & 52.102 & 50.451 & 51.24  & 54.06  & 53.204 & 51.887 & 50.887 & 55.229 & 51.602 & 61.029 \\
64    & 53.12  & 50.416 & 51.92  & 53.622 & 53.18  & 53.013 & 51.951 & 56.011 & 51.607 & 61.736 \\
65    & 55.109 & 50.82  & 53.753 & 53.847 & 54.304 & 53.449 & 52.476 & 56.327 & 54.071 & 62.496 \\
66    & 54.956 & 52.596 & 54.104 & 54.064 & 55.104 & 55.416 & 52.464 & 56.111 & 54.398 & 62.782 \\
67    & 57.089 & 52.918 & 56.331 & 54.291 & 54.429 & 53.467 & 53.198 & 56.518 & 54.893 & 62.804 \\
68    & 56.916 & 53.278 & 56.336 & 54.864 & 56.764 & 51.913 & 53.727 & 57.498 & 53.884 & 62.938 \\
69    & 57.427 & 54.111 & 56.782 & 54.913 & 58.04  & 53.964 & 53.718 & 57.669 & 53.982 & 63.331 \\
70    & 57.707 & 54.749 & 57.671 & 55.384 & 56.178 & 54.516 & 53.896 & 58.233 & 53.629 & 64.027 \\
71    & 58.976 & 53.871 & 57.342 & 54.564 & 55.733 & 55.649 & 54.887 & 57.16  & 55.671 & 63.304 \\
72    & 59.958 & 53.269 & 56.198 & 54.307 & 55.502 & 57.618 & 53.487 & 57.311 & 56.076 & 63.291 \\
73    & 60.5   & 52.5   & 54.516 & 55.098 & 56.122 & 58.429 & 52.144 & 57.493 & 56.927 & 64.251 \\
74    & 60.891 & 54.289 & 53.402 & 54.442 & 56.789 & 59.184 & 50.322 & 58.056 & 57.4   & 61.931 \\
75    & 58.864 & 54.064 & 53.94  & 54.987 & 58.833 & 59.442 & 51.511 & 57.416 & 55.629 & 62.442 \\
76    & 60.949 & 52.456 & 54.082 & 54.316 & 55.616 & 59.978 & 52.664 & 58.369 & 56.129 & 63.902 \\
77    & 60.687 & 51.549 & 54.078 & 52.567 & 49.544 & 59.962 & 50.462 & 57.753 & 53.182 & 63.613 \\
78    & 60.436 & 53.14  & 50.367 & 52.189 & 59.218 & 60.236 & 54.018 & 56.14  & 49.384 & 62.944 \\
79    & 59.909 & 54.484 & 54.904 & 52.9   & 59.633 & 60.051 & 53.18  & 54.411 & 54.744 & 60.218 \\
\bottomrule\end{longtable}
\normalsize
