# Supplementary material for: Rehearsal-Free Continual Learning over Small Non-I.I.D. Batches
Source: arXiv:1907.03799 source file (2020-04-21)
Supplement: Supplementary file 15 [file 79_CWR.tex]

\subsection{CWR*, NICv2 - 79}
\fontsize{8}{11}\selectfont
\begin{longtable}[c]{rgrgrgrgrgr}
\hline
Batch & Run 0  & Run 1  & Run 2  & Run 3  & Run 4  & Run 5  & Run 6  & Run 7  & Run 8  & Run 9  \\ \hline
\endfirsthead
\endhead
0     & 7.174  & 7.174  & 7.174  & 7.174  & 7.174  & 7.174  & 7.174  & 7.174  & 7.174  & 7.174  \\
1     & 14     & 14     & 14     & 14     & 14     & 14     & 14     & 14     & 14     & 14     \\
2     & 14.391 & 14.696 & 12.522 & 14.739 & 14.696 & 12.957 & 13.087 & 15.87  & 14.783 & 13.348 \\
3     & 14.696 & 13.783 & 14.435 & 15.348 & 14.739 & 13.652 & 15.348 & 16     & 17.261 & 14.522 \\
4     & 17.304 & 15.565 & 13.957 & 15.087 & 14.391 & 13     & 15.87  & 16.739 & 17.957 & 14.739 \\
5     & 18     & 15.348 & 14.565 & 16     & 15.13  & 14.957 & 15.565 & 17.348 & 18.609 & 15.522 \\
6     & 18.217 & 15.913 & 15.478 & 15.826 & 14.826 & 16.174 & 17.478 & 19.174 & 20.087 & 18.174 \\
7     & 20.217 & 15.913 & 17.087 & 17.565 & 16.87  & 18.174 & 17.609 & 19.87  & 19.826 & 19.609 \\
8     & 21.13  & 16.696 & 17.522 & 17.87  & 17.565 & 19.217 & 17.478 & 20     & 20.739 & 20.522 \\
9     & 21.609 & 17.696 & 19.087 & 18.435 & 17.826 & 20.435 & 18.391 & 20.609 & 21.217 & 21.522 \\
10    & 23.217 & 17.652 & 19.174 & 19.783 & 18.174 & 21.391 & 19.391 & 20.826 & 19.565 & 22     \\
11    & 23.304 & 18.652 & 18.87  & 19.435 & 18.261 & 21.348 & 20.478 & 20.739 & 20.522 & 23.783 \\
12    & 23.826 & 18.826 & 20.261 & 20.217 & 19.043 & 21.217 & 19.826 & 21.391 & 22.304 & 25.522 \\
13    & 22.957 & 18.435 & 20.565 & 21.087 & 20.174 & 22     & 20.261 & 21.696 & 22.565 & 25.391 \\
14    & 24.652 & 19.609 & 20.826 & 21.478 & 19.087 & 22.304 & 20.217 & 22.826 & 23.435 & 26.435 \\
15    & 25.13  & 20.087 & 21.739 & 22.217 & 20.261 & 22.261 & 21.304 & 24.696 & 22.87  & 26.783 \\
16    & 25.217 & 20.913 & 23.043 & 22     & 21.348 & 23.043 & 21.652 & 25.174 & 24.304 & 27.087 \\
17    & 28.261 & 21.13  & 23.652 & 23     & 21.826 & 24.261 & 24.174 & 25.043 & 23.13  & 27.87  \\
18    & 29.87  & 21.652 & 24.652 & 25.478 & 23.043 & 24.391 & 24.043 & 26.478 & 23.913 & 29.13  \\
19    & 30.565 & 22.13  & 25.391 & 26.174 & 24.13  & 24.652 & 25.348 & 27.174 & 24.565 & 30.174 \\
20    & 30.957 & 22.696 & 25.522 & 26.043 & 25.696 & 24.783 & 26.304 & 27.565 & 25.696 & 31.435 \\
21    & 31.783 & 22.348 & 25.913 & 26.522 & 26.261 & 25.217 & 28     & 28.435 & 25.391 & 32.478 \\
22    & 32     & 23.565 & 27.522 & 27.217 & 26.87  & 26.87  & 29.217 & 28.565 & 25.87  & 33.609 \\
23    & 32.348 & 24.217 & 28.261 & 26.783 & 27.609 & 26.87  & 29.783 & 29.087 & 27.609 & 34.435 \\
24    & 32.522 & 24.826 & 28.696 & 26.913 & 27.696 & 28.043 & 30.435 & 30.217 & 28.217 & 34.565 \\
25    & 33.87  & 26.13  & 29.783 & 27.391 & 28.913 & 28.739 & 30.913 & 31.957 & 28.783 & 35.435 \\
26    & 34.13  & 26.391 & 26.87  & 28.261 & 29.652 & 29.217 & 31.957 & 32.174 & 29.696 & 36.435 \\
27    & 34.217 & 27.739 & 28.435 & 29.174 & 30.304 & 29.522 & 32.087 & 32.348 & 29.522 & 36.87  \\
28    & 34.652 & 28.043 & 28     & 29.087 & 31.565 & 30.87  & 32.261 & 33     & 30.609 & 38.391 \\
29    & 35.522 & 27.087 & 28.087 & 29.783 & 32.261 & 32.261 & 32.696 & 33.348 & 31.13  & 39.913 \\
30    & 35.87  & 27.391 & 31.391 & 30.13  & 32.348 & 33.478 & 33     & 34.391 & 31.13  & 40.043 \\
31    & 37.348 & 29.043 & 32.174 & 30.565 & 33.522 & 34.304 & 33.261 & 35.174 & 31.696 & 40.435 \\
32    & 37.478 & 29.348 & 33.478 & 31.478 & 33.609 & 34.565 & 34     & 36.217 & 32.13  & 41.304 \\
33    & 37.783 & 30.391 & 33.696 & 31.913 & 34.304 & 35.609 & 34.609 & 37.043 & 32.652 & 41     \\
34    & 38.783 & 30.783 & 33.783 & 33.261 & 37.174 & 36.478 & 36     & 37.565 & 32.913 & 41.913 \\
35    & 40.043 & 31.348 & 31.217 & 33.739 & 37.913 & 36.783 & 37.304 & 37.739 & 33.304 & 43.043 \\
36    & 40.565 & 31.826 & 32.217 & 35.391 & 39.13  & 37.478 & 37.87  & 37.739 & 33.652 & 43.652 \\
37    & 40.957 & 32.522 & 33.217 & 36     & 39.696 & 37.696 & 36.348 & 38.261 & 34.087 & 43.783 \\
38    & 42.174 & 33.13  & 33.391 & 37.13  & 40.087 & 38     & 36.652 & 39.174 & 35.826 & 44.13  \\
39    & 43.565 & 35.174 & 34.435 & 38.652 & 39.957 & 38.13  & 38.652 & 39.217 & 36.957 & 44.522 \\
40    & 43.739 & 35.261 & 35.13  & 39.609 & 41.043 & 38.739 & 39.304 & 40.174 & 37.696 & 44.783 \\
41    & 43.435 & 36.652 & 36.304 & 40.174 & 41.13  & 39.13  & 39.13  & 40.783 & 37.652 & 44.609 \\
42    & 43.913 & 37.087 & 37.217 & 40.522 & 41.739 & 39.391 & 39.348 & 41.304 & 37.783 & 45.913 \\
43    & 45.13  & 38.522 & 38.391 & 41.609 & 42.783 & 39.957 & 40.304 & 41.391 & 38     & 45.826 \\
44    & 45.696 & 38.739 & 40.261 & 42.478 & 43.174 & 41.826 & 40.609 & 43.043 & 38.391 & 45.87  \\
45    & 46.391 & 39.087 & 41.13  & 42.826 & 42.913 & 41.826 & 41.87  & 43.783 & 38.609 & 46.217 \\
46    & 46.783 & 39.304 & 41.13  & 43.043 & 43.217 & 40.304 & 43.304 & 44.913 & 38.348 & 48.652 \\
47    & 47.217 & 41.043 & 44.261 & 43.261 & 43.913 & 42.13  & 44.652 & 44.435 & 37.87  & 49.391 \\
48    & 47.609 & 42.391 & 44.435 & 43.522 & 43.87  & 42.522 & 45.696 & 43.13  & 39.522 & 49.783 \\
49    & 47.435 & 43.652 & 44.522 & 43.652 & 44.13  & 42.826 & 45.609 & 43.522 & 40.261 & 50.957 \\
50    & 47.565 & 43.478 & 43.565 & 45.435 & 44.783 & 43.696 & 45.565 & 43.87  & 40     & 51.261 \\
51    & 43.261 & 43.348 & 43.478 & 47.13  & 44.826 & 44.261 & 46.478 & 45.13  & 40.348 & 51.348 \\
52    & 43.565 & 44.783 & 44.304 & 48.043 & 45.304 & 44.609 & 46.696 & 45.348 & 41.435 & 51.913 \\
53    & 46.522 & 45.957 & 45.348 & 48.478 & 46.174 & 45.217 & 47.087 & 46.217 & 41.739 & 50.913 \\
54    & 47.304 & 46.478 & 45.652 & 49.609 & 46.696 & 45.304 & 47.261 & 47.13  & 42.087 & 51.304 \\
55    & 47.348 & 47.174 & 46.391 & 49.261 & 47.348 & 45.739 & 47.522 & 47.348 & 43.348 & 52.391 \\
56    & 47.783 & 47.348 & 47.565 & 49.348 & 48.13  & 46.478 & 47.783 & 48.391 & 44     & 52.174 \\
57    & 49.696 & 47.913 & 48.522 & 50.348 & 47.087 & 46.304 & 47.826 & 49.261 & 44.565 & 52.348 \\
58    & 50.565 & 47.913 & 48.652 & 50.696 & 47.87  & 47.13  & 48.261 & 49.783 & 46.13  & 53.522 \\
59    & 52.043 & 48.043 & 50.174 & 51.13  & 48.522 & 47.696 & 48.913 & 51.087 & 47     & 53.435 \\
60    & 52.609 & 48.478 & 50.348 & 52.826 & 48.522 & 48.391 & 49.913 & 51.348 & 48.348 & 53.478 \\
61    & 53.174 & 48.913 & 51.217 & 52.348 & 48.87  & 49.478 & 50.87  & 52     & 49.261 & 54.652 \\
62    & 53.304 & 49.826 & 51.783 & 52.783 & 48.87  & 50.478 & 51.565 & 53.174 & 49.391 & 55.391 \\
63    & 53.609 & 49.913 & 50.217 & 53.348 & 49.304 & 50.522 & 51.826 & 53.696 & 49.913 & 57.261 \\
64    & 54.13  & 50.522 & 52     & 54.087 & 50.13  & 51.217 & 52.217 & 54.087 & 49.609 & 57.565 \\
65    & 55.304 & 50.652 & 54.261 & 55.043 & 52.348 & 51.043 & 52.043 & 54.087 & 50.087 & 58.609 \\
66    & 55.87  & 51.435 & 54.87  & 55.087 & 52.696 & 51.435 & 52.783 & 54.957 & 50.565 & 58.13  \\
67    & 56.478 & 51.435 & 55.565 & 55.609 & 52.783 & 51.87  & 53     & 56.435 & 51.043 & 58.261 \\
68    & 57.174 & 52.087 & 56.304 & 55.87  & 52.783 & 53.261 & 54.348 & 56.87  & 52.609 & 58.087 \\
69    & 58.043 & 51.783 & 56.435 & 55.87  & 53.739 & 53.217 & 55.13  & 57.261 & 53.435 & 57.565 \\
70    & 58.174 & 52.783 & 56.87  & 55.957 & 53.435 & 52.522 & 55.652 & 57.304 & 54.391 & 57.652 \\
71    & 58.739 & 53.13  & 56.522 & 56.87  & 53.652 & 53.739 & 55.696 & 56.87  & 55.87  & 56.826 \\
72    & 58.652 & 52.609 & 56.217 & 57     & 53.739 & 54.391 & 56.826 & 58.304 & 55.609 & 57.261 \\
73    & 59.348 & 52.783 & 56.348 & 57.522 & 53.739 & 55.522 & 56.826 & 59.087 & 56     & 57.435 \\
74    & 59.826 & 53.391 & 55.696 & 57.435 & 54.217 & 55.174 & 56.565 & 59.304 & 55.87  & 57.739 \\
75    & 59.348 & 52.826 & 55.826 & 57.391 & 54.522 & 54.957 & 57.217 & 59.391 & 55.826 & 58.087 \\
76    & 59.348 & 52.696 & 55.217 & 58.261 & 54.87  & 55.043 & 57.391 & 59.783 & 56.304 & 58.478 \\
77    & 59.783 & 53.652 & 55.739 & 58.913 & 54.696 & 55.696 & 56.739 & 59.609 & 56.174 & 58.348 \\
78    & 59.478 & 53.565 & 55.435 & 59.435 & 54.783 & 56.087 & 57.087 & 59.913 & 56.348 & 58.13  \\
79    & 59.348 & 54.13  & 56.087 & 59.043 & 54.522 & 56.13  & 56.826 & 60     & 57.13  & 57.522 \\
\bottomrule\end{longtable}
\normalsize
