# Supplementary material for: Rehearsal-Free Continual Learning over Small Non-I.I.D. Batches
Source: arXiv:1907.03799 source file (2020-04-21)
Supplement: Supplementary file 16 [file 79_EWC.tex]

\subsection{EWC, NICv2 - 79}
\fontsize{8}{11}\selectfont
\begin{longtable}[c]{rgrgrgrgrgr}
\hline
Batch & Run 0  & Run 1  & Run 2  & Run 3  & Run 4  & Run 5  & Run 6  & Run 7  & Run 8  & Run 9  \\ \hline
\endfirsthead
\endhead
0     & 1.522  & 1.522  & 1.522  & 1.522  & 1.522  & 1.522  & 1.522  & 1.522  & 1.522  & 1.522  \\
1     & 13.783 & 13.87  & 13.87  & 13.826 & 13.826 & 13.826 & 13.87  & 13.87  & 13.826 & 13.87  \\
2     & 13.957 & 14.87  & 12.522 & 14.348 & 14.87  & 13.609 & 13.391 & 14.348 & 14.478 & 13.435 \\
3     & 14.609 & 15.043 & 13.957 & 15.174 & 14.217 & 13.957 & 14.043 & 14.696 & 15.043 & 14     \\
4     & 15.652 & 15.174 & 14.522 & 15.13  & 14.217 & 14.043 & 15.435 & 16.087 & 15.652 & 14.696 \\
5     & 15.913 & 16.565 & 14.739 & 15.87  & 15.478 & 15     & 15.435 & 16.043 & 16.391 & 15.261 \\
6     & 16.783 & 17     & 14.739 & 15.696 & 15.652 & 15.522 & 15.783 & 16.435 & 16.957 & 15.783 \\
7     & 17.304 & 17     & 15.304 & 15.826 & 16.348 & 16     & 16.391 & 16.217 & 17     & 16.174 \\
8     & 17.522 & 17.043 & 15.87  & 16     & 16.739 & 16.348 & 16.652 & 17     & 17.739 & 16.478 \\
9     & 18.391 & 17.13  & 15.652 & 15.304 & 17.087 & 16.652 & 17.565 & 16.957 & 17.913 & 16.217 \\
10    & 18.87  & 17.304 & 15.783 & 16     & 16.957 & 16.739 & 17.957 & 18.13  & 18.739 & 16.261 \\
11    & 19.261 & 17.478 & 16.261 & 16.696 & 17     & 16.522 & 18.522 & 18.522 & 19.652 & 17.261 \\
12    & 20.174 & 17.13  & 16.304 & 17.957 & 17.043 & 16.522 & 18.696 & 18.609 & 19.913 & 17.739 \\
13    & 20.043 & 17.609 & 16.261 & 18.826 & 17.391 & 16.87  & 18.565 & 18.957 & 20.348 & 18.826 \\
14    & 21.087 & 18.261 & 16.609 & 18.478 & 17.087 & 18.13  & 18.348 & 19.043 & 19.913 & 19.696 \\
15    & 21.522 & 18.522 & 16.565 & 19.13  & 17.478 & 18.304 & 18.174 & 19.87  & 20     & 19.652 \\
16    & 21.913 & 18.783 & 16.957 & 19.043 & 16.87  & 19.391 & 18.783 & 20.652 & 19.957 & 19.87  \\
17    & 23.826 & 18.652 & 17.609 & 18.522 & 17.217 & 20.13  & 19.783 & 21.043 & 20.478 & 20.348 \\
18    & 23.87  & 18.913 & 17.261 & 18.957 & 17.87  & 20.13  & 20.522 & 21.565 & 21     & 20.913 \\
19    & 25.478 & 18.957 & 17.087 & 19.739 & 18.087 & 19.87  & 21.13  & 21.739 & 21.435 & 20.826 \\
20    & 25.565 & 19.087 & 17.043 & 20.261 & 18.261 & 19.435 & 21.609 & 21.783 & 21.478 & 20.696 \\
21    & 25.478 & 19.217 & 17.391 & 20.826 & 19.13  & 20.217 & 22.696 & 22.348 & 21.565 & 20.609 \\
22    & 26.087 & 19.565 & 18.043 & 21.826 & 19.043 & 21     & 23.304 & 22.348 & 21.913 & 22.087 \\
23    & 25.652 & 20.957 & 18.348 & 21.913 & 19.826 & 21.957 & 24.261 & 23.609 & 22.435 & 22.435 \\
24    & 26     & 20.913 & 18.478 & 22     & 20     & 22.652 & 24.565 & 23.522 & 23.043 & 23.13  \\
25    & 26.826 & 21.609 & 19.87  & 22.348 & 20.565 & 23.261 & 25.565 & 23.913 & 22.87  & 23.609 \\
26    & 27.261 & 21.652 & 19.696 & 22.696 & 21.087 & 22.174 & 27.478 & 25.13  & 23.217 & 23.739 \\
27    & 27.348 & 21.609 & 19.391 & 23.522 & 21.826 & 22.522 & 28.435 & 26.043 & 23.522 & 24.261 \\
28    & 27.478 & 21.391 & 20.348 & 23.217 & 22.783 & 22.739 & 28.826 & 26.696 & 24.174 & 25.522 \\
29    & 28.087 & 21.261 & 20.609 & 23.957 & 23.435 & 23.87  & 29.043 & 26.696 & 24.652 & 25.913 \\
30    & 28     & 22.87  & 21.261 & 24.174 & 23.13  & 24.739 & 29.261 & 26.391 & 24.87  & 25.957 \\
31    & 28.739 & 22.87  & 21.043 & 24.826 & 24.826 & 25.522 & 29.652 & 27.565 & 25.043 & 27.261 \\
32    & 28.957 & 22.435 & 20.043 & 25.783 & 26     & 25.739 & 29.87  & 28.13  & 25.826 & 28.174 \\
33    & 29.87  & 23     & 20.087 & 27     & 26.087 & 27.043 & 30.565 & 28.261 & 26.87  & 28.565 \\
34    & 29.739 & 23.826 & 20.87  & 27.391 & 26.783 & 27.435 & 31.261 & 28.261 & 27.391 & 28.696 \\
35    & 30.87  & 23.783 & 21.609 & 28.217 & 27.13  & 28.174 & 31.739 & 28.652 & 27.348 & 29.304 \\
36    & 30.87  & 24.261 & 22.565 & 28.261 & 27.435 & 28.87  & 31.913 & 26.739 & 27.13  & 29.348 \\
37    & 31.609 & 24.522 & 22.435 & 29.783 & 26.783 & 28.565 & 32.13  & 27.609 & 27.478 & 29.565 \\
38    & 31.739 & 24.13  & 23.435 & 30.174 & 26.348 & 28.826 & 32.609 & 28.913 & 27.826 & 30.174 \\
39    & 31.87  & 24.304 & 24.304 & 30.391 & 27.522 & 29.696 & 32     & 29.174 & 29.565 & 29.783 \\
40    & 32.13  & 24.478 & 24.696 & 28.826 & 27.783 & 30.043 & 33     & 29.043 & 30.13  & 29.565 \\
41    & 32.957 & 24.348 & 24.957 & 30.217 & 29.087 & 30.348 & 34.565 & 29.652 & 30.913 & 29.565 \\
42    & 33.217 & 24.522 & 25.391 & 31     & 30.565 & 29.696 & 35.174 & 29.87  & 30.87  & 29.348 \\
43    & 33.043 & 25.652 & 25.957 & 32.348 & 30.609 & 29.826 & 35.087 & 29.304 & 30.652 & 30.174 \\
44    & 32.609 & 25.696 & 26.739 & 33.043 & 29.87  & 30.435 & 34.739 & 30.087 & 30.522 & 29.913 \\
45    & 32.348 & 26.739 & 26.913 & 33.348 & 30.217 & 31.435 & 35.304 & 30.217 & 30.652 & 30.174 \\
46    & 33.435 & 27.957 & 27.435 & 33.565 & 31.13  & 31.087 & 34.565 & 30.217 & 31.043 & 29.826 \\
47    & 34.391 & 27.609 & 28.261 & 34     & 32.304 & 30.522 & 35.043 & 31.261 & 30.13  & 29.696 \\
48    & 35.522 & 29     & 28.609 & 34.783 & 33.739 & 30.565 & 35.652 & 30.652 & 31.087 & 30.478 \\
49    & 35.478 & 27.609 & 30.826 & 34.261 & 34.087 & 31.13  & 35.087 & 31.13  & 30.652 & 31.174 \\
50    & 35.435 & 29     & 31.739 & 35.261 & 34.478 & 31.087 & 35.174 & 33.087 & 31.391 & 31.522 \\
51    & 35.217 & 29.435 & 32.913 & 36.826 & 34.087 & 32     & 35.13  & 30.696 & 30.696 & 32.217 \\
52    & 36     & 28.826 & 33.435 & 37.261 & 34.739 & 32.087 & 33.739 & 30.478 & 32.217 & 32.739 \\
53    & 37.087 & 29.391 & 33.609 & 37.304 & 34.043 & 32.043 & 35.217 & 29.565 & 33.435 & 33.13  \\
54    & 37.391 & 30.348 & 34     & 37.783 & 33.261 & 30.174 & 35.87  & 31     & 33.957 & 33.87  \\
55    & 38.652 & 31.174 & 34.696 & 37     & 33.826 & 30.217 & 35.913 & 31.391 & 34.783 & 34.391 \\
56    & 38.652 & 31.435 & 34.13  & 35.609 & 34.348 & 30.565 & 36.13  & 31.913 & 35.652 & 34.087 \\
57    & 38.174 & 31.391 & 34.783 & 36.13  & 34.652 & 31.522 & 35.565 & 32.609 & 36.739 & 35.217 \\
58    & 37.348 & 31.957 & 35.435 & 38.652 & 34.609 & 32.957 & 35.478 & 33.304 & 36.783 & 35.522 \\
59    & 38.304 & 32     & 36.739 & 39.565 & 34.565 & 34.043 & 36.217 & 34.87  & 37.696 & 36.13  \\
60    & 38.609 & 32.957 & 36.913 & 38.957 & 33.565 & 35.304 & 35.783 & 34.957 & 37.435 & 37.783 \\
61    & 38.348 & 32.609 & 36.478 & 39.826 & 34.217 & 36.087 & 33.913 & 34.304 & 38.826 & 37.609 \\
62    & 38.217 & 32.739 & 36.783 & 39     & 34.261 & 36.174 & 35.174 & 34.522 & 39.478 & 38.043 \\
63    & 37.739 & 32.261 & 36     & 37.826 & 33.348 & 36.522 & 35.522 & 34.87  & 40.13  & 38.174 \\
64    & 37.261 & 32.652 & 36.739 & 38.522 & 33.522 & 38.174 & 35.391 & 35     & 40     & 37.739 \\
65    & 36.696 & 33.304 & 38.261 & 38.304 & 33.739 & 39.522 & 35.913 & 34.783 & 40.478 & 38     \\
66    & 37.435 & 35.217 & 39.348 & 39.304 & 34.739 & 38.217 & 37.217 & 34.652 & 40.652 & 38.696 \\
67    & 38.043 & 33.043 & 39.609 & 39.304 & 34.261 & 37.261 & 38.565 & 33.826 & 41.087 & 40.087 \\
68    & 37.87  & 32.87  & 41.522 & 38.13  & 34.522 & 38.87  & 39.087 & 34.957 & 40.478 & 41.522 \\
69    & 37.522 & 32.261 & 42     & 28.652 & 35.913 & 39.696 & 40     & 35.13  & 41.348 & 41.435 \\
70    & 36     & 31.435 & 42.87  & 29.739 & 36.391 & 40.391 & 40.652 & 34.435 & 41.87  & 42.783 \\
71    & 36.87  & 32.739 & 43.478 & 17.609 & 38     & 39.652 & 41.348 & 31.565 & 42.304 & 42.348 \\
72    & 36.739 & 33.696 & 43.696 & 18.261 & 39.043 & 40.435 & 39.478 & 30.043 & 42.13  & 42.522 \\
73    & 37.696 & 34     & 44.217 & 18.783 & 39.565 & 40.609 & 38.261 & 32.87  & 42.217 & 42.957 \\
74    & 38.913 & 34.913 & 44.174 & 20.826 & 40.783 & 40.304 & 38.913 & 31.696 & 41.696 & 43.391 \\
75    & 39.565 & 34.739 & 44.261 & 21.043 & 40.957 & 40.13  & 39.13  & 33.391 & 38.391 & 41.478 \\
76    & 40.435 & 34.478 & 43     & 23.043 & 41.13  & 41.696 & 39.435 & 31.174 & 39.304 & 41.826 \\
77    & 39.826 & 35.174 & 42.043 & 24.348 & 41.609 & 40.261 & 40.957 & 30.957 & 38.87  & 40.696 \\
78    & 38.522 & 33.348 & 42.043 & 24.217 & 40.304 & 39.261 & 39.739 & 31.304 & 40.391 & 41.087 \\
79    & 37.043 & 34.217 & 42.652 & 23.652 & 40.913 & 38.435 & 38.739 & 31.13  & 42     & 41     \\
\bottomrule\end{longtable}
\normalsize
