# Supplementary material for: Rehearsal-Free Continual Learning over Small Non-I.I.D. Batches
Source: arXiv:1907.03799 source file (2020-04-21)
Supplement: Supplementary file 17 [file 79_LWF.tex]

\subsection{LWF, NICv2 - 79}
\fontsize{8}{11}\selectfont
\begin{longtable}[c]{rgrgrgrgrgr}
\hline
Batch & Run 0  & Run 1  & Run 2  & Run 3  & Run 4  & Run 5  & Run 6  & Run 7  & Run 8  & Run 9  \\ \hline
\endfirsthead
\endhead
0     & 1.522  & 1.522  & 1.522  & 1.522  & 1.522  & 1.522  & 1.522  & 1.522  & 1.522  & 1.522  \\
1     & 13.826 & 13.783 & 13.826 & 13.87  & 13.87  & 13.87  & 13.826 & 13.87  & 13.87  & 13.87  \\
2     & 14.304 & 14.565 & 13.391 & 14.261 & 14.522 & 13.696 & 13.957 & 14.087 & 14.522 & 13.696 \\
3     & 14.652 & 14.913 & 14.652 & 15.087 & 14.348 & 14.304 & 13.783 & 14.522 & 14.913 & 13.913 \\
4     & 15.13  & 14.783 & 14.87  & 14.87  & 14.435 & 13.957 & 14.957 & 15.261 & 15.087 & 14.391 \\
5     & 15.565 & 15.217 & 14.652 & 15.174 & 15     & 14.957 & 15     & 15.13  & 15.391 & 15.652 \\
6     & 16.043 & 15.652 & 14.696 & 15.304 & 14.87  & 15.174 & 14.913 & 15.652 & 15.739 & 15.478 \\
7     & 17.087 & 15.696 & 15.217 & 15.696 & 15.478 & 15.522 & 15.13  & 16.348 & 15.435 & 15.478 \\
8     & 17.304 & 15.522 & 15.87  & 15.739 & 16.087 & 15.87  & 15.478 & 17.261 & 16.391 & 15.739 \\
9     & 17.609 & 15.783 & 15.913 & 15.348 & 15.913 & 15.696 & 16.913 & 17.304 & 17.217 & 15.87  \\
10    & 17.913 & 16.565 & 15.783 & 15.261 & 16.913 & 16.174 & 18.522 & 17.696 & 17.478 & 15.783 \\
11    & 18.522 & 16.609 & 16.304 & 17.087 & 17.174 & 16.652 & 18.739 & 18.522 & 17.957 & 17.391 \\
12    & 19.522 & 15.87  & 16.435 & 17.522 & 17.174 & 16.565 & 18.565 & 19.217 & 18.174 & 18.522 \\
13    & 19.217 & 16.826 & 16.87  & 17.87  & 17.478 & 17.217 & 18.261 & 19.087 & 18.913 & 20.13  \\
14    & 19.478 & 17.348 & 16.739 & 18.391 & 17.348 & 18.565 & 18.522 & 19.087 & 18.826 & 20.435 \\
15    & 19.913 & 18.217 & 16.739 & 18.565 & 17.696 & 18.87  & 19.174 & 20.087 & 18.957 & 20.391 \\
16    & 20.304 & 18.043 & 17.304 & 19.087 & 17.391 & 19.087 & 19.696 & 20     & 19.478 & 20.696 \\
17    & 20.478 & 17.609 & 17.652 & 19.043 & 17.913 & 20.13  & 20.174 & 20.304 & 19.304 & 21     \\
18    & 22.565 & 17.913 & 18.739 & 18.522 & 18.087 & 20.087 & 21.565 & 20.913 & 20.217 & 21.783 \\
19    & 23.348 & 18.174 & 19.435 & 19.435 & 18.391 & 20.217 & 21.696 & 21.609 & 20.565 & 21.913 \\
20    & 24.13  & 18.087 & 20.043 & 20.478 & 18.435 & 20.957 & 22.783 & 21.565 & 21.304 & 21.696 \\
21    & 23.913 & 18.783 & 19.435 & 21.13  & 19.522 & 20.826 & 21.913 & 22.522 & 21.13  & 21.957 \\
22    & 24     & 19     & 19.435 & 20.609 & 19.87  & 21.261 & 22.957 & 23.261 & 22     & 22.913 \\
23    & 24.696 & 19.87  & 20.13  & 21.739 & 20.739 & 20.957 & 24.348 & 22.478 & 22.304 & 23.087 \\
24    & 26.391 & 21.087 & 19.913 & 21.826 & 21.087 & 22.652 & 24.304 & 22.87  & 23.304 & 23.739 \\
25    & 26.348 & 21.739 & 21.522 & 22.087 & 19.261 & 23.13  & 25.174 & 21.87  & 23.391 & 24.565 \\
26    & 26.957 & 20.391 & 21.783 & 21.609 & 18.652 & 23.391 & 25.739 & 23.217 & 23.348 & 24.783 \\
27    & 28.043 & 19.304 & 21.391 & 22.696 & 19.696 & 22.348 & 27.261 & 24.913 & 23.957 & 25.174 \\
28    & 26.739 & 18.391 & 21.826 & 22.957 & 22.826 & 22.565 & 26.783 & 23.913 & 24.478 & 25.652 \\
29    & 26.478 & 19.174 & 22.304 & 23.043 & 24.565 & 23.217 & 24.522 & 24.043 & 25.348 & 25.652 \\
30    & 26.783 & 20.13  & 21.783 & 23.174 & 25.348 & 22.565 & 24.913 & 22.087 & 25.435 & 25.13  \\
31    & 28.043 & 19.957 & 21.609 & 23.435 & 25.87  & 22.652 & 25.739 & 23.739 & 23.739 & 25.957 \\
32    & 29.087 & 18.522 & 21.609 & 24.739 & 26.13  & 24.435 & 25.304 & 25.304 & 23.739 & 26.826 \\
33    & 29.348 & 18.217 & 21.957 & 23.783 & 25.478 & 25.826 & 25.435 & 25.957 & 24.435 & 26.783 \\
34    & 29.348 & 19.696 & 22.087 & 24.348 & 26     & 25.391 & 27.565 & 27.478 & 25.565 & 28.087 \\
35    & 29.609 & 21     & 22.739 & 25.478 & 27.565 & 25.391 & 28.348 & 26.391 & 25.217 & 28.783 \\
36    & 29.522 & 21.783 & 24.348 & 25.739 & 28.13  & 25.87  & 29.13  & 25.652 & 25.565 & 27.913 \\
37    & 29.565 & 20.304 & 26.565 & 26.652 & 28.13  & 26.043 & 29.13  & 26.13  & 24.522 & 27.391 \\
38    & 29.957 & 21.565 & 26.087 & 27.13  & 28.87  & 27.087 & 28.652 & 26.522 & 22.304 & 28.652 \\
39    & 29.043 & 22.87  & 25.609 & 27.652 & 30.565 & 26.348 & 28.391 & 28.13  & 24.522 & 28.652 \\
40    & 30.435 & 20.478 & 25.957 & 28.739 & 31.609 & 25.217 & 27.913 & 29.217 & 26.304 & 28.087 \\
41    & 29.783 & 21.391 & 25.783 & 27.348 & 30.391 & 26.304 & 29.087 & 29.043 & 27.739 & 27.913 \\
42    & 30.304 & 24.043 & 28     & 28.522 & 30.217 & 25.913 & 30.13  & 29     & 27.348 & 28.739 \\
43    & 30.435 & 23.391 & 27.826 & 29.087 & 30.348 & 26.043 & 31.304 & 28.87  & 27.348 & 28.13  \\
44    & 30.522 & 21.174 & 26.043 & 28.391 & 29.087 & 27.087 & 30.522 & 28.696 & 26.435 & 29.217 \\
45    & 30.217 & 21     & 25.435 & 27.261 & 28.913 & 29.043 & 31.478 & 27.652 & 26.783 & 30.87  \\
46    & 30.826 & 22.304 & 27.522 & 27.043 & 29.565 & 29.13  & 32.304 & 27.696 & 28.217 & 30.739 \\
47    & 30.348 & 23.174 & 27.217 & 26.565 & 30     & 26.304 & 32     & 27.217 & 25.739 & 30.913 \\
48    & 31.87  & 24.435 & 27.957 & 27.478 & 30.87  & 25.87  & 29.391 & 26.478 & 24.478 & 31.087 \\
49    & 30.87  & 25.652 & 30.174 & 26.435 & 31.522 & 27.826 & 29.087 & 26.217 & 24.739 & 30     \\
50    & 30.565 & 24.87  & 30.087 & 25.739 & 32.217 & 27.913 & 30.304 & 28.87  & 25.652 & 29.478 \\
51    & 31.304 & 23.043 & 30.522 & 29.217 & 32.174 & 28.304 & 29.957 & 26.478 & 25.565 & 29.696 \\
52    & 32.696 & 20.565 & 29.696 & 29.522 & 32.217 & 25.565 & 29.565 & 25.087 & 24.478 & 31.087 \\
53    & 35     & 23.565 & 30.87  & 29.87  & 31.652 & 25.174 & 28.826 & 25.435 & 24.609 & 30.261 \\
54    & 33.348 & 25.348 & 30.043 & 32.174 & 30.957 & 24.13  & 29     & 26.652 & 27.174 & 31.478 \\
55    & 32.696 & 23.478 & 30.043 & 33.087 & 31.478 & 24.565 & 29.13  & 29.435 & 28.826 & 32.174 \\
56    & 34.522 & 24.957 & 30.217 & 33.348 & 30.913 & 26.565 & 29.783 & 29.913 & 29.435 & 29.826 \\
57    & 34.261 & 26.348 & 31.739 & 32.348 & 32.261 & 28.087 & 29.609 & 30.739 & 29.478 & 32.478 \\
58    & 34.043 & 27.696 & 33     & 33     & 33.217 & 30.174 & 30.652 & 31.87  & 28.87  & 34.478 \\
59    & 33.739 & 27.783 & 31.739 & 33     & 31.217 & 29.87  & 31.435 & 30.304 & 30.87  & 34.957 \\
60    & 34.826 & 25.478 & 29.217 & 34.087 & 31.348 & 30.913 & 31.609 & 30.87  & 29.565 & 36.304 \\
61    & 35.217 & 26.565 & 29.391 & 32.522 & 32.217 & 30.174 & 29.304 & 31.043 & 28.261 & 36.565 \\
62    & 34     & 27.391 & 30     & 30.522 & 32.957 & 28.696 & 31     & 30.478 & 29.739 & 35.217 \\
63    & 32.87  & 27.696 & 29.435 & 29.696 & 31     & 28.565 & 30.261 & 29.696 & 32.435 & 35.913 \\
64    & 31.783 & 26.391 & 27.783 & 29.348 & 27.304 & 30.87  & 29.565 & 29.609 & 32.391 & 35.174 \\
65    & 32.174 & 26.522 & 27.522 & 27.261 & 28.478 & 32.304 & 30.826 & 31.609 & 32.565 & 34.348 \\
66    & 32.174 & 28.783 & 28.783 & 29.304 & 30.304 & 31     & 32.391 & 28.87  & 32.174 & 34.13  \\
67    & 30.783 & 29.087 & 28.696 & 30.609 & 28.174 & 31.261 & 32     & 26.217 & 31.957 & 34.522 \\
68    & 31.652 & 27.913 & 31.739 & 30.652 & 28.391 & 33.304 & 32.87  & 27.913 & 32.478 & 35.261 \\
69    & 32.652 & 26.304 & 32.652 & 31.957 & 31.609 & 33.565 & 32.087 & 28.478 & 34.261 & 35.391 \\
70    & 32.652 & 26.087 & 31.826 & 30.043 & 31.652 & 34.522 & 32.304 & 29.13  & 34.261 & 35.957 \\
71    & 33.957 & 27.217 & 30.522 & 24.522 & 30.261 & 34.652 & 30.348 & 27.478 & 33.043 & 32.087 \\
72    & 32.696 & 26.261 & 29.391 & 23.913 & 30.783 & 33.261 & 28.783 & 24.652 & 33.261 & 31.261 \\
73    & 32.435 & 24.087 & 29.348 & 24.391 & 28.87  & 33.13  & 26.043 & 27.13  & 32.087 & 29.826 \\
74    & 33.435 & 23.478 & 26.609 & 27.174 & 30.13  & 32.348 & 23.304 & 24.13  & 31.652 & 33.348 \\
75    & 32.217 & 22.391 & 27.565 & 24.913 & 32.217 & 30.957 & 23.217 & 23.565 & 28.739 & 30.565 \\
76    & 30.826 & 21.304 & 26.304 & 23.522 & 31.304 & 30.783 & 25.522 & 22.261 & 29     & 29.217 \\
77    & 31.087 & 22.174 & 27.391 & 26.522 & 30.609 & 26.261 & 27.217 & 22.609 & 28.261 & 29.217 \\
78    & 29.348 & 22.261 & 27.783 & 27.391 & 29.783 & 26.957 & 26.261 & 22.87  & 27.522 & 30.043 \\
79    & 26.739 & 21.957 & 28.826 & 25     & 30.957 & 26.522 & 27     & 23.87  & 28.261 & 31.304 \\
\bottomrule\end{longtable}
\normalsize
