# Supplementary material for: Rehearsal-Free Continual Learning over Small Non-I.I.D. Batches
Source: arXiv:1907.03799 source file (2020-04-21)
Supplement: Supplementary file 18 [file 79_NAIVE.tex]

\subsection{Naive, NICv2 - 79}
\fontsize{8}{11}\selectfont
\begin{longtable}[c]{rgrgrgrgrgr}
\hline
Batch & Run 0  & Run 1  & Run 2  & Run 3  & Run 4  & Run 5  & Run 6  & Run 7  & Run 8  & Run 9  \\ \hline
\endfirsthead
\endhead
0     & 1.522  & 1.522  & 1.522  & 1.522  & 1.522  & 1.522  & 1.522  & 1.522  & 1.522  & 1.522  \\ 
1     & 13.826 & 13.826 & 13.87  & 13.87  & 13.87  & 13.826 & 13.826 & 13.826 & 13.87  & 13.87  \\ 
2     & 14.391 & 14.478 & 13.478 & 14.13  & 14.435 & 13.652 & 13.783 & 14.13  & 14.478 & 13.696 \\ 
3     & 14.609 & 14.783 & 14.739 & 14.957 & 14.478 & 14.043 & 13.826 & 14.435 & 14.826 & 13.913 \\ 
4     & 15.261 & 14.826 & 14.739 & 14.696 & 14.478 & 13.739 & 14.435 & 14.87  & 15     & 14.435 \\ 
5     & 15.652 & 15.174 & 14.696 & 15.087 & 14.913 & 14.739 & 14.478 & 14.957 & 15.565 & 15.13  \\ 
6     & 16.087 & 15.783 & 14.609 & 15.087 & 14.565 & 14.957 & 14.87  & 15.391 & 15.348 & 15.391 \\ 
7     & 16.783 & 15.435 & 14.739 & 15.391 & 15.087 & 15.304 & 14.783 & 15.783 & 15.043 & 15.478 \\ 
8     & 17     & 15.348 & 15.13  & 15.826 & 15.783 & 15.522 & 14.739 & 16.435 & 15.739 & 15.304 \\ 
9     & 16.783 & 15.565 & 15.696 & 15.217 & 16.087 & 14.826 & 15.957 & 16.739 & 16.783 & 15.435 \\ 
10    & 17.522 & 15.87  & 15.739 & 15.087 & 16.043 & 15.652 & 17.478 & 16.783 & 17     & 15.696 \\ 
11    & 17.565 & 16     & 16.13  & 16.174 & 16.522 & 16.174 & 18     & 17.348 & 18.217 & 16.261 \\ 
12    & 18.087 & 15.696 & 16.391 & 16.739 & 16.696 & 16.261 & 17.609 & 17.826 & 19.043 & 16.739 \\ 
13    & 18.478 & 16.304 & 16.652 & 16.435 & 16.826 & 16.739 & 17.174 & 18.087 & 18.739 & 17.87  \\ 
14    & 19.435 & 17.043 & 16.304 & 17.087 & 16.565 & 17.652 & 17.652 & 18.348 & 18.826 & 18.783 \\ 
15    & 19.478 & 17.696 & 16.391 & 18     & 17.696 & 18.217 & 17.565 & 18.348 & 19.087 & 18.957 \\ 
16    & 20.043 & 17.87  & 17.043 & 18.391 & 17.652 & 17.696 & 18.348 & 18.87  & 18.957 & 19.13  \\ 
17    & 20.13  & 17.478 & 17.522 & 18.913 & 18.348 & 18.435 & 19.13  & 19.174 & 19.13  & 19.739 \\ 
18    & 21.522 & 17.087 & 18     & 18.696 & 18     & 19.087 & 20     & 19.565 & 19.522 & 20.565 \\ 
19    & 21.565 & 17.478 & 18.435 & 19.13  & 17.87  & 19.696 & 20.522 & 20.087 & 19.652 & 20.565 \\ 
20    & 22.87  & 17.957 & 19.043 & 18.957 & 18.043 & 20.174 & 21.087 & 20.261 & 20.652 & 20.478 \\ 
21    & 23.435 & 18.826 & 18.913 & 20.174 & 18.217 & 20.217 & 20.957 & 21.13  & 20.565 & 21.13  \\ 
22    & 23.739 & 19.217 & 18.609 & 20.304 & 18.739 & 20.565 & 21.391 & 21.609 & 20.783 & 21.435 \\ 
23    & 24.478 & 19.217 & 18.609 & 20.87  & 19.435 & 20.565 & 22.391 & 21.739 & 21.217 & 21.783 \\ 
24    & 25.13  & 20.826 & 19     & 21.087 & 19.565 & 21.435 & 22.87  & 21.913 & 22     & 22.87  \\ 
25    & 25.652 & 20.957 & 19.826 & 20.696 & 19.13  & 22.391 & 23.261 & 22.087 & 22.957 & 23.696 \\ 
26    & 26.478 & 21.217 & 20     & 20.696 & 18.087 & 22.826 & 24.913 & 22.348 & 22.609 & 23.348 \\ 
27    & 26.522 & 19.565 & 20.174 & 21.174 & 18.739 & 21.826 & 26.957 & 24.391 & 23.043 & 24.043 \\ 
28    & 26.261 & 19.826 & 20.565 & 22.348 & 21.565 & 21.87  & 26.565 & 23.565 & 23.435 & 24.87  \\ 
29    & 25.739 & 19.826 & 20.783 & 22.391 & 22.391 & 22.826 & 24.783 & 23.826 & 24.522 & 24.696 \\ 
30    & 25.696 & 20.565 & 20.565 & 22.391 & 23.565 & 22.435 & 25.304 & 22.174 & 24.261 & 24.609 \\ 
31    & 27     & 20.217 & 20.739 & 22.565 & 24.174 & 21.913 & 26.522 & 23.391 & 23.13  & 25.13  \\ 
32    & 28.217 & 18.739 & 20.348 & 23.391 & 25.043 & 22.87  & 25.87  & 24.565 & 22.913 & 26.043 \\ 
33    & 27.739 & 17.783 & 20.174 & 24.087 & 25.13  & 25.043 & 25.609 & 24.652 & 24.261 & 26.739 \\ 
34    & 27.261 & 19.348 & 21.348 & 24.13  & 25.304 & 24.696 & 26.87  & 25.913 & 25.087 & 27.391 \\ 
35    & 27.696 & 21     & 21.478 & 24.261 & 25.957 & 25.304 & 28.826 & 26.174 & 25     & 27.478 \\ 
36    & 27.696 & 21.391 & 22.304 & 24.783 & 26.478 & 24.957 & 29.174 & 25.783 & 25.217 & 26.826 \\ 
37    & 28.174 & 19.957 & 23.783 & 26.043 & 25.87  & 25.609 & 29.217 & 26.043 & 25.348 & 26.478 \\ 
38    & 28.739 & 20.391 & 24.304 & 26.478 & 26.826 & 26.13  & 28.913 & 26.261 & 23.696 & 27.913 \\ 
39    & 28.087 & 21.739 & 24.217 & 26.826 & 28.696 & 26.304 & 28.478 & 26.435 & 24.783 & 27.957 \\ 
40    & 29.043 & 20.783 & 24.652 & 27.261 & 28.696 & 25.478 & 29.348 & 27.652 & 27.13  & 27.522 \\ 
41    & 28.304 & 21.783 & 24.826 & 27.217 & 29.348 & 26.043 & 29.826 & 28.261 & 28.304 & 27.087 \\ 
42    & 28.304 & 24.261 & 25.696 & 27.348 & 29.174 & 25.957 & 30.087 & 28.174 & 27.522 & 27.696 \\ 
43    & 28.565 & 24.217 & 25.391 & 28.13  & 29.174 & 26     & 31     & 28.435 & 27.043 & 27.652 \\ 
44    & 27.913 & 22.174 & 24.304 & 28.435 & 28.609 & 26.652 & 30.913 & 28.478 & 27.13  & 28.565 \\ 
45    & 28     & 21.739 & 23.478 & 28.565 & 26.913 & 28.565 & 31.739 & 28.826 & 27.174 & 29.609 \\ 
46    & 29.565 & 22.087 & 24.783 & 28.174 & 28.391 & 28.957 & 32.217 & 28.739 & 28.652 & 29.522 \\ 
47    & 30.304 & 22.348 & 25.565 & 27.609 & 28.826 & 27.652 & 31.304 & 27.87  & 26.696 & 29.957 \\ 
48    & 31     & 24.043 & 26.391 & 27.957 & 29.87  & 27.957 & 29.478 & 27.391 & 26     & 29.826 \\ 
49    & 31.13  & 25.652 & 28.522 & 27.174 & 30.174 & 27.783 & 29.826 & 26.348 & 25.261 & 29.609 \\ 
50    & 30.087 & 26.217 & 28.478 & 25.957 & 30.391 & 27.87  & 30.609 & 28.261 & 26.043 & 28.609 \\ 
51    & 30.652 & 25.348 & 28.696 & 28.261 & 30.435 & 27.87  & 30.043 & 26.217 & 25.87  & 28.739 \\ 
52    & 31.826 & 22.261 & 27.913 & 29.783 & 30.696 & 26.13  & 29.652 & 25.174 & 25.087 & 29.217 \\ 
53    & 32.87  & 23.826 & 29.13  & 30.261 & 30.13  & 26.087 & 28.609 & 26.043 & 24.783 & 29.043 \\ 
54    & 31.391 & 26.304 & 29.391 & 31.478 & 30.348 & 24.696 & 28.957 & 26.696 & 27.261 & 30.565 \\ 
55    & 30.739 & 25.217 & 28.652 & 32.087 & 29.957 & 24.565 & 29.696 & 28.087 & 27.739 & 32     \\ 
56    & 31.696 & 25.652 & 29.261 & 32.696 & 29.739 & 26     & 29.696 & 27.696 & 29     & 29.739 \\ 
57    & 32.913 & 26.304 & 30.217 & 32.478 & 30.522 & 27.522 & 29.565 & 28.348 & 29.652 & 31.565 \\ 
58    & 32.217 & 26.87  & 30.913 & 33.261 & 30.565 & 29.478 & 30.261 & 30.174 & 29.304 & 32.696 \\ 
59    & 32.435 & 26.826 & 30.087 & 32.826 & 29.783 & 29.696 & 30.826 & 30     & 30.652 & 33.609 \\ 
60    & 33.478 & 26.217 & 28.565 & 33.13  & 29.217 & 29.957 & 30.87  & 29.739 & 29.522 & 33.957 \\ 
61    & 33.913 & 26.522 & 28.609 & 31.783 & 29.957 & 29.696 & 30.13  & 29.87  & 27.783 & 34.478 \\ 
62    & 34.522 & 27.565 & 28.652 & 30.826 & 31.391 & 29.174 & 30.435 & 30.261 & 29.174 & 34.522 \\ 
63    & 32.174 & 27.652 & 27.913 & 30.696 & 30.522 & 29.087 & 30     & 30.087 & 30.957 & 35.13  \\ 
64    & 31.261 & 27.391 & 26.435 & 30.043 & 28.565 & 30.522 & 28.391 & 30.13  & 31.913 & 33.696 \\ 
65    & 31.435 & 27.348 & 25.913 & 28.565 & 28.783 & 30.739 & 29.348 & 31.652 & 31.783 & 33.174 \\ 
66    & 31.174 & 28.652 & 27.957 & 29.087 & 29.652 & 30.565 & 30.087 & 30.261 & 32.391 & 32.217 \\ 
67    & 30.391 & 29.174 & 28.13  & 30.043 & 27.565 & 30.522 & 31.609 & 27.478 & 32.217 & 32.913 \\ 
68    & 30.696 & 28.826 & 30     & 29.826 & 26.826 & 31.696 & 31.957 & 28     & 32.435 & 33.304 \\ 
69    & 31.304 & 27.348 & 30.957 & 30.217 & 29.087 & 33.261 & 31.217 & 28.261 & 33.87  & 34.087 \\ 
70    & 32.043 & 27.522 & 30.826 & 30.652 & 30.565 & 34.435 & 31.783 & 28.783 & 33     & 34     \\ 
71    & 32.87  & 27     & 29.261 & 28.043 & 29.957 & 34.696 & 32.174 & 28.261 & 32.652 & 32.957 \\ 
72    & 32.261 & 26.696 & 28.391 & 25.565 & 30.261 & 33.565 & 30.652 & 26.652 & 32.783 & 31.478 \\ 
73    & 31.435 & 25.304 & 29.435 & 25.261 & 29.435 & 33.13  & 26.783 & 27.826 & 31.826 & 30.435 \\ 
74    & 32.043 & 24.826 & 27.13  & 26.739 & 31     & 32.13  & 24.478 & 25.13  & 31.913 & 30.391 \\ 
75    & 30.739 & 22.783 & 27.609 & 27.217 & 32.609 & 31     & 24.522 & 24.217 & 28.696 & 29.217 \\ 
76    & 29.565 & 21.957 & 26.087 & 26.087 & 32.261 & 30.87  & 25.522 & 23.087 & 28.522 & 28.348 \\ 
77    & 30.217 & 22     & 27.261 & 26.87  & 31.304 & 27.913 & 26.348 & 23.565 & 27.348 & 28.478 \\ 
78    & 28.696 & 22.652 & 27.652 & 27.478 & 30.304 & 28.348 & 25.478 & 23.565 & 27.304 & 29.957 \\ 
79    & 27.043 & 22.739 & 28.478 & 25.652 & 30.348 & 26.913 & 25.478 & 23.739 & 27.261 & 29.826 \\ 
\bottomrule\end{longtable}
\normalsize
