# Supplementary material for: Rehearsal-Free Continual Learning over Small Non-I.I.D. Batches
Source: arXiv:1907.03799 source file (2020-04-21)
Supplement: Supplementary file 19 [file freeze_all.tex]

\subsection{Naive, NI scenario, Frozen Depthwise and Pointwise Layers}
\fontsize{8}{11}\selectfont
\begin{longtable}[c]{rgrgrgrgrgr}
\hline
Batch & Run 0  & Run 1  & Run 2  & Run 3  & Run 4  & Run 5  & Run 6  & Run 7  & Run 8  & Run 9  \\ \hline
\endfirsthead
\endhead
1     & 47.771 & 52.407 & 46.867 & 48.371 & 40.833 & 37.078 & 44.704 & 39.662 & 37.942 & 48.849 \\
2     & 47.698 & 54.84  & 55.713 & 54.131 & 43.104 & 39.229 & 53.676 & 52.336 & 39.524 & 54.567 \\
3     & 53.642 & 58.033 & 54.173 & 60.087 & 43.502 & 45.069 & 53.036 & 49.251 & 39.371 & 57.256 \\
4     & 50.533 & 61.291 & 55.858 & 61.929 & 39.858 & 49.911 & 55.596 & 50.276 & 43.698 & 58.349 \\
5     & 48.24  & 60.569 & 57.378 & 57.664 & 45.562 & 48.5   & 61.318 & 51.804 & 46.251 & 57.413 \\
6     & 59.993 & 59.567 & 55.384 & 62.269 & 42.071 & 48.176 & 62.282 & 48.602 & 45.124 & 64.256 \\
7     & 58.033 & 59.064 & 54.569 & 62.936 & 50.353 & 42.938 & 60.156 & 44.86  & 39.14  & 65.62  \\
8     & 56.662 & 55.727 & 60.233 & 60.536 & 49.087 & 58.804 & 59.496 & 49.818 & 43.598 & 65.529 \\
\bottomrule\end{longtable}
\normalsize
