# Supplementary material for: Rehearsal-Free Continual Learning over Small Non-I.I.D. Batches
Source: arXiv:1907.03799 source file (2020-04-21)
Supplement: Supplementary file 20 [file freeze_depth.tex]

\subsection{Naive, NI scenario, Frozen Depthwise Layers}
\fontsize{8}{11}\selectfont
\begin{longtable}[c]{rgrgrgrgrgr}
\hline
Batch & Run 0  & Run 1  & Run 2  & Run 3  & Run 4  & Run 5  & Run 6  & Run 7  & Run 8  & Run 9  \\ \hline
\endfirsthead
\endhead
1     & 46.671 & 52.982 & 44.256 & 48.096 & 40.858 & 36.6   & 46.52  & 39.418 & 37.084 & 48.198 \\
2     & 49.149 & 59.52  & 58.973 & 58.207 & 48.271 & 45.373 & 57.864 & 58.26  & 45.478 & 56.293 \\
3     & 59.298 & 63.838 & 62.784 & 62.022 & 54.811 & 52.118 & 62.802 & 58.593 & 48.002 & 61.338 \\
4     & 63.504 & 68.076 & 67.107 & 64.629 & 56.229 & 59.722 & 68.093 & 65.042 & 53.591 & 67.273 \\
5     & 61.142 & 72.073 & 69.013 & 70.247 & 65.918 & 65.818 & 71.396 & 67.396 & 62.631 & 69.504 \\
6     & 65.509 & 73.502 & 71.018 & 73.622 & 69.409 & 63.329 & 74.451 & 67.94  & 60.802 & 73.102 \\
7     & 69.109 & 74.996 & 72.382 & 75.353 & 71.313 & 66.144 & 73.7   & 71.291 & 65.462 & 75.633 \\
8     & 69.498 & 75.093 & 74.691 & 74.353 & 74.709 & 67.631 & 75.2   & 68.338 & 67.496 & 76.229 \\
\bottomrule\end{longtable}
\normalsize
