# Supplementary material for: Rehearsal-Free Continual Learning over Small Non-I.I.D. Batches
Source: arXiv:1907.03799 source file (2020-04-21)
Supplement: Supplementary file 21 [file freeze_point.tex]

\subsection{Naive, NI scenario, Frozen Pointwise Layers}
\fontsize{8}{11}\selectfont
\begin{longtable}[c]{rgrgrgrgrgr}
\hline
Batch & Run 0  & Run 1  & Run 2  & Run 3  & Run 4  & Run 5  & Run 6  & Run 7  & Run 8  & Run 9  \\ \hline
\endfirsthead
\endhead
1     & 47.647 & 52.802 & 46.909 & 49.053 & 41.471 & 37.611 & 44.016 & 39.907 & 37.644 & 48.089 \\
2     & 38.967 & 51.98  & 51.927 & 57.467 & 48.411 & 40.284 & 48.238 & 48.533 & 40.629 & 54.436 \\
3     & 50.162 & 53.338 & 45.451 & 61.558 & 40.169 & 39.082 & 52.467 & 46.076 & 38.573 & 57.333 \\
4     & 46.049 & 54.262 & 49.798 & 63.269 & 38.698 & 41.984 & 59.042 & 43.498 & 38.987 & 53.884 \\
5     & 35.98  & 44.804 & 49.629 & 50.178 & 44.667 & 44.071 & 64.487 & 44.513 & 39.082 & 48.367 \\
6     & 46.367 & 53.982 & 50.733 & 56.813 & 51.427 & 38.616 & 58.847 & 42.447 & 30.831 & 60.913 \\
7     & 47.316 & 48.4   & 54.729 & 59.044 & 55.013 & 30.307 & 43.187 & 42.916 & 24.258 & 62.233 \\
8     & 48.087 & 47.807 & 55.516 & 52.344 & 62.644 & 56.756 & 43.993 & 34.069 & 30.78  & 61.673 \\
\bottomrule\end{longtable}
\normalsize
