# Supplementary material for: Rehearsal-Free Continual Learning over Small Non-I.I.D. Batches
Source: arXiv:1907.03799 source file (2020-04-21)
Supplement: Supplementary file 22 [file tune_all.tex]

\subsection{Naive, NI scenario, tune all (no frozen layers)}
\fontsize{8}{11}\selectfont
\begin{longtable}[c]{rgrgrgrgrgr}
\hline
Batch & Run 0  & Run 1  & Run 2  & Run 3  & Run 4  & Run 5  & Run 6  & Run 7  & Run 8  & Run 9  \\ \hline
\endfirsthead
\endhead
1     & 47.718 & 52.738 & 45.724 & 47.938 & 40.989 & 38.156 & 45.46  & 39.198 & 37.322 & 47.762 \\
2     & 47.049 & 58.802 & 61.167 & 60.133 & 49.336 & 46.842 & 54.464 & 60.047 & 46.967 & 55.924 \\
3     & 58.096 & 63.336 & 59.371 & 63.398 & 53.973 & 54.671 & 61.893 & 61.187 & 46.938 & 62.153 \\
4     & 60.702 & 67.087 & 65.867 & 64.476 & 54.833 & 59.416 & 68.004 & 65.642 & 52.209 & 66.08  \\
5     & 53.587 & 68.842 & 63.4   & 64.493 & 65.507 & 66.162 & 71.102 & 67.938 & 63.291 & 64.958 \\
6     & 59.971 & 72.356 & 70.802 & 69.84  & 71.078 & 65.236 & 72.356 & 68.067 & 63.7   & 71.771 \\
7     & 67.864 & 74.609 & 73.18  & 74.438 & 70.476 & 67.289 & 69.649 & 71.018 & 66.458 & 74.851 \\
8     & 70.573 & 72.976 & 74.422 & 72.051 & 76.478 & 66.84  & 72.673 & 66.558 & 69.022 & 75.889 \\
\bottomrule
\end{longtable}
\normalsize
